# Supplementary material for: Six Permutation Patterns Force Quasirandomness
Source: arXiv:2303.04776 ancillary file (2024-10-03)
Supplement: Supplementary file 1 [file FlagAppendix.pdf]

# Appendix A: Data for Verifying the Flag Algebra Proof

The purpose of this appendix is to provide data that can be used to verify equation (3.4) in the proof of Theorem 3.1. In particular, we include the expression $\sum_{\pi \in S_6} d(\rho^*, \pi) \cdot \pi$ and all of the expressions $[\![x_i \times x_j]\!]$ and $[\![y_i \times y_j]\!]$ for $1 \le i \le j \le 5$ in their entirety. We have written Java programs that can be used to compute all of the coefficients given below; they have been made available at `https://github.com/pbd345/qr-perms/blob/8bd59855a6afdc0f4e0cb605e3afaeec7f2317f9/FlagProof.zip`.

$$
\begin{aligned}
\sum_{\pi \in S_6} d(\rho^*, \pi) \cdot \pi = {} & 123456 + \frac{4}{5} \cdot 123465 + \frac{4}{5} \cdot 123546 + \frac{13}{20} \cdot 123564 + \frac{13}{20} \cdot 123645 + \frac{11}{20} \cdot 123654 \\
& + \frac{4}{5} \cdot 124356 + \frac{2}{3} \cdot 124365 + \frac{13}{20} \cdot 124536 + \frac{11}{20} \cdot 124563 + \frac{8}{15} \cdot 124635 + \frac{9}{20} \cdot 124653 \\
& + \frac{13}{20} \cdot 125346 + \frac{8}{15} \cdot 125364 + \frac{11}{20} \cdot 125436 + \frac{9}{20} \cdot 125463 + \frac{7}{15} \cdot 125634 + \frac{2}{5} \cdot 125643 \\
& + \frac{11}{20} \cdot 126345 + \frac{9}{20} \cdot 126354 + \frac{9}{20} \cdot 126435 + \frac{2}{5} \cdot 126453 + \frac{2}{5} \cdot 126534 + \frac{2}{5} \cdot 126543 \\
& + \frac{4}{5} \cdot 132456 + \frac{2}{3} \cdot 132465 + \frac{2}{3} \cdot 132546 + \frac{7}{12} \cdot 132564 + \frac{7}{12} \cdot 132645 + \frac{11}{20} \cdot 132654 \\
& + \frac{13}{20} \cdot 134256 + \frac{7}{12} \cdot 134265 + \frac{11}{20} \cdot 134526 + \frac{1}{2} \cdot 134562 + \frac{7}{15} \cdot 134625 + \frac{2}{5} \cdot 134652 \\
& + \frac{8}{15} \cdot 135246 + \frac{29}{60} \cdot 135264 + \frac{9}{20} \cdot 135426 + \frac{2}{5} \cdot 135462 + \frac{13}{30} \cdot 135624 + \frac{7}{20} \cdot 135642 \\
& + \frac{7}{15} \cdot 136245 + \frac{13}{30} \cdot 136254 + \frac{23}{60} \cdot 136425 + \frac{7}{20} \cdot 136452 + \frac{11}{30} \cdot 136524 + \frac{7}{20} \cdot 136542 \\
& + \frac{13}{20} \cdot 142356 + \frac{7}{12} \cdot 142365 + \frac{8}{15} \cdot 142536 + \frac{7}{15} \cdot 142563 + \frac{29}{60} \cdot 142635 + \frac{13}{30} \cdot 142653 \\
& + \frac{11}{20} \cdot 143256 + \frac{11}{20} \cdot 143265 + \frac{9}{20} \cdot 143526 + \frac{2}{5} \cdot 143562 + \frac{13}{30} \cdot 143625 + \frac{11}{30} \cdot 143652 \\
& + \frac{7}{15} \cdot 145236 + \frac{13}{30} \cdot 145263 + \frac{2}{5} \cdot 145326 + \frac{7}{20} \cdot 145362 + \frac{9}{20} \cdot 145623 + \frac{7}{20} \cdot 145632 \\
& + \frac{13}{30} \cdot 146235 + \frac{23}{60} \cdot 146253 + \frac{11}{30} \cdot 146325 + \frac{1}{3} \cdot 146352 + \frac{23}{60} \cdot 146523 + \frac{7}{20} \cdot 146532 \\
& + \frac{11}{20} \cdot 152346 + \frac{7}{15} \cdot 152364 + \frac{9}{20} \cdot 152436 + \frac{23}{60} \cdot 152463 + \frac{13}{30} \cdot 152634 + \frac{11}{30} \cdot 152643 \\
& + \frac{9}{20} \cdot 153246 + \frac{13}{30} \cdot 153264 + \frac{2}{5} \cdot 153426 + \frac{7}{20} \cdot 153462 + \frac{23}{60} \cdot 153624 + \frac{1}{3} \cdot 153642 \\
& + \frac{2}{5} \cdot 154236 + \frac{11}{30} \cdot 154263 + \frac{2}{5} \cdot 154326 + \frac{7}{20} \cdot 154362 + \frac{23}{60} \cdot 154623 + \frac{7}{20} \cdot 154632 \\
& + \frac{9}{20} \cdot 156234 + \frac{23}{60} \cdot 156243 + \frac{23}{60} \cdot 156324 + \frac{11}{30} \cdot 156342 + \frac{11}{30} \cdot 156423 + \frac{2}{5} \cdot 156432 \\
& + \frac{1}{2} \cdot 162345 + \frac{2}{5} \cdot 162354 + \frac{2}{5} \cdot 162435 + \frac{7}{20} \cdot 162453 + \frac{7}{20} \cdot 162534 + \frac{7}{20} \cdot 162543 \\
& + \frac{2}{5} \cdot 163245 + \frac{11}{30} \cdot 163254 + \frac{7}{20} \cdot 163425 + \frac{7}{20} \cdot 163452 + \frac{1}{3} \cdot 163524 + \frac{7}{20} \cdot 163542 \\
& + \frac{7}{20} \cdot 164235 + \frac{1}{3} \cdot 164253 + \frac{7}{20} \cdot 164325 + \frac{7}{20} \cdot 164352 + \frac{11}{30} \cdot 164523 + \frac{2}{5} \cdot 164532 \\
& + \frac{7}{20} \cdot 165234 + \frac{7}{20} \cdot 165243 + \frac{7}{20} \cdot 165324 + \frac{2}{5} \cdot 165342 + \frac{2}{5} \cdot 165423 + \frac{1}{2} \cdot 165432
\end{aligned}
$$

$$+ \frac{4}{5} \cdot 213456 + \frac{2}{3} \cdot 213465 + \frac{2}{3} \cdot 213546 + \frac{7}{12} \cdot 213564 + \frac{7}{12} \cdot 213645 + \frac{11}{20} \cdot 213654$$
$$+ \frac{2}{3} \cdot 214356 + \frac{3}{5} \cdot 214365 + \frac{7}{12} \cdot 214536 + \frac{11}{20} \cdot 214563 + \frac{8}{15} \cdot 214635 + \frac{31}{60} \cdot 214653$$
$$+ \frac{7}{12} \cdot 215346 + \frac{8}{15} \cdot 215364 + \frac{11}{20} \cdot 215436 + \frac{31}{60} \cdot 215463 + \frac{8}{15} \cdot 215634 + \frac{8}{15} \cdot 215643$$
$$+ \frac{11}{20} \cdot 216345 + \frac{31}{60} \cdot 216354 + \frac{31}{60} \cdot 216435 + \frac{8}{15} \cdot 216453 + \frac{8}{15} \cdot 216534 + \frac{3}{5} \cdot 216543$$
$$+ \frac{13}{20} \cdot 231456 + \frac{7}{12} \cdot 231465 + \frac{7}{12} \cdot 231546 + \frac{17}{30} \cdot 231564 + \frac{17}{30} \cdot 231645 + \frac{3}{5} \cdot 231654$$
$$+ \frac{11}{20} \cdot 234156 + \frac{11}{20} \cdot 234165 + \frac{1}{2} \cdot 234516 + \frac{1}{2} \cdot 234561 + \frac{9}{20} \cdot 234615 + \frac{2}{5} \cdot 234651$$
$$+ \frac{7}{15} \cdot 235146 + \frac{29}{60} \cdot 235164 + \frac{2}{5} \cdot 235416 + \frac{2}{5} \cdot 235461 + \frac{9}{20} \cdot 235614 + \frac{7}{20} \cdot 235641$$
$$+ \frac{13}{30} \cdot 236145 + \frac{7}{15} \cdot 236154 + \frac{11}{30} \cdot 236415 + \frac{7}{20} \cdot 236451 + \frac{23}{60} \cdot 236514 + \frac{7}{20} \cdot 236541$$
$$+ \frac{8}{15} \cdot 241356 + \frac{8}{15} \cdot 241365 + \frac{29}{60} \cdot 241536 + \frac{29}{60} \cdot 241563 + \frac{1}{2} \cdot 241635 + \frac{31}{60} \cdot 241653$$
$$+ \frac{9}{20} \cdot 243156 + \frac{31}{60} \cdot 243165 + \frac{2}{5} \cdot 243516 + \frac{2}{5} \cdot 243561 + \frac{5}{12} \cdot 243615 + \frac{11}{30} \cdot 243651$$
$$+ \frac{13}{30} \cdot 245136 + \frac{7}{15} \cdot 245163 + \frac{7}{20} \cdot 245316 + \frac{7}{20} \cdot 245361 + \frac{1}{2} \cdot 245613 + \frac{7}{20} \cdot 245631$$
$$+ \frac{13}{30} \cdot 246135 + \frac{9}{20} \cdot 246153 + \frac{7}{20} \cdot 246315 + \frac{1}{3} \cdot 246351 + \frac{13}{30} \cdot 246513 + \frac{7}{20} \cdot 246531$$
$$+ \frac{7}{15} \cdot 251346 + \frac{9}{20} \cdot 251364 + \frac{13}{30} \cdot 251436 + \frac{13}{30} \cdot 251463 + \frac{29}{60} \cdot 251634 + \frac{29}{60} \cdot 251643$$
$$+ \frac{23}{60} \cdot 253146 + \frac{13}{30} \cdot 253164 + \frac{7}{20} \cdot 253416 + \frac{7}{20} \cdot 253461 + \frac{2}{5} \cdot 253614 + \frac{1}{3} \cdot 253641$$
$$+ \frac{11}{30} \cdot 254136 + \frac{2}{5} \cdot 254163 + \frac{7}{20} \cdot 254316 + \frac{7}{20} \cdot 254361 + \frac{13}{30} \cdot 254613 + \frac{7}{20} \cdot 254631$$
$$+ \frac{29}{60} \cdot 256134 + \frac{29}{60} \cdot 256143 + \frac{2}{5} \cdot 256314 + \frac{11}{30} \cdot 256341 + \frac{5}{12} \cdot 256413 + \frac{2}{5} \cdot 256431$$
$$+ \frac{9}{20} \cdot 261345 + \frac{5}{12} \cdot 261354 + \frac{5}{12} \cdot 261435 + \frac{13}{30} \cdot 261453 + \frac{13}{30} \cdot 261534 + \frac{1}{2} \cdot 261543$$
$$+ \frac{11}{30} \cdot 263145 + \frac{2}{5} \cdot 263154 + \frac{1}{3} \cdot 263415 + \frac{7}{20} \cdot 263451 + \frac{7}{20} \cdot 263514 + \frac{7}{20} \cdot 263541$$
$$+ \frac{7}{20} \cdot 264135 + \frac{2}{5} \cdot 264153 + \frac{1}{3} \cdot 264315 + \frac{7}{20} \cdot 264351 + \frac{5}{12} \cdot 264513 + \frac{2}{5} \cdot 264531$$
$$+ \frac{23}{60} \cdot 265134 + \frac{9}{20} \cdot 265143 + \frac{11}{30} \cdot 265314 + \frac{2}{5} \cdot 265341 + \frac{9}{20} \cdot 265413 + \frac{1}{2} \cdot 265431$$
$$+ \frac{13}{20} \cdot 312456 + \frac{7}{12} \cdot 312465 + \frac{7}{12} \cdot 312546 + \frac{17}{30} \cdot 312564 + \frac{17}{30} \cdot 312645 + \frac{3}{5} \cdot 312654$$
$$+ \frac{8}{15} \cdot 314256 + \frac{8}{15} \cdot 314265 + \frac{7}{15} \cdot 314526 + \frac{9}{20} \cdot 314562 + \frac{9}{20} \cdot 314625 + \frac{5}{12} \cdot 314652$$
$$+ \frac{29}{60} \cdot 315246 + \frac{1}{2} \cdot 315264 + \frac{13}{30} \cdot 315426 + \frac{5}{12} \cdot 315462 + \frac{29}{60} \cdot 315624 + \frac{13}{30} \cdot 315642$$
$$+ \frac{29}{60} \cdot 316245 + \frac{31}{60} \cdot 316254 + \frac{13}{30} \cdot 316425 + \frac{13}{30} \cdot 316452 + \frac{29}{60} \cdot 316524 + \frac{1}{2} \cdot 316542$$
$$+ \frac{11}{20} \cdot 321456 + \frac{11}{20} \cdot 321465 + \frac{11}{20} \cdot 321546 + \frac{3}{5} \cdot 321564 + \frac{3}{5} \cdot 321645 + \frac{7}{10} \cdot 321654$$
$$+ \frac{9}{20} \cdot 324156 + \frac{31}{60} \cdot 324165 + \frac{2}{5} \cdot 324516 + \frac{2}{5} \cdot 324561 + \frac{5}{12} \cdot 324615 + \frac{11}{30} \cdot 324651$$

$$+\frac{13}{30}\cdot 325146+\frac{31}{60}\cdot 325164+\frac{11}{30}\cdot 325416+\frac{11}{30}\cdot 325461+\frac{29}{60}\cdot 325614+\frac{23}{60}\cdot 325641$$
$$+\frac{7}{15}\cdot 326145+\frac{17}{30}\cdot 326154+\frac{2}{5}\cdot 326415+\frac{23}{60}\cdot 326451+\frac{29}{60}\cdot 326514+\frac{9}{20}\cdot 326541$$
$$+\frac{7}{15}\cdot 341256+\frac{8}{15}\cdot 341265+\frac{13}{30}\cdot 341526+\frac{9}{20}\cdot 341562+\frac{29}{60}\cdot 341625+\frac{29}{60}\cdot 341652$$
$$+\frac{2}{5}\cdot 342156+\frac{8}{15}\cdot 342165+\frac{7}{20}\cdot 342516+\frac{7}{20}\cdot 342561+\frac{13}{30}\cdot 342615+\frac{23}{60}\cdot 342651$$
$$+\frac{9}{20}\cdot 345126+\frac{1}{2}\cdot 345162+\frac{7}{20}\cdot 345216+\frac{7}{20}\cdot 345261+\frac{3}{5}\cdot 345612+\frac{2}{5}\cdot 345621$$
$$+\frac{29}{60}\cdot 346125+\frac{29}{60}\cdot 346152+\frac{23}{60}\cdot 346215+\frac{11}{30}\cdot 346251+\frac{8}{15}\cdot 346512+\frac{2}{5}\cdot 346521$$
$$+\frac{13}{30}\cdot 351246+\frac{29}{60}\cdot 351264+\frac{23}{60}\cdot 351426+\frac{2}{5}\cdot 351462+\frac{1}{2}\cdot 351624+\frac{9}{20}\cdot 351642$$
$$+\frac{11}{30}\cdot 352146+\frac{29}{60}\cdot 352164+\frac{1}{3}\cdot 352416+\frac{1}{3}\cdot 352461+\frac{9}{20}\cdot 352614+\frac{23}{60}\cdot 352641$$
$$+\frac{23}{60}\cdot 354126+\frac{13}{30}\cdot 354162+\frac{7}{20}\cdot 354216+\frac{7}{20}\cdot 354261+\frac{8}{15}\cdot 354612+\frac{2}{5}\cdot 354621$$
$$+\frac{17}{30}\cdot 356124+\frac{31}{60}\cdot 356142+\frac{7}{15}\cdot 356214+\frac{13}{30}\cdot 356241+\frac{31}{60}\cdot 356412+\frac{9}{20}\cdot 356421$$
$$+\frac{9}{20}\cdot 361245+\frac{29}{60}\cdot 361254+\frac{2}{5}\cdot 361425+\frac{2}{5}\cdot 361452+\frac{9}{20}\cdot 361524+\frac{7}{15}\cdot 361542$$
$$+\frac{23}{60}\cdot 362145+\frac{29}{60}\cdot 362154+\frac{7}{20}\cdot 362415+\frac{11}{30}\cdot 362451+\frac{13}{30}\cdot 362514+\frac{13}{30}\cdot 362541$$
$$+\frac{2}{5}\cdot 364125+\frac{13}{30}\cdot 364152+\frac{11}{30}\cdot 364215+\frac{23}{60}\cdot 364251+\frac{31}{60}\cdot 364512+\frac{9}{20}\cdot 364521$$
$$+\frac{7}{15}\cdot 365124+\frac{29}{60}\cdot 365142+\frac{13}{30}\cdot 365214+\frac{7}{15}\cdot 365241+\frac{11}{20}\cdot 365412+\frac{11}{20}\cdot 365421$$
$$+\frac{11}{20}\cdot 412356+\frac{11}{20}\cdot 412365+\frac{7}{15}\cdot 412536+\frac{13}{30}\cdot 412563+\frac{29}{60}\cdot 412635+\frac{7}{15}\cdot 412653$$
$$+\frac{9}{20}\cdot 413256+\frac{31}{60}\cdot 413265+\frac{23}{60}\cdot 413526+\frac{11}{30}\cdot 413562+\frac{13}{30}\cdot 413625+\frac{2}{5}\cdot 413652$$
$$+\frac{13}{30}\cdot 415236+\frac{13}{30}\cdot 415263+\frac{11}{30}\cdot 415326+\frac{7}{20}\cdot 415362+\frac{29}{60}\cdot 415623+\frac{23}{60}\cdot 415632$$
$$+\frac{7}{15}\cdot 416235+\frac{9}{20}\cdot 416253+\frac{2}{5}\cdot 416325+\frac{2}{5}\cdot 416352+\frac{29}{60}\cdot 416523+\frac{9}{20}\cdot 416532$$
$$+\frac{9}{20}\cdot 421356+\frac{31}{60}\cdot 421365+\frac{13}{30}\cdot 421536+\frac{7}{15}\cdot 421563+\frac{31}{60}\cdot 421635+\frac{17}{30}\cdot 421653$$
$$+\frac{2}{5}\cdot 423156+\frac{8}{15}\cdot 423165+\frac{7}{20}\cdot 423516+\frac{7}{20}\cdot 423561+\frac{13}{30}\cdot 423615+\frac{23}{60}\cdot 423651$$
$$+\frac{23}{60}\cdot 425136+\frac{9}{20}\cdot 425163+\frac{1}{3}\cdot 425316+\frac{1}{3}\cdot 425361+\frac{29}{60}\cdot 425613+\frac{11}{30}\cdot 425631$$
$$+\frac{9}{20}\cdot 426135+\frac{1}{2}\cdot 426153+\frac{2}{5}\cdot 426315+\frac{23}{60}\cdot 426351+\frac{29}{60}\cdot 426513+\frac{13}{30}\cdot 426531$$
$$+\frac{2}{5}\cdot 431256+\frac{8}{15}\cdot 431265+\frac{11}{30}\cdot 431526+\frac{23}{60}\cdot 431562+\frac{29}{60}\cdot 431625+\frac{29}{60}\cdot 431652$$
$$+\frac{2}{5}\cdot 432156+\frac{3}{5}\cdot 432165+\frac{7}{20}\cdot 432516+\frac{7}{20}\cdot 432561+\frac{1}{2}\cdot 432615+\frac{9}{20}\cdot 432651$$
$$+\frac{23}{60}\cdot 435126+\frac{13}{30}\cdot 435162+\frac{7}{20}\cdot 435216+\frac{7}{20}\cdot 435261+\frac{8}{15}\cdot 435612+\frac{2}{5}\cdot 435621$$
$$+\frac{29}{60}\cdot 436125+\frac{29}{60}\cdot 436152+\frac{9}{20}\cdot 436215+\frac{13}{30}\cdot 436251+\frac{8}{15}\cdot 436512+\frac{7}{15}\cdot 436521$$

$$
\begin{aligned}
&+ \frac{9}{20} \cdot 451236 + \frac{29}{60} \cdot 451263 + \frac{23}{60} \cdot 451326 + \frac{2}{5} \cdot 451362 + \frac{17}{30} \cdot 451623 + \frac{7}{15} \cdot 451632 \\
&+ \frac{23}{60} \cdot 452136 + \frac{29}{60} \cdot 452163 + \frac{11}{30} \cdot 452316 + \frac{11}{30} \cdot 452361 + \frac{31}{60} \cdot 452613 + \frac{13}{30} \cdot 452631 \\
&+ \frac{11}{30} \cdot 453126 + \frac{5}{12} \cdot 453162 + \frac{2}{5} \cdot 453216 + \frac{2}{5} \cdot 453261 + \frac{31}{60} \cdot 453612 + \frac{9}{20} \cdot 453621 \\
&+ \frac{7}{10} \cdot 456123 + \frac{3}{5} \cdot 456132 + \frac{3}{5} \cdot 456213 + \frac{11}{20} \cdot 456231 + \frac{11}{20} \cdot 456312 + \frac{11}{20} \cdot 456321 \\
&+ \frac{1}{2} \cdot 461235 + \frac{29}{60} \cdot 461253 + \frac{13}{30} \cdot 461325 + \frac{13}{30} \cdot 461352 + \frac{31}{60} \cdot 461523 + \frac{29}{60} \cdot 461532 \\
&+ \frac{13}{30} \cdot 462135 + \frac{29}{60} \cdot 462153 + \frac{5}{12} \cdot 462315 + \frac{13}{30} \cdot 462351 + \frac{1}{2} \cdot 462513 + \frac{29}{60} \cdot 462531 \\
&+ \frac{5}{12} \cdot 463125 + \frac{9}{20} \cdot 463152 + \frac{9}{20} \cdot 463215 + \frac{7}{15} \cdot 463251 + \frac{8}{15} \cdot 463512 + \frac{8}{15} \cdot 463521 \\
&+ \frac{3}{5} \cdot 465123 + \frac{17}{30} \cdot 465132 + \frac{17}{30} \cdot 465213 + \frac{7}{12} \cdot 465231 + \frac{7}{12} \cdot 465312 + \frac{13}{20} \cdot 465321 \\
&+ \frac{1}{2} \cdot 512346 + \frac{9}{20} \cdot 512364 + \frac{2}{5} \cdot 512436 + \frac{11}{30} \cdot 512463 + \frac{9}{20} \cdot 512634 + \frac{23}{60} \cdot 512643 \\
&+ \frac{2}{5} \cdot 513246 + \frac{5}{12} \cdot 513264 + \frac{7}{20} \cdot 513426 + \frac{1}{3} \cdot 513462 + \frac{2}{5} \cdot 513624 + \frac{7}{20} \cdot 513642 \\
&+ \frac{7}{20} \cdot 514236 + \frac{7}{20} \cdot 514263 + \frac{7}{20} \cdot 514326 + \frac{1}{3} \cdot 514362 + \frac{2}{5} \cdot 514623 + \frac{11}{30} \cdot 514632 \\
&+ \frac{1}{2} \cdot 516234 + \frac{13}{30} \cdot 516243 + \frac{13}{30} \cdot 516324 + \frac{5}{12} \cdot 516342 + \frac{5}{12} \cdot 516423 + \frac{9}{20} \cdot 516432 \\
&+ \frac{2}{5} \cdot 521346 + \frac{5}{12} \cdot 521364 + \frac{11}{30} \cdot 521436 + \frac{2}{5} \cdot 521463 + \frac{29}{60} \cdot 521634 + \frac{29}{60} \cdot 521643 \\
&+ \frac{7}{20} \cdot 523146 + \frac{13}{30} \cdot 523164 + \frac{7}{20} \cdot 523416 + \frac{7}{20} \cdot 523461 + \frac{2}{5} \cdot 523614 + \frac{11}{30} \cdot 523641 \\
&+ \frac{1}{3} \cdot 524136 + \frac{2}{5} \cdot 524163 + \frac{7}{20} \cdot 524316 + \frac{7}{20} \cdot 524361 + \frac{13}{30} \cdot 524613 + \frac{23}{60} \cdot 524631 \\
&+ \frac{29}{60} \cdot 526134 + \frac{29}{60} \cdot 526143 + \frac{13}{30} \cdot 526314 + \frac{13}{30} \cdot 526341 + \frac{9}{20} \cdot 526413 + \frac{7}{15} \cdot 526431 \\
&+ \frac{7}{20} \cdot 531246 + \frac{13}{30} \cdot 531264 + \frac{1}{3} \cdot 531426 + \frac{7}{20} \cdot 531462 + \frac{9}{20} \cdot 531624 + \frac{13}{30} \cdot 531642 \\
&+ \frac{7}{20} \cdot 532146 + \frac{1}{2} \cdot 532164 + \frac{7}{20} \cdot 532416 + \frac{7}{20} \cdot 532461 + \frac{7}{15} \cdot 532614 + \frac{13}{30} \cdot 532641 \\
&+ \frac{11}{30} \cdot 534126 + \frac{5}{12} \cdot 534162 + \frac{2}{5} \cdot 534216 + \frac{2}{5} \cdot 534261 + \frac{31}{60} \cdot 534612 + \frac{9}{20} \cdot 534621 \\
&+ \frac{31}{60} \cdot 536124 + \frac{1}{2} \cdot 536142 + \frac{29}{60} \cdot 536214 + \frac{29}{60} \cdot 536241 + \frac{8}{15} \cdot 536412 + \frac{8}{15} \cdot 536421 \\
&+ \frac{7}{20} \cdot 541236 + \frac{23}{60} \cdot 541263 + \frac{7}{20} \cdot 541326 + \frac{11}{30} \cdot 541362 + \frac{7}{15} \cdot 541623 + \frac{13}{30} \cdot 541632 \\
&+ \frac{7}{20} \cdot 542136 + \frac{9}{20} \cdot 542163 + \frac{2}{5} \cdot 542316 + \frac{2}{5} \cdot 542361 + \frac{29}{60} \cdot 542613 + \frac{7}{15} \cdot 542631 \\
&+ \frac{2}{5} \cdot 543126 + \frac{9}{20} \cdot 543162 + \frac{1}{2} \cdot 543216 + \frac{1}{2} \cdot 543261 + \frac{11}{20} \cdot 543612 + \frac{11}{20} \cdot 543621 \\
&+ \frac{3}{5} \cdot 546123 + \frac{17}{30} \cdot 546132 + \frac{17}{30} \cdot 546213 + \frac{7}{12} \cdot 546231 + \frac{7}{12} \cdot 546312 + \frac{13}{20} \cdot 546321 \\
&+ \frac{3}{5} \cdot 561234 + \frac{8}{15} \cdot 561243 + \frac{8}{15} \cdot 561324 + \frac{31}{60} \cdot 561342 + \frac{31}{60} \cdot 561423 + \frac{11}{20} \cdot 561432 \\
&+ \frac{8}{15} \cdot 562134 + \frac{8}{15} \cdot 562143 + \frac{31}{60} \cdot 562314 + \frac{11}{20} \cdot 562341 + \frac{8}{15} \cdot 562413 + \frac{7}{12} \cdot 562431
\end{aligned}
$$

$$
\begin{aligned}
&+\frac{31}{60}\cdot 563124+\frac{8}{15}\cdot 563142+\frac{11}{20}\cdot 563214+\frac{7}{12}\cdot 563241+\frac{3}{5}\cdot 563412+\frac{2}{3}\cdot 563421\\
&+\frac{11}{20}\cdot 564123+\frac{7}{12}\cdot 564132+\frac{7}{12}\cdot 564213+\frac{2}{3}\cdot 564231+\frac{2}{3}\cdot 564312+\frac{4}{5}\cdot 564321\\
&+\frac{1}{2}\cdot 612345+\frac{2}{5}\cdot 612354+\frac{2}{5}\cdot 612435+\frac{7}{20}\cdot 612453+\frac{7}{20}\cdot 612534+\frac{7}{20}\cdot 612543\\
&+\frac{2}{5}\cdot 613245+\frac{11}{30}\cdot 613254+\frac{7}{20}\cdot 613425+\frac{7}{20}\cdot 613452+\frac{1}{3}\cdot 613524+\frac{7}{20}\cdot 613542\\
&+\frac{7}{20}\cdot 614235+\frac{1}{3}\cdot 614253+\frac{7}{20}\cdot 614325+\frac{7}{20}\cdot 614352+\frac{11}{30}\cdot 614523+\frac{2}{5}\cdot 614532\\
&+\frac{7}{20}\cdot 615234+\frac{7}{20}\cdot 615243+\frac{7}{20}\cdot 615324+\frac{2}{5}\cdot 615342+\frac{2}{5}\cdot 615423+\frac{1}{2}\cdot 615432\\
&+\frac{2}{5}\cdot 621345+\frac{11}{30}\cdot 621354+\frac{11}{30}\cdot 621435+\frac{23}{60}\cdot 621453+\frac{23}{60}\cdot 621534+\frac{9}{20}\cdot 621543\\
&+\frac{7}{20}\cdot 623145+\frac{23}{60}\cdot 623154+\frac{7}{20}\cdot 623415+\frac{2}{5}\cdot 623451+\frac{11}{30}\cdot 623514+\frac{2}{5}\cdot 623541\\
&+\frac{1}{3}\cdot 624135+\frac{23}{60}\cdot 624153+\frac{7}{20}\cdot 624315+\frac{2}{5}\cdot 624351+\frac{13}{30}\cdot 624513+\frac{9}{20}\cdot 624531\\
&+\frac{11}{30}\cdot 625134+\frac{13}{30}\cdot 625143+\frac{23}{60}\cdot 625314+\frac{9}{20}\cdot 625341+\frac{7}{15}\cdot 625413+\frac{11}{20}\cdot 625431\\
&+\frac{7}{20}\cdot 631245+\frac{23}{60}\cdot 631254+\frac{1}{3}\cdot 631425+\frac{11}{30}\cdot 631452+\frac{23}{60}\cdot 631524+\frac{13}{30}\cdot 631542\\
&+\frac{7}{20}\cdot 632145+\frac{9}{20}\cdot 632154+\frac{7}{20}\cdot 632415+\frac{2}{5}\cdot 632451+\frac{13}{30}\cdot 632514+\frac{7}{15}\cdot 632541\\
&+\frac{11}{30}\cdot 634125+\frac{13}{30}\cdot 634152+\frac{2}{5}\cdot 634215+\frac{9}{20}\cdot 634251+\frac{11}{20}\cdot 634512+\frac{11}{20}\cdot 634521\\
&+\frac{13}{30}\cdot 635124+\frac{29}{60}\cdot 635142+\frac{7}{15}\cdot 635214+\frac{8}{15}\cdot 635241+\frac{7}{12}\cdot 635412+\frac{13}{20}\cdot 635421\\
&+\frac{7}{20}\cdot 641235+\frac{11}{30}\cdot 641253+\frac{7}{20}\cdot 641325+\frac{23}{60}\cdot 641352+\frac{13}{30}\cdot 641523+\frac{7}{15}\cdot 641532\\
&+\frac{7}{20}\cdot 642135+\frac{13}{30}\cdot 642153+\frac{2}{5}\cdot 642315+\frac{9}{20}\cdot 642351+\frac{29}{60}\cdot 642513+\frac{8}{15}\cdot 642531\\
&+\frac{2}{5}\cdot 643125+\frac{7}{15}\cdot 643152+\frac{1}{2}\cdot 643215+\frac{11}{20}\cdot 643251+\frac{7}{12}\cdot 643512+\frac{13}{20}\cdot 643521\\
&+\frac{11}{20}\cdot 645123+\frac{7}{12}\cdot 645132+\frac{7}{12}\cdot 645213+\frac{2}{3}\cdot 645231+\frac{2}{3}\cdot 645312+\frac{4}{5}\cdot 645321\\
&+\frac{2}{5}\cdot 651234+\frac{2}{5}\cdot 651243+\frac{2}{5}\cdot 651324+\frac{9}{20}\cdot 651342+\frac{9}{20}\cdot 651423+\frac{11}{20}\cdot 651432\\
&+\frac{2}{5}\cdot 652134+\frac{7}{15}\cdot 652143+\frac{9}{20}\cdot 652314+\frac{11}{20}\cdot 652341+\frac{8}{15}\cdot 652413+\frac{13}{20}\cdot 652431\\
&+\frac{9}{20}\cdot 653124+\frac{8}{15}\cdot 653142+\frac{11}{20}\cdot 653214+\frac{13}{20}\cdot 653241+\frac{2}{3}\cdot 653412+\frac{4}{5}\cdot 653421\\
&+\frac{11}{20}\cdot 654123+\frac{13}{20}\cdot 654132+\frac{13}{20}\cdot 654213+\frac{4}{5}\cdot 654231+\frac{4}{5}\cdot 654312+654321
\end{aligned}
$$

$$
\begin{aligned}
[\![x_1\times x_1]\!] &= \frac{7}{15}\cdot 123456+\frac{2}{45}\cdot 123465+\frac{2}{45}\cdot 123546-\frac{1}{15}\cdot 123564-\frac{1}{15}\cdot 123645+\frac{2}{45}\cdot 124356\\
&+\frac{1}{45}\cdot 124365-\frac{1}{15}\cdot 124536+\frac{4}{45}\cdot 124635-\frac{1}{15}\cdot 125346+\frac{4}{45}\cdot 125364+\frac{13}{45}\cdot 125634\\
&-\frac{2}{9}\cdot 123654-\frac{1}{9}\cdot 124563-\frac{2}{45}\cdot 124653-\frac{2}{9}\cdot 125436-\frac{2}{45}\cdot 125463-\frac{1}{9}\cdot 126345
\end{aligned}
$$

$$- \frac{2}{45} \cdot 126354 - \frac{2}{45} \cdot 126435 + \frac{2}{45} \cdot 126453 + \frac{2}{45} \cdot 132456 - \frac{1}{15} \cdot 134256 + \frac{4}{45} \cdot 135246$$
$$+ \frac{2}{45} \cdot 136245 + \frac{13}{45} \cdot 145236 + \frac{1}{45} \cdot 146235 - \frac{1}{15} \cdot 156234 - \frac{1}{9} \cdot 134526 + \frac{1}{9} \cdot 134562$$
$$- \frac{1}{15} \cdot 142356 + \frac{4}{45} \cdot 142536 + \frac{2}{45} \cdot 142563 + \frac{1}{45} \cdot 145263 - \frac{1}{15} \cdot 145623 - \frac{1}{9} \cdot 152346$$
$$+ \frac{1}{9} \cdot 162345 - \frac{2}{9} \cdot 143256 - \frac{2}{45} \cdot 143526 + \frac{1}{15} \cdot 143562 - \frac{4}{45} \cdot 145362 - \frac{11}{45} \cdot 145632$$
$$- \frac{2}{45} \cdot 153246 + \frac{1}{15} \cdot 163245 - \frac{4}{45} \cdot 164235 - \frac{11}{45} \cdot 165234 + \frac{2}{45} \cdot 213456 + \frac{1}{45} \cdot 214356$$
$$- \frac{1}{15} \cdot 215346 - \frac{11}{45} \cdot 216345 - \frac{1}{15} \cdot 214536 - \frac{11}{45} \cdot 214563 - \frac{1}{15} \cdot 231456 - \frac{1}{15} \cdot 231465$$
$$- \frac{1}{15} \cdot 231546 + \frac{1}{15} \cdot 231564 + \frac{1}{15} \cdot 231645 - \frac{1}{9} \cdot 234156 - \frac{11}{45} \cdot 234165 + \frac{1}{9} \cdot 234516$$
$$+ \frac{2}{45} \cdot 235146 - \frac{2}{45} \cdot 235164 - \frac{1}{15} \cdot 235614 + \frac{14}{45} \cdot 234561 + \frac{2}{45} \cdot 234651 + \frac{1}{15} \cdot 235416$$
$$- \frac{1}{15} \cdot 235641 + \frac{2}{9} \cdot 236145 + \frac{1}{15} \cdot 236415 - \frac{1}{15} \cdot 236451 + \frac{4}{45} \cdot 241356 + \frac{2}{45} \cdot 251346$$
$$- \frac{1}{15} \cdot 312456 - \frac{1}{15} \cdot 312465 - \frac{1}{15} \cdot 312546 + \frac{1}{15} \cdot 312564 + \frac{1}{15} \cdot 312645 - \frac{1}{9} \cdot 412356$$
$$- \frac{11}{45} \cdot 412365 + \frac{2}{45} \cdot 412536 - \frac{2}{45} \cdot 412635 + \frac{1}{9} \cdot 512346 - \frac{1}{15} \cdot 512634 + \frac{4}{45} \cdot 314256$$
$$+ \frac{2}{45} \cdot 314526 - \frac{2}{9} \cdot 321456 + \frac{13}{45} \cdot 341256 + \frac{1}{45} \cdot 341526 - \frac{1}{15} \cdot 341562 - \frac{1}{15} \cdot 345126$$
$$+ \frac{1}{9} \cdot 345162 + \frac{13}{45} \cdot 345612 + \frac{1}{45} \cdot 351246 - \frac{1}{15} \cdot 361245 - \frac{1}{15} \cdot 451236 + \frac{1}{9} \cdot 461235$$
$$+ \frac{13}{45} \cdot 561234 - \frac{4}{45} \cdot 342516 - \frac{1}{15} \cdot 342561 - \frac{11}{45} \cdot 345216 - \frac{2}{45} \cdot 345261 + \frac{2}{45} \cdot 345621$$
$$+ \frac{2}{9} \cdot 412563 + \frac{1}{15} \cdot 512436 + \frac{1}{15} \cdot 512463 + \frac{14}{45} \cdot 612345 + \frac{2}{45} \cdot 612354 - \frac{1}{15} \cdot 612453$$
$$- \frac{1}{15} \cdot 612534 + \frac{2}{45} \cdot 423156 - \frac{1}{15} \cdot 423516 - \frac{1}{15} \cdot 423561 - \frac{1}{15} \cdot 523146 - \frac{4}{15} \cdot 523416$$
$$- \frac{2}{45} \cdot 523461 - \frac{1}{15} \cdot 623145 - \frac{2}{45} \cdot 623415 + \frac{2}{45} \cdot 623451 - \frac{4}{45} \cdot 531246 - \frac{11}{45} \cdot 541236$$
$$- \frac{1}{15} \cdot 631245 - \frac{2}{45} \cdot 641235 + \frac{2}{45} \cdot 651234 + \frac{1}{45} \cdot 132546 - \frac{2}{45} \cdot 135426 - \frac{2}{45} \cdot 152436$$
$$+ \frac{2}{45} \cdot 153426 + \frac{2}{45} \cdot 152364 + \frac{1}{45} \cdot 152634 + \frac{2}{45} \cdot 134625 + \frac{1}{45} \cdot 135624 + \frac{1}{15} \cdot 134652$$
$$- \frac{4}{45} \cdot 135642 + \frac{1}{15} \cdot 162354 - \frac{4}{45} \cdot 162534 + \frac{1}{45} \cdot 213465 - \frac{1}{15} \cdot 213645 - \frac{1}{15} \cdot 213564$$
$$+ \frac{1}{15} \cdot 263145 + \frac{2}{45} \cdot 263415 + \frac{1}{15} \cdot 413562 + \frac{2}{45} \cdot 513462 - \frac{2}{45} \cdot 324156 + \frac{1}{15} \cdot 324516$$
$$- \frac{2}{45} \cdot 421356 + \frac{1}{15} \cdot 521346 - \frac{1}{15} \cdot 132645 - \frac{1}{15} \cdot 132564 - \frac{1}{15} \cdot 134265 + \frac{2}{45} \cdot 324561$$
$$- \frac{1}{15} \cdot 142365 - \frac{2}{45} \cdot 243156 - \frac{2}{45} \cdot 413256 + \frac{1}{45} \cdot 245136 + \frac{1}{9} \cdot 245163 + \frac{1}{9} \cdot 245613$$
$$+ \frac{1}{45} \cdot 415236 + \frac{1}{9} \cdot 416235 + \frac{1}{9} \cdot 516234 - \frac{4}{45} \cdot 245316 - \frac{1}{45} \cdot 245361 - \frac{2}{45} \cdot 245631$$
$$+ \frac{2}{45} \cdot 621345 - \frac{1}{15} \cdot 153462 - \frac{1}{15} \cdot 163425 - \frac{4}{15} \cdot 163452 - \frac{1}{15} \cdot 253416 - \frac{1}{45} \cdot 253461$$
$$- \frac{2}{45} \cdot 263451 - \frac{1}{15} \cdot 513426 - \frac{1}{45} \cdot 613425 - \frac{2}{45} \cdot 613452 - \frac{4}{45} \cdot 514236 - \frac{1}{45} \cdot 614235$$

$$-\frac{2}{45}\cdot 615234-\frac{2}{45}\cdot 241563-\frac{2}{45}\cdot 316245-\frac{1}{15}\cdot 136452-\frac{1}{15}\cdot 162453+\frac{1}{15}\cdot 126543$$
$$+\frac{1}{45}\cdot 132465-\frac{2}{45}\cdot 135264+\frac{2}{45}\cdot 136254-\frac{4}{45}\cdot 146253-\frac{2}{45}\cdot 156243-\frac{2}{45}\cdot 142635$$
$$+\frac{2}{45}\cdot 142653-\frac{2}{45}\cdot 146523+\frac{2}{45}\cdot 143265+\frac{2}{45}\cdot 143625+\frac{7}{45}\cdot 143652+\frac{2}{45}\cdot 146325$$
$$+\frac{1}{45}\cdot 146352+\frac{2}{45}\cdot 153264+\frac{2}{45}\cdot 154263+\frac{7}{45}\cdot 163254+\frac{1}{45}\cdot 164253+\frac{2}{15}\cdot 214365$$
$$+\frac{1}{45}\cdot 215364+\frac{1}{45}\cdot 214635+\frac{1}{15}\cdot 231654-\frac{1}{15}\cdot 236514-\frac{1}{9}\cdot 236541+\frac{1}{45}\cdot 241365$$
$$-\frac{4}{45}\cdot 251364-\frac{1}{45}\cdot 261354+\frac{1}{15}\cdot 312654-\frac{1}{15}\cdot 512643+\frac{1}{45}\cdot 314265-\frac{4}{45}\cdot 314625$$
$$-\frac{1}{45}\cdot 314652+\frac{2}{45}\cdot 321465+\frac{2}{45}\cdot 341265-\frac{1}{15}\cdot 341625-\frac{8}{45}\cdot 341652-\frac{1}{15}\cdot 346125$$
$$+\frac{2}{45}\cdot 346512-\frac{1}{15}\cdot 351264-\frac{8}{45}\cdot 361254-\frac{1}{15}\cdot 451263+\frac{2}{45}\cdot 561243+\frac{1}{15}\cdot 342165$$
$$+\frac{2}{45}\cdot 342615-\frac{2}{45}\cdot 342651-\frac{1}{45}\cdot 346215+\frac{1}{45}\cdot 346251+\frac{1}{15}\cdot 346521-\frac{1}{9}\cdot 612543$$
$$+\frac{1}{9}\cdot 423165+\frac{1}{15}\cdot 423615-\frac{2}{45}\cdot 423651+\frac{1}{15}\cdot 523164+\frac{7}{45}\cdot 523614+\frac{1}{45}\cdot 523641$$
$$-\frac{2}{45}\cdot 623154+\frac{1}{45}\cdot 623514+\frac{1}{15}\cdot 623541+\frac{1}{15}\cdot 431265+\frac{2}{45}\cdot 531264-\frac{1}{45}\cdot 541263$$
$$-\frac{2}{45}\cdot 631254+\frac{1}{45}\cdot 641253+\frac{1}{15}\cdot 651243+\frac{1}{15}\cdot 154326-\frac{4}{45}\cdot 153624-\frac{2}{45}\cdot 156324$$
$$+\frac{2}{45}\cdot 135462-\frac{2}{45}\cdot 154623+\frac{2}{45}\cdot 162435+\frac{2}{45}\cdot 132654+\frac{2}{45}\cdot 152643+\frac{1}{45}\cdot 153642$$
$$+\frac{2}{45}\cdot 136524+\frac{1}{45}\cdot 163524+\frac{1}{45}\cdot 213546+\frac{2}{45}\cdot 241635+\frac{2}{45}\cdot 315264+\frac{2}{45}\cdot 243516$$
$$-\frac{2}{45}\cdot 241536+\frac{2}{45}\cdot 251436-\frac{4}{45}\cdot 351426-\frac{2}{45}\cdot 451326-\frac{2}{45}\cdot 243615-\frac{1}{45}\cdot 246135$$
$$-\frac{2}{45}\cdot 246315-\frac{2}{45}\cdot 261435-\frac{2}{45}\cdot 264135+\frac{1}{45}\cdot 264315-\frac{2}{45}\cdot 315246+\frac{2}{45}\cdot 315426$$
$$-\frac{2}{45}\cdot 354126+\frac{2}{45}\cdot 513246-\frac{2}{45}\cdot 315462-\frac{1}{45}\cdot 415263-\frac{2}{45}\cdot 415362-\frac{2}{45}\cdot 513264$$
$$-\frac{2}{45}\cdot 514263+\frac{1}{45}\cdot 514362+\frac{2}{45}\cdot 321546+\frac{2}{45}\cdot 325146+\frac{7}{45}\cdot 325416+\frac{2}{45}\cdot 352146$$
$$+\frac{1}{45}\cdot 352416+\frac{2}{45}\cdot 421536+\frac{2}{45}\cdot 431526+\frac{7}{45}\cdot 521436+\frac{1}{45}\cdot 531426+\frac{1}{45}\cdot 354621$$
$$+\frac{1}{45}\cdot 624351+\frac{1}{45}\cdot 651324+\frac{1}{9}\cdot 156342+\frac{1}{15}\cdot 156423-\frac{2}{45}\cdot 152463+\frac{1}{15}\cdot 156432$$
$$-\frac{1}{45}\cdot 136542-\frac{1}{45}\cdot 154362-\frac{2}{45}\cdot 163542-\frac{2}{45}\cdot 164352+\frac{1}{9}\cdot 164532+\frac{1}{9}\cdot 165342$$
$$+\frac{1}{15}\cdot 215643+\frac{1}{9}\cdot 216453-\frac{1}{15}\cdot 241653-\frac{2}{45}\cdot 246153+\frac{2}{45}\cdot 251463-\frac{1}{15}\cdot 251643$$
$$-\frac{8}{45}\cdot 256143+\frac{2}{45}\cdot 256314+\frac{2}{45}\cdot 246351+\frac{8}{45}\cdot 256341+\frac{1}{45}\cdot 246513+\frac{8}{45}\cdot 254163$$
$$-\frac{1}{15}\cdot 256413+\frac{1}{15}\cdot 261453+\frac{1}{45}\cdot 264153-\frac{2}{45}\cdot 264513-\frac{1}{15}\cdot 315624+\frac{2}{45}\cdot 351624$$
$$+\frac{1}{9}\cdot 356124-\frac{2}{45}\cdot 413526+\frac{2}{45}\cdot 413625+\frac{2}{45}\cdot 315642+\frac{1}{15}\cdot 321564-\frac{1}{15}\cdot 325164$$
$$-\frac{8}{45}\cdot 325614-\frac{1}{15}\cdot 352164-\frac{2}{45}\cdot 352614+\frac{1}{15}\cdot 356214-\frac{1}{15}\cdot 356412+\frac{2}{45}\cdot 351462$$

$$+\frac{7}{45}\cdot 361452+\frac{2}{45}\cdot 451362+\frac{1}{45}\cdot 461352-\frac{1}{15}\cdot 561342-\frac{2}{45}\cdot 356421-\frac{1}{15}\cdot 415623$$
$$+\frac{2}{45}\cdot 513624+\frac{2}{45}\cdot 514623+\frac{2}{45}\cdot 613524+\frac{8}{45}\cdot 614523+\frac{1}{45}\cdot 425631-\frac{2}{45}\cdot 524631$$
$$-\frac{2}{45}\cdot 624531-\frac{1}{15}\cdot 431562-\frac{2}{45}\cdot 531462+\frac{1}{45}\cdot 631452-\frac{2}{45}\cdot 641352-\frac{2}{45}\cdot 651342$$
$$+\frac{2}{45}\cdot 215634-\frac{2}{45}\cdot 136425+\frac{1}{15}\cdot 316452+\frac{1}{45}\cdot 413652-\frac{2}{45}\cdot 325641-\frac{1}{45}\cdot 415632$$
$$-\frac{2}{45}\cdot 513642+\frac{2}{45}\cdot 253164-\frac{1}{15}\cdot 256134-\frac{2}{45}\cdot 516342+\frac{1}{45}\cdot 356241-\frac{2}{45}\cdot 621453$$
$$+\frac{1}{9}\cdot 164523+\frac{1}{45}\cdot 264531+\frac{1}{45}\cdot 624513+\frac{1}{45}\cdot 615342-\frac{1}{45}\cdot 162543-\frac{1}{45}\cdot 164325$$
$$+\frac{1}{15}\cdot 165423+\frac{1}{15}\cdot 216534-\frac{1}{15}\cdot 316254+\frac{2}{45}\cdot 316425-\frac{1}{15}\cdot 316524-\frac{2}{45}\cdot 416253$$
$$-\frac{8}{45}\cdot 416523-\frac{1}{15}\cdot 251634-\frac{2}{45}\cdot 253146+\frac{1}{9}\cdot 451623+\frac{2}{45}\cdot 253614+\frac{2}{45}\cdot 253641$$
$$+\frac{2}{45}\cdot 261534+\frac{8}{45}\cdot 416325+\frac{1}{45}\cdot 416352+\frac{1}{45}\cdot 516243-\frac{1}{15}\cdot 516423+\frac{1}{15}\cdot 321645$$
$$-\frac{1}{15}\cdot 421635-\frac{1}{15}\cdot 431625-\frac{8}{45}\cdot 521634-\frac{2}{45}\cdot 531624+\frac{1}{15}\cdot 541623+\frac{2}{45}\cdot 361425$$
$$+\frac{2}{45}\cdot 364125+\frac{1}{45}\cdot 364152-\frac{1}{15}\cdot 364512-\frac{1}{15}\cdot 561423-\frac{1}{15}\cdot 362145-\frac{2}{45}\cdot 362415$$
$$+\frac{1}{45}\cdot 362451-\frac{2}{45}\cdot 364251-\frac{2}{45}\cdot 364521+\frac{2}{45}\cdot 614253+\frac{1}{45}\cdot 625134-\frac{2}{45}\cdot 625314$$
$$-\frac{2}{45}\cdot 625341-\frac{2}{45}\cdot 651423+\frac{1}{45}\cdot 263154-\frac{2}{45}\cdot 326451-\frac{2}{45}\cdot 263514-\frac{1}{45}\cdot 265134$$
$$-\frac{2}{45}\cdot 621534+\frac{1}{45}\cdot 526341+\frac{1}{45}\cdot 641523+\frac{7}{45}\cdot 165432+\frac{2}{45}\cdot 213654+\frac{8}{45}\cdot 216543$$
$$+\frac{2}{45}\cdot 254136-\frac{1}{45}\cdot 254316-\frac{2}{45}\cdot 351642+\frac{1}{15}\cdot 451632-\frac{4}{45}\cdot 254361-\frac{1}{45}\cdot 254631$$
$$-\frac{1}{45}\cdot 514326-\frac{1}{15}\cdot 516432+\frac{1}{5}\cdot 321654+\frac{4}{45}\cdot 531642+\frac{1}{9}\cdot 541632-\frac{2}{45}\cdot 361524$$
$$-\frac{2}{45}\cdot 361542+\frac{1}{15}\cdot 365124-\frac{2}{45}\cdot 365142-\frac{1}{9}\cdot 365412-\frac{1}{9}\cdot 561432+\frac{4}{45}\cdot 362514$$
$$+\frac{2}{45}\cdot 362541+\frac{1}{9}\cdot 365214+\frac{1}{45}\cdot 365241+\frac{2}{45}\cdot 365421-\frac{4}{45}\cdot 614325-\frac{1}{45}\cdot 614352$$
$$+\frac{2}{45}\cdot 625143+\frac{1}{45}\cdot 625413+\frac{2}{45}\cdot 625431+\frac{2}{45}\cdot 651432-\frac{1}{45}\cdot 264351-\frac{1}{15}\cdot 265413$$
$$+\frac{2}{45}\cdot 415326-\frac{2}{45}\cdot 461532-\frac{1}{45}\cdot 615324+\frac{2}{45}\cdot 426531+\frac{1}{45}\cdot 526431+\frac{2}{45}\cdot 631542$$
$$+\frac{1}{45}\cdot 641532+\frac{1}{15}\cdot 432156-\frac{4}{45}\cdot 425136-\frac{2}{45}\cdot 452136-\frac{1}{9}\cdot 432561-\frac{1}{45}\cdot 324615$$
$$-\frac{2}{45}\cdot 435126-\frac{1}{45}\cdot 521364+\frac{2}{45}\cdot 215436+\frac{1}{45}\cdot 425316+\frac{1}{45}\cdot 524136+\frac{2}{45}\cdot 435612$$
$$+\frac{2}{45}\cdot 562134+\frac{1}{15}\cdot 435621-\frac{1}{9}\cdot 632145+\frac{1}{15}\cdot 632451+\frac{1}{15}\cdot 652134+\frac{1}{45}\cdot 326415$$
$$-\frac{2}{45}\cdot 325461-\frac{2}{45}\cdot 243651-\frac{2}{45}\cdot 426135-\frac{8}{45}\cdot 436125+\frac{1}{45}\cdot 426315+\frac{8}{45}\cdot 432165$$
$$-\frac{1}{45}\cdot 426513+\frac{1}{45}\cdot 436512-\frac{8}{45}\cdot 452163-\frac{1}{45}\cdot 462153+\frac{1}{45}\cdot 562143+\frac{2}{45}\cdot 436521$$
$$-\frac{2}{45}\cdot 621435-\frac{2}{45}\cdot 613254+\frac{2}{45}\cdot 532641+\frac{2}{45}\cdot 632541+\frac{2}{45}\cdot 642153+\frac{2}{45}\cdot 652143$$

$$
\begin{aligned}
&-\frac{2}{45}\cdot 425163+\frac{1}{45}\cdot 521463+\frac{1}{45}\cdot 524163-\frac{1}{45}\cdot 436152-\frac{1}{45}\cdot 526143+\frac{2}{45}\cdot 436251\\
&+\frac{2}{45}\cdot 632514-\frac{1}{45}\cdot 432516+\frac{1}{9}\cdot 452316+\frac{1}{15}\cdot 453126-\frac{1}{15}\cdot 453162-\frac{1}{15}\cdot 453612\\
&-\frac{2}{45}\cdot 462315-\frac{1}{15}\cdot 562314+\frac{8}{45}\cdot 452361+\frac{1}{45}\cdot 452631+\frac{1}{15}\cdot 453216-\frac{2}{45}\cdot 453621\\
&+\frac{1}{9}\cdot 534126-\frac{2}{45}\cdot 534162+\frac{1}{9}\cdot 534216+\frac{1}{45}\cdot 534261+\frac{8}{45}\cdot 634125+\frac{1}{45}\cdot 634152\\
&-\frac{2}{45}\cdot 634251+\frac{1}{9}\cdot 542316+\frac{1}{45}\cdot 642315-\frac{2}{45}\cdot 652314+\frac{2}{45}\cdot 425361+\frac{1}{45}\cdot 435162\\
&-\frac{2}{45}\cdot 524316-\frac{2}{45}\cdot 532416+\frac{1}{45}\cdot 526314+\frac{2}{45}\cdot 631425+\frac{2}{45}\cdot 352461+\frac{4}{15}\cdot 456123\\
&+\frac{2}{45}\cdot 456132+\frac{2}{45}\cdot 456213-\frac{1}{9}\cdot 456231-\frac{1}{9}\cdot 456312+\frac{1}{45}\cdot 462351-\frac{1}{9}\cdot 562341\\
&-\frac{2}{15}\cdot 456321-\frac{1}{15}\cdot 534612-\frac{2}{45}\cdot 534621-\frac{1}{9}\cdot 634512-\frac{2}{15}\cdot 634521-\frac{2}{45}\cdot 642351\\
&-\frac{2}{15}\cdot 652341-\frac{1}{45}\cdot 354261-\frac{1}{45}\cdot 524361+\frac{1}{45}\cdot 462135-\frac{1}{15}\cdot 463125+\frac{1}{45}\cdot 426153\\
&-\frac{1}{15}\cdot 463215+\frac{1}{45}\cdot 462513+\frac{2}{45}\cdot 463512+\frac{2}{45}\cdot 562413-\frac{2}{45}\cdot 462531-\frac{1}{45}\cdot 463521\\
&+\frac{2}{45}\cdot 624135+\frac{1}{45}\cdot 536142-\frac{2}{45}\cdot 536241-\frac{2}{45}\cdot 635142-\frac{1}{45}\cdot 635241-\frac{2}{45}\cdot 542613\\
&-\frac{2}{45}\cdot 642513-\frac{1}{45}\cdot 652413-\frac{1}{45}\cdot 532146+\frac{1}{15}\cdot 543126+\frac{1}{45}\cdot 524613-\frac{1}{15}\cdot 563124\\
&-\frac{2}{45}\cdot 653124+\frac{1}{45}\cdot 635124-\frac{1}{15}\cdot 543162+\frac{2}{45}\cdot 536412+\frac{2}{45}\cdot 563142-\frac{2}{45}\cdot 536214\\
&-\frac{1}{45}\cdot 536421-\frac{1}{45}\cdot 642531-\frac{1}{45}\cdot 653142+\frac{7}{45}\cdot 543216-\frac{2}{45}\cdot 532614-\frac{1}{9}\cdot 543612\\
&-\frac{1}{9}\cdot 563214+\frac{1}{45}\cdot 542631+\frac{2}{45}\cdot 543621-\frac{1}{45}\cdot 624315+\frac{1}{45}\cdot 643152+\frac{2}{45}\cdot 643251\\
&+\frac{2}{45}\cdot 653214-\frac{1}{45}\cdot 641325+\frac{1}{45}\cdot 463251+\frac{1}{45}\cdot 635214+\frac{1}{5}\cdot 563412-\frac{1}{45}\cdot 562431\\
&-\frac{1}{45}\cdot 563241+\frac{2}{45}\cdot 563421-\frac{1}{9}\cdot 564123-\frac{1}{45}\cdot 564132-\frac{1}{45}\cdot 564213+\frac{2}{45}\cdot 564231\\
&+\frac{2}{45}\cdot 564312-\frac{1}{9}\cdot 645123-\frac{1}{45}\cdot 645132-\frac{1}{45}\cdot 645213+\frac{2}{45}\cdot 645231+\frac{2}{45}\cdot 645312\\
&+\frac{2}{45}\cdot 653412+\frac{2}{45}\cdot 465123+\frac{2}{45}\cdot 546123-\frac{1}{45}\cdot 465231-\frac{1}{45}\cdot 546231-\frac{1}{45}\cdot 465312\\
&-\frac{1}{45}\cdot 546312-\frac{1}{45}\cdot 635412-\frac{1}{45}\cdot 643512+\frac{1}{15}\cdot 564321+\frac{1}{15}\cdot 645321+\frac{1}{15}\cdot 653421\\
&-\frac{2}{15}\cdot 654123+\frac{1}{15}\cdot 654231+\frac{1}{15}\cdot 654312
\end{aligned}
$$

$$
\begin{aligned}
\llbracket x_1\times x_2\rrbracket =&\ \frac{1}{5}\cdot 123456+\frac{1}{45}\cdot 123465+\frac{1}{45}\cdot 123546-\frac{7}{90}\cdot 143256-\frac{1}{45}\cdot 143526-\frac{1}{90}\cdot 143562\\
&-\frac{1}{45}\cdot 153246-\frac{1}{45}\cdot 153426-\frac{1}{90}\cdot 153462-\frac{1}{90}\cdot 163245-\frac{1}{90}\cdot 163425-\frac{1}{18}\cdot 163452\\
&-\frac{1}{45}\cdot 214356-\frac{1}{45}\cdot 214536-\frac{1}{10}\cdot 214563-\frac{1}{45}\cdot 215346-\frac{1}{10}\cdot 216345-\frac{1}{90}\cdot 234156\\
&+\frac{1}{45}\cdot 234516+\frac{2}{15}\cdot 234561-\frac{7}{90}\cdot 321456-\frac{1}{90}\cdot 412356+\frac{1}{45}\cdot 512346+\frac{2}{15}\cdot 612345
\end{aligned}
$$

$$+\frac{1}{45}\cdot 124356+\frac{1}{45}\cdot 132456-\frac{7}{90}\cdot 123654-\frac{1}{45}\cdot 124653-\frac{1}{45}\cdot 126354-\frac{1}{45}\cdot 126453$$
$$-\frac{1}{90}\cdot 134652-\frac{1}{90}\cdot 136452-\frac{1}{90}\cdot 162354-\frac{1}{90}\cdot 162453-\frac{1}{45}\cdot 213465-\frac{1}{45}\cdot 213564$$
$$-\frac{1}{45}\cdot 231465-\frac{1}{45}\cdot 231564-\frac{1}{10}\cdot 234165-\frac{1}{90}\cdot 235164-\frac{1}{90}\cdot 241563-\frac{1}{45}\cdot 245163$$
$$-\frac{1}{45}\cdot 213645-\frac{1}{45}\cdot 312465-\frac{1}{45}\cdot 312645-\frac{1}{90}\cdot 316245-\frac{1}{10}\cdot 412365-\frac{1}{90}\cdot 412635$$
$$-\frac{1}{45}\cdot 416235+\frac{1}{90}\cdot 235461+\frac{1}{90}\cdot 243561-\frac{1}{90}\cdot 245361-\frac{1}{90}\cdot 253461-\frac{1}{45}\cdot 324156$$
$$-\frac{1}{90}\cdot 324516-\frac{1}{45}\cdot 421356-\frac{1}{45}\cdot 423156-\frac{1}{90}\cdot 423516-\frac{1}{90}\cdot 521346-\frac{1}{90}\cdot 523146$$
$$-\frac{1}{18}\cdot 523416+\frac{1}{90}\cdot 612435+\frac{1}{90}\cdot 613245-\frac{1}{90}\cdot 613425-\frac{1}{90}\cdot 614235+\frac{1}{45}\cdot 213456$$
$$-\frac{7}{90}\cdot 125436-\frac{1}{45}\cdot 125463-\frac{1}{45}\cdot 126435-\frac{1}{45}\cdot 132546-\frac{1}{45}\cdot 132564-\frac{1}{45}\cdot 231546$$
$$-\frac{1}{45}\cdot 132645-\frac{1}{45}\cdot 312546-\frac{1}{90}\cdot 134526+\frac{1}{45}\cdot 134562-\frac{1}{45}\cdot 243156-\frac{1}{45}\cdot 413256$$
$$-\frac{1}{90}\cdot 152346+\frac{1}{45}\cdot 162345-\frac{1}{45}\cdot 124365-\frac{1}{45}\cdot 134265-\frac{1}{45}\cdot 142365-\frac{1}{90}\cdot 124563$$
$$-\frac{1}{45}\cdot 135426-\frac{1}{45}\cdot 152436-\frac{1}{90}\cdot 235416-\frac{1}{90}\cdot 253416-\frac{1}{90}\cdot 512436-\frac{1}{90}\cdot 513426$$
$$-\frac{1}{90}\cdot 126345+\frac{1}{90}\cdot 143265+\frac{1}{45}\cdot 143625+\frac{2}{45}\cdot 143652+\frac{1}{45}\cdot 153264+\frac{1}{90}\cdot 153624$$
$$+\frac{1}{90}\cdot 153642+\frac{2}{45}\cdot 163254+\frac{1}{90}\cdot 163524+\frac{1}{90}\cdot 163542+\frac{1}{15}\cdot 214365+\frac{1}{45}\cdot 214635$$
$$+\frac{1}{45}\cdot 215364+\frac{1}{90}\cdot 234651+\frac{1}{90}\cdot 321465+\frac{1}{90}\cdot 612354+\frac{1}{90}\cdot 132654+\frac{1}{45}\cdot 136254$$
$$+\frac{1}{45}\cdot 142653+\frac{1}{90}\cdot 146253+\frac{1}{90}\cdot 146352+\frac{1}{90}\cdot 164253+\frac{1}{90}\cdot 164352+\frac{1}{45}\cdot 241365$$
$$+\frac{1}{90}\cdot 251364+\frac{1}{90}\cdot 251463+\frac{1}{90}\cdot 253164+\frac{2}{45}\cdot 254163+\frac{1}{45}\cdot 314265+\frac{1}{90}\cdot 314625$$
$$+\frac{1}{90}\cdot 316425+\frac{1}{90}\cdot 413625+\frac{2}{45}\cdot 416325-\frac{1}{18}\cdot 254361+\frac{1}{90}\cdot 321546+\frac{1}{45}\cdot 325146$$
$$+\frac{2}{45}\cdot 325416+\frac{1}{45}\cdot 421536+\frac{1}{90}\cdot 425136+\frac{1}{90}\cdot 425316+\frac{2}{45}\cdot 521436+\frac{1}{90}\cdot 524136$$
$$+\frac{1}{90}\cdot 524316-\frac{1}{18}\cdot 614325+\frac{1}{45}\cdot 124635+\frac{2}{45}\cdot 125634+\frac{1}{45}\cdot 142536+\frac{1}{45}\cdot 142635$$
$$+\frac{2}{45}\cdot 145236+\frac{1}{90}\cdot 146235+\frac{1}{90}\cdot 152634+\frac{1}{45}\cdot 125364-\frac{7}{90}\cdot 145632-\frac{1}{90}\cdot 146532$$
$$-\frac{1}{90}\cdot 154632+\frac{1}{90}\cdot 156432+\frac{1}{90}\cdot 164532+\frac{1}{45}\cdot 215643-\frac{1}{90}\cdot 251643-\frac{1}{18}\cdot 256143$$
$$+\frac{1}{45}\cdot 216453+\frac{1}{90}\cdot 235641+\frac{1}{90}\cdot 253641+\frac{1}{45}\cdot 256341+\frac{1}{90}\cdot 321564-\frac{1}{18}\cdot 325614$$
$$+\frac{2}{45}\cdot 412563+\frac{1}{45}\cdot 415263+\frac{1}{90}\cdot 415623+\frac{1}{45}\cdot 512463+\frac{1}{45}\cdot 514263+\frac{1}{90}\cdot 514623$$
$$+\frac{1}{90}\cdot 612453+\frac{1}{90}\cdot 614253+\frac{1}{45}\cdot 614523+\frac{1}{90}\cdot 136524+\frac{1}{90}\cdot 136542+\frac{1}{45}\cdot 241635$$
$$+\frac{1}{90}\cdot 413652+\frac{1}{90}\cdot 245613-\frac{1}{90}\cdot 245631+\frac{1}{90}\cdot 154263+\frac{1}{90}\cdot 154362+\frac{1}{45}\cdot 514362$$
$$+\frac{1}{45}\cdot 524163-\frac{1}{90}\cdot 613452+\frac{1}{45}\cdot 135246+\frac{1}{45}\cdot 135264+\frac{1}{90}\cdot 135624+\frac{1}{90}\cdot 145263$$

$$- \frac{7}{90} \cdot 165234 - \frac{1}{90} \cdot 165243 - \frac{1}{90} \cdot 165324 + \frac{1}{90} \cdot 165342 + \frac{1}{90} \cdot 165423 + \frac{1}{45} \cdot 216534$$
$$- \frac{1}{90} \cdot 316524 - \frac{1}{18} \cdot 416523 + \frac{2}{45} \cdot 236145 + \frac{1}{45} \cdot 236415 + \frac{1}{90} \cdot 236451 + \frac{1}{45} \cdot 246135$$
$$+ \frac{1}{45} \cdot 246315 + \frac{1}{90} \cdot 246351 + \frac{1}{90} \cdot 256134 + \frac{1}{90} \cdot 256314 + \frac{1}{90} \cdot 321645 - \frac{1}{18} \cdot 521634$$
$$+ \frac{1}{90} \cdot 612534 + \frac{1}{90} \cdot 613524 + \frac{1}{90} \cdot 152643 + \frac{1}{90} \cdot 162543 + \frac{1}{90} \cdot 263154 + \frac{1}{45} \cdot 315264$$
$$- \frac{1}{90} \cdot 263451 + \frac{1}{90} \cdot 146325 + \frac{1}{90} \cdot 164325 + \frac{1}{45} \cdot 264315 + \frac{1}{45} \cdot 426315 + \frac{1}{90} \cdot 516234$$
$$- \frac{1}{90} \cdot 615234 - \frac{1}{45} \cdot 125643 - \frac{1}{90} \cdot 135462 - \frac{1}{90} \cdot 135642 - \frac{1}{45} \cdot 145326 - \frac{1}{90} \cdot 145362$$
$$+ \frac{1}{15} \cdot 165432 + \frac{2}{15} \cdot 216543 + \frac{1}{90} \cdot 316542 - \frac{1}{90} \cdot 236154 - \frac{1}{45} \cdot 236514 - \frac{1}{30} \cdot 236541$$
$$- \frac{1}{45} \cdot 246153 - \frac{1}{90} \cdot 246513 - \frac{1}{90} \cdot 246531 - \frac{1}{90} \cdot 256413 - \frac{1}{90} \cdot 256431 + \frac{2}{15} \cdot 321654$$
$$+ \frac{1}{45} \cdot 421653 - \frac{1}{90} \cdot 521643 - \frac{1}{30} \cdot 612543 - \frac{1}{90} \cdot 613542 - \frac{1}{90} \cdot 614532 - \frac{1}{45} \cdot 126534$$
$$- \frac{1}{45} \cdot 154236 - \frac{1}{90} \cdot 162435 - \frac{1}{90} \cdot 162534 - \frac{1}{90} \cdot 164235 + \frac{1}{90} \cdot 261543 - \frac{1}{90} \cdot 263541$$
$$- \frac{1}{90} \cdot 265341 + \frac{1}{45} \cdot 326154 - \frac{1}{90} \cdot 326514 - \frac{1}{90} \cdot 412653 - \frac{1}{45} \cdot 416253 - \frac{1}{45} \cdot 512643$$
$$- \frac{1}{90} \cdot 516243 - \frac{1}{90} \cdot 516423 - \frac{1}{90} \cdot 615243 - \frac{1}{90} \cdot 615423 + \frac{1}{90} \cdot 213654 + \frac{1}{90} \cdot 324561$$
$$+ \frac{1}{90} \cdot 215436 + \frac{1}{45} \cdot 251436 + \frac{1}{45} \cdot 315426 + \frac{1}{90} \cdot 351426 + \frac{1}{90} \cdot 352416 + \frac{1}{90} \cdot 531426$$
$$+ \frac{1}{90} \cdot 532416 + \frac{1}{90} \cdot 621345 - \frac{1}{45} \cdot 213546 - \frac{1}{45} \cdot 231645 - \frac{1}{45} \cdot 132465 + \frac{1}{90} \cdot 312654$$
$$- \frac{1}{90} \cdot 314652 - \frac{1}{90} \cdot 316452 - \frac{1}{45} \cdot 324651 - \frac{1}{45} \cdot 326451 - \frac{1}{18} \cdot 341652 - \frac{1}{45} \cdot 342651$$
$$+ \frac{1}{45} \cdot 431265 - \frac{1}{90} \cdot 431625 + \frac{2}{15} \cdot 432165 + \frac{1}{90} \cdot 432615 - \frac{1}{90} \cdot 521364 - \frac{1}{90} \cdot 523164$$
$$- \frac{1}{45} \cdot 621354 - \frac{1}{45} \cdot 621534 - \frac{1}{45} \cdot 623154 - \frac{1}{45} \cdot 312564 + \frac{1}{90} \cdot 231654 - \frac{1}{90} \cdot 324615$$
$$- \frac{1}{45} \cdot 325641 - \frac{1}{90} \cdot 423615 - \frac{1}{45} \cdot 423651 + \frac{1}{45} \cdot 342165 - \frac{1}{90} \cdot 352164 + \frac{1}{90} \cdot 532164$$
$$- \frac{1}{90} \cdot 261354 - \frac{1}{90} \cdot 261453 - \frac{1}{18} \cdot 361254 - \frac{1}{45} \cdot 621453 - \frac{1}{45} \cdot 631254 + \frac{1}{90} \cdot 254136$$
$$+ \frac{1}{90} \cdot 254316 + \frac{1}{45} \cdot 264135 + \frac{1}{45} \cdot 264153 + \frac{1}{45} \cdot 315246 + \frac{1}{90} \cdot 326415 + \frac{1}{90} \cdot 345162$$
$$- \frac{7}{90} \cdot 345216 - \frac{1}{90} \cdot 345261 + \frac{1}{90} \cdot 431526 + \frac{1}{90} \cdot 432516 - \frac{1}{90} \cdot 623415 + \frac{1}{45} \cdot 241356$$
$$+ \frac{2}{45} \cdot 341256 + \frac{1}{45} \cdot 314256 + \frac{1}{90} \cdot 351246 + \frac{1}{90} \cdot 415236 - \frac{1}{18} \cdot 452163 + \frac{1}{45} \cdot 423165$$
$$+ \frac{1}{90} \cdot 342561 + \frac{1}{90} \cdot 352461 + \frac{1}{45} \cdot 452361 - \frac{1}{90} \cdot 354216 - \frac{1}{90} \cdot 435216 + \frac{1}{90} \cdot 453216$$
$$+ \frac{1}{90} \cdot 534216 + \frac{1}{45} \cdot 263145 + \frac{1}{90} \cdot 346125 + \frac{1}{90} \cdot 364125 + \frac{1}{90} \cdot 623145 + \frac{1}{90} \cdot 624135$$
$$+ \frac{1}{45} \cdot 634125 - \frac{1}{90} \cdot 254613 - \frac{1}{90} \cdot 254631 - \frac{1}{90} \cdot 264351 - \frac{1}{90} \cdot 264513 - \frac{1}{90} \cdot 264531$$
$$- \frac{1}{90} \cdot 315462 - \frac{1}{90} \cdot 315624 - \frac{1}{90} \cdot 315642 - \frac{1}{45} \cdot 325461 + \frac{1}{15} \cdot 345612 + \frac{1}{45} \cdot 345621$$

$$- \frac{1}{45} \cdot 431562 - \frac{1}{30} \cdot 432561 - \frac{1}{90} \cdot 523461 + \frac{1}{45} \cdot 623451 - \frac{1}{90} \cdot 243615 - \frac{1}{45} \cdot 243651$$
$$- \frac{1}{90} \cdot 341625 - \frac{1}{90} \cdot 342615 - \frac{1}{90} \cdot 354162 - \frac{1}{90} \cdot 354261 - \frac{1}{90} \cdot 524361 - \frac{1}{90} \cdot 534162$$
$$- \frac{1}{90} \cdot 534261 + \frac{1}{90} \cdot 235146 + \frac{1}{90} \cdot 251346 + \frac{1}{90} \cdot 253146 + \frac{1}{90} \cdot 134625 + \frac{1}{90} \cdot 136245$$
$$+ \frac{1}{90} \cdot 136425 - \frac{1}{90} \cdot 362154 + \frac{1}{90} \cdot 346152 + \frac{1}{90} \cdot 346251 + \frac{1}{45} \cdot 361452 + \frac{1}{90} \cdot 362451$$
$$+ \frac{1}{90} \cdot 364152 + \frac{1}{90} \cdot 364251 - \frac{1}{18} \cdot 436125 + \frac{1}{45} \cdot 523614 + \frac{1}{90} \cdot 526134 + \frac{1}{90} \cdot 526314$$
$$+ \frac{1}{90} \cdot 623514 + \frac{1}{90} \cdot 625134 + \frac{1}{90} \cdot 625314 + \frac{1}{45} \cdot 241536 + \frac{1}{90} \cdot 245136 + \frac{1}{90} \cdot 341526$$
$$+ \frac{1}{45} \cdot 413562 + \frac{1}{45} \cdot 415362 + \frac{1}{90} \cdot 423561 + \frac{1}{90} \cdot 425361 + \frac{1}{90} \cdot 451263 + \frac{1}{90} \cdot 451362$$
$$- \frac{7}{90} \cdot 541236 - \frac{1}{90} \cdot 541326 - \frac{1}{90} \cdot 542136 + \frac{1}{90} \cdot 542316 + \frac{1}{90} \cdot 543126 + \frac{1}{90} \cdot 631245$$
$$+ \frac{1}{90} \cdot 631425 + \frac{1}{90} \cdot 415326 + \frac{1}{45} \cdot 416352 + \frac{1}{90} \cdot 514326 + \frac{1}{90} \cdot 521463 + \frac{1}{90} \cdot 352146$$
$$+ \frac{1}{90} \cdot 532146 + \frac{1}{90} \cdot 461235 - \frac{1}{90} \cdot 641235 + \frac{1}{90} \cdot 314526 + \frac{1}{90} \cdot 412536 + \frac{1}{90} \cdot 413526$$
$$+ \frac{1}{90} \cdot 142563 + \frac{1}{90} \cdot 152364 + \frac{1}{90} \cdot 152463 - \frac{1}{90} \cdot 431652 + \frac{1}{90} \cdot 425613 + \frac{1}{90} \cdot 425631$$
$$+ \frac{1}{90} \cdot 523641 + \frac{1}{90} \cdot 524613 + \frac{1}{90} \cdot 524631 + \frac{1}{90} \cdot 461253 + \frac{1}{90} \cdot 461352 + \frac{1}{90} \cdot 631452$$
$$+ \frac{1}{90} \cdot 641253 + \frac{1}{90} \cdot 641352 - \frac{1}{45} \cdot 342156 - \frac{1}{90} \cdot 243516 - \frac{1}{90} \cdot 245316 - \frac{1}{90} \cdot 342516$$
$$- \frac{1}{90} \cdot 421563 - \frac{1}{45} \cdot 425163 - \frac{1}{90} \cdot 435162 - \frac{1}{90} \cdot 435261 - \frac{1}{90} \cdot 453162 - \frac{1}{90} \cdot 453261$$
$$+ \frac{1}{15} \cdot 543216 - \frac{1}{30} \cdot 632145 - \frac{1}{90} \cdot 632415 - \frac{1}{90} \cdot 634215 - \frac{1}{45} \cdot 431256 - \frac{1}{90} \cdot 513246$$
$$- \frac{1}{90} \cdot 514236 - \frac{1}{90} \cdot 531246 - \frac{1}{90} \cdot 532461 - \frac{1}{90} \cdot 542361 - \frac{1}{90} \cdot 326145 - \frac{1}{45} \cdot 362145$$
$$- \frac{1}{45} \cdot 426135 - \frac{1}{90} \cdot 462135 - \frac{1}{90} \cdot 463125 - \frac{1}{90} \cdot 642135 - \frac{1}{90} \cdot 643125 - \frac{1}{90} \cdot 365124$$
$$- \frac{1}{90} \cdot 365142 - \frac{1}{90} \cdot 365412 - \frac{1}{45} \cdot 426153 - \frac{1}{90} \cdot 426513 - \frac{1}{90} \cdot 436152 - \frac{1}{45} \cdot 436512$$
$$+ \frac{1}{15} \cdot 456123 + \frac{1}{90} \cdot 456132 + \frac{1}{90} \cdot 456213 - \frac{1}{90} \cdot 456231 - \frac{1}{90} \cdot 456312 - \frac{1}{90} \cdot 541623$$
$$- \frac{1}{90} \cdot 542613 - \frac{1}{90} \cdot 543612 - \frac{1}{90} \cdot 634512 + \frac{1}{15} \cdot 561234 - \frac{1}{90} \cdot 451632 - \frac{1}{90} \cdot 461532$$
$$- \frac{1}{90} \cdot 561432 - \frac{1}{45} \cdot 562143 - \frac{1}{90} \cdot 462153 - \frac{1}{90} \cdot 526143 - \frac{1}{90} \cdot 562341 - \frac{1}{90} \cdot 356214$$
$$- \frac{1}{90} \cdot 536214 - \frac{1}{90} \cdot 563214 + \frac{1}{90} \cdot 465123 + \frac{1}{90} \cdot 546123 - \frac{1}{90} \cdot 564123 - \frac{1}{90} \cdot 645123$$
$$+ \frac{1}{45} \cdot 365214 + \frac{1}{90} \cdot 365241 + \frac{1}{90} \cdot 365421 + \frac{1}{90} \cdot 426351 + \frac{1}{90} \cdot 426531 + \frac{1}{90} \cdot 436251$$
$$+ \frac{1}{45} \cdot 436521 - \frac{1}{30} \cdot 456321 + \frac{1}{45} \cdot 541632 + \frac{1}{90} \cdot 542631 + \frac{1}{90} \cdot 543621 - \frac{1}{30} \cdot 634521$$
$$- \frac{1}{90} \cdot 516324 - \frac{1}{90} \cdot 516342 - \frac{1}{90} \cdot 614352 - \frac{1}{90} \cdot 615324 - \frac{1}{90} \cdot 615342 - \frac{1}{45} \cdot 621435$$
$$- \frac{1}{90} \cdot 251634 - \frac{1}{90} \cdot 261435 - \frac{1}{90} \cdot 261534 + \frac{1}{45} \cdot 651234 - \frac{1}{45} \cdot 613254 - \frac{1}{90} \cdot 351264$$

$$- \frac{1}{90} \cdot 513264 - \frac{1}{90} \cdot 531264 - \frac{1}{90} \cdot 461325 - \frac{1}{90} \cdot 462315 - \frac{1}{90} \cdot 624315 - \frac{1}{90} \cdot 641325$$
$$- \frac{1}{90} \cdot 642315 + \frac{1}{90} \cdot 526413 + \frac{1}{90} \cdot 526431 + \frac{1}{90} \cdot 625413 + \frac{1}{90} \cdot 625431 + \frac{1}{90} \cdot 631524$$
$$+ \frac{1}{90} \cdot 631542 + \frac{1}{90} \cdot 632514 + \frac{1}{45} \cdot 632541 + \frac{1}{90} \cdot 352641 + \frac{1}{90} \cdot 362541 + \frac{1}{90} \cdot 532641$$
$$+ \frac{1}{90} \cdot 463152 + \frac{1}{90} \cdot 463251 + \frac{1}{90} \cdot 643152 + \frac{1}{90} \cdot 643251 - \frac{1}{30} \cdot 652341 + \frac{1}{90} \cdot 641532$$
$$+ \frac{1}{90} \cdot 651432 + \frac{1}{45} \cdot 652143 + \frac{1}{90} \cdot 624153 + \frac{1}{90} \cdot 625143 + \frac{1}{90} \cdot 642153 + \frac{1}{90} \cdot 635214$$
$$+ \frac{1}{90} \cdot 653214 - \frac{1}{30} \cdot 654123$$

$$[\![x_1 \times x_3]\!] = \frac{4}{45} \cdot 124356 + \frac{1}{45} \cdot 125346 + \frac{1}{30} \cdot 126345 + \frac{1}{15} \cdot 124536 + \frac{1}{30} \cdot 124563 + \frac{4}{45} \cdot 132456$$
$$+ \frac{2}{45} \cdot 132465 + \frac{2}{45} \cdot 132546 + \frac{2}{45} \cdot 132564 + \frac{2}{45} \cdot 132645 + \frac{1}{15} \cdot 134256 + \frac{1}{15} \cdot 134265$$
$$+ \frac{1}{90} \cdot 134526 - \frac{1}{30} \cdot 134625 - \frac{2}{45} \cdot 135246 + \frac{1}{45} \cdot 135264 + \frac{2}{45} \cdot 135624 - \frac{4}{45} \cdot 134562$$
$$- \frac{1}{15} \cdot 134652 - \frac{7}{90} \cdot 135426 - \frac{2}{45} \cdot 135462 + \frac{2}{45} \cdot 135642 - \frac{1}{30} \cdot 136245 - \frac{1}{90} \cdot 136425$$
$$+ \frac{1}{45} \cdot 136452 + \frac{1}{45} \cdot 142356 + \frac{1}{18} \cdot 152346 - \frac{4}{45} \cdot 162345 + \frac{4}{45} \cdot 213456 + \frac{2}{45} \cdot 213465$$
$$+ \frac{2}{45} \cdot 213546 + \frac{2}{45} \cdot 213564 + \frac{2}{45} \cdot 213645 + \frac{2}{45} \cdot 214356 + \frac{1}{15} \cdot 214536 + \frac{17}{90} \cdot 214563$$
$$+ \frac{1}{45} \cdot 215346 + \frac{17}{90} \cdot 216345 + \frac{2}{45} \cdot 231456 + \frac{2}{45} \cdot 231465 + \frac{2}{45} \cdot 231546 - \frac{1}{15} \cdot 231564$$
$$- \frac{1}{15} \cdot 231645 + \frac{1}{30} \cdot 234156 + \frac{17}{90} \cdot 234165 - \frac{4}{45} \cdot 234516 + \frac{1}{15} \cdot 234615 + \frac{1}{90} \cdot 235146$$
$$+ \frac{1}{30} \cdot 235164 + \frac{4}{45} \cdot 235614 - \frac{2}{9} \cdot 234561 - \frac{2}{45} \cdot 235416 + \frac{1}{45} \cdot 235461 + \frac{1}{30} \cdot 235641$$
$$- \frac{2}{15} \cdot 236145 - \frac{1}{30} \cdot 236415 + \frac{1}{90} \cdot 236451 - \frac{2}{45} \cdot 241356 + \frac{1}{90} \cdot 251346 + \frac{2}{45} \cdot 261345$$
$$- \frac{1}{30} \cdot 243156 - \frac{2}{45} \cdot 243516 + \frac{1}{45} \cdot 243561 - \frac{1}{90} \cdot 253146 - \frac{1}{45} \cdot 253416 - \frac{1}{90} \cdot 253461$$
$$- \frac{7}{90} \cdot 263145 - \frac{1}{15} \cdot 263415 - \frac{1}{30} \cdot 263451 + \frac{2}{45} \cdot 312456 + \frac{2}{45} \cdot 312465 + \frac{2}{45} \cdot 312546$$
$$- \frac{1}{15} \cdot 312564 - \frac{1}{15} \cdot 312645 + \frac{1}{30} \cdot 412356 + \frac{17}{90} \cdot 412365 - \frac{1}{30} \cdot 412536 + \frac{1}{30} \cdot 412635$$
$$- \frac{4}{45} \cdot 512346 + \frac{2}{45} \cdot 512364 + \frac{1}{9} \cdot 512634 - \frac{2}{45} \cdot 314256 - \frac{1}{30} \cdot 314526 + \frac{1}{15} \cdot 314562$$
$$+ \frac{1}{45} \cdot 315246 + \frac{1}{30} \cdot 316245 + \frac{4}{45} \cdot 415236 - \frac{1}{45} \cdot 516234 - \frac{1}{18} \cdot 324156 - \frac{1}{15} \cdot 324516$$
$$- \frac{2}{15} \cdot 412563 - \frac{1}{15} \cdot 512436 - \frac{7}{90} \cdot 512463 - \frac{2}{9} \cdot 612345 + \frac{1}{45} \cdot 612435 + \frac{1}{30} \cdot 612453$$
$$+ \frac{1}{90} \cdot 612534 - \frac{1}{18} \cdot 413256 - \frac{2}{45} \cdot 513246 + \frac{1}{45} \cdot 514236 + \frac{1}{45} \cdot 613245 - \frac{1}{90} \cdot 614235$$
$$- \frac{1}{30} \cdot 615234 - \frac{1}{30} \cdot 421356 - \frac{2}{45} \cdot 521346 + \frac{4}{45} \cdot 123465 + \frac{2}{45} \cdot 123645 + \frac{2}{45} \cdot 124365$$
$$- \frac{2}{45} \cdot 124635 + \frac{1}{45} \cdot 142365 + \frac{1}{45} \cdot 142635 + \frac{4}{45} \cdot 146235 + \frac{2}{45} \cdot 123564 + \frac{4}{45} \cdot 123546$$

$$-\frac{1}{18}\cdot 126435-\frac{2}{45}\cdot 162435-\frac{1}{15}\cdot 163245+\frac{2}{45}\cdot 163425+\frac{1}{45}\cdot 164235+\frac{1}{30}\cdot 241563$$
$$-\frac{2}{45}\cdot 245163+\frac{1}{30}\cdot 245361+\frac{1}{9}\cdot 361245-\frac{1}{45}\cdot 461235-\frac{1}{90}\cdot 413526+\frac{2}{45}\cdot 513426$$
$$-\frac{1}{30}\cdot 413562-\frac{1}{15}\cdot 513462+\frac{1}{90}\cdot 423561-\frac{1}{30}\cdot 523461+\frac{1}{30}\cdot 613425+\frac{1}{90}\cdot 631245$$
$$-\frac{1}{30}\cdot 641235-\frac{1}{18}\cdot 124653+\frac{2}{45}\cdot 351246+\frac{1}{90}\cdot 152364-\frac{2}{45}\cdot 142536+\frac{1}{90}\cdot 142563$$
$$+\frac{2}{45}\cdot 152634-\frac{7}{90}\cdot 143526-\frac{2}{45}\cdot 143562+\frac{1}{45}\cdot 423516-\frac{2}{45}\cdot 162354-\frac{1}{90}\cdot 152436$$
$$-\frac{1}{90}\cdot 153246+\frac{1}{45}\cdot 241536+\frac{2}{45}\cdot 341526+\frac{4}{45}\cdot 341562+\frac{2}{45}\cdot 342516+\frac{1}{30}\cdot 342561$$
$$-\frac{2}{45}\cdot 125364-\frac{1}{30}\cdot 125463-\frac{1}{90}\cdot 152463-\frac{1}{45}\cdot 153462+\frac{1}{30}\cdot 623145-\frac{1}{30}\cdot 126354$$
$$-\frac{4}{45}\cdot 132654-\frac{1}{18}\cdot 136254-\frac{1}{45}\cdot 136524-\frac{4}{45}\cdot 213654-\frac{2}{15}\cdot 214365-\frac{2}{45}\cdot 214635$$
$$-\frac{1}{30}\cdot 214653-\frac{2}{45}\cdot 215364-\frac{1}{90}\cdot 216354-\frac{1}{9}\cdot 231654+\frac{1}{15}\cdot 236514+\frac{7}{90}\cdot 236541$$
$$-\frac{2}{45}\cdot 241365+\frac{1}{18}\cdot 251364+\frac{2}{45}\cdot 261354-\frac{1}{90}\cdot 243165+\frac{4}{45}\cdot 243615+\frac{1}{9}\cdot 243651$$
$$-\frac{1}{90}\cdot 253164+\frac{1}{90}\cdot 253614-\frac{1}{45}\cdot 253641-\frac{1}{90}\cdot 263154+\frac{1}{45}\cdot 263514+\frac{1}{90}\cdot 263541$$
$$-\frac{1}{9}\cdot 312654+\frac{1}{45}\cdot 412653+\frac{1}{15}\cdot 512643-\frac{2}{45}\cdot 314265+\frac{1}{18}\cdot 314625+\frac{1}{15}\cdot 314652$$
$$-\frac{1}{15}\cdot 315264+\frac{1}{90}\cdot 316254+\frac{1}{45}\cdot 415263-\frac{1}{30}\cdot 324165+\frac{1}{15}\cdot 324615+\frac{4}{45}\cdot 324651$$
$$+\frac{7}{90}\cdot 612543-\frac{1}{30}\cdot 413265+\frac{2}{45}\cdot 513264+\frac{1}{90}\cdot 514263+\frac{1}{9}\cdot 613254-\frac{1}{45}\cdot 614253$$
$$+\frac{1}{90}\cdot 615243-\frac{1}{90}\cdot 421365+\frac{2}{45}\cdot 521364+\frac{4}{45}\cdot 621354-\frac{4}{45}\cdot 143265-\frac{1}{18}\cdot 143625$$
$$+\frac{1}{45}\cdot 146325-\frac{4}{45}\cdot 215436-\frac{1}{18}\cdot 315426+\frac{1}{45}\cdot 415326-\frac{1}{90}\cdot 215463-\frac{1}{90}\cdot 251463$$
$$-\frac{1}{9}\cdot 254163-\frac{1}{30}\cdot 216435-\frac{1}{15}\cdot 241635-\frac{1}{18}\cdot 316425-\frac{1}{18}\cdot 413625-\frac{1}{9}\cdot 416325$$
$$+\frac{7}{90}\cdot 254361+\frac{1}{45}\cdot 246135+\frac{1}{90}\cdot 246315+\frac{2}{45}\cdot 261435+\frac{1}{90}\cdot 264135-\frac{2}{45}\cdot 264315$$
$$-\frac{1}{30}\cdot 361425-\frac{1}{45}\cdot 246351+\frac{1}{90}\cdot 264351+\frac{4}{45}\cdot 315462+\frac{1}{90}\cdot 415362-\frac{2}{45}\cdot 514362$$
$$-\frac{1}{30}\cdot 513624+\frac{1}{9}\cdot 325461-\frac{1}{45}\cdot 425361+\frac{1}{90}\cdot 524361+\frac{7}{90}\cdot 614325-\frac{1}{45}\cdot 613524$$
$$+\frac{1}{90}\cdot 615324+\frac{1}{9}\cdot 621435-\frac{1}{45}\cdot 631425+\frac{1}{90}\cdot 641325-\frac{2}{45}\cdot 125643-\frac{1}{15}\cdot 126453$$
$$-\frac{1}{90}\cdot 142653+\frac{1}{15}\cdot 146253-\frac{1}{45}\cdot 152643+\frac{1}{15}\cdot 156243-\frac{1}{45}\cdot 145326+\frac{2}{45}\cdot 156324$$
$$+\frac{1}{45}\cdot 145362-\frac{1}{45}\cdot 156342+\frac{1}{9}\cdot 145623+\frac{2}{45}\cdot 146523-\frac{1}{15}\cdot 154263+\frac{1}{15}\cdot 154623$$
$$-\frac{1}{45}\cdot 164523+\frac{1}{15}\cdot 251634+\frac{1}{18}\cdot 256134-\frac{2}{45}\cdot 215643+\frac{2}{45}\cdot 251643+\frac{11}{90}\cdot 256143$$
$$-\frac{1}{15}\cdot 216453+\frac{1}{90}\cdot 241653+\frac{1}{15}\cdot 246153+\frac{1}{45}\cdot 245316-\frac{1}{18}\cdot 256314-\frac{1}{9}\cdot 256341$$
$$-\frac{1}{45}\cdot 245613+\frac{1}{45}\cdot 254613+\frac{1}{30}\cdot 256413+\frac{1}{90}\cdot 264153+\frac{1}{90}\cdot 264513-\frac{1}{18}\cdot 245631$$

$$- \frac{1}{30} \cdot 246531 - \frac{1}{90} \cdot 254631 + \frac{1}{45} \cdot 256431 + \frac{2}{45} \cdot 315624 - \frac{1}{45} \cdot 316452 + \frac{1}{30} \cdot 413652$$
$$- \frac{1}{30} \cdot 416352 + \frac{1}{45} \cdot 513642 + \frac{1}{18} \cdot 516342 + \frac{1}{10} \cdot 325641 + \frac{1}{30} \cdot 415623 - \frac{1}{90} \cdot 514623$$
$$- \frac{1}{9} \cdot 614523 - \frac{1}{30} \cdot 415632 + \frac{1}{90} \cdot 514632 - \frac{1}{18} \cdot 613452 - \frac{1}{30} \cdot 613542 - \frac{1}{90} \cdot 614352$$
$$+ \frac{1}{45} \cdot 614532 - \frac{1}{90} \cdot 521463 + \frac{1}{10} \cdot 621453 - \frac{4}{45} \cdot 125634 - \frac{1}{9} \cdot 361452 - \frac{1}{15} \cdot 143652$$
$$- \frac{4}{45} \cdot 145236 + \frac{1}{90} \cdot 325164 + \frac{1}{9} \cdot 145632 + \frac{7}{45} \cdot 325614 - \frac{1}{18} \cdot 461352 - \frac{1}{15} \cdot 153426$$
$$+ \frac{1}{15} \cdot 153624 + \frac{1}{45} \cdot 154632 + \frac{1}{9} \cdot 163452 + \frac{1}{45} \cdot 163542 + \frac{1}{45} \cdot 164352 - \frac{2}{45} \cdot 126534$$
$$- \frac{1}{90} \cdot 153264 - \frac{1}{15} \cdot 154236 + \frac{1}{9} \cdot 156234 - \frac{2}{45} \cdot 216534 + \frac{2}{45} \cdot 316524 + \frac{11}{90} \cdot 416523$$
$$+ \frac{1}{30} \cdot 361524 + \frac{1}{90} \cdot 265134 - \frac{1}{30} \cdot 265314 + \frac{1}{18} \cdot 516423 + \frac{1}{45} \cdot 326145 + \frac{1}{30} \cdot 326415$$
$$+ \frac{7}{90} \cdot 326451 - \frac{1}{30} \cdot 426315 + \frac{1}{90} \cdot 426351 - \frac{1}{30} \cdot 526134 - \frac{1}{18} \cdot 526314 - \frac{1}{90} \cdot 526341$$
$$+ \frac{7}{90} \cdot 621534 + \frac{1}{90} \cdot 631524 - \frac{1}{90} \cdot 641523 - \frac{1}{15} \cdot 163254 + \frac{1}{9} \cdot 165234 + \frac{7}{45} \cdot 521634$$
$$+ \frac{1}{45} \cdot 165243 + \frac{1}{30} \cdot 531624 - \frac{4}{45} \cdot 126543 - \frac{4}{45} \cdot 154326 - \frac{1}{45} \cdot 154362 - \frac{1}{45} \cdot 162543$$
$$- \frac{1}{45} \cdot 164532 - \frac{8}{45} \cdot 216543 - \frac{1}{45} \cdot 316542 - \frac{1}{30} \cdot 416532 - \frac{1}{90} \cdot 251436 - \frac{1}{15} \cdot 254136$$
$$- \frac{1}{45} \cdot 254316 - \frac{1}{45} \cdot 261543 - \frac{1}{45} \cdot 361542 - \frac{1}{90} \cdot 265143 + \frac{1}{90} \cdot 265413 + \frac{2}{45} \cdot 265431$$
$$+ \frac{1}{30} \cdot 516432 + \frac{1}{45} \cdot 326154 + \frac{4}{45} \cdot 326514 + \frac{1}{18} \cdot 326541 + \frac{1}{45} \cdot 426153 + \frac{7}{90} \cdot 426513$$
$$- \frac{1}{45} \cdot 426531 + \frac{1}{90} \cdot 526143 + \frac{1}{45} \cdot 526413 + \frac{1}{90} \cdot 526431 + \frac{2}{45} \cdot 615432 + \frac{1}{18} \cdot 621543$$
$$- \frac{1}{45} \cdot 631542 + \frac{1}{90} \cdot 641532 - \frac{1}{45} \cdot 165342 + \frac{1}{45} \cdot 421653 + \frac{1}{15} \cdot 521643 - \frac{4}{45} \cdot 321465$$
$$- \frac{4}{45} \cdot 321546 - \frac{1}{18} \cdot 421536 - \frac{1}{45} \cdot 431526 - \frac{1}{9} \cdot 321564 + \frac{1}{15} \cdot 431562 - \frac{1}{9} \cdot 321645$$
$$+ \frac{1}{15} \cdot 362145 + \frac{7}{90} \cdot 432561 + \frac{1}{90} \cdot 421635 + \frac{1}{90} \cdot 351462 - \frac{1}{45} \cdot 352461 + \frac{1}{45} \cdot 531462$$
$$+ \frac{1}{90} \cdot 532461 + \frac{7}{90} \cdot 632145 - \frac{1}{45} \cdot 624135 + \frac{1}{90} \cdot 642135 - \frac{1}{5} \cdot 321654 - \frac{1}{15} \cdot 325416$$
$$- \frac{2}{45} \cdot 342165 + \frac{7}{45} \cdot 341652 + \frac{1}{10} \cdot 342651 + \frac{1}{15} \cdot 351264 + \frac{2}{45} \cdot 352164 + \frac{7}{45} \cdot 361254$$
$$+ \frac{1}{15} \cdot 362154 - \frac{1}{15} \cdot 521436 - \frac{1}{15} \cdot 423165 + \frac{4}{45} \cdot 431652 + \frac{1}{18} \cdot 432651 + \frac{1}{10} \cdot 623154$$
$$+ \frac{1}{90} \cdot 524163 - \frac{1}{45} \cdot 532164 + \frac{1}{18} \cdot 632154 - \frac{1}{90} \cdot 325146 - \frac{1}{45} \cdot 423615 + \frac{7}{90} \cdot 423651$$
$$+ \frac{1}{90} \cdot 462153 - \frac{2}{45} \cdot 431265 + \frac{2}{45} \cdot 341625 + \frac{2}{45} \cdot 431625 - \frac{1}{45} \cdot 432615 + \frac{7}{90} \cdot 631254$$
$$- \frac{4}{45} \cdot 341256 - \frac{2}{45} \cdot 342156 + \frac{1}{9} \cdot 345126 + \frac{1}{9} \cdot 345216 + \frac{1}{30} \cdot 346125 - \frac{1}{30} \cdot 346215$$
$$+ \frac{1}{15} \cdot 351426 + \frac{1}{45} \cdot 362415 + \frac{1}{15} \cdot 354126 + \frac{1}{45} \cdot 354216 - \frac{1}{90} \cdot 364125 + \frac{1}{90} \cdot 364215$$
$$- \frac{1}{15} \cdot 423156 - \frac{1}{9} \cdot 523614 + \frac{1}{15} \cdot 425136 + \frac{1}{15} \cdot 425163 + \frac{2}{45} \cdot 435126 + \frac{1}{9} \cdot 523416$$

$$+ \frac{1}{45} \cdot 524316 + \frac{1}{45} \cdot 532416 + \frac{1}{18} \cdot 451263 + \frac{2}{45} \cdot 451326 - \frac{1}{18} \cdot 451362 - \frac{1}{45} \cdot 352146$$
$$+ \frac{1}{15} \cdot 452136 + \frac{11}{90} \cdot 452163 - \frac{1}{45} \cdot 452316 - \frac{1}{9} \cdot 452361 + \frac{1}{18} \cdot 462315 - \frac{1}{45} \cdot 534126$$
$$- \frac{1}{45} \cdot 345162 + \frac{1}{45} \cdot 354162 + \frac{1}{30} \cdot 453162 + \frac{1}{90} \cdot 534162 - \frac{1}{18} \cdot 345261 - \frac{1}{90} \cdot 354261$$
$$- \frac{1}{30} \cdot 435261 + \frac{1}{45} \cdot 453261 - \frac{1}{9} \cdot 634125 - \frac{1}{18} \cdot 623415 - \frac{1}{90} \cdot 624315 - \frac{1}{30} \cdot 632415$$
$$+ \frac{1}{45} \cdot 634215 - \frac{8}{45} \cdot 345612 - \frac{8}{45} \cdot 345621 - \frac{2}{45} \cdot 346512 - \frac{4}{45} \cdot 346521 - \frac{2}{45} \cdot 362451$$
$$- \frac{1}{45} \cdot 354612 - \frac{1}{15} \cdot 354621 + \frac{1}{90} \cdot 425613 - \frac{2}{45} \cdot 425631 - \frac{2}{45} \cdot 435612 - \frac{4}{45} \cdot 435621$$
$$- \frac{8}{45} \cdot 623451 - \frac{4}{45} \cdot 623541 - \frac{1}{15} \cdot 624351 - \frac{4}{45} \cdot 632451 + \frac{1}{90} \cdot 346152 - \frac{2}{45} \cdot 346251$$
$$- \frac{2}{45} \cdot 523641 - \frac{1}{90} \cdot 364152 - \frac{1}{15} \cdot 356124 - \frac{1}{15} \cdot 356214 - \frac{2}{45} \cdot 365124 - \frac{2}{45} \cdot 365214$$
$$+ \frac{1}{90} \cdot 352614 - \frac{2}{45} \cdot 356142 - \frac{1}{18} \cdot 356241 - \frac{2}{45} \cdot 365142 - \frac{1}{30} \cdot 365241 + \frac{7}{90} \cdot 436152$$
$$- \frac{1}{45} \cdot 436251 - \frac{2}{45} \cdot 625134 - \frac{2}{45} \cdot 623514 - \frac{1}{18} \cdot 624513 - \frac{1}{30} \cdot 625413 - \frac{1}{45} \cdot 532614$$
$$- \frac{1}{45} \cdot 632514 - \frac{2}{45} \cdot 431256 + \frac{11}{90} \cdot 436125 + \frac{1}{9} \cdot 451236 + \frac{1}{18} \cdot 463125 - \frac{1}{30} \cdot 461253$$
$$- \frac{1}{90} \cdot 462351 + \frac{1}{90} \cdot 541263 - \frac{1}{30} \cdot 541362 - \frac{1}{90} \cdot 635124 + \frac{1}{9} \cdot 541236 + \frac{1}{45} \cdot 542136$$
$$- \frac{1}{90} \cdot 524613 - \frac{1}{15} \cdot 451623 - \frac{1}{15} \cdot 451632 - \frac{2}{45} \cdot 541623 - \frac{2}{45} \cdot 541632 + \frac{1}{90} \cdot 351642$$
$$- \frac{2}{45} \cdot 452613 - \frac{1}{18} \cdot 452631 - \frac{2}{45} \cdot 542613 - \frac{1}{30} \cdot 542631 - \frac{2}{45} \cdot 631452 - \frac{2}{45} \cdot 641253$$
$$- \frac{1}{18} \cdot 634152 - \frac{1}{30} \cdot 643152 - \frac{4}{45} \cdot 432156 - \frac{8}{45} \cdot 432165 - \frac{1}{30} \cdot 436215 + \frac{1}{30} \cdot 463215$$
$$+ \frac{1}{45} \cdot 463152 + \frac{1}{90} \cdot 463251 - \frac{1}{45} \cdot 532146 - \frac{1}{45} \cdot 534216 - \frac{1}{90} \cdot 542163 + \frac{1}{90} \cdot 543162$$
$$+ \frac{2}{45} \cdot 543261 + \frac{1}{90} \cdot 635214 + \frac{2}{45} \cdot 643215 - \frac{1}{45} \cdot 542316 - \frac{1}{45} \cdot 351624 + \frac{1}{45} \cdot 356412$$
$$+ \frac{2}{45} \cdot 436512 + \frac{1}{45} \cdot 453612 - \frac{1}{5} \cdot 456123 - \frac{1}{15} \cdot 456132 - \frac{1}{15} \cdot 456213 + \frac{1}{30} \cdot 456231$$
$$+ \frac{1}{30} \cdot 456312 + \frac{1}{45} \cdot 463512 - \frac{1}{15} \cdot 465123 - \frac{1}{45} \cdot 465132 - \frac{1}{45} \cdot 465213 + \frac{1}{90} \cdot 465231$$
$$+ \frac{1}{90} \cdot 465312 + \frac{1}{45} \cdot 536412 - \frac{1}{15} \cdot 546123 - \frac{1}{45} \cdot 546132 - \frac{1}{45} \cdot 546213 + \frac{1}{90} \cdot 546231$$
$$+ \frac{1}{90} \cdot 546312 + \frac{1}{30} \cdot 634512 + \frac{1}{90} \cdot 635412 + \frac{1}{90} \cdot 643512 - \frac{2}{45} \cdot 561243 - \frac{1}{45} \cdot 561324$$
$$+ \frac{1}{45} \cdot 561342 - \frac{2}{45} \cdot 562134 + \frac{2}{45} \cdot 562143 + \frac{1}{45} \cdot 562314 + \frac{1}{30} \cdot 562341 + \frac{1}{45} \cdot 562413$$
$$+ \frac{1}{90} \cdot 462531 + \frac{1}{90} \cdot 562431 + \frac{1}{45} \cdot 563142 + \frac{1}{90} \cdot 536241 + \frac{1}{90} \cdot 563241 + \frac{1}{30} \cdot 564123$$
$$+ \frac{1}{30} \cdot 645123 + \frac{1}{90} \cdot 564132 + \frac{1}{90} \cdot 635142 + \frac{1}{90} \cdot 645132 + \frac{1}{90} \cdot 564213 + \frac{1}{90} \cdot 642513$$
$$+ \frac{1}{90} \cdot 645213 + \frac{1}{90} \cdot 352641 + \frac{1}{45} \cdot 356421 - \frac{2}{45} \cdot 436521 + \frac{1}{45} \cdot 453621 + \frac{1}{10} \cdot 456321$$
$$+ \frac{1}{45} \cdot 463521 + \frac{1}{30} \cdot 465321 + \frac{1}{45} \cdot 536421 + \frac{1}{30} \cdot 546321 + \frac{1}{45} \cdot 634251 + \frac{1}{10} \cdot 634521$$

$$
\begin{aligned}
&+\frac{1}{45}\cdot 624531+\frac{1}{30}\cdot 635421+\frac{1}{30}\cdot 643521-\frac{8}{45}\cdot 561234-\frac{8}{45}\cdot 651234-\frac{4}{45}\cdot 651243\\
&-\frac{1}{15}\cdot 651324-\frac{4}{45}\cdot 652134+\frac{1}{90}\cdot 624153-\frac{2}{45}\cdot 632541-\frac{1}{45}\cdot 532641-\frac{1}{45}\cdot 362541\\
&+\frac{1}{45}\cdot 635241+\frac{1}{45}\cdot 642531+\frac{1}{45}\cdot 652314+\frac{1}{10}\cdot 652341+\frac{1}{45}\cdot 651342+\frac{1}{30}\cdot 652431\\
&+\frac{1}{30}\cdot 653241-\frac{2}{45}\cdot 652143-\frac{1}{45}\cdot 642153-\frac{1}{45}\cdot 625143+\frac{1}{45}\cdot 652413+\frac{1}{45}\cdot 653142\\
&+\frac{1}{10}\cdot 654123+\frac{1}{30}\cdot 654132+\frac{1}{30}\cdot 654213
\end{aligned}
$$

$$
\begin{aligned}
[\![x_1\times x_4]\!] =& \frac{1}{9}\cdot 132456+\frac{1}{18}\cdot 134256+\frac{1}{30}\cdot 134526-\frac{2}{45}\cdot 134562+\frac{1}{18}\cdot 142356+\frac{1}{30}\cdot 152346\\
&-\frac{2}{45}\cdot 162345+\frac{8}{45}\cdot 213456+\frac{2}{45}\cdot 213465+\frac{1}{15}\cdot 213546+\frac{1}{30}\cdot 213564+\frac{1}{30}\cdot 213645\\
&+\frac{2}{45}\cdot 214356+\frac{7}{90}\cdot 214536+\frac{17}{90}\cdot 214563+\frac{7}{90}\cdot 215346+\frac{17}{90}\cdot 216345+\frac{1}{18}\cdot 231456\\
&+\frac{1}{18}\cdot 231465+\frac{1}{30}\cdot 231546-\frac{1}{15}\cdot 231564-\frac{1}{15}\cdot 231645+\frac{1}{18}\cdot 234156+\frac{17}{90}\cdot 234165\\
&-\frac{2}{15}\cdot 234516+\frac{1}{30}\cdot 234615+\frac{1}{18}\cdot 235164+\frac{7}{90}\cdot 235614-\frac{2}{9}\cdot 234561-\frac{1}{18}\cdot 234651\\
&-\frac{1}{18}\cdot 235416+\frac{1}{90}\cdot 235461+\frac{1}{90}\cdot 235641-\frac{2}{15}\cdot 236145-\frac{1}{30}\cdot 236415+\frac{1}{90}\cdot 236451\\
&-\frac{1}{15}\cdot 241356+\frac{1}{30}\cdot 241536+\frac{1}{90}\cdot 241563+\frac{1}{18}\cdot 245136-\frac{1}{45}\cdot 245163-\frac{1}{90}\cdot 245613\\
&-\frac{1}{45}\cdot 251346+\frac{7}{90}\cdot 261345-\frac{2}{45}\cdot 243156-\frac{1}{18}\cdot 243516+\frac{1}{30}\cdot 243561+\frac{1}{90}\cdot 245361\\
&-\frac{1}{18}\cdot 245631-\frac{1}{30}\cdot 253146-\frac{1}{45}\cdot 253416+\frac{1}{90}\cdot 253461-\frac{7}{90}\cdot 263145-\frac{1}{15}\cdot 263415\\
&-\frac{1}{18}\cdot 263451+\frac{1}{18}\cdot 312456+\frac{1}{18}\cdot 312465+\frac{1}{30}\cdot 312546-\frac{1}{15}\cdot 312564-\frac{1}{15}\cdot 312645\\
&+\frac{1}{18}\cdot 412356+\frac{17}{90}\cdot 412365+\frac{1}{18}\cdot 412635-\frac{2}{15}\cdot 512346+\frac{1}{30}\cdot 512364+\frac{7}{90}\cdot 512634\\
&-\frac{1}{15}\cdot 314256-\frac{1}{45}\cdot 314526+\frac{7}{90}\cdot 314562+\frac{1}{30}\cdot 315246+\frac{1}{90}\cdot 316245+\frac{1}{18}\cdot 415236\\
&-\frac{1}{45}\cdot 416235-\frac{1}{90}\cdot 516234-\frac{2}{15}\cdot 412563-\frac{1}{18}\cdot 512436-\frac{1}{30}\cdot 512463-\frac{2}{9}\cdot 612345\\
&-\frac{1}{18}\cdot 612354+\frac{1}{90}\cdot 612435+\frac{1}{90}\cdot 612453+\frac{1}{90}\cdot 612534-\frac{2}{45}\cdot 413256-\frac{1}{30}\cdot 413526\\
&-\frac{7}{90}\cdot 413562-\frac{1}{18}\cdot 513246-\frac{1}{45}\cdot 513426-\frac{1}{15}\cdot 513462+\frac{1}{30}\cdot 613245+\frac{1}{90}\cdot 613425\\
&-\frac{1}{18}\cdot 613452+\frac{1}{90}\cdot 614235-\frac{1}{18}\cdot 615234+\frac{4}{45}\cdot 124356+\frac{1}{30}\cdot 124536+\frac{1}{90}\cdot 124563\\
&+\frac{1}{30}\cdot 125346+\frac{1}{90}\cdot 126345+\frac{1}{45}\cdot 132465+\frac{2}{45}\cdot 132546+\frac{1}{18}\cdot 132564+\frac{1}{18}\cdot 132645\\
&+\frac{1}{90}\cdot 134265-\frac{1}{15}\cdot 324156-\frac{1}{18}\cdot 134652-\frac{1}{18}\cdot 324516+\frac{1}{18}\cdot 324561-\frac{2}{45}\cdot 135246\\
&+\frac{1}{90}\cdot 135264+\frac{1}{30}\cdot 135624-\frac{1}{45}\cdot 136245-\frac{1}{45}\cdot 135426-\frac{1}{30}\cdot 135462+\frac{1}{90}\cdot 136425\\
&+\frac{1}{90}\cdot 142365-\frac{1}{15}\cdot 421356-\frac{2}{45}\cdot 142536-\frac{1}{45}\cdot 142563+\frac{1}{90}\cdot 142635+\frac{1}{30}\cdot 152634
\end{aligned}
$$

$$- \frac{1}{18} \cdot 162354 - \frac{1}{18} \cdot 521346 + \frac{1}{18} \cdot 621345 - \frac{1}{45} \cdot 152436 + \frac{1}{90} \cdot 152463 - \frac{1}{30} \cdot 162435$$
$$+ \frac{1}{15} \cdot 123546 + \frac{1}{18} \cdot 341526 + \frac{1}{18} \cdot 351246 + \frac{1}{30} \cdot 123564 + \frac{11}{90} \cdot 341562 + \frac{1}{30} \cdot 123645$$
$$+ \frac{11}{90} \cdot 361245 + \frac{2}{45} \cdot 124365 - \frac{1}{15} \cdot 143526 + \frac{2}{45} \cdot 342516 + \frac{1}{45} \cdot 423516 - \frac{1}{18} \cdot 143562$$
$$+ \frac{1}{30} \cdot 342561 + \frac{1}{30} \cdot 423561 - \frac{1}{45} \cdot 124635 - \frac{1}{45} \cdot 124653 - \frac{1}{15} \cdot 153246 + \frac{1}{45} \cdot 523146$$
$$+ \frac{2}{45} \cdot 531246 - \frac{1}{45} \cdot 125364 - \frac{1}{18} \cdot 163245 + \frac{1}{30} \cdot 623145 + \frac{1}{30} \cdot 631245 - \frac{1}{45} \cdot 126354$$
$$- \frac{1}{9} \cdot 213654 - \frac{2}{15} \cdot 214365 - \frac{1}{45} \cdot 214635 - \frac{1}{45} \cdot 215364 - \frac{1}{18} \cdot 231654 + \frac{1}{90} \cdot 236154$$
$$+ \frac{1}{18} \cdot 236514 + \frac{7}{90} \cdot 236541 - \frac{1}{15} \cdot 241365 - \frac{1}{15} \cdot 241635 + \frac{1}{45} \cdot 246135 + \frac{1}{90} \cdot 246153$$
$$- \frac{1}{90} \cdot 246513 + \frac{1}{18} \cdot 251364 + \frac{1}{15} \cdot 261354 + \frac{1}{45} \cdot 243165 + \frac{4}{45} \cdot 243615 + \frac{1}{9} \cdot 243651$$
$$+ \frac{1}{45} \cdot 246315 - \frac{1}{90} \cdot 246351 + \frac{1}{90} \cdot 246531 - \frac{2}{45} \cdot 253164 - \frac{1}{90} \cdot 253614 - \frac{1}{90} \cdot 253641$$
$$+ \frac{1}{30} \cdot 263514 + \frac{1}{90} \cdot 263541 - \frac{1}{18} \cdot 312654 + \frac{1}{90} \cdot 412653 + \frac{1}{18} \cdot 512643 - \frac{1}{15} \cdot 314265$$
$$+ \frac{1}{18} \cdot 314625 + \frac{1}{15} \cdot 314652 - \frac{1}{15} \cdot 315264 + \frac{1}{45} \cdot 415263 + \frac{1}{90} \cdot 416253 - \frac{1}{90} \cdot 516243$$
$$+ \frac{7}{90} \cdot 612543 + \frac{1}{45} \cdot 413265 - \frac{2}{45} \cdot 413625 + \frac{4}{45} \cdot 513264 - \frac{1}{90} \cdot 513624 + \frac{1}{30} \cdot 513642$$
$$+ \frac{1}{9} \cdot 613254 - \frac{1}{90} \cdot 613524 + \frac{1}{90} \cdot 613542 + \frac{1}{45} \cdot 514263 - \frac{1}{90} \cdot 614253 + \frac{1}{90} \cdot 615243$$
$$- \frac{1}{9} \cdot 215436 - \frac{1}{30} \cdot 251436 - \frac{1}{30} \cdot 254136 - \frac{1}{30} \cdot 315426 - \frac{1}{30} \cdot 415326 - \frac{1}{15} \cdot 215463$$
$$- \frac{1}{45} \cdot 251463 - \frac{1}{9} \cdot 254163 - \frac{1}{15} \cdot 216435 - \frac{1}{45} \cdot 316425 - \frac{1}{9} \cdot 416325 + \frac{7}{90} \cdot 254361$$
$$+ \frac{1}{90} \cdot 254613 + \frac{2}{45} \cdot 261435 - \frac{2}{45} \cdot 264315 - \frac{1}{90} \cdot 254631 - \frac{1}{90} \cdot 264351 + \frac{2}{45} \cdot 315462$$
$$- \frac{2}{45} \cdot 514362 + \frac{1}{90} \cdot 516324 + \frac{7}{90} \cdot 614325 - \frac{1}{90} \cdot 614352 - \frac{1}{90} \cdot 615324 + \frac{1}{15} \cdot 251634$$
$$+ \frac{7}{90} \cdot 256134 - \frac{4}{45} \cdot 215643 + \frac{1}{15} \cdot 251643 + \frac{11}{90} \cdot 256143 - \frac{4}{45} \cdot 216453 - \frac{2}{45} \cdot 256314$$
$$- \frac{1}{9} \cdot 256341 + \frac{1}{18} \cdot 256413 - \frac{1}{90} \cdot 261453 - \frac{1}{90} \cdot 264153 + \frac{1}{18} \cdot 264513 + \frac{1}{90} \cdot 256431$$
$$+ \frac{1}{90} \cdot 264531 + \frac{1}{15} \cdot 315624 - \frac{1}{90} \cdot 315642 - \frac{1}{90} \cdot 316452 - \frac{1}{90} \cdot 416352 + \frac{1}{18} \cdot 516342$$
$$+ \frac{7}{90} \cdot 415623 - \frac{2}{45} \cdot 514623 - \frac{1}{9} \cdot 614523 - \frac{2}{45} \cdot 415632 - \frac{1}{90} \cdot 514632 + \frac{1}{90} \cdot 614532$$
$$+ \frac{1}{90} \cdot 615342 - \frac{2}{45} \cdot 125463 - \frac{1}{90} \cdot 351462 - \frac{4}{45} \cdot 125634 - \frac{2}{45} \cdot 125643 - \frac{2}{45} \cdot 126453$$
$$- \frac{1}{9} \cdot 361452 - \frac{1}{18} \cdot 142653 - \frac{1}{30} \cdot 143625 - \frac{1}{15} \cdot 143652 - \frac{4}{45} \cdot 145236 - \frac{2}{45} \cdot 145326$$
$$+ \frac{1}{30} \cdot 145263 + \frac{2}{45} \cdot 145362 + \frac{1}{45} \cdot 325164 + \frac{13}{90} \cdot 145623 + \frac{1}{9} \cdot 145632 + \frac{7}{45} \cdot 325614$$
$$+ \frac{1}{9} \cdot 325641 + \frac{1}{30} \cdot 146235 - \frac{1}{90} \cdot 146325 + \frac{2}{45} \cdot 146253 + \frac{1}{90} \cdot 146352 + \frac{1}{18} \cdot 146523$$
$$+ \frac{2}{45} \cdot 146532 - \frac{1}{15} \cdot 153426 + \frac{2}{45} \cdot 153462 + \frac{1}{45} \cdot 521463 + \frac{1}{15} \cdot 153624 + \frac{1}{90} \cdot 153642$$

$$+\frac{1}{9}\cdot 163452+\frac{1}{9}\cdot 621453+\frac{2}{45}\cdot 163542-\frac{4}{45}\cdot 216534+\frac{1}{15}\cdot 316524+\frac{11}{90}\cdot 416523$$
$$-\frac{1}{90}\cdot 261534-\frac{2}{45}\cdot 265134-\frac{1}{90}\cdot 265314+\frac{1}{90}\cdot 265341+\frac{1}{18}\cdot 516423+\frac{1}{90}\cdot 615423$$
$$-\frac{2}{45}\cdot 126435-\frac{1}{90}\cdot 361425-\frac{2}{45}\cdot 126534-\frac{1}{15}\cdot 163254-\frac{1}{30}\cdot 153264-\frac{1}{18}\cdot 136254$$
$$+\frac{2}{45}\cdot 163425+\frac{1}{45}\cdot 326415+\frac{1}{9}\cdot 326451+\frac{1}{90}\cdot 163524-\frac{2}{45}\cdot 154236+\frac{2}{45}\cdot 164235$$
$$+\frac{1}{45}\cdot 421635+\frac{1}{90}\cdot 164253-\frac{1}{90}\cdot 154263+\frac{13}{90}\cdot 156234+\frac{1}{9}\cdot 165234+\frac{7}{45}\cdot 521634$$
$$+\frac{1}{9}\cdot 621534+\frac{1}{18}\cdot 156243+\frac{2}{45}\cdot 165243-\frac{2}{45}\cdot 132654-\frac{1}{30}\cdot 152643-\frac{1}{30}\cdot 136524$$
$$-\frac{1}{45}\cdot 136542-\frac{1}{45}\cdot 162543-\frac{8}{45}\cdot 216543-\frac{1}{90}\cdot 316542-\frac{1}{45}\cdot 416532-\frac{1}{90}\cdot 261543$$
$$-\frac{1}{45}\cdot 265143+\frac{2}{45}\cdot 265413+\frac{4}{45}\cdot 265431+\frac{2}{45}\cdot 516432+\frac{4}{45}\cdot 615432-\frac{2}{15}\cdot 321546$$
$$-\frac{1}{90}\cdot 421536-\frac{1}{90}\cdot 431526-\frac{1}{90}\cdot 325146-\frac{1}{90}\cdot 352146-\frac{1}{6}\cdot 321564+\frac{1}{90}\cdot 421563$$
$$+\frac{7}{90}\cdot 431562-\frac{1}{6}\cdot 321645+\frac{1}{90}\cdot 326145+\frac{7}{90}\cdot 362145-\frac{2}{45}\cdot 324165-\frac{2}{45}\cdot 421365$$
$$+\frac{7}{90}\cdot 432561+\frac{2}{45}\cdot 324615+\frac{4}{45}\cdot 324651+\frac{2}{45}\cdot 521364+\frac{7}{90}\cdot 632145+\frac{4}{45}\cdot 621354$$
$$-\frac{1}{15}\cdot 143265-\frac{1}{15}\cdot 321465-\frac{1}{5}\cdot 321654-\frac{1}{15}\cdot 325416+\frac{1}{9}\cdot 325461+\frac{7}{45}\cdot 341652$$
$$+\frac{1}{15}\cdot 342651+\frac{1}{15}\cdot 326514+\frac{2}{45}\cdot 351264+\frac{1}{45}\cdot 352164+\frac{7}{45}\cdot 361254+\frac{4}{45}\cdot 362154$$
$$+\frac{1}{15}\cdot 326541-\frac{1}{15}\cdot 521436-\frac{2}{45}\cdot 423165+\frac{1}{45}\cdot 421653+\frac{1}{90}\cdot 526143+\frac{1}{9}\cdot 621435$$
$$-\frac{1}{90}\cdot 523164+\frac{1}{15}\cdot 623154+\frac{1}{15}\cdot 521643+\frac{1}{15}\cdot 621543-\frac{1}{90}\cdot 524163-\frac{1}{90}\cdot 423615$$
$$+\frac{1}{15}\cdot 423651+\frac{1}{45}\cdot 326154+\frac{1}{90}\cdot 426513-\frac{1}{90}\cdot 426315+\frac{2}{45}\cdot 341625+\frac{1}{45}\cdot 431625$$
$$+\frac{4}{45}\cdot 431652+\frac{1}{15}\cdot 631254-\frac{4}{45}\cdot 341256-\frac{2}{45}\cdot 342156+\frac{7}{90}\cdot 345126+\frac{1}{9}\cdot 345216$$
$$+\frac{1}{90}\cdot 346125+\frac{1}{45}\cdot 346215+\frac{1}{15}\cdot 351426-\frac{1}{90}\cdot 352416+\frac{1}{90}\cdot 362415+\frac{2}{45}\cdot 351642$$
$$-\frac{1}{30}\cdot 352461+\frac{1}{90}\cdot 352641+\frac{7}{90}\cdot 354126+\frac{2}{45}\cdot 354216-\frac{1}{45}\cdot 364125-\frac{1}{90}\cdot 364215$$
$$-\frac{4}{45}\cdot 423156-\frac{1}{9}\cdot 523614+\frac{4}{45}\cdot 425136+\frac{1}{18}\cdot 425163-\frac{1}{90}\cdot 425316-\frac{2}{45}\cdot 526314$$
$$+\frac{1}{9}\cdot 523416+\frac{1}{15}\cdot 524316-\frac{1}{30}\cdot 624135+\frac{1}{90}\cdot 624153+\frac{7}{90}\cdot 451326-\frac{1}{45}\cdot 451362$$
$$+\frac{1}{18}\cdot 452136+\frac{11}{90}\cdot 452163-\frac{1}{45}\cdot 452316-\frac{1}{9}\cdot 452361-\frac{1}{30}\cdot 425361+\frac{1}{90}\cdot 342615$$
$$-\frac{1}{90}\cdot 452613-\frac{1}{30}\cdot 452631+\frac{1}{18}\cdot 435126+\frac{1}{45}\cdot 453126-\frac{1}{90}\cdot 524136-\frac{1}{45}\cdot 534126$$
$$-\frac{1}{90}\cdot 531426-\frac{1}{30}\cdot 345162+\frac{1}{90}\cdot 354162+\frac{1}{90}\cdot 435162+\frac{1}{30}\cdot 453162+\frac{1}{90}\cdot 534162$$
$$-\frac{1}{9}\cdot 634125-\frac{1}{30}\cdot 631425-\frac{1}{30}\cdot 346152-\frac{1}{45}\cdot 364152-\frac{1}{30}\cdot 634152-\frac{8}{45}\cdot 345612$$
$$-\frac{8}{45}\cdot 345621-\frac{4}{45}\cdot 346512-\frac{4}{45}\cdot 346521-\frac{1}{15}\cdot 356124-\frac{1}{18}\cdot 356214-\frac{1}{18}\cdot 362451$$

$$- \frac{1}{45} \cdot 354612 - \frac{1}{15} \cdot 354621 + \frac{1}{90} \cdot 356412 - \frac{1}{90} \cdot 356421 + \frac{1}{90} \cdot 364512 - \frac{1}{90} \cdot 364521$$
$$+ \frac{1}{90} \cdot 425613 - \frac{1}{18} \cdot 425631 + \frac{1}{90} \cdot 426351 - \frac{8}{45} \cdot 623451 - \frac{4}{45} \cdot 623541 - \frac{2}{45} \cdot 524613$$
$$- \frac{1}{15} \cdot 624351 - \frac{1}{90} \cdot 624531 - \frac{1}{90} \cdot 625341 - \frac{1}{30} \cdot 345261 - \frac{1}{30} \cdot 435261 - \frac{4}{45} \cdot 435621$$
$$- \frac{1}{30} \cdot 346251 - \frac{1}{30} \cdot 523461 - \frac{1}{30} \cdot 532461 - \frac{1}{30} \cdot 523641 - \frac{4}{45} \cdot 632451 + \frac{2}{45} \cdot 361524$$
$$- \frac{1}{18} \cdot 365124 - \frac{2}{45} \cdot 365214 - \frac{1}{45} \cdot 361542 - \frac{1}{30} \cdot 362541 - \frac{1}{30} \cdot 356142 - \frac{1}{30} \cdot 356241$$
$$- \frac{2}{45} \cdot 365142 - \frac{1}{45} \cdot 365241 + \frac{1}{18} \cdot 426135 + \frac{1}{45} \cdot 426153 + \frac{1}{90} \cdot 526134 - \frac{1}{18} \cdot 625134$$
$$- \frac{1}{30} \cdot 623514 - \frac{1}{30} \cdot 625143 - \frac{1}{30} \cdot 624513 - \frac{1}{45} \cdot 625413 - \frac{2}{45} \cdot 431256 + \frac{11}{90} \cdot 436125$$
$$+ \frac{7}{90} \cdot 451236 + \frac{1}{90} \cdot 451263 - \frac{1}{30} \cdot 461235 + \frac{1}{90} \cdot 461325 + \frac{1}{90} \cdot 462135 + \frac{1}{90} \cdot 462315$$
$$+ \frac{1}{30} \cdot 463125 - \frac{1}{30} \cdot 461253 - \frac{1}{45} \cdot 461352 - \frac{1}{30} \cdot 462351 + \frac{1}{90} \cdot 531264 - \frac{1}{90} \cdot 536124$$
$$+ \frac{1}{90} \cdot 631524 - \frac{1}{30} \cdot 635124 + \frac{1}{90} \cdot 531462 + \frac{1}{9} \cdot 541236 + \frac{1}{45} \cdot 541263 + \frac{2}{45} \cdot 541326$$
$$- \frac{1}{90} \cdot 541362 - \frac{1}{30} \cdot 526341 - \frac{1}{45} \cdot 526431 - \frac{1}{30} \cdot 426531 - \frac{1}{15} \cdot 451623 - \frac{1}{18} \cdot 451632$$
$$- \frac{1}{18} \cdot 541623 - \frac{2}{45} \cdot 541632 - \frac{1}{18} \cdot 631452 - \frac{1}{30} \cdot 641253 - \frac{1}{30} \cdot 461523 - \frac{2}{45} \cdot 461532$$
$$- \frac{1}{30} \cdot 641523 - \frac{1}{45} \cdot 641532 - \frac{1}{30} \cdot 631542 - \frac{4}{45} \cdot 154326 - \frac{1}{45} \cdot 154362 - \frac{1}{45} \cdot 164325$$
$$- \frac{8}{45} \cdot 432156 - \frac{1}{45} \cdot 435216 - \frac{8}{45} \cdot 432165 - \frac{1}{30} \cdot 432615 - \frac{1}{45} \cdot 436215 + \frac{1}{30} \cdot 453216$$
$$+ \frac{1}{90} \cdot 453261 + \frac{1}{90} \cdot 354261 + \frac{2}{45} \cdot 432651 + \frac{7}{90} \cdot 436152 - \frac{1}{90} \cdot 436251 + \frac{7}{90} \cdot 462153$$
$$+ \frac{2}{45} \cdot 463152 - \frac{1}{90} \cdot 534216 - \frac{1}{30} \cdot 532164 - \frac{1}{45} \cdot 532614 - \frac{1}{30} \cdot 632415 + \frac{1}{90} \cdot 634215$$
$$+ \frac{1}{90} \cdot 624315 + \frac{2}{45} \cdot 632154 - \frac{1}{90} \cdot 632514 - \frac{1}{45} \cdot 542136 - \frac{1}{45} \cdot 542163 - \frac{1}{90} \cdot 542316$$
$$+ \frac{1}{90} \cdot 542361 + \frac{1}{90} \cdot 524361 - \frac{1}{90} \cdot 532641 + \frac{1}{30} \cdot 543126 - \frac{1}{30} \cdot 642135 + \frac{1}{90} \cdot 643125$$
$$+ \frac{1}{90} \cdot 641325 - \frac{1}{90} \cdot 642153 + \frac{1}{30} \cdot 154623 + \frac{1}{30} \cdot 156324 - \frac{1}{45} \cdot 156342 - \frac{1}{45} \cdot 156423$$
$$- \frac{1}{45} \cdot 164523 + \frac{2}{45} \cdot 436512 + \frac{1}{90} \cdot 453612 - \frac{1}{45} \cdot 351624 - \frac{1}{5} \cdot 456123 - \frac{1}{10} \cdot 456132$$
$$- \frac{1}{30} \cdot 456213 + \frac{1}{30} \cdot 456231 + \frac{1}{30} \cdot 456312 + \frac{1}{45} \cdot 463512 - \frac{1}{10} \cdot 465123 - \frac{2}{45} \cdot 465132$$
$$- \frac{1}{45} \cdot 465213 + \frac{1}{45} \cdot 465231 + \frac{1}{45} \cdot 465312 + \frac{1}{90} \cdot 534612 + \frac{1}{45} \cdot 536412 + \frac{1}{30} \cdot 634512$$
$$+ \frac{1}{45} \cdot 635412 - \frac{1}{45} \cdot 561324 + \frac{1}{90} \cdot 561342 + \frac{1}{90} \cdot 561423 + \frac{2}{45} \cdot 562143 + \frac{1}{90} \cdot 562314$$
$$+ \frac{1}{30} \cdot 562341 + \frac{1}{45} \cdot 562413 + \frac{1}{45} \cdot 562431 + \frac{1}{90} \cdot 563124 + \frac{1}{45} \cdot 563142 - \frac{1}{30} \cdot 546123$$
$$+ \frac{1}{30} \cdot 564123 + \frac{1}{30} \cdot 645123 - \frac{1}{45} \cdot 546132 + \frac{1}{45} \cdot 564132 + \frac{1}{45} \cdot 645132 - \frac{1}{45} \cdot 154632$$
$$- \frac{1}{30} \cdot 156432 - \frac{1}{30} \cdot 164532 - \frac{2}{45} \cdot 436521 + \frac{1}{30} \cdot 453621 + \frac{1}{10} \cdot 456321 + \frac{1}{45} \cdot 463521$$

$$+\frac{1}{15}\cdot 465321-\frac{1}{90}\cdot 534261+\frac{1}{30}\cdot 534621+\frac{1}{45}\cdot 536241+\frac{1}{45}\cdot 536421+\frac{1}{30}\cdot 634251$$
$$+\frac{1}{10}\cdot 634521+\frac{1}{45}\cdot 635241+\frac{1}{15}\cdot 635421-\frac{8}{45}\cdot 561234-\frac{4}{45}\cdot 561243-\frac{8}{45}\cdot 651234$$
$$-\frac{4}{45}\cdot 651243-\frac{1}{15}\cdot 651324-\frac{1}{90}\cdot 651342-\frac{1}{90}\cdot 651423-\frac{1}{30}\cdot 623415-\frac{1}{30}\cdot 641235$$
$$-\frac{4}{45}\cdot 652134-\frac{1}{45}\cdot 164352-\frac{1}{30}\cdot 165342-\frac{2}{45}\cdot 632541-\frac{1}{90}\cdot 642315+\frac{1}{30}\cdot 642351$$
$$+\frac{1}{45}\cdot 642513+\frac{1}{45}\cdot 642531+\frac{1}{30}\cdot 652314+\frac{1}{10}\cdot 652341+\frac{1}{45}\cdot 652413+\frac{1}{15}\cdot 652431$$
$$-\frac{1}{45}\cdot 165324-\frac{1}{30}\cdot 165423-\frac{2}{45}\cdot 652143+\frac{1}{30}\cdot 653124+\frac{1}{45}\cdot 653142+\frac{1}{10}\cdot 654123$$
$$+\frac{1}{15}\cdot 654132$$

$$[\![x_1\times x_5]\!]=\frac{1}{90}\cdot 124536-\frac{1}{45}\cdot 124563-\frac{1}{30}\cdot 125346-\frac{1}{45}\cdot 126345+\frac{1}{45}\cdot 132456-\frac{1}{45}\cdot 132465$$
$$+\frac{1}{90}\cdot 132564+\frac{1}{90}\cdot 132645-\frac{1}{90}\cdot 142356-\frac{1}{18}\cdot 142365-\frac{1}{90}\cdot 142635+\frac{1}{45}\cdot 152346$$
$$+\frac{1}{30}\cdot 152364-\frac{1}{90}\cdot 152634+\frac{1}{30}\cdot 134256-\frac{1}{45}\cdot 134526+\frac{2}{45}\cdot 134562+\frac{1}{90}\cdot 142563$$
$$+\frac{1}{18}\cdot 152436+\frac{1}{45}\cdot 152463+\frac{2}{45}\cdot 162345+\frac{1}{90}\cdot 162354+\frac{1}{90}\cdot 162435-\frac{1}{45}\cdot 162453$$
$$-\frac{2}{45}\cdot 162534+\frac{4}{45}\cdot 213456+\frac{1}{45}\cdot 213546-\frac{1}{90}\cdot 213564-\frac{1}{90}\cdot 213645+\frac{1}{90}\cdot 231456$$
$$+\frac{1}{90}\cdot 243156-\frac{1}{90}\cdot 243516+\frac{1}{90}\cdot 243561-\frac{1}{45}\cdot 253146-\frac{1}{15}\cdot 253416-\frac{1}{45}\cdot 253461$$
$$-\frac{2}{45}\cdot 263145+\frac{1}{90}\cdot 312456-\frac{1}{45}\cdot 314256-\frac{1}{30}\cdot 314526+\frac{1}{30}\cdot 314562+\frac{1}{90}\cdot 315246$$
$$-\frac{1}{45}\cdot 316245+\frac{1}{18}\cdot 415236+\frac{1}{45}\cdot 416235+\frac{1}{90}\cdot 516234-\frac{1}{30}\cdot 324156-\frac{1}{90}\cdot 324516$$
$$+\frac{1}{18}\cdot 324561-\frac{1}{90}\cdot 413256-\frac{1}{90}\cdot 513246-\frac{1}{45}\cdot 514236+\frac{1}{90}\cdot 613245-\frac{1}{45}\cdot 614235$$
$$-\frac{1}{90}\cdot 421356+\frac{1}{90}\cdot 521346+\frac{1}{18}\cdot 621345-\frac{4}{45}\cdot 123465-\frac{1}{90}\cdot 123564+\frac{1}{45}\cdot 125364$$
$$-\frac{1}{90}\cdot 134265-\frac{1}{90}\cdot 135264-\frac{1}{18}\cdot 145263-\frac{1}{90}\cdot 123645-\frac{1}{45}\cdot 123546+\frac{1}{90}\cdot 125463$$
$$+\frac{1}{90}\cdot 135462+\frac{1}{90}\cdot 143562+\frac{1}{45}\cdot 145362+\frac{1}{45}\cdot 234156+\frac{1}{18}\cdot 214536+\frac{1}{90}\cdot 215346$$
$$-\frac{1}{90}\cdot 312546+\frac{1}{45}\cdot 412356-\frac{1}{90}\cdot 412536-\frac{2}{45}\cdot 234516-\frac{1}{18}\cdot 234651-\frac{1}{45}\cdot 236451$$
$$-\frac{1}{45}\cdot 413526-\frac{2}{45}\cdot 512346-\frac{1}{90}\cdot 512436+\frac{1}{90}\cdot 341562-\frac{1}{90}\cdot 345162-\frac{1}{30}\cdot 512364$$
$$-\frac{1}{90}\cdot 512634+\frac{1}{45}\cdot 342561-\frac{1}{18}\cdot 612354-\frac{1}{45}\cdot 612534+\frac{1}{45}\cdot 623145+\frac{1}{30}\cdot 126354$$
$$+\frac{1}{90}\cdot 231465-\frac{1}{90}\cdot 135426+\frac{1}{45}\cdot 136425+\frac{1}{90}\cdot 235416-\frac{1}{90}\cdot 235461+\frac{2}{45}\cdot 236415$$
$$+\frac{1}{90}\cdot 241536-\frac{1}{45}\cdot 241563+\frac{1}{90}\cdot 341526+\frac{1}{45}\cdot 412635-\frac{1}{18}\cdot 143526+\frac{2}{45}\cdot 342516$$
$$-\frac{1}{90}\cdot 612435+\frac{1}{90}\cdot 153246-\frac{1}{90}\cdot 163245+\frac{1}{90}\cdot 312465-\frac{1}{90}\cdot 231546+\frac{1}{45}\cdot 423516$$

$$+\frac{1}{90}\cdot 124653-\frac{1}{90}\cdot 134652+\frac{1}{45}\cdot 235164-\frac{1}{45}\cdot 245163+\frac{1}{45}\cdot 245361-\frac{1}{90}\cdot 126435$$
$$+\frac{1}{15}\cdot 163425+\frac{1}{45}\cdot 613425+\frac{1}{45}\cdot 124635+\frac{2}{45}\cdot 132654-\frac{1}{90}\cdot 152643-\frac{1}{90}\cdot 134625$$
$$-\frac{1}{45}\cdot 162543-\frac{1}{45}\cdot 213654+\frac{1}{18}\cdot 243165+\frac{2}{45}\cdot 243615+\frac{1}{90}\cdot 253164+\frac{1}{45}\cdot 253614$$
$$+\frac{1}{90}\cdot 253641-\frac{1}{30}\cdot 263154+\frac{1}{90}\cdot 263514+\frac{2}{45}\cdot 263541-\frac{1}{45}\cdot 314265+\frac{1}{45}\cdot 314652$$
$$-\frac{1}{90}\cdot 316254-\frac{1}{18}\cdot 416253-\frac{1}{90}\cdot 516243-\frac{1}{30}\cdot 324165+\frac{1}{30}\cdot 413265+\frac{1}{90}\cdot 514263$$
$$+\frac{1}{90}\cdot 614253+\frac{2}{45}\cdot 615243-\frac{1}{90}\cdot 421365-\frac{1}{45}\cdot 521364+\frac{1}{45}\cdot 143265+\frac{1}{45}\cdot 153264$$
$$-\frac{1}{30}\cdot 154263-\frac{1}{45}\cdot 154362-\frac{1}{30}\cdot 136245-\frac{1}{45}\cdot 241356-\frac{1}{45}\cdot 215436-\frac{1}{45}\cdot 315426$$
$$+\frac{1}{30}\cdot 415326+\frac{1}{30}\cdot 235146+\frac{1}{90}\cdot 246351+\frac{1}{45}\cdot 514326+\frac{1}{45}\cdot 351462+\frac{1}{90}\cdot 354162$$
$$-\frac{1}{45}\cdot 513624-\frac{1}{90}\cdot 516324-\frac{1}{90}\cdot 352461+\frac{1}{90}\cdot 613524-\frac{1}{90}\cdot 624135+\frac{1}{90}\cdot 156243$$
$$+\frac{1}{45}\cdot 126453-\frac{1}{90}\cdot 135624-\frac{1}{45}\cdot 143625+\frac{1}{45}\cdot 145326+\frac{1}{18}\cdot 146325-\frac{1}{30}\cdot 156324$$
$$+\frac{1}{90}\cdot 153642-\frac{1}{90}\cdot 136524+\frac{1}{30}\cdot 145623-\frac{1}{90}\cdot 146523-\frac{1}{90}\cdot 154623-\frac{1}{45}\cdot 156423$$
$$+\frac{1}{90}\cdot 163524+\frac{1}{45}\cdot 214635-\frac{1}{30}\cdot 245136+\frac{1}{45}\cdot 251634+\frac{2}{45}\cdot 256134+\frac{1}{45}\cdot 215364$$
$$-\frac{1}{30}\cdot 235614-\frac{1}{45}\cdot 245631-\frac{1}{45}\cdot 254631+\frac{1}{90}\cdot 256431+\frac{1}{90}\cdot 264531-\frac{1}{90}\cdot 315642$$
$$+\frac{1}{90}\cdot 351642-\frac{1}{30}\cdot 356142-\frac{1}{90}\cdot 316452+\frac{1}{90}\cdot 413652-\frac{1}{90}\cdot 415362-\frac{1}{45}\cdot 416352$$
$$+\frac{1}{90}\cdot 513642+\frac{2}{45}\cdot 516342+\frac{1}{30}\cdot 325641-\frac{1}{45}\cdot 356241-\frac{1}{18}\cdot 415632+\frac{1}{45}\cdot 514632$$
$$-\frac{1}{45}\cdot 613452-\frac{1}{45}\cdot 614352+\frac{1}{90}\cdot 614532+\frac{1}{90}\cdot 615342-\frac{1}{90}\cdot 421563+\frac{1}{18}\cdot 425163$$
$$+\frac{2}{45}\cdot 425613-\frac{1}{90}\cdot 521463+\frac{1}{45}\cdot 524163+\frac{1}{90}\cdot 524613+\frac{1}{30}\cdot 621453-\frac{1}{45}\cdot 624513$$
$$+\frac{1}{90}\cdot 214653-\frac{1}{30}\cdot 215463+\frac{1}{90}\cdot 325164+\frac{1}{45}\cdot 146532-\frac{1}{90}\cdot 246513+\frac{1}{45}\cdot 251643$$
$$-\frac{1}{45}\cdot 154632+\frac{1}{90}\cdot 254613-\frac{1}{30}\cdot 352614+\frac{1}{45}\cdot 163542+\frac{1}{90}\cdot 164253-\frac{2}{45}\cdot 164352$$
$$+\frac{1}{45}\cdot 264153-\frac{2}{45}\cdot 136254+\frac{1}{30}\cdot 146235-\frac{1}{45}\cdot 146253-\frac{1}{45}\cdot 154236+\frac{1}{90}\cdot 146352$$
$$+\frac{1}{30}\cdot 156234+\frac{1}{45}\cdot 164235+\frac{1}{45}\cdot 415623-\frac{1}{90}\cdot 265134-\frac{1}{45}\cdot 265314-\frac{1}{90}\cdot 265341$$
$$-\frac{1}{30}\cdot 413625+\frac{1}{90}\cdot 514623-\frac{1}{90}\cdot 316425+\frac{1}{45}\cdot 516423+\frac{1}{90}\cdot 326145+\frac{1}{30}\cdot 326415$$
$$+\frac{1}{90}\cdot 326451-\frac{1}{90}\cdot 615423+\frac{1}{90}\cdot 621534+\frac{1}{30}\cdot 216354-\frac{1}{18}\cdot 216435-\frac{2}{45}\cdot 261435$$
$$-\frac{1}{45}\cdot 361425-\frac{1}{90}\cdot 362415+\frac{1}{30}\cdot 364152+\frac{2}{45}\cdot 165243-\frac{2}{45}\cdot 165324-\frac{1}{30}\cdot 256314$$
$$-\frac{1}{30}\cdot 526314+\frac{4}{45}\cdot 126543-\frac{1}{30}\cdot 156432-\frac{1}{90}\cdot 164532-\frac{2}{45}\cdot 215643+\frac{1}{18}\cdot 231654$$
$$+\frac{1}{90}\cdot 265143+\frac{1}{90}\cdot 265413+\frac{2}{45}\cdot 265431+\frac{1}{18}\cdot 312654+\frac{1}{90}\cdot 412653-\frac{1}{90}\cdot 512643$$

$$+\frac{1}{45}\cdot 316524+\frac{1}{90}\cdot 316542+\frac{1}{30}\cdot 516432+\frac{1}{90}\cdot 326541+\frac{2}{45}\cdot 615432+\frac{1}{90}\cdot 621543$$
$$-\frac{1}{90}\cdot 165342-\frac{1}{30}\cdot 165423-\frac{2}{45}\cdot 216534+\frac{1}{45}\cdot 251436-\frac{1}{18}\cdot 254136-\frac{1}{90}\cdot 261534$$
$$-\frac{1}{90}\cdot 264135-\frac{1}{90}\cdot 236154-\frac{1}{90}\cdot 236514-\frac{2}{45}\cdot 365142-\frac{1}{90}\cdot 416532-\frac{1}{90}\cdot 362541$$
$$-\frac{1}{30}\cdot 365241-\frac{1}{45}\cdot 521643-\frac{1}{15}\cdot 526143-\frac{1}{45}\cdot 526413-\frac{1}{90}\cdot 625143-\frac{1}{30}\cdot 625413$$
$$+\frac{1}{45}\cdot 321465-\frac{2}{45}\cdot 321546+\frac{1}{90}\cdot 431526+\frac{1}{45}\cdot 432516+\frac{1}{90}\cdot 251346+\frac{1}{90}\cdot 435162$$
$$-\frac{1}{90}\cdot 425361-\frac{2}{45}\cdot 435261-\frac{1}{90}\cdot 631425-\frac{2}{45}\cdot 632415-\frac{1}{45}\cdot 241365-\frac{1}{45}\cdot 216453$$
$$-\frac{1}{90}\cdot 241653-\frac{1}{18}\cdot 321645+\frac{2}{45}\cdot 325146-\frac{1}{45}\cdot 341625+\frac{2}{45}\cdot 342165+\frac{1}{90}\cdot 342615$$
$$+\frac{1}{90}\cdot 421635+\frac{1}{45}\cdot 423165+\frac{1}{45}\cdot 431652+\frac{1}{15}\cdot 436152-\frac{1}{30}\cdot 423651-\frac{1}{90}\cdot 432651$$
$$+\frac{1}{90}\cdot 436251+\frac{1}{90}\cdot 531264-\frac{1}{90}\cdot 531624-\frac{1}{90}\cdot 532164-\frac{1}{30}\cdot 631254-\frac{1}{90}\cdot 632154$$
$$+\frac{1}{90}\cdot 632514-\frac{1}{18}\cdot 321564+\frac{1}{30}\cdot 251463+\frac{2}{45}\cdot 431265-\frac{1}{45}\cdot 431625-\frac{1}{90}\cdot 432615$$
$$+\frac{1}{90}\cdot 261543-\frac{1}{45}\cdot 245316+\frac{1}{30}\cdot 354126+\frac{2}{45}\cdot 354216+\frac{1}{30}\cdot 364125+\frac{1}{45}\cdot 364215$$
$$+\frac{1}{45}\cdot 425136-\frac{1}{90}\cdot 425316-\frac{1}{45}\cdot 426315-\frac{1}{90}\cdot 435126-\frac{2}{45}\cdot 435216+\frac{2}{45}\cdot 524316$$
$$-\frac{1}{90}\cdot 531426-\frac{1}{45}\cdot 532416-\frac{1}{45}\cdot 451263+\frac{1}{90}\cdot 451326-\frac{1}{90}\cdot 451362+\frac{1}{90}\cdot 352146$$
$$-\frac{1}{45}\cdot 423156+\frac{1}{90}\cdot 452136-\frac{1}{90}\cdot 342651-\frac{1}{30}\cdot 345126+\frac{1}{45}\cdot 453126-\frac{1}{90}\cdot 524136$$
$$-\frac{1}{45}\cdot 453162+\frac{1}{90}\cdot 523164+\frac{1}{90}\cdot 453261-\frac{1}{90}\cdot 623154+\frac{1}{90}\cdot 346215+\frac{1}{90}\cdot 634215$$
$$+\frac{1}{90}\cdot 245613-\frac{1}{90}\cdot 364512-\frac{1}{30}\cdot 364521-\frac{1}{90}\cdot 425631+\frac{1}{45}\cdot 526341+\frac{2}{45}\cdot 435612$$
$$+\frac{1}{45}\cdot 524361-\frac{1}{30}\cdot 625341-\frac{1}{90}\cdot 531462-\frac{1}{90}\cdot 631452-\frac{1}{90}\cdot 234615-\frac{2}{45}\cdot 346512$$
$$+\frac{1}{45}\cdot 523461-\frac{1}{90}\cdot 451632-\frac{1}{90}\cdot 452613-\frac{1}{45}\cdot 452631+\frac{1}{90}\cdot 523641+\frac{1}{90}\cdot 453612$$
$$+\frac{1}{30}\cdot 453621-\frac{1}{45}\cdot 634152+\frac{1}{30}\cdot 634251+\frac{1}{90}\cdot 246315+\frac{1}{90}\cdot 246153+\frac{1}{90}\cdot 261453$$
$$+\frac{1}{90}\cdot 351246+\frac{1}{30}\cdot 361245+\frac{1}{90}\cdot 362145-\frac{2}{45}\cdot 346125-\frac{1}{90}\cdot 423615-\frac{1}{90}\cdot 426135$$
$$-\frac{2}{45}\cdot 461253-\frac{1}{90}\cdot 461352+\frac{1}{45}\cdot 463152+\frac{1}{45}\cdot 462351+\frac{1}{30}\cdot 463251+\frac{1}{30}\cdot 536124$$
$$+\frac{2}{45}\cdot 536214+\frac{1}{45}\cdot 635124+\frac{1}{30}\cdot 635214-\frac{1}{90}\cdot 352416-\frac{1}{30}\cdot 451236-\frac{2}{45}\cdot 534162$$
$$-\frac{1}{90}\cdot 534261+\frac{1}{18}\cdot 541263-\frac{1}{45}\cdot 541362-\frac{1}{90}\cdot 542361+\frac{1}{45}\cdot 641235+\frac{1}{45}\cdot 641325$$
$$-\frac{1}{90}\cdot 642315-\frac{1}{90}\cdot 643125+\frac{1}{30}\cdot 361524-\frac{1}{90}\cdot 461325+\frac{1}{45}\cdot 541326+\frac{1}{90}\cdot 462135$$
$$-\frac{1}{45}\cdot 542136+\frac{1}{90}\cdot 431562-\frac{1}{90}\cdot 426531+\frac{1}{90}\cdot 532641-\frac{1}{90}\cdot 631542+\frac{1}{90}\cdot 642153$$
$$-\frac{1}{45}\cdot 352164-\frac{4}{45}\cdot 432156+\frac{1}{30}\cdot 453216+\frac{1}{90}\cdot 534216+\frac{1}{90}\cdot 542163-\frac{1}{30}\cdot 543162$$

$$
\begin{aligned}
&-\frac{2}{45}\cdot 543261-\frac{2}{45}\cdot 643215+\frac{1}{90}\cdot 542316+\frac{1}{30}\cdot 543126-\frac{1}{90}\cdot 436215-\frac{1}{90}\cdot 463215\\
&+\frac{1}{90}\cdot 356412-\frac{1}{30}\cdot 465123-\frac{1}{45}\cdot 465132+\frac{1}{90}\cdot 465231+\frac{1}{90}\cdot 465312-\frac{1}{90}\cdot 534612\\
&+\frac{1}{90}\cdot 536241+\frac{1}{30}\cdot 546123+\frac{1}{45}\cdot 546213-\frac{1}{90}\cdot 546231-\frac{1}{90}\cdot 546312+\frac{1}{90}\cdot 635412\\
&+\frac{1}{45}\cdot 641523+\frac{1}{90}\cdot 642513-\frac{1}{90}\cdot 643512-\frac{2}{45}\cdot 561243+\frac{1}{90}\cdot 561342+\frac{1}{90}\cdot 461523\\
&-\frac{1}{90}\cdot 561423+\frac{2}{45}\cdot 562134+\frac{1}{90}\cdot 562314-\frac{1}{90}\cdot 462531+\frac{1}{90}\cdot 562431-\frac{1}{90}\cdot 563124\\
&-\frac{1}{90}\cdot 563241-\frac{1}{30}\cdot 456132+\frac{1}{90}\cdot 564132-\frac{1}{90}\cdot 635142+\frac{1}{90}\cdot 645132+\frac{1}{30}\cdot 456213\\
&-\frac{1}{90}\cdot 564213-\frac{1}{90}\cdot 645213+\frac{1}{90}\cdot 346251-\frac{1}{90}\cdot 356214-\frac{1}{90}\cdot 356421+\frac{1}{30}\cdot 465321\\
&+\frac{1}{90}\cdot 534621+\frac{1}{90}\cdot 526431-\frac{1}{30}\cdot 546321+\frac{1}{30}\cdot 635421+\frac{1}{90}\cdot 641532-\frac{1}{30}\cdot 643521\\
&+\frac{1}{90}\cdot 261345+\frac{1}{90}\cdot 541623-\frac{1}{30}\cdot 651423-\frac{1}{90}\cdot 461235+\frac{1}{90}\cdot 641253+\frac{1}{30}\cdot 652314\\
&+\frac{1}{90}\cdot 623514-\frac{1}{90}\cdot 624531-\frac{1}{90}\cdot 362451+\frac{1}{90}\cdot 642351-\frac{1}{90}\cdot 542631+\frac{1}{30}\cdot 652431\\
&-\frac{1}{30}\cdot 653241-\frac{1}{90}\cdot 651342-\frac{1}{90}\cdot 625134+\frac{1}{90}\cdot 365124+\frac{1}{90}\cdot 653124-\frac{1}{90}\cdot 643152\\
&+\frac{1}{30}\cdot 654132-\frac{1}{30}\cdot 654213
\end{aligned}
$$

$$
\begin{aligned}
[\![x_2\times x_2]\!]=&\frac{2}{15}\cdot 123456+\frac{2}{45}\cdot 123465+\frac{2}{45}\cdot 132456+\frac{2}{45}\cdot 124356-\frac{1}{45}\cdot 125436-\frac{1}{45}\cdot 125463\\
&-\frac{1}{45}\cdot 126435-\frac{2}{45}\cdot 126453-\frac{1}{45}\cdot 135426+\frac{1}{45}\cdot 135462-\frac{1}{45}\cdot 136425-\frac{1}{45}\cdot 136452\\
&-\frac{1}{45}\cdot 152436-\frac{1}{45}\cdot 152463-\frac{2}{45}\cdot 153426-\frac{1}{45}\cdot 153462+\frac{1}{45}\cdot 162435-\frac{1}{45}\cdot 162453\\
&-\frac{1}{45}\cdot 163425-\frac{1}{45}\cdot 163452-\frac{1}{45}\cdot 213564-\frac{1}{45}\cdot 214536-\frac{1}{45}\cdot 214563-\frac{1}{45}\cdot 231546\\
&-\frac{1}{45}\cdot 241536-\frac{1}{45}\cdot 241563-\frac{1}{45}\cdot 213645-\frac{1}{45}\cdot 215346-\frac{1}{45}\cdot 216345-\frac{1}{45}\cdot 312546\\
&-\frac{1}{45}\cdot 315246-\frac{1}{45}\cdot 316245+\frac{2}{45}\cdot 234516+\frac{4}{45}\cdot 234561+\frac{1}{45}\cdot 243516+\frac{2}{45}\cdot 243561\\
&-\frac{1}{45}\cdot 321456-\frac{1}{45}\cdot 324156-\frac{1}{45}\cdot 421356-\frac{2}{45}\cdot 423156+\frac{2}{45}\cdot 512346+\frac{1}{45}\cdot 513246\\
&+\frac{4}{45}\cdot 612345+\frac{2}{45}\cdot 613245+\frac{2}{45}\cdot 123546+\frac{2}{45}\cdot 213456-\frac{1}{45}\cdot 123654-\frac{1}{45}\cdot 124653\\
&-\frac{1}{45}\cdot 126354-\frac{1}{45}\cdot 132564-\frac{1}{45}\cdot 134265-\frac{1}{45}\cdot 135264-\frac{1}{45}\cdot 231465-\frac{1}{45}\cdot 234165\\
&-\frac{1}{45}\cdot 235164-\frac{1}{45}\cdot 132645-\frac{1}{45}\cdot 142365-\frac{1}{45}\cdot 142635-\frac{1}{45}\cdot 312465-\frac{1}{45}\cdot 412365\\
&-\frac{1}{45}\cdot 412635+\frac{2}{45}\cdot 134562+\frac{2}{45}\cdot 235461-\frac{1}{45}\cdot 143256-\frac{1}{45}\cdot 143526-\frac{1}{45}\cdot 153246\\
&-\frac{1}{45}\cdot 243156-\frac{1}{45}\cdot 253146-\frac{1}{45}\cdot 253416-\frac{1}{45}\cdot 413256-\frac{1}{45}\cdot 413526-\frac{1}{45}\cdot 423516\\
&-\frac{1}{45}\cdot 513426-\frac{1}{45}\cdot 523146-\frac{1}{45}\cdot 523416+\frac{2}{45}\cdot 162345+\frac{2}{45}\cdot 612435+\frac{2}{45}\cdot 156423
\end{aligned}
$$

$$
\begin{aligned}
&+\frac{2}{45}\cdot 156432+\frac{2}{45}\cdot 165423+\frac{2}{45}\cdot 165432+\frac{2}{45}\cdot 216534+\frac{4}{45}\cdot 216543+\frac{1}{45}\cdot 261534\\
&+\frac{2}{45}\cdot 261543+\frac{2}{45}\cdot 215643+\frac{1}{45}\cdot 315642+\frac{2}{45}\cdot 316542-\frac{1}{45}\cdot 236514-\frac{1}{45}\cdot 236541\\
&-\frac{1}{45}\cdot 246513-\frac{1}{45}\cdot 246531-\frac{1}{45}\cdot 263514-\frac{1}{45}\cdot 263541-\frac{1}{45}\cdot 264513-\frac{1}{45}\cdot 264531\\
&+\frac{2}{15}\cdot 321654+\frac{2}{45}\cdot 326154+\frac{2}{45}\cdot 421653+\frac{2}{45}\cdot 426153-\frac{1}{45}\cdot 512643-\frac{1}{45}\cdot 513642\\
&-\frac{1}{45}\cdot 516243-\frac{1}{45}\cdot 516342-\frac{1}{45}\cdot 612543-\frac{1}{45}\cdot 613542-\frac{1}{45}\cdot 615243-\frac{1}{45}\cdot 615342\\
&+\frac{2}{45}\cdot 312654+\frac{2}{45}\cdot 321645-\frac{1}{45}\cdot 314625-\frac{1}{45}\cdot 314652-\frac{1}{45}\cdot 315624-\frac{1}{45}\cdot 324615\\
&-\frac{2}{45}\cdot 324651-\frac{1}{45}\cdot 325614-\frac{1}{45}\cdot 325641-\frac{1}{45}\cdot 341625-\frac{1}{45}\cdot 341652+\frac{1}{45}\cdot 342615\\
&-\frac{1}{45}\cdot 342651-\frac{2}{45}\cdot 351624-\frac{1}{45}\cdot 351642-\frac{1}{45}\cdot 352614-\frac{1}{45}\cdot 352641+\frac{2}{45}\cdot 431265\\
&+\frac{4}{45}\cdot 432165+\frac{1}{45}\cdot 531264+\frac{2}{45}\cdot 532164-\frac{2}{45}\cdot 621354-\frac{1}{45}\cdot 621453-\frac{1}{45}\cdot 623154\\
&-\frac{1}{45}\cdot 624153+\frac{2}{45}\cdot 231654+\frac{2}{45}\cdot 321564-\frac{1}{45}\cdot 326451-\frac{1}{45}\cdot 423651-\frac{1}{45}\cdot 426351\\
&+\frac{2}{45}\cdot 342165+\frac{2}{45}\cdot 432615-\frac{1}{45}\cdot 251364-\frac{1}{45}\cdot 251634-\frac{1}{45}\cdot 261354-\frac{1}{45}\cdot 351264\\
&-\frac{1}{45}\cdot 361254-\frac{1}{45}\cdot 361524-\frac{1}{45}\cdot 521364-\frac{1}{45}\cdot 521634-\frac{1}{45}\cdot 531624-\frac{1}{45}\cdot 621534\\
&-\frac{1}{45}\cdot 631254-\frac{1}{45}\cdot 631524+\frac{2}{45}\cdot 345612+\frac{2}{45}\cdot 345621+\frac{2}{45}\cdot 354612+\frac{2}{45}\cdot 354621\\
&-\frac{1}{45}\cdot 431562-\frac{1}{45}\cdot 432561-\frac{1}{45}\cdot 435162-\frac{1}{45}\cdot 435261-\frac{1}{45}\cdot 531462-\frac{1}{45}\cdot 532461\\
&-\frac{1}{45}\cdot 534162-\frac{1}{45}\cdot 534261+\frac{2}{45}\cdot 623451+\frac{2}{45}\cdot 624351+\frac{2}{45}\cdot 453126+\frac{2}{45}\cdot 453216\\
&+\frac{2}{45}\cdot 543126+\frac{2}{45}\cdot 543216-\frac{1}{45}\cdot 362145-\frac{1}{45}\cdot 362415-\frac{1}{45}\cdot 462135-\frac{1}{45}\cdot 462315\\
&-\frac{1}{45}\cdot 632145-\frac{1}{45}\cdot 632415-\frac{1}{45}\cdot 642135-\frac{1}{45}\cdot 642315+\frac{2}{45}\cdot 561234+\frac{2}{45}\cdot 561324\\
&+\frac{2}{45}\cdot 651234+\frac{2}{45}\cdot 651324
\end{aligned}
$$

$$
\begin{aligned}
[\![x_2\times x_3]\!] &= \frac{2}{45}\cdot 123546+\frac{1}{45}\cdot 123645+\frac{2}{45}\cdot 132546+\frac{1}{45}\cdot 132645+\frac{2}{45}\cdot 124536+\frac{2}{45}\cdot 124356\\
&+\frac{2}{45}\cdot 124365+\frac{2}{45}\cdot 134256+\frac{2}{45}\cdot 134265+\frac{2}{45}\cdot 132456-\frac{1}{45}\cdot 124653-\frac{2}{45}\cdot 134562\\
&-\frac{1}{45}\cdot 134652+\frac{1}{45}\cdot 134526-\frac{1}{45}\cdot 152346-\frac{1}{45}\cdot 153246-\frac{2}{45}\cdot 162345-\frac{1}{45}\cdot 163245\\
&+\frac{2}{45}\cdot 213456+\frac{2}{45}\cdot 213465+\frac{1}{45}\cdot 231456+\frac{1}{45}\cdot 231465+\frac{2}{45}\cdot 214356+\frac{2}{45}\cdot 213546\\
&+\frac{1}{45}\cdot 213564+\frac{2}{45}\cdot 214536+\frac{2}{45}\cdot 214563+\frac{1}{45}\cdot 231546-\frac{1}{45}\cdot 231564-\frac{1}{45}\cdot 241563\\
&+\frac{1}{45}\cdot 213645+\frac{2}{45}\cdot 216345-\frac{1}{45}\cdot 231645+\frac{1}{45}\cdot 312546-\frac{1}{45}\cdot 312564-\frac{1}{45}\cdot 312645\\
&+\frac{1}{45}\cdot 316245+\frac{2}{45}\cdot 234165-\frac{1}{9}\cdot 234561-\frac{2}{45}\cdot 234516-\frac{1}{45}\cdot 243516-\frac{1}{45}\cdot 243561
\end{aligned}
$$

$$- \frac{1}{45} \cdot 236145 - \frac{1}{90} \cdot 253146 + \frac{1}{45} \cdot 261345 - \frac{1}{45} \cdot 263145 + \frac{1}{90} \cdot 351246 + \frac{1}{45} \cdot 361245$$
$$- \frac{1}{45} \cdot 235461 - \frac{1}{45} \cdot 236415 - \frac{1}{45} \cdot 236451 - \frac{1}{90} \cdot 253416 - \frac{1}{45} \cdot 253461 - \frac{1}{45} \cdot 263415$$
$$- \frac{1}{30} \cdot 263451 + \frac{2}{45} \cdot 412365 - \frac{1}{45} \cdot 413256 - \frac{1}{45} \cdot 412563 - \frac{1}{90} \cdot 413526 - \frac{1}{45} \cdot 413562$$
$$+ \frac{1}{45} \cdot 412635 + \frac{1}{90} \cdot 415236 + \frac{1}{45} \cdot 416235 + \frac{1}{45} \cdot 512634 - \frac{1}{90} \cdot 516234 - \frac{1}{45} \cdot 324516$$
$$- \frac{1}{90} \cdot 423516 - \frac{1}{45} \cdot 423561 - \frac{1}{9} \cdot 612345 - \frac{2}{45} \cdot 512346 - \frac{1}{45} \cdot 513246 - \frac{1}{45} \cdot 613245$$
$$- \frac{1}{45} \cdot 512436 - \frac{1}{30} \cdot 514236 - \frac{1}{45} \cdot 612435 - \frac{1}{45} \cdot 612534 - \frac{1}{45} \cdot 614235 - \frac{1}{30} \cdot 615234$$
$$- \frac{1}{90} \cdot 531246 - \frac{1}{45} \cdot 631245 + \frac{2}{45} \cdot 123465 + \frac{1}{45} \cdot 123564 - \frac{1}{45} \cdot 126435 + \frac{1}{45} \cdot 312456$$
$$+ \frac{2}{45} \cdot 132465 + \frac{1}{45} \cdot 132564 - \frac{1}{45} \cdot 235164 + \frac{1}{45} \cdot 312465 - \frac{1}{45} \cdot 324156 - \frac{1}{45} \cdot 135462$$
$$- \frac{1}{90} \cdot 136425 + \frac{1}{90} \cdot 146235 - \frac{1}{90} \cdot 461235 - \frac{1}{90} \cdot 136452 - \frac{1}{45} \cdot 152436 - \frac{1}{90} \cdot 152463$$
$$+ \frac{1}{45} \cdot 512364 - \frac{1}{45} \cdot 512463 + \frac{1}{90} \cdot 152634 - \frac{1}{90} \cdot 153462 - \frac{1}{45} \cdot 513462 - \frac{1}{30} \cdot 523461$$
$$- \frac{1}{45} \cdot 162435 - \frac{1}{90} \cdot 162534 - \frac{1}{30} \cdot 164235 - \frac{1}{30} \cdot 641235 - \frac{1}{45} \cdot 125643 - \frac{2}{45} \cdot 126543$$
$$- \frac{1}{90} \cdot 135642 - \frac{1}{30} \cdot 136542 - \frac{1}{45} \cdot 126534 - \frac{2}{45} \cdot 154236 - \frac{2}{45} \cdot 154326 - \frac{1}{30} \cdot 164325$$
$$- \frac{2}{45} \cdot 132654 - \frac{1}{45} \cdot 136254 + \frac{1}{45} \cdot 154623 + \frac{1}{45} \cdot 154632 + \frac{1}{45} \cdot 164523 + \frac{1}{45} \cdot 164532$$
$$- \frac{1}{90} \cdot 136524 + \frac{1}{45} \cdot 156243 + \frac{1}{45} \cdot 156342 + \frac{1}{45} \cdot 165243 + \frac{1}{45} \cdot 165342 - \frac{1}{90} \cdot 152643$$
$$- \frac{1}{90} \cdot 162543 - \frac{2}{45} \cdot 215436 - \frac{1}{45} \cdot 216435 - \frac{1}{45} \cdot 251436 - \frac{1}{90} \cdot 251463 + \frac{1}{45} \cdot 261435$$
$$+ \frac{1}{30} \cdot 261453 - \frac{2}{45} \cdot 213654 - \frac{1}{45} \cdot 214653 + \frac{1}{45} \cdot 314652 + \frac{1}{90} \cdot 316452 - \frac{1}{45} \cdot 216534$$
$$- \frac{4}{45} \cdot 216543 + \frac{1}{90} \cdot 261534 - \frac{1}{90} \cdot 261543 - \frac{1}{45} \cdot 215643 + \frac{1}{90} \cdot 315642 - \frac{1}{90} \cdot 316542$$
$$- \frac{1}{90} \cdot 254136 - \frac{1}{45} \cdot 254163 - \frac{1}{90} \cdot 254316 - \frac{1}{90} \cdot 264135 - \frac{1}{45} \cdot 264315 - \frac{4}{45} \cdot 231654$$
$$- \frac{1}{45} \cdot 236154 + \frac{1}{45} \cdot 254361 + \frac{1}{90} \cdot 254613 + \frac{1}{90} \cdot 254631 - \frac{1}{90} \cdot 264351 + \frac{1}{45} \cdot 264513$$
$$+ \frac{1}{45} \cdot 264531 + \frac{1}{45} \cdot 236514 + \frac{1}{45} \cdot 236541 + \frac{1}{90} \cdot 246513 + \frac{1}{90} \cdot 246531 + \frac{1}{90} \cdot 263514$$
$$+ \frac{1}{90} \cdot 263541 + \frac{1}{45} \cdot 256143 + \frac{1}{45} \cdot 265143 - \frac{1}{90} \cdot 251643 + \frac{1}{90} \cdot 351642 + \frac{1}{45} \cdot 256413$$
$$+ \frac{1}{45} \cdot 256431 + \frac{1}{45} \cdot 265413 + \frac{1}{45} \cdot 265431 - \frac{1}{90} \cdot 415326 - \frac{1}{90} \cdot 415362 - \frac{1}{45} \cdot 416325$$
$$- \frac{1}{30} \cdot 514326 - \frac{1}{45} \cdot 514362 - \frac{4}{45} \cdot 312654 + \frac{1}{90} \cdot 416253 + \frac{1}{45} \cdot 416523 - \frac{1}{45} \cdot 415632$$
$$+ \frac{2}{45} \cdot 326514 + \frac{2}{45} \cdot 326541 + \frac{1}{90} \cdot 426513 + \frac{1}{90} \cdot 426531 - \frac{1}{90} \cdot 516324 + \frac{1}{45} \cdot 516342$$
$$+ \frac{1}{45} \cdot 614325 + \frac{1}{90} \cdot 614352 - \frac{1}{90} \cdot 615324 + \frac{1}{45} \cdot 615342 + \frac{1}{45} \cdot 512643 + \frac{1}{90} \cdot 513642$$
$$+ \frac{1}{90} \cdot 516243 + \frac{1}{45} \cdot 612543 + \frac{1}{90} \cdot 613542 + \frac{1}{90} \cdot 615243 + \frac{1}{45} \cdot 614532 + \frac{1}{45} \cdot 615432$$

$$+ \frac{1}{45} \cdot 521643 + \frac{1}{45} \cdot 531642 + \frac{2}{45} \cdot 621543 + \frac{1}{90} \cdot 631542 - \frac{2}{45} \cdot 241653 - \frac{1}{90} \cdot 246153$$
$$- \frac{2}{45} \cdot 143265 + \frac{2}{45} \cdot 215634 - \frac{1}{45} \cdot 142653 - \frac{1}{45} \cdot 143625 - \frac{1}{45} \cdot 143652 - \frac{1}{45} \cdot 241635$$
$$+ \frac{2}{45} \cdot 261354 - \frac{1}{45} \cdot 163254 - \frac{2}{45} \cdot 321546 - \frac{4}{45} \cdot 321564 - \frac{2}{45} \cdot 321465 - \frac{1}{45} \cdot 324165$$
$$- \frac{2}{45} \cdot 325164 - \frac{1}{45} \cdot 421563 - \frac{1}{90} \cdot 425163 - \frac{4}{45} \cdot 321645 - \frac{1}{5} \cdot 321654 - \frac{2}{45} \cdot 326154$$
$$- \frac{2}{45} \cdot 421653 - \frac{1}{45} \cdot 426153 - \frac{1}{45} \cdot 315264 - \frac{1}{45} \cdot 315426 - \frac{1}{45} \cdot 325146 - \frac{1}{45} \cdot 325416$$
$$+ \frac{2}{45} \cdot 341265 - \frac{1}{45} \cdot 342165 + \frac{1}{45} \cdot 315462 + \frac{1}{18} \cdot 315624 + \frac{2}{45} \cdot 325461 + \frac{1}{15} \cdot 325614$$
$$+ \frac{1}{15} \cdot 325641 + \frac{1}{45} \cdot 314625 + \frac{1}{45} \cdot 324615 + \frac{1}{15} \cdot 324651 + \frac{1}{18} \cdot 341625 + \frac{1}{15} \cdot 341652$$
$$+ \frac{1}{90} \cdot 342615 + \frac{1}{15} \cdot 342651 + \frac{2}{45} \cdot 351624 + \frac{1}{90} \cdot 352614 + \frac{1}{45} \cdot 352641 + \frac{1}{45} \cdot 243615$$
$$+ \frac{2}{45} \cdot 243651 + \frac{1}{15} \cdot 361254 + \frac{1}{45} \cdot 362154 - \frac{1}{90} \cdot 462153 + \frac{1}{30} \cdot 316524 + \frac{1}{30} \cdot 361524$$
$$+ \frac{1}{45} \cdot 362514 + \frac{1}{90} \cdot 362541 - \frac{1}{45} \cdot 521436 + \frac{2}{45} \cdot 521364 + \frac{1}{30} \cdot 523164 + \frac{1}{15} \cdot 521634$$
$$- \frac{1}{90} \cdot 526143 + \frac{1}{30} \cdot 431625 + \frac{2}{45} \cdot 431652 - \frac{1}{90} \cdot 432615 + \frac{2}{45} \cdot 432651 + \frac{1}{30} \cdot 531624$$
$$+ \frac{1}{90} \cdot 532641 + \frac{2}{45} \cdot 621435 + \frac{1}{15} \cdot 621453 + \frac{1}{15} \cdot 621354 + \frac{1}{15} \cdot 623154 + \frac{1}{45} \cdot 624153$$
$$+ \frac{2}{45} \cdot 613254 + \frac{1}{90} \cdot 625143 + \frac{2}{45} \cdot 632154 + \frac{1}{90} \cdot 642153 - \frac{1}{90} \cdot 316425 - \frac{1}{45} \cdot 413265$$
$$- \frac{1}{90} \cdot 413625 - \frac{1}{45} \cdot 153264 + \frac{1}{90} \cdot 423615 + \frac{2}{45} \cdot 326451 + \frac{2}{45} \cdot 423651 + \frac{1}{45} \cdot 426351$$
$$- \frac{1}{45} \cdot 421536 - \frac{1}{45} \cdot 431265 + \frac{1}{30} \cdot 251634 + \frac{2}{45} \cdot 621534 + \frac{1}{45} \cdot 251364 + \frac{1}{30} \cdot 351264$$
$$+ \frac{1}{90} \cdot 531264 + \frac{2}{45} \cdot 631254 + \frac{1}{45} \cdot 631524 + \frac{1}{45} \cdot 513264 - \frac{1}{90} \cdot 532164 + \frac{1}{90} \cdot 135624$$
$$+ \frac{1}{90} \cdot 245136 + \frac{1}{90} \cdot 245316 + \frac{1}{45} \cdot 245361 + \frac{1}{90} \cdot 145263 + \frac{1}{90} \cdot 145362 - \frac{1}{45} \cdot 245163$$
$$- \frac{1}{90} \cdot 245613 - \frac{1}{90} \cdot 245631 + \frac{1}{45} \cdot 145623 + \frac{1}{45} \cdot 145632 + \frac{1}{45} \cdot 163452 + \frac{1}{90} \cdot 341526$$
$$- \frac{1}{90} \cdot 342516 + \frac{1}{45} \cdot 345126 + \frac{1}{45} \cdot 345216 - \frac{1}{90} \cdot 345162 - \frac{1}{90} \cdot 345261 - \frac{4}{45} \cdot 345612$$
$$- \frac{4}{45} \cdot 345621 - \frac{2}{45} \cdot 354612 - \frac{2}{45} \cdot 354621 - \frac{1}{90} \cdot 346152 - \frac{1}{90} \cdot 346251 - \frac{1}{45} \cdot 361452$$
$$- \frac{1}{90} \cdot 362451 - \frac{1}{90} \cdot 364152 - \frac{1}{90} \cdot 364251 - \frac{1}{45} \cdot 346512 - \frac{1}{45} \cdot 346521 - \frac{1}{45} \cdot 364512$$
$$- \frac{1}{45} \cdot 364521 + \frac{1}{45} \cdot 523416 - \frac{1}{90} \cdot 524361 - \frac{1}{90} \cdot 425613 - \frac{1}{90} \cdot 425631 - \frac{1}{45} \cdot 523614$$
$$- \frac{1}{90} \cdot 523641 - \frac{1}{90} \cdot 524613 - \frac{1}{90} \cdot 524631 - \frac{1}{45} \cdot 435612 - \frac{1}{45} \cdot 435621 - \frac{1}{45} \cdot 534612$$
$$- \frac{1}{45} \cdot 534621 - \frac{4}{45} \cdot 623451 - \frac{2}{45} \cdot 624351 - \frac{1}{45} \cdot 623541 - \frac{1}{45} \cdot 625341 - \frac{1}{45} \cdot 632451$$
$$- \frac{1}{45} \cdot 642351 - \frac{1}{90} \cdot 253164 - \frac{1}{90} \cdot 154263 - \frac{1}{90} \cdot 154362 - \frac{1}{90} \cdot 514263 + \frac{1}{90} \cdot 426135$$
$$- \frac{1}{90} \cdot 146325 - \frac{1}{90} \cdot 246315 - \frac{1}{45} \cdot 431256 - \frac{2}{45} \cdot 432156 - \frac{1}{45} \cdot 342156 - \frac{1}{30} \cdot 432516$$

$$- \frac{4}{45} \cdot 432165 - \frac{1}{90} \cdot 431526 + \frac{1}{45} \cdot 354126 + \frac{1}{45} \cdot 354216 + \frac{1}{45} \cdot 534126 + \frac{1}{45} \cdot 534216$$
$$+ \frac{1}{45} \cdot 431562 + \frac{1}{45} \cdot 432561 + \frac{1}{90} \cdot 435162 + \frac{1}{90} \cdot 435261 + \frac{1}{90} \cdot 531462 + \frac{1}{90} \cdot 532461$$
$$+ \frac{1}{45} \cdot 534162 + \frac{1}{45} \cdot 534261 + \frac{1}{90} \cdot 354162 + \frac{1}{90} \cdot 354261 + \frac{1}{45} \cdot 436125 - \frac{1}{45} \cdot 346215$$
$$+ \frac{1}{90} \cdot 436152 + \frac{1}{90} \cdot 436251 - \frac{1}{90} \cdot 352146 - \frac{1}{90} \cdot 532146 + \frac{1}{45} \cdot 452136 + \frac{1}{45} \cdot 452316$$
$$+ \frac{1}{45} \cdot 542136 + \frac{1}{45} \cdot 542316 + \frac{1}{45} \cdot 452163 + \frac{1}{45} \cdot 542163 - \frac{1}{90} \cdot 352164 + \frac{1}{45} \cdot 453162$$
$$+ \frac{1}{45} \cdot 453261 + \frac{1}{45} \cdot 543162 + \frac{1}{45} \cdot 543261 + \frac{1}{45} \cdot 362145 + \frac{1}{45} \cdot 632145 + \frac{1}{90} \cdot 362415$$
$$+ \frac{1}{90} \cdot 462135 + \frac{1}{45} \cdot 462315 + \frac{1}{90} \cdot 632415 + \frac{1}{90} \cdot 642135 + \frac{1}{45} \cdot 642315 - \frac{1}{90} \cdot 461325$$
$$+ \frac{1}{90} \cdot 624315 - \frac{1}{90} \cdot 641325 + \frac{1}{90} \cdot 632514 + \frac{1}{45} \cdot 634215 + \frac{1}{45} \cdot 643215 + \frac{1}{90} \cdot 162453$$
$$+ \frac{1}{90} \cdot 513426 + \frac{1}{45} \cdot 613425 + \frac{1}{90} \cdot 163425 - \frac{1}{90} \cdot 613452 + \frac{1}{45} \cdot 156234 + \frac{1}{45} \cdot 165234$$
$$+ \frac{1}{90} \cdot 523146 - \frac{1}{90} \cdot 623415 - \frac{1}{90} \cdot 526134 - \frac{1}{90} \cdot 526314 - \frac{1}{90} \cdot 623514 - \frac{1}{90} \cdot 625134$$
$$- \frac{1}{90} \cdot 625314 + \frac{1}{45} \cdot 256134 + \frac{1}{45} \cdot 265134 + \frac{1}{45} \cdot 356124 + \frac{1}{45} \cdot 365124 + \frac{1}{45} \cdot 451236$$
$$+ \frac{1}{45} \cdot 541236 - \frac{1}{90} \cdot 461253 - \frac{1}{90} \cdot 461352 - \frac{1}{90} \cdot 631452 - \frac{1}{90} \cdot 641253 - \frac{1}{90} \cdot 641352$$
$$+ \frac{1}{45} \cdot 451263 + \frac{1}{45} \cdot 451623 + \frac{1}{45} \cdot 541263 + \frac{1}{45} \cdot 541623 - \frac{4}{45} \cdot 561234 - \frac{4}{45} \cdot 651234$$
$$- \frac{2}{45} \cdot 561324 - \frac{2}{45} \cdot 651324 - \frac{1}{45} \cdot 561243 - \frac{1}{45} \cdot 561423 - \frac{1}{45} \cdot 651243 - \frac{1}{45} \cdot 651423$$
$$- \frac{1}{45} \cdot 562134 - \frac{1}{45} \cdot 563124 - \frac{1}{45} \cdot 652134 - \frac{1}{45} \cdot 653124$$

$$[\![x_2 \times x_4]\!] = \frac{4}{45} \cdot 132456 + \frac{1}{45} \cdot 134256 + \frac{1}{45} \cdot 142356 + \frac{4}{45} \cdot 213456 + \frac{2}{45} \cdot 213465 + \frac{2}{45} \cdot 231456$$
$$+ \frac{1}{45} \cdot 231465 + \frac{4}{45} \cdot 214356 + \frac{2}{45} \cdot 312456 + \frac{1}{45} \cdot 312465 + \frac{2}{45} \cdot 213546 + \frac{1}{45} \cdot 213564$$
$$+ \frac{2}{45} \cdot 214536 + \frac{2}{45} \cdot 214563 + \frac{1}{45} \cdot 231546 - \frac{1}{45} \cdot 231564 - \frac{1}{45} \cdot 241563 + \frac{1}{45} \cdot 213645$$
$$+ \frac{2}{45} \cdot 215346 + \frac{2}{45} \cdot 216345 - \frac{1}{45} \cdot 231645 + \frac{1}{45} \cdot 312546 - \frac{1}{45} \cdot 312564 - \frac{1}{45} \cdot 312645$$
$$- \frac{1}{45} \cdot 316245 - \frac{1}{45} \cdot 234156 + \frac{2}{45} \cdot 234165 - \frac{1}{45} \cdot 243156 - \frac{1}{9} \cdot 234561 - \frac{2}{45} \cdot 234651$$
$$- \frac{1}{15} \cdot 234516 - \frac{1}{45} \cdot 243516 + \frac{1}{45} \cdot 235164 + \frac{1}{45} \cdot 235614 + \frac{1}{90} \cdot 245136 + \frac{1}{90} \cdot 245613$$
$$- \frac{1}{45} \cdot 236145 - \frac{1}{90} \cdot 253146 + \frac{1}{45} \cdot 261345 - \frac{1}{45} \cdot 263145 - \frac{2}{45} \cdot 235416 - \frac{2}{45} \cdot 235461$$
$$- \frac{1}{45} \cdot 235641 - \frac{1}{30} \cdot 245316 - \frac{1}{90} \cdot 245631 - \frac{1}{45} \cdot 236415 - \frac{1}{45} \cdot 236451 - \frac{1}{90} \cdot 253416$$
$$- \frac{1}{45} \cdot 263415 - \frac{1}{90} \cdot 263451 - \frac{1}{45} \cdot 412356 + \frac{2}{45} \cdot 412365 - \frac{1}{45} \cdot 413256 + \frac{1}{45} \cdot 314562$$
$$- \frac{1}{45} \cdot 412563 - \frac{1}{90} \cdot 413526 - \frac{1}{45} \cdot 413562 + \frac{1}{45} \cdot 412635 + \frac{1}{90} \cdot 415236 + \frac{1}{45} \cdot 512634$$

$$+\frac{1}{90}\cdot 516234-\frac{1}{9}\cdot 612345-\frac{2}{45}\cdot 612354-\frac{1}{15}\cdot 512346-\frac{1}{45}\cdot 513246-\frac{2}{45}\cdot 512436$$
$$-\frac{1}{45}\cdot 512463-\frac{1}{90}\cdot 513426-\frac{1}{45}\cdot 513462-\frac{2}{45}\cdot 612435-\frac{1}{45}\cdot 612453-\frac{1}{90}\cdot 613452$$
$$-\frac{1}{30}\cdot 514236-\frac{1}{45}\cdot 612534-\frac{1}{90}\cdot 615234+\frac{2}{45}\cdot 124356+\frac{1}{45}\cdot 124536+\frac{1}{45}\cdot 125346$$
$$+\frac{1}{45}\cdot 124563+\frac{1}{45}\cdot 126345+\frac{2}{45}\cdot 132546+\frac{2}{45}\cdot 132465+\frac{1}{45}\cdot 132564+\frac{1}{45}\cdot 132645$$
$$-\frac{1}{45}\cdot 135426-\frac{1}{45}\cdot 324156-\frac{1}{45}\cdot 134562-\frac{1}{45}\cdot 135462+\frac{2}{45}\cdot 324561+\frac{1}{90}\cdot 135624$$
$$-\frac{1}{90}\cdot 136425-\frac{1}{45}\cdot 134652-\frac{1}{90}\cdot 135642-\frac{1}{90}\cdot 136452-\frac{1}{45}\cdot 152436-\frac{1}{45}\cdot 421356$$
$$-\frac{1}{90}\cdot 152463+\frac{1}{90}\cdot 152634-\frac{1}{45}\cdot 162345-\frac{1}{45}\cdot 162435+\frac{2}{45}\cdot 621345-\frac{1}{45}\cdot 162354$$
$$-\frac{1}{90}\cdot 162453-\frac{1}{90}\cdot 162534-\frac{1}{45}\cdot 132654-\frac{1}{45}\cdot 136254-\frac{1}{45}\cdot 142653-\frac{1}{90}\cdot 136524$$
$$-\frac{1}{90}\cdot 136542-\frac{1}{90}\cdot 152643-\frac{1}{90}\cdot 162543-\frac{1}{45}\cdot 215436-\frac{1}{45}\cdot 215463-\frac{1}{45}\cdot 216435$$
$$-\frac{2}{45}\cdot 216453-\frac{1}{45}\cdot 251436-\frac{1}{90}\cdot 251463+\frac{1}{45}\cdot 261435+\frac{1}{90}\cdot 261453-\frac{1}{45}\cdot 213654$$
$$-\frac{1}{45}\cdot 214653-\frac{1}{45}\cdot 216354+\frac{1}{45}\cdot 261354-\frac{1}{45}\cdot 315426+\frac{1}{45}\cdot 315462-\frac{1}{90}\cdot 316425$$
$$+\frac{1}{90}\cdot 316452+\frac{1}{45}\cdot 314652-\frac{2}{45}\cdot 216534-\frac{4}{45}\cdot 216543+\frac{1}{90}\cdot 261534+\frac{1}{90}\cdot 261543$$
$$-\frac{2}{45}\cdot 215643+\frac{1}{90}\cdot 315642+\frac{1}{90}\cdot 316542-\frac{1}{90}\cdot 254136-\frac{1}{45}\cdot 254163-\frac{1}{30}\cdot 254316$$
$$-\frac{1}{90}\cdot 264135-\frac{1}{45}\cdot 264315-\frac{2}{45}\cdot 231654+\frac{1}{45}\cdot 236154-\frac{1}{45}\cdot 241653+\frac{1}{90}\cdot 246153$$
$$+\frac{1}{45}\cdot 254361+\frac{1}{90}\cdot 254613+\frac{1}{90}\cdot 254631+\frac{1}{90}\cdot 264351+\frac{1}{45}\cdot 264513+\frac{1}{45}\cdot 264531$$
$$+\frac{1}{45}\cdot 236514+\frac{1}{45}\cdot 236541+\frac{1}{90}\cdot 246513+\frac{1}{90}\cdot 246531+\frac{1}{90}\cdot 263514+\frac{1}{90}\cdot 263541$$
$$-\frac{1}{45}\cdot 265134+\frac{1}{45}\cdot 256143+\frac{1}{45}\cdot 265341+\frac{2}{45}\cdot 265431+\frac{1}{45}\cdot 256413+\frac{1}{45}\cdot 256431$$
$$+\frac{1}{45}\cdot 265413-\frac{1}{90}\cdot 415326-\frac{1}{90}\cdot 415362-\frac{1}{45}\cdot 416325-\frac{1}{30}\cdot 514326-\frac{1}{45}\cdot 514362$$
$$-\frac{2}{45}\cdot 312654-\frac{1}{45}\cdot 316254+\frac{1}{45}\cdot 412653+\frac{1}{90}\cdot 416253+\frac{1}{45}\cdot 416523-\frac{1}{45}\cdot 415632$$
$$+\frac{1}{90}\cdot 516324+\frac{1}{45}\cdot 516342+\frac{1}{45}\cdot 614325+\frac{1}{90}\cdot 614352+\frac{1}{90}\cdot 615324+\frac{1}{45}\cdot 615342$$
$$+\frac{1}{45}\cdot 512643+\frac{1}{90}\cdot 513642+\frac{1}{90}\cdot 516243+\frac{1}{45}\cdot 612543+\frac{1}{90}\cdot 613542+\frac{1}{90}\cdot 615243$$
$$+\frac{1}{45}\cdot 516423+\frac{1}{45}\cdot 516432+\frac{1}{45}\cdot 615423+\frac{2}{45}\cdot 615432+\frac{1}{45}\cdot 614532-\frac{1}{15}\cdot 143265$$
$$-\frac{1}{45}\cdot 153264-\frac{1}{90}\cdot 253164-\frac{1}{45}\cdot 143625-\frac{1}{45}\cdot 143652-\frac{1}{45}\cdot 241635-\frac{1}{45}\cdot 163254$$
$$-\frac{1}{15}\cdot 321546-\frac{2}{15}\cdot 321564-\frac{1}{15}\cdot 321465-\frac{1}{45}\cdot 421536-\frac{2}{45}\cdot 421563-\frac{1}{45}\cdot 325164$$
$$-\frac{1}{90}\cdot 425163-\frac{2}{15}\cdot 321645-\frac{1}{5}\cdot 321654-\frac{2}{45}\cdot 326154-\frac{2}{45}\cdot 421653-\frac{1}{45}\cdot 426153$$
$$-\frac{1}{45}\cdot 315264-\frac{1}{45}\cdot 325146-\frac{1}{45}\cdot 325416+\frac{4}{45}\cdot 341265+\frac{1}{18}\cdot 351264+\frac{1}{90}\cdot 352164$$

$$+\frac{1}{30}\cdot\mathsf{315624}+\frac{1}{15}\cdot\mathsf{325461}+\frac{1}{15}\cdot\mathsf{325614}+\frac{1}{15}\cdot\mathsf{325641}+\frac{1}{45}\cdot\mathsf{314625}+\frac{2}{45}\cdot\mathsf{324615}$$
$$+\frac{1}{15}\cdot\mathsf{324651}+\frac{1}{18}\cdot\mathsf{341625}+\frac{1}{15}\cdot\mathsf{341652}+\frac{1}{90}\cdot\mathsf{342615}+\frac{2}{45}\cdot\mathsf{342651}+\frac{2}{45}\cdot\mathsf{351624}$$
$$+\frac{1}{30}\cdot\mathsf{351642}+\frac{1}{90}\cdot\mathsf{352614}+\frac{1}{45}\cdot\mathsf{352641}+\frac{1}{45}\cdot\mathsf{243615}+\frac{1}{45}\cdot\mathsf{243651}-\frac{2}{45}\cdot\mathsf{326145}$$
$$+\frac{1}{15}\cdot\mathsf{361254}+\frac{2}{45}\cdot\mathsf{362154}+\frac{1}{15}\cdot\mathsf{326451}+\frac{1}{15}\cdot\mathsf{326541}+\frac{1}{90}\cdot\mathsf{316524}+\frac{1}{45}\cdot\mathsf{326514}$$
$$+\frac{1}{30}\cdot\mathsf{361524}+\frac{1}{45}\cdot\mathsf{361542}+\frac{1}{45}\cdot\mathsf{362514}+\frac{1}{90}\cdot\mathsf{362541}-\frac{1}{45}\cdot\mathsf{521436}+\frac{2}{45}\cdot\mathsf{423165}$$
$$+\frac{2}{45}\cdot\mathsf{521364}+\frac{1}{30}\cdot\mathsf{523164}+\frac{1}{45}\cdot\mathsf{513264}+\frac{1}{15}\cdot\mathsf{521634}+\frac{1}{45}\cdot\mathsf{521643}-\frac{1}{90}\cdot\mathsf{526143}$$
$$+\frac{1}{15}\cdot\mathsf{621435}+\frac{1}{15}\cdot\mathsf{621453}+\frac{1}{15}\cdot\mathsf{621354}+\frac{2}{45}\cdot\mathsf{623154}+\frac{1}{45}\cdot\mathsf{624153}+\frac{1}{45}\cdot\mathsf{613254}$$
$$+\frac{1}{15}\cdot\mathsf{621534}+\frac{1}{15}\cdot\mathsf{621543}+\frac{1}{90}\cdot\mathsf{625143}-\frac{1}{90}\cdot\mathsf{413625}-\frac{1}{45}\cdot\mathsf{421635}-\frac{1}{90}\cdot\mathsf{426135}$$
$$+\frac{1}{30}\cdot\mathsf{423615}+\frac{2}{45}\cdot\mathsf{423651}+\frac{1}{45}\cdot\mathsf{426351}-\frac{1}{90}\cdot\mathsf{426513}+\frac{1}{90}\cdot\mathsf{426531}+\frac{1}{90}\cdot\mathsf{431625}$$
$$+\frac{2}{45}\cdot\mathsf{431652}+\frac{1}{30}\cdot\mathsf{251634}+\frac{1}{45}\cdot\mathsf{251364}+\frac{1}{90}\cdot\mathsf{531264}+\frac{1}{90}\cdot\mathsf{531624}+\frac{2}{45}\cdot\mathsf{631254}$$
$$+\frac{1}{45}\cdot\mathsf{631524}+\frac{1}{90}\cdot\mathsf{251643}+\frac{1}{45}\cdot\mathsf{531642}+\frac{1}{90}\cdot\mathsf{631542}+\frac{1}{45}\cdot\mathsf{143562}+\frac{1}{90}\cdot\mathsf{145263}$$
$$+\frac{1}{90}\cdot\mathsf{145362}+\frac{1}{90}\cdot\mathsf{153462}+\frac{1}{45}\cdot\mathsf{145623}+\frac{1}{45}\cdot\mathsf{145632}+\frac{1}{45}\cdot\mathsf{163452}+\frac{1}{90}\cdot\mathsf{341526}$$
$$-\frac{1}{90}\cdot\mathsf{342516}+\frac{1}{90}\cdot\mathsf{423516}+\frac{1}{45}\cdot\mathsf{345126}+\frac{1}{45}\cdot\mathsf{345216}-\frac{1}{30}\cdot\mathsf{345162}-\frac{1}{30}\cdot\mathsf{345261}$$
$$-\frac{1}{90}\cdot\mathsf{354162}-\frac{1}{90}\cdot\mathsf{354261}-\frac{4}{45}\cdot\mathsf{345612}-\frac{4}{45}\cdot\mathsf{345621}-\frac{2}{45}\cdot\mathsf{354612}-\frac{2}{45}\cdot\mathsf{354621}$$
$$+\frac{1}{45}\cdot\mathsf{346125}+\frac{1}{45}\cdot\mathsf{346215}+\frac{1}{45}\cdot\mathsf{356124}+\frac{1}{45}\cdot\mathsf{356214}-\frac{1}{90}\cdot\mathsf{346152}-\frac{1}{90}\cdot\mathsf{346251}$$
$$-\frac{1}{45}\cdot\mathsf{361452}-\frac{1}{90}\cdot\mathsf{362451}-\frac{1}{90}\cdot\mathsf{364152}-\frac{1}{90}\cdot\mathsf{364251}-\frac{2}{45}\cdot\mathsf{346512}-\frac{2}{45}\cdot\mathsf{346521}$$
$$-\frac{1}{45}\cdot\mathsf{356412}-\frac{1}{45}\cdot\mathsf{356421}-\frac{1}{45}\cdot\mathsf{364512}-\frac{1}{45}\cdot\mathsf{364521}+\frac{1}{45}\cdot\mathsf{523416}-\frac{1}{30}\cdot\mathsf{523461}$$
$$-\frac{1}{90}\cdot\mathsf{524361}-\frac{1}{90}\cdot\mathsf{425613}-\frac{1}{90}\cdot\mathsf{425631}-\frac{1}{45}\cdot\mathsf{523614}-\frac{1}{90}\cdot\mathsf{523641}-\frac{1}{90}\cdot\mathsf{524613}$$
$$-\frac{1}{90}\cdot\mathsf{524631}-\frac{4}{45}\cdot\mathsf{623451}-\frac{2}{45}\cdot\mathsf{624351}-\frac{2}{45}\cdot\mathsf{623541}-\frac{1}{45}\cdot\mathsf{624531}-\frac{1}{45}\cdot\mathsf{625341}$$
$$-\frac{1}{45}\cdot\mathsf{154236}-\frac{2}{45}\cdot\mathsf{154326}-\frac{1}{45}\cdot\mathsf{145326}-\frac{1}{90}\cdot\mathsf{154263}-\frac{1}{90}\cdot\mathsf{154362}-\frac{1}{90}\cdot\mathsf{514263}$$
$$-\frac{1}{90}\cdot\mathsf{146325}-\frac{1}{90}\cdot\mathsf{164325}-\frac{1}{90}\cdot\mathsf{246315}-\frac{2}{45}\cdot\mathsf{431256}-\frac{4}{45}\cdot\mathsf{432156}-\frac{1}{90}\cdot\mathsf{531246}$$
$$-\frac{1}{30}\cdot\mathsf{532146}-\frac{2}{45}\cdot\mathsf{342156}-\frac{1}{30}\cdot\mathsf{432516}-\frac{4}{45}\cdot\mathsf{432165}-\frac{1}{30}\cdot\mathsf{532164}-\frac{1}{30}\cdot\mathsf{432615}$$
$$-\frac{1}{90}\cdot\mathsf{431526}+\frac{1}{45}\cdot\mathsf{435126}+\frac{1}{45}\cdot\mathsf{435216}+\frac{2}{45}\cdot\mathsf{534126}+\frac{2}{45}\cdot\mathsf{534216}+\frac{1}{45}\cdot\mathsf{354126}$$
$$+\frac{1}{45}\cdot\mathsf{354216}+\frac{1}{45}\cdot\mathsf{431562}+\frac{1}{45}\cdot\mathsf{432561}+\frac{1}{90}\cdot\mathsf{435162}+\frac{1}{90}\cdot\mathsf{435261}+\frac{1}{90}\cdot\mathsf{531462}$$
$$+\frac{1}{90}\cdot\mathsf{532461}+\frac{1}{45}\cdot\mathsf{534162}+\frac{1}{45}\cdot\mathsf{534261}-\frac{1}{45}\cdot\mathsf{532614}+\frac{1}{45}\cdot\mathsf{436125}+\frac{1}{45}\cdot\mathsf{436215}$$
$$+\frac{1}{45}\cdot\mathsf{432651}+\frac{1}{90}\cdot\mathsf{532641}+\frac{1}{90}\cdot\mathsf{436152}+\frac{1}{90}\cdot\mathsf{436251}-\frac{1}{90}\cdot\mathsf{352146}+\frac{1}{45}\cdot\mathsf{452136}$$

$$+\frac{2}{45}\cdot 452316+\frac{1}{45}\cdot 542136+\frac{2}{45}\cdot 542316+\frac{1}{45}\cdot 451326+\frac{1}{45}\cdot 541326+\frac{1}{45}\cdot 452163$$
$$+\frac{1}{45}\cdot 542163+\frac{1}{45}\cdot 362145+\frac{1}{45}\cdot 632145+\frac{1}{90}\cdot 362415+\frac{1}{90}\cdot 462135+\frac{1}{45}\cdot 462315$$
$$+\frac{1}{90}\cdot 632415+\frac{1}{90}\cdot 642135+\frac{1}{45}\cdot 642315-\frac{1}{90}\cdot 461325-\frac{1}{90}\cdot 624315-\frac{1}{90}\cdot 641325$$
$$+\frac{1}{90}\cdot 462153+\frac{1}{45}\cdot 632154+\frac{1}{90}\cdot 642153+\frac{1}{90}\cdot 632514+\frac{1}{45}\cdot 163245+\frac{1}{90}\cdot 163425$$
$$+\frac{1}{90}\cdot 146235+\frac{1}{90}\cdot 164235+\frac{1}{45}\cdot 156234+\frac{1}{45}\cdot 165234+\frac{1}{90}\cdot 523146+\frac{1}{90}\cdot 351246$$
$$-\frac{1}{30}\cdot 623415-\frac{1}{90}\cdot 526134-\frac{1}{90}\cdot 526314-\frac{1}{90}\cdot 623514-\frac{1}{90}\cdot 625134-\frac{1}{90}\cdot 625314$$
$$+\frac{1}{45}\cdot 451236+\frac{1}{45}\cdot 541236-\frac{1}{30}\cdot 461235-\frac{1}{30}\cdot 641235-\frac{1}{90}\cdot 461253-\frac{1}{90}\cdot 461352$$
$$-\frac{1}{90}\cdot 631452-\frac{1}{90}\cdot 641253-\frac{1}{90}\cdot 641352+\frac{1}{45}\cdot 451263+\frac{1}{45}\cdot 451623+\frac{1}{45}\cdot 541263$$
$$+\frac{1}{45}\cdot 541623-\frac{4}{45}\cdot 561234-\frac{4}{45}\cdot 651234-\frac{2}{45}\cdot 561324-\frac{2}{45}\cdot 651324-\frac{2}{45}\cdot 561243$$
$$-\frac{1}{45}\cdot 561342-\frac{2}{45}\cdot 651243-\frac{1}{45}\cdot 651342-\frac{1}{45}\cdot 561423-\frac{1}{45}\cdot 651423$$

$$[\![x_2\times x_5]\!]=-\frac{2}{45}\cdot 123546-\frac{1}{45}\cdot 123564-\frac{1}{45}\cdot 125346-\frac{2}{45}\cdot 124365-\frac{1}{45}\cdot 142356-\frac{2}{45}\cdot 142365$$
$$+\frac{2}{45}\cdot 132456+\frac{1}{45}\cdot 134256+\frac{1}{45}\cdot 134526+\frac{1}{45}\cdot 134562+\frac{1}{45}\cdot 143526+\frac{2}{45}\cdot 143562$$
$$+\frac{1}{45}\cdot 126345+\frac{1}{45}\cdot 126354+\frac{1}{45}\cdot 162345+\frac{2}{45}\cdot 213456+\frac{1}{45}\cdot 231456+\frac{2}{45}\cdot 214356$$
$$-\frac{1}{45}\cdot 235416-\frac{1}{45}\cdot 235461-\frac{1}{45}\cdot 253416-\frac{1}{45}\cdot 253461-\frac{1}{45}\cdot 412356-\frac{1}{45}\cdot 413256$$
$$+\frac{2}{45}\cdot 412635+\frac{1}{45}\cdot 416235+\frac{1}{45}\cdot 512634+\frac{1}{45}\cdot 516234+\frac{2}{45}\cdot 324561+\frac{1}{45}\cdot 342561$$
$$-\frac{2}{45}\cdot 512436-\frac{2}{45}\cdot 514236-\frac{1}{45}\cdot 612435-\frac{1}{45}\cdot 614235+\frac{1}{45}\cdot 521346+\frac{1}{45}\cdot 523146$$
$$+\frac{2}{45}\cdot 621345+\frac{1}{45}\cdot 623145-\frac{2}{45}\cdot 123465-\frac{1}{45}\cdot 123645+\frac{1}{45}\cdot 124536+\frac{2}{45}\cdot 214536$$
$$+\frac{1}{45}\cdot 124563+\frac{1}{45}\cdot 125463+\frac{1}{45}\cdot 312456-\frac{1}{45}\cdot 234156-\frac{1}{45}\cdot 234516-\frac{1}{45}\cdot 324156$$
$$-\frac{1}{45}\cdot 134652-\frac{1}{45}\cdot 136452-\frac{2}{45}\cdot 234651-\frac{1}{45}\cdot 236451-\frac{1}{45}\cdot 152346-\frac{1}{45}\cdot 152436$$
$$-\frac{1}{45}\cdot 512346-\frac{2}{45}\cdot 241563-\frac{1}{45}\cdot 245163-\frac{1}{45}\cdot 341562-\frac{1}{45}\cdot 345162+\frac{2}{45}\cdot 145362$$
$$+\frac{1}{45}\cdot 243561+\frac{1}{45}\cdot 245361-\frac{2}{45}\cdot 612354-\frac{1}{45}\cdot 612534+\frac{1}{45}\cdot 163245+\frac{1}{45}\cdot 163425$$
$$+\frac{1}{45}\cdot 613245+\frac{1}{45}\cdot 613425+\frac{1}{45}\cdot 126534+\frac{2}{45}\cdot 126543+\frac{1}{45}\cdot 162543+\frac{1}{45}\cdot 125643$$
$$+\frac{1}{45}\cdot 145326+\frac{1}{45}\cdot 154362-\frac{1}{45}\cdot 146523-\frac{1}{45}\cdot 146532-\frac{1}{45}\cdot 164523-\frac{1}{45}\cdot 164532$$
$$-\frac{1}{45}\cdot 156324-\frac{1}{45}\cdot 156342-\frac{1}{45}\cdot 165324-\frac{1}{45}\cdot 165342-\frac{1}{45}\cdot 216435-\frac{2}{45}\cdot 216453$$
$$-\frac{1}{45}\cdot 214653-\frac{1}{45}\cdot 314652-\frac{1}{45}\cdot 316452+\frac{2}{45}\cdot 231654+\frac{1}{45}\cdot 236154+\frac{1}{45}\cdot 256413$$

$$+\frac{1}{45}\cdot 256431+\frac{1}{45}\cdot 265413+\frac{1}{45}\cdot 265431+\frac{2}{45}\cdot 312654+\frac{1}{45}\cdot 316254+\frac{2}{45}\cdot 412653$$
$$+\frac{1}{45}\cdot 416253+\frac{1}{45}\cdot 316524+\frac{1}{45}\cdot 316542+\frac{1}{45}\cdot 361524+\frac{1}{45}\cdot 361542-\frac{2}{45}\cdot 415632$$
$$-\frac{1}{45}\cdot 416532+\frac{1}{45}\cdot 614532+\frac{1}{45}\cdot 615432-\frac{1}{45}\cdot 521643-\frac{1}{45}\cdot 526143+\frac{1}{45}\cdot 213654$$
$$-\frac{1}{45}\cdot 143265-\frac{2}{45}\cdot 215634-\frac{1}{45}\cdot 215643-\frac{1}{45}\cdot 251634-\frac{1}{45}\cdot 251643-\frac{1}{45}\cdot 321546$$
$$-\frac{2}{45}\cdot 321564-\frac{1}{45}\cdot 325164-\frac{2}{45}\cdot 421563-\frac{1}{45}\cdot 425163+\frac{2}{45}\cdot 341265+\frac{1}{45}\cdot 342165$$
$$+\frac{1}{45}\cdot 421365+\frac{2}{45}\cdot 423165+\frac{1}{45}\cdot 521364+\frac{1}{45}\cdot 523164+\frac{1}{45}\cdot 421635-\frac{1}{45}\cdot 423651$$
$$-\frac{1}{45}\cdot 432615-\frac{1}{45}\cdot 432651-\frac{1}{45}\cdot 631254-\frac{1}{45}\cdot 632154+\frac{1}{45}\cdot 132654+\frac{1}{45}\cdot 215436$$
$$-\frac{1}{45}\cdot 216534-\frac{2}{45}\cdot 321645-\frac{1}{45}\cdot 326145-\frac{1}{45}\cdot 321465+\frac{1}{45}\cdot 243165+\frac{1}{45}\cdot 325641$$
$$+\frac{1}{45}\cdot 326541+\frac{1}{45}\cdot 341625+\frac{1}{45}\cdot 431265+\frac{1}{45}\cdot 431625+\frac{1}{45}\cdot 431652+\frac{1}{45}\cdot 436152$$
$$-\frac{1}{45}\cdot 241653+\frac{1}{45}\cdot 261543+\frac{1}{45}\cdot 621453+\frac{1}{45}\cdot 621543-\frac{1}{45}\cdot 352164-\frac{1}{45}\cdot 352614$$
$$-\frac{1}{45}\cdot 532164-\frac{1}{45}\cdot 532614-\frac{1}{45}\cdot 234615-\frac{1}{45}\cdot 243651+\frac{1}{45}\cdot 245613+\frac{1}{45}\cdot 245631$$
$$+\frac{1}{45}\cdot 254613+\frac{1}{45}\cdot 254631+\frac{1}{45}\cdot 325461-\frac{1}{45}\cdot 346512-\frac{1}{45}\cdot 346521-\frac{1}{45}\cdot 364512$$
$$-\frac{1}{45}\cdot 364521-\frac{1}{45}\cdot 523461-\frac{1}{45}\cdot 524361-\frac{1}{45}\cdot 415623-\frac{1}{45}\cdot 451632+\frac{1}{45}\cdot 435612$$
$$+\frac{1}{45}\cdot 435621+\frac{1}{45}\cdot 453612+\frac{1}{45}\cdot 453621-\frac{1}{45}\cdot 623541-\frac{1}{45}\cdot 625341+\frac{1}{45}\cdot 632451$$
$$+\frac{1}{45}\cdot 634251-\frac{1}{45}\cdot 154236-\frac{1}{45}\cdot 514326-\frac{1}{45}\cdot 431256-\frac{2}{45}\cdot 432156-\frac{1}{45}\cdot 342156$$
$$-\frac{1}{45}\cdot 432516+\frac{1}{45}\cdot 354126+\frac{1}{45}\cdot 354216+\frac{1}{45}\cdot 534126+\frac{1}{45}\cdot 534216+\frac{1}{45}\cdot 452136$$
$$+\frac{1}{45}\cdot 452316+\frac{1}{45}\cdot 542136+\frac{1}{45}\cdot 542316+\frac{2}{45}\cdot 541263+\frac{1}{45}\cdot 542163-\frac{1}{45}\cdot 542361$$
$$-\frac{1}{45}\cdot 543261-\frac{1}{45}\cdot 463125-\frac{1}{45}\cdot 463215-\frac{1}{45}\cdot 643125-\frac{1}{45}\cdot 643215-\frac{1}{45}\cdot 613254$$
$$+\frac{1}{45}\cdot 613452+\frac{1}{45}\cdot 614352+\frac{1}{45}\cdot 261345+\frac{1}{45}\cdot 621435-\frac{1}{45}\cdot 461235-\frac{1}{45}\cdot 461325$$
$$-\frac{1}{45}\cdot 641235-\frac{1}{45}\cdot 641325+\frac{1}{45}\cdot 451263+\frac{1}{45}\cdot 541623-\frac{1}{45}\cdot 561243-\frac{1}{45}\cdot 561423$$
$$-\frac{1}{45}\cdot 651243-\frac{1}{45}\cdot 651423+\frac{1}{45}\cdot 562134+\frac{1}{45}\cdot 562314+\frac{1}{45}\cdot 652134+\frac{1}{45}\cdot 652314$$

$$\llbracket x_3\times x_3\rrbracket=\frac{2}{45}\cdot 123564+\frac{1}{9}\cdot 123654+\frac{1}{15}\cdot 132564+\frac{8}{45}\cdot 132654+\frac{1}{15}\cdot 124653+\frac{1}{9}\cdot 125436$$
$$+\frac{1}{15}\cdot 126435+\frac{1}{15}\cdot 135426+\frac{2}{45}\cdot 132465+\frac{1}{45}\cdot 134265+\frac{1}{45}\cdot 125463-\frac{1}{45}\cdot 135462$$
$$-\frac{2}{45}\cdot 136452-\frac{1}{15}\cdot 135624-\frac{1}{45}\cdot 136524-\frac{2}{45}\cdot 152364-\frac{2}{45}\cdot 162354+\frac{2}{45}\cdot 213546$$
$$+\frac{1}{15}\cdot 213645+\frac{1}{15}\cdot 231546+\frac{8}{45}\cdot 231645-\frac{2}{45}\cdot 235146+\frac{4}{45}\cdot 236145+\frac{2}{45}\cdot 213465$$

$$+\frac{2}{15}\cdot 214365+\frac{8}{45}\cdot 312645+\frac{8}{45}\cdot 213654+\frac{2}{45}\cdot 214653+\frac{4}{15}\cdot 231654+\frac{4}{45}\cdot 236154$$
$$+\frac{4}{45}\cdot 241653+\frac{1}{45}\cdot 246153+\frac{1}{15}\cdot 213564+\frac{8}{45}\cdot 231564+\frac{4}{15}\cdot 312654+\frac{8}{45}\cdot 312564$$
$$-\frac{2}{45}\cdot 235416+\frac{1}{15}\cdot 231465-\frac{1}{15}\cdot 234165-\frac{4}{45}\cdot 234615-\frac{2}{15}\cdot 235461-\frac{2}{45}\cdot 236451$$
$$-\frac{2}{15}\cdot 234651-\frac{2}{9}\cdot 243651-\frac{2}{45}\cdot 235614-\frac{1}{45}\cdot 236514-\frac{1}{15}\cdot 251364-\frac{1}{45}\cdot 253164$$
$$-\frac{1}{9}\cdot 261354-\frac{4}{45}\cdot 351264-\frac{7}{45}\cdot 361254-\frac{4}{45}\cdot 235641-\frac{1}{15}\cdot 236541+\frac{1}{45}\cdot 412635$$
$$-\frac{1}{15}\cdot 314625-\frac{1}{15}\cdot 412365+\frac{2}{45}\cdot 413265-\frac{1}{9}\cdot 314652+\frac{2}{45}\cdot 412653-\frac{2}{45}\cdot 413652$$
$$+\frac{4}{45}\cdot 412563+\frac{2}{45}\cdot 516243-\frac{2}{9}\cdot 324651-\frac{7}{45}\cdot 423651-\frac{4}{45}\cdot 512634-\frac{2}{15}\cdot 612435$$
$$-\frac{2}{45}\cdot 612534-\frac{4}{45}\cdot 512364-\frac{4}{45}\cdot 513264-\frac{2}{15}\cdot 612354-\frac{2}{9}\cdot 613254-\frac{1}{15}\cdot 514263$$
$$-\frac{4}{45}\cdot 612453-\frac{1}{15}\cdot 612543-\frac{1}{9}\cdot 521364-\frac{4}{45}\cdot 531264-\frac{2}{9}\cdot 621354-\frac{7}{45}\cdot 631254$$
$$+\frac{2}{45}\cdot 123645+\frac{4}{45}\cdot 125346+\frac{2}{45}\cdot 124365+\frac{2}{45}\cdot 124635+\frac{2}{45}\cdot 214635+\frac{1}{45}\cdot 126354$$
$$+\frac{2}{45}\cdot 132546-\frac{2}{45}\cdot 142563+\frac{1}{15}\cdot 312465+\frac{1}{15}\cdot 132645+\frac{2}{45}\cdot 135246+\frac{1}{15}\cdot 235164$$
$$+\frac{2}{45}\cdot 324165-\frac{1}{15}\cdot 135642-\frac{1}{9}\cdot 324615+\frac{2}{45}\cdot 136254+\frac{2}{45}\cdot 316254+\frac{1}{15}\cdot 461253$$
$$-\frac{1}{45}\cdot 136542+\frac{1}{45}\cdot 152436+\frac{2}{45}\cdot 512463+\frac{1}{9}\cdot 142365-\frac{1}{15}\cdot 152634-\frac{1}{45}\cdot 152643$$
$$-\frac{1}{45}\cdot 512643-\frac{2}{45}\cdot 153624-\frac{2}{45}\cdot 153642-\frac{2}{15}\cdot 243615-\frac{1}{15}\cdot 423615-\frac{2}{45}\cdot 162453$$
$$-\frac{1}{45}\cdot 162543-\frac{2}{45}\cdot 164253+\frac{4}{45}\cdot 142356+\frac{1}{9}\cdot 143256+\frac{8}{45}\cdot 143265-\frac{2}{45}\cdot 143562$$
$$-\frac{2}{45}\cdot 145326-\frac{1}{9}\cdot 146235-\frac{1}{15}\cdot 146325-\frac{1}{45}\cdot 162435-\frac{4}{45}\cdot 163425+\frac{2}{45}\cdot 214356$$
$$+\frac{1}{45}\cdot 214536+\frac{1}{9}\cdot 215346+\frac{8}{45}\cdot 215436+\frac{2}{45}\cdot 216435+\frac{4}{45}\cdot 315264+\frac{2}{45}\cdot 315426$$
$$+\frac{1}{45}\cdot 316425+\frac{2}{45}\cdot 241356+\frac{2}{45}\cdot 241365+\frac{1}{45}\cdot 243156-\frac{2}{15}\cdot 243561-\frac{1}{45}\cdot 245136$$
$$-\frac{1}{15}\cdot 245316-\frac{2}{45}\cdot 246135-\frac{1}{15}\cdot 246315-\frac{4}{45}\cdot 245361-\frac{4}{45}\cdot 261435+\frac{1}{45}\cdot 254136$$
$$-\frac{1}{45}\cdot 254316-\frac{2}{45}\cdot 254361-\frac{1}{15}\cdot 264135+\frac{1}{45}\cdot 264351+\frac{1}{15}\cdot 413256+\frac{1}{15}\cdot 312546$$
$$-\frac{2}{15}\cdot 315462-\frac{1}{9}\cdot 415236-\frac{1}{15}\cdot 415326+\frac{4}{45}\cdot 416325+\frac{1}{15}\cdot 516324-\frac{2}{9}\cdot 325461$$
$$-\frac{2}{45}\cdot 425136-\frac{2}{45}\cdot 425316-\frac{4}{45}\cdot 513426-\frac{2}{15}\cdot 613245-\frac{4}{45}\cdot 613425-\frac{1}{45}\cdot 514326$$
$$-\frac{2}{45}\cdot 614325+\frac{1}{45}\cdot 615324-\frac{2}{45}\cdot 531426-\frac{2}{9}\cdot 621435+\frac{2}{45}\cdot 125364+\frac{2}{45}\cdot 215364$$
$$+\frac{1}{15}\cdot 143526+\frac{4}{45}\cdot 241635+\frac{2}{45}\cdot 143625+\frac{1}{45}\cdot 413625+\frac{2}{45}\cdot 142536-\frac{1}{45}\cdot 145263$$
$$-\frac{1}{15}\cdot 145362-\frac{2}{45}\cdot 415263-\frac{1}{15}\cdot 415362+\frac{1}{15}\cdot 461325-\frac{2}{45}\cdot 146253-\frac{2}{45}\cdot 146352$$
$$+\frac{1}{45}\cdot 153246-\frac{1}{45}\cdot 513246+\frac{1}{45}\cdot 154263-\frac{1}{45}\cdot 154362+\frac{1}{45}\cdot 524361-\frac{2}{45}\cdot 163524$$

$$- \frac{1}{45} \cdot 164325 + \frac{1}{45} \cdot 641325 - \frac{4}{45} \cdot 145623 - \frac{4}{45} \cdot 145632 - \frac{1}{9} \cdot 163452 - \frac{1}{15} \cdot 214563$$
$$- \frac{4}{45} \cdot 314562 - \frac{4}{45} \cdot 215634 - \frac{2}{45} \cdot 215643 - \frac{2}{45} \cdot 216453 - \frac{1}{15} \cdot 316452 + \frac{1}{15} \cdot 241563$$
$$+ \frac{1}{15} \cdot 245613 + \frac{1}{15} \cdot 245631 + \frac{2}{45} \cdot 246513 + \frac{2}{45} \cdot 246531 + \frac{2}{15} \cdot 245163 - \frac{1}{45} \cdot 251463$$
$$- \frac{1}{9} \cdot 261453 - \frac{2}{45} \cdot 351462 + \frac{4}{45} \cdot 254163 + \frac{1}{45} \cdot 254613 + \frac{1}{45} \cdot 254631 - \frac{2}{45} \cdot 264153$$
$$+ \frac{1}{45} \cdot 264513 + \frac{1}{45} \cdot 264531 - \frac{2}{45} \cdot 415623 - \frac{1}{45} \cdot 516342 + \frac{4}{45} \cdot 325164 + \frac{1}{45} \cdot 425613$$
$$+ \frac{1}{45} \cdot 425631 + \frac{1}{15} \cdot 613452 + \frac{2}{45} \cdot 613542 + \frac{2}{45} \cdot 513462 + \frac{1}{45} \cdot 614352 + \frac{1}{45} \cdot 615342$$
$$+ \frac{1}{45} \cdot 631452 + \frac{2}{45} \cdot 361452 + \frac{1}{45} \cdot 142635 - \frac{7}{45} \cdot 325614 - \frac{1}{5} \cdot 325641 + \frac{1}{15} \cdot 461352$$
$$- \frac{2}{45} \cdot 154623 - \frac{2}{45} \cdot 154632 - \frac{2}{45} \cdot 514623 - \frac{2}{45} \cdot 514632 - \frac{1}{5} \cdot 621453 - \frac{2}{45} \cdot 163542$$
$$- \frac{2}{45} \cdot 164352 - \frac{4}{45} \cdot 156234 - \frac{4}{45} \cdot 165234 - \frac{1}{45} \cdot 162534 - \frac{1}{15} \cdot 216345 - \frac{2}{45} \cdot 251346$$
$$- \frac{4}{45} \cdot 261345 + \frac{2}{45} \cdot 263145 - \frac{2}{45} \cdot 216534 - \frac{4}{45} \cdot 315624 - \frac{1}{15} \cdot 316524 + \frac{2}{45} \cdot 263415$$
$$+ \frac{1}{15} \cdot 263451 - \frac{4}{45} \cdot 256134 - \frac{4}{45} \cdot 265134 - \frac{4}{45} \cdot 251634 - \frac{4}{45} \cdot 261534 - \frac{4}{45} \cdot 351624$$
$$- \frac{4}{45} \cdot 361524 + \frac{2}{45} \cdot 256341 + \frac{2}{45} \cdot 265341 + \frac{2}{45} \cdot 416235 - \frac{1}{45} \cdot 514236 + \frac{1}{15} \cdot 416253$$
$$- \frac{2}{45} \cdot 416523 - \frac{7}{45} \cdot 326451 - \frac{1}{15} \cdot 426351 + \frac{1}{15} \cdot 516234 + \frac{1}{15} \cdot 615234 + \frac{2}{45} \cdot 614523$$
$$+ \frac{2}{45} \cdot 615423 - \frac{7}{45} \cdot 521634 - \frac{4}{45} \cdot 531624 - \frac{7}{45} \cdot 621534 - \frac{1}{15} \cdot 631524 + \frac{1}{45} \cdot 316245$$
$$+ \frac{1}{45} \cdot 135264 - \frac{2}{45} \cdot 326415 - \frac{2}{45} \cdot 253614 - \frac{2}{45} \cdot 253641 + \frac{2}{45} \cdot 154236 - \frac{1}{45} \cdot 164235$$
$$- \frac{2}{45} \cdot 246351 - \frac{2}{45} \cdot 156243 - \frac{2}{45} \cdot 165243 - \frac{2}{45} \cdot 614253 - \frac{2}{45} \cdot 613524 + \frac{2}{45} \cdot 312456$$
$$+ \frac{1}{9} \cdot 321456 + \frac{8}{45} \cdot 321465 + \frac{1}{15} \cdot 324156 + \frac{8}{45} \cdot 321546 + \frac{4}{15} \cdot 321564 + \frac{4}{15} \cdot 321645$$
$$+ \frac{2}{45} \cdot 326145 + \frac{2}{45} \cdot 314256 + \frac{2}{45} \cdot 314265 - \frac{2}{15} \cdot 324561 - \frac{1}{15} \cdot 341526 - \frac{2}{45} \cdot 341562$$
$$- \frac{1}{15} \cdot 342516 - \frac{4}{45} \cdot 342561 - \frac{1}{15} \cdot 351246 - \frac{1}{45} \cdot 352146 - \frac{4}{45} \cdot 361245 - \frac{1}{45} \cdot 362145$$
$$- \frac{2}{45} \cdot 351426 - \frac{2}{45} \cdot 352416 + \frac{1}{45} \cdot 421356 + \frac{2}{45} \cdot 421536 + \frac{4}{45} \cdot 421563 + \frac{2}{45} \cdot 421635$$
$$+ \frac{1}{15} \cdot 526134 - \frac{1}{45} \cdot 431526 - \frac{1}{45} \cdot 431562 - \frac{1}{45} \cdot 432516 - \frac{1}{15} \cdot 432561 - \frac{2}{15} \cdot 621345$$
$$- \frac{2}{45} \cdot 521346 - \frac{2}{45} \cdot 523146 - \frac{4}{45} \cdot 623145 - \frac{2}{45} \cdot 524136 - \frac{1}{45} \cdot 532146 - \frac{1}{15} \cdot 632145$$
$$+ \frac{2}{45} \cdot 231456 + \frac{1}{45} \cdot 425163 - \frac{1}{45} \cdot 243516 - \frac{2}{45} \cdot 423516 - \frac{2}{45} \cdot 423561 + \frac{2}{45} \cdot 462135$$
$$- \frac{2}{45} \cdot 631245 + \frac{2}{5} \cdot 321654 + \frac{4}{45} \cdot 426153 + \frac{1}{45} \cdot 315246 - \frac{4}{45} \cdot 341265 - \frac{2}{45} \cdot 342165$$
$$- \frac{4}{45} \cdot 315642 - \frac{4}{45} \cdot 341625 - \frac{7}{45} \cdot 341652 - \frac{4}{45} \cdot 342615 - \frac{1}{5} \cdot 342651 - \frac{2}{45} \cdot 351642$$
$$- \frac{2}{45} \cdot 352614 - \frac{1}{15} \cdot 352641 - \frac{2}{45} \cdot 362154 + \frac{1}{15} \cdot 462153 - \frac{1}{15} \cdot 316542 - \frac{4}{45} \cdot 326514$$

$$
\begin{aligned}
&-\frac{2}{15}\cdot 326541-\frac{2}{45}\cdot 361542-\frac{2}{45}\cdot 362514-\frac{1}{45}\cdot 362541-\frac{2}{45}\cdot 423165-\frac{1}{9}\cdot 523164\\
&-\frac{2}{45}\cdot 524163-\frac{2}{45}\cdot 521643+\frac{1}{15}\cdot 526143-\frac{1}{15}\cdot 431625-\frac{4}{45}\cdot 431652-\frac{1}{15}\cdot 432615\\
&-\frac{2}{15}\cdot 432651-\frac{2}{45}\cdot 531642-\frac{2}{45}\cdot 532614-\frac{1}{45}\cdot 532641-\frac{1}{5}\cdot 623154-\frac{1}{15}\cdot 624153\\
&-\frac{2}{15}\cdot 621543-\frac{1}{45}\cdot 625143-\frac{2}{15}\cdot 632154-\frac{1}{45}\cdot 642153-\frac{1}{45}\cdot 352164+\frac{4}{45}\cdot 421653\\
&-\frac{1}{15}\cdot 532164+\frac{4}{45}\cdot 326154-\frac{2}{45}\cdot 431265-\frac{1}{45}\cdot 251643-\frac{1}{15}\cdot 261543+\frac{1}{45}\cdot 241536\\
&-\frac{4}{45}\cdot 345126-\frac{4}{45}\cdot 345216-\frac{2}{45}\cdot 346125-\frac{2}{45}\cdot 354126-\frac{2}{45}\cdot 354216-\frac{2}{45}\cdot 364125\\
&-\frac{2}{45}\cdot 364215+\frac{2}{45}\cdot 523614+\frac{1}{15}\cdot 526314-\frac{1}{9}\cdot 523416-\frac{2}{45}\cdot 524316-\frac{2}{45}\cdot 532416\\
&+\frac{1}{15}\cdot 345162+\frac{1}{15}\cdot 345261+\frac{2}{45}\cdot 435162+\frac{2}{45}\cdot 435261-\frac{1}{45}\cdot 462315+\frac{1}{45}\cdot 346152\\
&+\frac{1}{45}\cdot 346251+\frac{1}{45}\cdot 354162+\frac{1}{45}\cdot 354261+\frac{1}{45}\cdot 534162+\frac{1}{45}\cdot 534261+\frac{1}{15}\cdot 623415\\
&+\frac{2}{45}\cdot 632415+\frac{1}{45}\cdot 623514+\frac{1}{45}\cdot 624315+\frac{1}{45}\cdot 642315+\frac{4}{15}\cdot 345612+\frac{4}{15}\cdot 345621\\
&+\frac{2}{15}\cdot 346512+\frac{2}{15}\cdot 346521-\frac{2}{45}\cdot 352461+\frac{2}{15}\cdot 354612+\frac{2}{15}\cdot 354621+\frac{4}{45}\cdot 364512\\
&+\frac{4}{45}\cdot 364521-\frac{2}{45}\cdot 425361+\frac{2}{15}\cdot 435612+\frac{2}{15}\cdot 435621+\frac{4}{15}\cdot 623451+\frac{2}{15}\cdot 623541\\
&+\frac{2}{15}\cdot 624351+\frac{4}{45}\cdot 625341+\frac{2}{15}\cdot 632451+\frac{1}{45}\cdot 362451+\frac{1}{45}\cdot 364152+\frac{1}{45}\cdot 364251\\
&+\frac{1}{15}\cdot 523461+\frac{1}{45}\cdot 523641+\frac{1}{45}\cdot 524613+\frac{1}{45}\cdot 524631+\frac{4}{45}\cdot 534612+\frac{4}{45}\cdot 534621\\
&+\frac{4}{45}\cdot 642351-\frac{2}{45}\cdot 356124-\frac{2}{45}\cdot 365124+\frac{2}{45}\cdot 356142+\frac{2}{45}\cdot 356241+\frac{2}{45}\cdot 365142\\
&+\frac{2}{45}\cdot 365241+\frac{1}{15}\cdot 426135-\frac{1}{45}\cdot 426513-\frac{1}{45}\cdot 436152-\frac{1}{45}\cdot 436251+\frac{1}{45}\cdot 625134\\
&+\frac{1}{45}\cdot 625314+\frac{2}{45}\cdot 624513+\frac{2}{45}\cdot 625413-\frac{1}{45}\cdot 632514-\frac{2}{45}\cdot 436125-\frac{2}{45}\cdot 624135\\
&-\frac{2}{45}\cdot 256143-\frac{2}{45}\cdot 265143+\frac{2}{45}\cdot 356412+\frac{2}{45}\cdot 356421+\frac{2}{45}\cdot 365412+\frac{2}{45}\cdot 365421\\
&-\frac{1}{45}\cdot 426531+\frac{2}{45}\cdot 436512+\frac{2}{45}\cdot 436521+\frac{2}{45}\cdot 624531+\frac{2}{45}\cdot 625431+\frac{2}{45}\cdot 632541\\
&-\frac{1}{45}\cdot 531246-\frac{4}{45}\cdot 451236-\frac{4}{45}\cdot 451263-\frac{4}{45}\cdot 541236-\frac{4}{45}\cdot 541263-\frac{2}{45}\cdot 631425\\
&-\frac{2}{45}\cdot 452136-\frac{2}{45}\cdot 542136+\frac{2}{45}\cdot 452361+\frac{2}{45}\cdot 542361+\frac{1}{15}\cdot 461235+\frac{1}{15}\cdot 641235\\
&+\frac{2}{45}\cdot 634125+\frac{2}{45}\cdot 643125-\frac{2}{45}\cdot 451623-\frac{2}{45}\cdot 541623+\frac{2}{45}\cdot 452613+\frac{2}{45}\cdot 452631\\
&+\frac{2}{45}\cdot 542613+\frac{2}{45}\cdot 542631+\frac{1}{45}\cdot 641253+\frac{1}{45}\cdot 641352-\frac{1}{45}\cdot 631542+\frac{2}{45}\cdot 634152\\
&+\frac{2}{45}\cdot 643152-\frac{2}{45}\cdot 452163-\frac{2}{45}\cdot 542163+\frac{2}{45}\cdot 453612+\frac{2}{45}\cdot 453621+\frac{2}{45}\cdot 543612\\
&+\frac{2}{45}\cdot 543621+\frac{2}{45}\cdot 634251+\frac{2}{45}\cdot 643251+\frac{4}{15}\cdot 561234+\frac{2}{15}\cdot 561243+\frac{4}{15}\cdot 651234\\
&+\frac{2}{15}\cdot 651243+\frac{2}{15}\cdot 561324+\frac{4}{45}\cdot 561423+\frac{2}{15}\cdot 651324+\frac{4}{45}\cdot 651423+\frac{2}{15}\cdot 562134
\end{aligned}
$$

$$
\begin{aligned}
&+ \frac{2}{15} \cdot 652134 + \frac{4}{45} \cdot 563124 + \frac{4}{45} \cdot 653124 + \frac{2}{45} \cdot 561342 + \frac{2}{45} \cdot 561432 + \frac{2}{45} \cdot 651342 \\
&+ \frac{2}{45} \cdot 651432 + \frac{2}{45} \cdot 562143 + \frac{2}{45} \cdot 652143 + \frac{2}{45} \cdot 562314 + \frac{2}{45} \cdot 563214 + \frac{2}{45} \cdot 652314 \\
&+ \frac{2}{45} \cdot 653214
\end{aligned}
$$

$$
\begin{aligned}
\llbracket x_3 \times x_4 \rrbracket = &\frac{2}{45} \cdot 132465 + \frac{2}{45} \cdot 134265 + \frac{1}{45} \cdot 134625 + \frac{4}{45} \cdot 142365 + \frac{2}{45} \cdot 213546 + \frac{1}{45} \cdot 213645 \\
&+ \frac{4}{45} \cdot 231546 + \frac{8}{45} \cdot 231645 - \frac{1}{45} \cdot 235146 + \frac{1}{9} \cdot 236145 + \frac{2}{45} \cdot 213465 + \frac{2}{15} \cdot 214365 \\
&+ \frac{1}{9} \cdot 241635 - \frac{1}{45} \cdot 246135 + \frac{4}{45} \cdot 312546 + \frac{8}{45} \cdot 312645 + \frac{1}{15} \cdot 213654 + \frac{1}{5} \cdot 231654 \\
&+ \frac{1}{15} \cdot 236154 + \frac{1}{9} \cdot 241653 + \frac{1}{30} \cdot 246153 + \frac{1}{45} \cdot 213564 + \frac{8}{45} \cdot 231564 + \frac{1}{5} \cdot 312654 \\
&+ \frac{8}{45} \cdot 312564 - \frac{1}{15} \cdot 235416 - \frac{1}{45} \cdot 236415 - \frac{1}{15} \cdot 234165 - \frac{1}{15} \cdot 234615 - \frac{1}{45} \cdot 243165 \\
&- \frac{2}{15} \cdot 243615 + \frac{4}{45} \cdot 231465 - \frac{1}{9} \cdot 235461 - \frac{1}{15} \cdot 236451 - \frac{1}{15} \cdot 234651 - \frac{8}{45} \cdot 243651 \\
&- \frac{1}{45} \cdot 236514 + \frac{1}{30} \cdot 246513 - \frac{1}{15} \cdot 235614 - \frac{1}{15} \cdot 251364 + \frac{1}{30} \cdot 253164 - \frac{2}{15} \cdot 261354 \\
&+ \frac{2}{45} \cdot 263154 - \frac{1}{15} \cdot 236541 + \frac{1}{90} \cdot 246531 - \frac{1}{15} \cdot 235641 - \frac{1}{45} \cdot 512436 - \frac{1}{15} \cdot 314625 \\
&- \frac{1}{15} \cdot 412365 + \frac{1}{45} \cdot 413265 + \frac{4}{45} \cdot 312465 - \frac{2}{15} \cdot 314652 + \frac{1}{45} \cdot 412653 + \frac{1}{45} \cdot 413652 \\
&+ \frac{1}{15} \cdot 412563 + \frac{1}{30} \cdot 516243 - \frac{1}{15} \cdot 512634 - \frac{1}{9} \cdot 612435 - \frac{1}{15} \cdot 612534 - \frac{1}{15} \cdot 512364 \\
&- \frac{4}{45} \cdot 513264 - \frac{1}{15} \cdot 612354 - \frac{8}{45} \cdot 613254 - \frac{1}{45} \cdot 512643 + \frac{1}{90} \cdot 513642 - \frac{1}{15} \cdot 612543 \\
&+ \frac{1}{90} \cdot 613542 - \frac{1}{30} \cdot 514263 - \frac{1}{15} \cdot 612453 + \frac{2}{45} \cdot 124365 + \frac{1}{15} \cdot 125364 + \frac{1}{15} \cdot 215364 \\
&+ \frac{2}{45} \cdot 124635 + \frac{1}{45} \cdot 124653 + \frac{2}{45} \cdot 214635 + \frac{1}{45} \cdot 126354 + \frac{2}{45} \cdot 132546 + \frac{1}{45} \cdot 132564 \\
&+ \frac{1}{15} \cdot 142536 + \frac{1}{45} \cdot 132645 + \frac{1}{15} \cdot 132654 + \frac{1}{45} \cdot 142653 + \frac{2}{45} \cdot 135246 + \frac{1}{45} \cdot 135426 \\
&+ \frac{1}{45} \cdot 135264 + \frac{1}{15} \cdot 324165 - \frac{1}{90} \cdot 135624 - \frac{1}{30} \cdot 135642 - \frac{1}{9} \cdot 324615 - \frac{2}{9} \cdot 324651 \\
&+ \frac{1}{45} \cdot 136245 + \frac{2}{45} \cdot 136254 - \frac{1}{30} \cdot 136452 - \frac{1}{30} \cdot 136542 + \frac{1}{90} \cdot 136524 + \frac{1}{45} \cdot 152436 \\
&- \frac{1}{90} \cdot 152463 + \frac{1}{45} \cdot 421365 - \frac{1}{9} \cdot 521364 - \frac{1}{30} \cdot 152634 - \frac{1}{90} \cdot 152643 - \frac{1}{30} \cdot 162453 \\
&- \frac{2}{9} \cdot 621354 - \frac{1}{30} \cdot 162534 - \frac{1}{30} \cdot 162543 + \frac{2}{45} \cdot 214356 + \frac{1}{45} \cdot 214536 + \frac{1}{15} \cdot 314256 \\
&+ \frac{1}{15} \cdot 314265 + \frac{1}{15} \cdot 215346 + \frac{2}{15} \cdot 215436 + \frac{2}{45} \cdot 216435 + \frac{4}{45} \cdot 315264 + \frac{1}{45} \cdot 315426 \\
&+ \frac{1}{90} \cdot 316425 + \frac{2}{45} \cdot 241356 + \frac{2}{45} \cdot 241365 + \frac{2}{45} \cdot 241536 - \frac{7}{45} \cdot 243561 - \frac{1}{90} \cdot 245136 \\
&- \frac{1}{30} \cdot 245316 - \frac{1}{30} \cdot 246315 - \frac{4}{45} \cdot 245361 - \frac{1}{45} \cdot 251346 + \frac{1}{15} \cdot 254163 + \frac{1}{30} \cdot 254613 \\
&- \frac{2}{15} \cdot 261435 - \frac{1}{90} \cdot 253416 - \frac{2}{45} \cdot 253461 - \frac{1}{30} \cdot 254316 - \frac{1}{15} \cdot 254361 + \frac{1}{90} \cdot 254136
\end{aligned}
$$

$$- \frac{1}{18} \cdot 264135 + \frac{1}{45} \cdot 264315 + \frac{1}{90} \cdot 264351 + \frac{2}{45} \cdot 413256 + \frac{1}{45} \cdot 513624 + \frac{1}{90} \cdot 413526$$
$$- \frac{2}{15} \cdot 315462 - \frac{7}{90} \cdot 415236 - \frac{1}{18} \cdot 415326 + \frac{1}{15} \cdot 416325 + \frac{1}{30} \cdot 516324 - \frac{1}{18} \cdot 513426$$
$$- \frac{7}{45} \cdot 613245 - \frac{4}{45} \cdot 613425 - \frac{1}{30} \cdot 514236 - \frac{1}{30} \cdot 514326 - \frac{2}{45} \cdot 614235 - \frac{1}{15} \cdot 614325$$
$$+ \frac{1}{90} \cdot 615324 + \frac{2}{45} \cdot 125346 + \frac{1}{15} \cdot 125436 - \frac{2}{45} \cdot 351426 + \frac{1}{15} \cdot 125463 + \frac{2}{45} \cdot 215463$$
$$+ \frac{1}{15} \cdot 126435 + \frac{1}{15} \cdot 142356 + \frac{2}{15} \cdot 143256 + \frac{4}{45} \cdot 143526 + \frac{1}{5} \cdot 143265 + \frac{4}{45} \cdot 143625$$
$$+ \frac{1}{18} \cdot 413625 - \frac{1}{45} \cdot 145326 - \frac{2}{45} \cdot 243516 + \frac{2}{45} \cdot 325146 - \frac{2}{45} \cdot 325416 - \frac{1}{18} \cdot 145263$$
$$- \frac{1}{10} \cdot 145362 - \frac{4}{15} \cdot 325461 - \frac{2}{45} \cdot 415263 - \frac{1}{18} \cdot 415362 + \frac{1}{45} \cdot 142635 - \frac{7}{90} \cdot 146235$$
$$- \frac{1}{90} \cdot 146325 + \frac{2}{45} \cdot 143652 - \frac{1}{15} \cdot 146253 - \frac{2}{45} \cdot 146352 + \frac{2}{45} \cdot 153246 - \frac{2}{45} \cdot 513246$$
$$- \frac{2}{45} \cdot 521436 + \frac{1}{15} \cdot 153264 - \frac{1}{10} \cdot 163425 - \frac{4}{15} \cdot 621435 + \frac{2}{45} \cdot 163254 - \frac{2}{45} \cdot 163524$$
$$- \frac{1}{15} \cdot 214563 - \frac{2}{15} \cdot 314562 - \frac{1}{10} \cdot 316452 + \frac{1}{9} \cdot 241563 + \frac{1}{30} \cdot 245613 + \frac{1}{30} \cdot 245631$$
$$+ \frac{4}{45} \cdot 245163 - \frac{7}{90} \cdot 251634 - \frac{1}{18} \cdot 251643 - \frac{4}{45} \cdot 256134 - \frac{1}{15} \cdot 256143 - \frac{1}{90} \cdot 251463$$
$$- \frac{1}{10} \cdot 261453 + \frac{2}{45} \cdot 256341 + \frac{1}{45} \cdot 256431 + \frac{1}{90} \cdot 254631 - \frac{1}{45} \cdot 264153 + \frac{1}{45} \cdot 264531$$
$$+ \frac{2}{45} \cdot 413562 - \frac{2}{45} \cdot 415623 - \frac{1}{45} \cdot 415632 + \frac{1}{30} \cdot 613452 + \frac{2}{45} \cdot 513462 + \frac{2}{45} \cdot 614523$$
$$+ \frac{1}{45} \cdot 614532 + \frac{1}{90} \cdot 614352 + \frac{1}{45} \cdot 615342 - \frac{1}{45} \cdot 351462 + \frac{4}{45} \cdot 125634 + \frac{2}{45} \cdot 125643$$
$$+ \frac{2}{45} \cdot 126453 + \frac{2}{45} \cdot 361452 + \frac{2}{45} \cdot 325164 - \frac{2}{15} \cdot 145623 - \frac{2}{15} \cdot 145632 - \frac{1}{5} \cdot 325614$$
$$- \frac{11}{45} \cdot 325641 - \frac{1}{15} \cdot 146523 - \frac{1}{15} \cdot 146532 - \frac{2}{45} \cdot 246351 - \frac{1}{18} \cdot 153462 - \frac{1}{15} \cdot 521463$$
$$- \frac{1}{45} \cdot 153624 - \frac{1}{45} \cdot 153642 - \frac{2}{15} \cdot 163452 - \frac{11}{45} \cdot 621453 - \frac{1}{15} \cdot 163542 - \frac{2}{45} \cdot 613524$$
$$- \frac{1}{90} \cdot 136425 - \frac{1}{15} \cdot 216345 + \frac{1}{90} \cdot 253146 - \frac{2}{15} \cdot 261345 + \frac{1}{15} \cdot 263145 + \frac{2}{45} \cdot 315246$$
$$+ \frac{1}{15} \cdot 316245 + \frac{1}{15} \cdot 316254 - \frac{7}{90} \cdot 315624 - \frac{1}{18} \cdot 316524 + \frac{1}{15} \cdot 263415 + \frac{1}{30} \cdot 263451$$
$$+ \frac{1}{90} \cdot 263514 + \frac{1}{45} \cdot 256314 - \frac{1}{15} \cdot 265134 + \frac{1}{45} \cdot 265314 + \frac{1}{90} \cdot 263541 + \frac{1}{45} \cdot 265341$$
$$+ \frac{2}{45} \cdot 416235 + \frac{1}{30} \cdot 416253 - \frac{1}{45} \cdot 416523 + \frac{1}{30} \cdot 516234 + \frac{1}{30} \cdot 615234 + \frac{1}{90} \cdot 615243$$
$$+ \frac{1}{45} \cdot 615423 + \frac{2}{45} \cdot 126534 - \frac{4}{45} \cdot 326415 - \frac{11}{45} \cdot 326451 - \frac{1}{45} \cdot 253641 + \frac{1}{45} \cdot 154236$$
$$- \frac{1}{18} \cdot 164235 + \frac{2}{45} \cdot 421635 - \frac{1}{45} \cdot 164253 + \frac{1}{90} \cdot 154263 - \frac{2}{15} \cdot 156234 - \frac{2}{15} \cdot 165234$$
$$- \frac{7}{45} \cdot 521634 - \frac{11}{45} \cdot 621534 - \frac{1}{15} \cdot 156243 - \frac{1}{15} \cdot 165243 - \frac{1}{45} \cdot 614253 + \frac{1}{15} \cdot 312456$$
$$+ \frac{1}{5} \cdot 321456 + \frac{4}{15} \cdot 321465 + \frac{4}{45} \cdot 324156 + \frac{4}{15} \cdot 321546 + \frac{1}{3} \cdot 321564 + \frac{1}{3} \cdot 321645$$
$$+ \frac{4}{45} \cdot 326145 - \frac{4}{45} \cdot 341256 - \frac{2}{45} \cdot 342156 - \frac{1}{5} \cdot 324561 - \frac{1}{45} \cdot 324516 - \frac{1}{10} \cdot 341526$$

$$
\begin{aligned}
&-\frac{1}{15}\cdot 341562-\frac{1}{10}\cdot 342516-\frac{4}{45}\cdot 342561-\frac{7}{90}\cdot 351246-\frac{1}{90}\cdot 352146-\frac{1}{9}\cdot 361245\\
&-\frac{2}{45}\cdot 362145-\frac{1}{10}\cdot 315642-\frac{2}{45}\cdot 352416-\frac{1}{30}\cdot 362415+\frac{2}{45}\cdot 421356-\frac{2}{45}\cdot 423156\\
&+\frac{1}{15}\cdot 421536+\frac{4}{45}\cdot 421563+\frac{1}{18}\cdot 526134-\frac{1}{5}\cdot 621345-\frac{1}{15}\cdot 521346-\frac{7}{90}\cdot 523146\\
&-\frac{4}{45}\cdot 623145-\frac{2}{45}\cdot 524136+\frac{1}{45}\cdot 134256+\frac{1}{15}\cdot 231456+\frac{1}{90}\cdot 425163-\frac{7}{90}\cdot 423516\\
&-\frac{2}{45}\cdot 423561+\frac{1}{90}\cdot 425613-\frac{1}{90}\cdot 425631-\frac{2}{45}\cdot 431256-\frac{1}{30}\cdot 431526-\frac{2}{45}\cdot 431562\\
&-\frac{2}{45}\cdot 631245-\frac{1}{90}\cdot 631452-\frac{1}{10}\cdot 261534+\frac{2}{5}\cdot 321654+\frac{1}{15}\cdot 426153-\frac{8}{45}\cdot 341265\\
&-\frac{4}{45}\cdot 342165-\frac{11}{90}\cdot 351264-\frac{1}{30}\cdot 352164-\frac{11}{90}\cdot 341625-\frac{2}{15}\cdot 341652-\frac{7}{90}\cdot 342615\\
&-\frac{2}{15}\cdot 342651-\frac{1}{15}\cdot 351624-\frac{7}{90}\cdot 351642-\frac{1}{30}\cdot 352614-\frac{1}{15}\cdot 352641+\frac{4}{45}\cdot 326154\\
&-\frac{8}{45}\cdot 361254-\frac{1}{15}\cdot 362154-\frac{1}{10}\cdot 316542-\frac{1}{5}\cdot 326541-\frac{1}{9}\cdot 326514-\frac{7}{90}\cdot 361524\\
&-\frac{2}{45}\cdot 361542-\frac{1}{45}\cdot 362514-\frac{1}{90}\cdot 362541-\frac{4}{45}\cdot 423165-\frac{1}{10}\cdot 523164-\frac{2}{45}\cdot 524163\\
&-\frac{1}{15}\cdot 521643+\frac{1}{18}\cdot 526143-\frac{2}{15}\cdot 623154-\frac{1}{15}\cdot 624153-\frac{1}{5}\cdot 621543-\frac{1}{90}\cdot 625143\\
&+\frac{4}{45}\cdot 421653-\frac{1}{18}\cdot 423615-\frac{4}{45}\cdot 423651+\frac{1}{90}\cdot 426513-\frac{1}{45}\cdot 426315-\frac{4}{45}\cdot 431265\\
&-\frac{7}{90}\cdot 431625-\frac{1}{15}\cdot 431652-\frac{4}{45}\cdot 631254-\frac{1}{10}\cdot 261543+\frac{1}{18}\cdot 426135-\frac{1}{30}\cdot 426531\\
&-\frac{7}{90}\cdot 531264-\frac{7}{90}\cdot 531624-\frac{2}{45}\cdot 531642-\frac{1}{30}\cdot 631542-\frac{1}{15}\cdot 345126-\frac{1}{15}\cdot 345216\\
&-\frac{1}{15}\cdot 346125-\frac{1}{45}\cdot 346215-\frac{2}{45}\cdot 352461-\frac{1}{15}\cdot 354126-\frac{1}{15}\cdot 354216-\frac{1}{45}\cdot 364125\\
&-\frac{1}{45}\cdot 364215+\frac{4}{45}\cdot 523614-\frac{1}{45}\cdot 425316+\frac{1}{18}\cdot 526314-\frac{1}{15}\cdot 523416-\frac{2}{45}\cdot 524316\\
&-\frac{2}{45}\cdot 624135+\frac{1}{45}\cdot 435126+\frac{1}{45}\cdot 435216+\frac{1}{10}\cdot 345162+\frac{1}{10}\cdot 345261+\frac{1}{18}\cdot 435162\\
&+\frac{1}{18}\cdot 435261+\frac{1}{18}\cdot 346152+\frac{7}{90}\cdot 346251+\frac{1}{10}\cdot 623415+\frac{1}{18}\cdot 632415+\frac{7}{90}\cdot 623514\\
&+\frac{4}{15}\cdot 345612+\frac{4}{15}\cdot 345621+\frac{8}{45}\cdot 346512+\frac{8}{45}\cdot 346521-\frac{2}{45}\cdot 356124+\frac{2}{15}\cdot 354612\\
&+\frac{2}{15}\cdot 354621+\frac{4}{45}\cdot 356412+\frac{4}{45}\cdot 356421+\frac{4}{45}\cdot 364512+\frac{4}{45}\cdot 364521-\frac{1}{45}\cdot 425361\\
&-\frac{1}{15}\cdot 426351+\frac{4}{15}\cdot 623451+\frac{8}{45}\cdot 623541+\frac{1}{30}\cdot 524613+\frac{2}{15}\cdot 624351+\frac{4}{45}\cdot 624531\\
&+\frac{4}{45}\cdot 625341+\frac{1}{30}\cdot 354162+\frac{1}{30}\cdot 354261+\frac{1}{90}\cdot 362451+\frac{1}{30}\cdot 364152+\frac{1}{30}\cdot 364251\\
&+\frac{1}{10}\cdot 523461+\frac{1}{30}\cdot 524361+\frac{1}{18}\cdot 523641+\frac{1}{30}\cdot 524631+\frac{4}{45}\cdot 435612+\frac{4}{45}\cdot 435621\\
&+\frac{1}{90}\cdot 532461+\frac{4}{45}\cdot 632451-\frac{1}{45}\cdot 365124+\frac{1}{45}\cdot 365214+\frac{1}{45}\cdot 356142+\frac{2}{45}\cdot 356241\\
&+\frac{1}{45}\cdot 365142+\frac{2}{45}\cdot 365241+\frac{1}{90}\cdot 625134+\frac{1}{30}\cdot 625314+\frac{2}{45}\cdot 624513+\frac{2}{45}\cdot 625413\\
&+\frac{7}{90}\cdot 461325+\frac{1}{18}\cdot 461352+\frac{1}{18}\cdot 462135+\frac{1}{30}\cdot 462153-\frac{1}{45}\cdot 462315+\frac{1}{45}\cdot 462513
\end{aligned}
$$

$$
\begin{aligned}
&- \frac{1}{15}\cdot 436125 - \frac{1}{90}\cdot 436152 - \frac{1}{15}\cdot 631524 - \frac{2}{45}\cdot 265143 + \frac{1}{15}\cdot 365412 + \frac{1}{15}\cdot 365421\\
&+ \frac{1}{45}\cdot 526413 + \frac{1}{15}\cdot 625431 - \frac{1}{18}\cdot 531246 - \frac{1}{45}\cdot 531426 - \frac{1}{30}\cdot 531462 - \frac{1}{15}\cdot 451236\\
&- \frac{1}{15}\cdot 451263 - \frac{1}{15}\cdot 541236 - \frac{1}{15}\cdot 541263 - \frac{1}{45}\cdot 451326 - \frac{1}{45}\cdot 541326 - \frac{1}{45}\cdot 631425\\
&+ \frac{1}{10}\cdot 461235 + \frac{1}{10}\cdot 641235 + \frac{1}{30}\cdot 641325 + \frac{1}{18}\cdot 461253 + \frac{1}{18}\cdot 641253 + \frac{1}{30}\cdot 641352\\
&+ \frac{1}{45}\cdot 526341 + \frac{1}{45}\cdot 526431 - \frac{2}{45}\cdot 451623 - \frac{1}{45}\cdot 451632 - \frac{2}{45}\cdot 541623 - \frac{1}{45}\cdot 541632\\
&+ \frac{1}{45}\cdot 461523 + \frac{1}{45}\cdot 461532 + \frac{1}{45}\cdot 641523 + \frac{1}{45}\cdot 641532 - \frac{1}{30}\cdot 154362 - \frac{1}{45}\cdot 154623\\
&- \frac{1}{45}\cdot 154632 - \frac{1}{45}\cdot 164352 - \frac{1}{30}\cdot 432516 - \frac{1}{15}\cdot 432561 - \frac{1}{30}\cdot 432615 - \frac{1}{15}\cdot 432651\\
&- \frac{1}{90}\cdot 532641 + \frac{1}{45}\cdot 534162 + \frac{1}{45}\cdot 534261 + \frac{2}{45}\cdot 534612 + \frac{2}{45}\cdot 534621 - \frac{1}{45}\cdot 436215\\
&- \frac{1}{45}\cdot 536124 - \frac{1}{45}\cdot 536214 + \frac{1}{90}\cdot 436251 + \frac{2}{45}\cdot 436512 + \frac{2}{45}\cdot 436521 + \frac{1}{45}\cdot 536412\\
&+ \frac{1}{45}\cdot 536421 + \frac{2}{45}\cdot 452361 + \frac{2}{45}\cdot 542361 + \frac{1}{45}\cdot 452613 + \frac{1}{45}\cdot 452631 + \frac{1}{45}\cdot 542613\\
&+ \frac{1}{45}\cdot 542631 + \frac{2}{45}\cdot 642351 + \frac{2}{45}\cdot 632541 + \frac{1}{45}\cdot 642531 + \frac{4}{15}\cdot 561234 + \frac{8}{45}\cdot 561243\\
&+ \frac{4}{15}\cdot 651234 + \frac{8}{45}\cdot 651243 + \frac{2}{15}\cdot 561324 + \frac{4}{45}\cdot 561342 + \frac{2}{15}\cdot 651324 + \frac{4}{45}\cdot 651342\\
&+ \frac{4}{45}\cdot 561423 + \frac{4}{45}\cdot 651423 + \frac{1}{30}\cdot 624315 + \frac{1}{90}\cdot 642135 + \frac{4}{45}\cdot 562134 + \frac{4}{45}\cdot 652134\\
&+ \frac{1}{15}\cdot 561432 + \frac{1}{15}\cdot 651432 - \frac{1}{30}\cdot 164325 - \frac{1}{45}\cdot 156324 - \frac{1}{45}\cdot 165324 - \frac{1}{30}\cdot 532146\\
&- \frac{1}{15}\cdot 632145 - \frac{1}{15}\cdot 632154 - \frac{1}{90}\cdot 642153 - \frac{1}{30}\cdot 532164 + \frac{1}{45}\cdot 642315 + \frac{1}{90}\cdot 632514\\
&- \frac{1}{45}\cdot 452136 - \frac{1}{45}\cdot 542136 + \frac{2}{45}\cdot 634125 + \frac{2}{45}\cdot 643125 + \frac{1}{45}\cdot 634152 + \frac{1}{45}\cdot 643152\\
&- \frac{1}{45}\cdot 452163 - \frac{1}{45}\cdot 542163 + \frac{2}{45}\cdot 563124 + \frac{2}{45}\cdot 653124 + \frac{2}{45}\cdot 562143 + \frac{1}{45}\cdot 563142\\
&+ \frac{2}{45}\cdot 652143 + \frac{1}{45}\cdot 653142
\end{aligned}
$$

$$
\begin{aligned}
[\![x_3 \times x_5]\!] = &- \frac{4}{45}\cdot 123654 - \frac{4}{45}\cdot 132654 - \frac{2}{45}\cdot 146253 - \frac{1}{45}\cdot 123564 - \frac{1}{45}\cdot 124536 - \frac{1}{45}\cdot 125436\\
&- \frac{1}{45}\cdot 142635 + \frac{2}{45}\cdot 126453 + \frac{1}{45}\cdot 134652 + \frac{2}{45}\cdot 143652 + \frac{4}{45}\cdot 125634 + \frac{2}{45}\cdot 126534\\
&+ \frac{1}{45}\cdot 162435 - \frac{1}{45}\cdot 213645 + \frac{2}{45}\cdot 231546 - \frac{2}{45}\cdot 235146 + \frac{1}{45}\cdot 236145 + \frac{2}{45}\cdot 231465\\
&+ \frac{2}{45}\cdot 234615 + \frac{2}{45}\cdot 341652 + \frac{1}{90}\cdot 346152 - \frac{1}{45}\cdot 412563 - \frac{2}{45}\cdot 412653 - \frac{1}{90}\cdot 516243\\
&+ \frac{2}{45}\cdot 342651 + \frac{1}{30}\cdot 346251 - \frac{1}{90}\cdot 514263 + \frac{1}{45}\cdot 521364 - \frac{1}{90}\cdot 523164 + \frac{2}{45}\cdot 623154\\
&+ \frac{1}{30}\cdot 623514 - \frac{1}{45}\cdot 123645 - \frac{4}{45}\cdot 213654 + \frac{2}{45}\cdot 125643 - \frac{1}{45}\cdot 132564 - \frac{1}{45}\cdot 142563\\
&+ \frac{2}{45}\cdot 312465 + \frac{2}{45}\cdot 324165 + \frac{1}{90}\cdot 136524 + \frac{1}{90}\cdot 136542 + \frac{1}{45}\cdot 236514 + \frac{2}{45}\cdot 142365
\end{aligned}
$$

$$
\begin{aligned}
&-\frac{1}{45}\cdot 152364-\frac{1}{90}\cdot 152463+\frac{2}{45}\cdot 512364-\frac{1}{45}\cdot 512463-\frac{2}{45}\cdot 142653+\frac{2}{45}\cdot 241653\\
&-\frac{1}{90}\cdot 341625-\frac{1}{90}\cdot 152643+\frac{1}{45}\cdot 512643+\frac{1}{45}\cdot 143625+\frac{2}{45}\cdot 243651+\frac{1}{90}\cdot 342615\\
&+\frac{1}{90}\cdot 162543+\frac{2}{45}\cdot 163254+\frac{1}{15}\cdot 263154+\frac{2}{45}\cdot 613254+\frac{1}{45}\cdot 125346-\frac{1}{45}\cdot 135264\\
&+\frac{2}{45}\cdot 143256+\frac{2}{45}\cdot 143265+\frac{1}{45}\cdot 135462-\frac{1}{45}\cdot 145326+\frac{1}{45}\cdot 163245-\frac{1}{45}\cdot 214536\\
&-\frac{1}{45}\cdot 314526+\frac{1}{90}\cdot 254136+\frac{1}{90}\cdot 254316+\frac{1}{45}\cdot 254361-\frac{1}{30}\cdot 264135-\frac{1}{90}\cdot 264351\\
&+\frac{2}{45}\cdot 312546-\frac{1}{45}\cdot 412536+\frac{1}{90}\cdot 413526-\frac{2}{45}\cdot 315426-\frac{1}{18}\cdot 415326+\frac{1}{45}\cdot 416325\\
&-\frac{1}{90}\cdot 516324-\frac{1}{45}\cdot 325146-\frac{2}{45}\cdot 325416-\frac{2}{45}\cdot 325461+\frac{1}{90}\cdot 514326+\frac{1}{45}\cdot 614325\\
&-\frac{1}{90}\cdot 615324-\frac{2}{45}\cdot 521436-\frac{2}{45}\cdot 621435-\frac{1}{45}\cdot 124635-\frac{1}{45}\cdot 214635-\frac{1}{45}\cdot 135246\\
&+\frac{1}{45}\cdot 215346-\frac{1}{45}\cdot 215436+\frac{2}{45}\cdot 142356+\frac{2}{45}\cdot 143526-\frac{2}{45}\cdot 235416-\frac{1}{30}\cdot 415236\\
&-\frac{1}{45}\cdot 146352-\frac{1}{45}\cdot 246351-\frac{1}{45}\cdot 513246+\frac{1}{90}\cdot 513426-\frac{1}{18}\cdot 251463+\frac{1}{45}\cdot 254163\\
&-\frac{2}{45}\cdot 351462-\frac{1}{90}\cdot 354162+\frac{2}{45}\cdot 513264+\frac{1}{90}\cdot 153462+\frac{1}{90}\cdot 154362+\frac{2}{45}\cdot 253461\\
&-\frac{1}{45}\cdot 163524-\frac{1}{45}\cdot 613524+\frac{1}{90}\cdot 164235+\frac{1}{90}\cdot 164325+\frac{2}{45}\cdot 614235+\frac{1}{45}\cdot 143562\\
&-\frac{1}{45}\cdot 145623-\frac{1}{45}\cdot 145632-\frac{2}{45}\cdot 163452-\frac{2}{45}\cdot 163542-\frac{1}{45}\cdot 214653-\frac{1}{45}\cdot 213564\\
&-\frac{1}{45}\cdot 314562-\frac{1}{90}\cdot 254613-\frac{1}{90}\cdot 254631+\frac{1}{45}\cdot 413562-\frac{1}{45}\cdot 315264+\frac{1}{30}\cdot 315624\\
&-\frac{1}{90}\cdot 315642-\frac{1}{30}\cdot 415362+\frac{1}{45}\cdot 416352-\frac{1}{45}\cdot 325164-\frac{1}{45}\cdot 325614-\frac{1}{15}\cdot 325641\\
&-\frac{1}{45}\cdot 514362-\frac{1}{90}\cdot 614352-\frac{2}{45}\cdot 521463-\frac{1}{15}\cdot 621453-\frac{1}{45}\cdot 124653-\frac{1}{45}\cdot 135426\\
&+\frac{1}{45}\cdot 125463+\frac{1}{45}\cdot 215463+\frac{1}{30}\cdot 135624+\frac{1}{30}\cdot 135642+\frac{1}{30}\cdot 136452+\frac{1}{15}\cdot 241563\\
&-\frac{1}{90}\cdot 145263-\frac{1}{30}\cdot 145362-\frac{2}{45}\cdot 235164-\frac{1}{45}\cdot 415263-\frac{1}{45}\cdot 146523-\frac{1}{45}\cdot 146532\\
&-\frac{1}{45}\cdot 513462+\frac{1}{90}\cdot 152634+\frac{1}{30}\cdot 251634+\frac{1}{90}\cdot 251643+\frac{1}{30}\cdot 513642+\frac{1}{45}\cdot 154623\\
&+\frac{1}{45}\cdot 154632-\frac{1}{45}\cdot 253614+\frac{1}{30}\cdot 352614+\frac{1}{45}\cdot 162354+\frac{1}{45}\cdot 154236-\frac{1}{45}\cdot 132645\\
&-\frac{1}{90}\cdot 136425-\frac{1}{45}\cdot 156234-\frac{1}{45}\cdot 165234-\frac{2}{45}\cdot 251346+\frac{1}{90}\cdot 253146-\frac{1}{45}\cdot 261345\\
&+\frac{2}{45}\cdot 263145+\frac{1}{45}\cdot 216435-\frac{2}{45}\cdot 236415-\frac{1}{90}\cdot 316452-\frac{2}{45}\cdot 361452-\frac{1}{90}\cdot 364152\\
&+\frac{1}{45}\cdot 415623+\frac{1}{45}\cdot 416523-\frac{1}{15}\cdot 326451-\frac{1}{30}\cdot 362451-\frac{1}{90}\cdot 364251+\frac{1}{45}\cdot 521634\\
&+\frac{1}{90}\cdot 526134+\frac{1}{90}\cdot 526314-\frac{1}{15}\cdot 621534-\frac{1}{30}\cdot 625134-\frac{1}{90}\cdot 625314-\frac{1}{45}\cdot 126354\\
&-\frac{1}{45}\cdot 216354-\frac{1}{45}\cdot 152436+\frac{1}{45}\cdot 126435-\frac{1}{45}\cdot 361425+\frac{1}{30}\cdot 162453+\frac{1}{30}\cdot 162534\\
&+\frac{1}{45}\cdot 316245-\frac{1}{30}\cdot 163425-\frac{1}{15}\cdot 326415-\frac{1}{30}\cdot 146235+\frac{1}{90}\cdot 154263+\frac{1}{90}\cdot 416253
\end{aligned}
$$

$$-\frac{1}{45}\cdot 156243-\frac{1}{45}\cdot 165243+\frac{1}{45}\cdot 156324+\frac{1}{45}\cdot 165324-\frac{1}{45}\cdot 241356-\frac{1}{45}\cdot 241365$$
$$+\frac{2}{45}\cdot 312456+\frac{1}{9}\cdot 321456+\frac{1}{9}\cdot 321465+\frac{2}{45}\cdot 324156-\frac{4}{45}\cdot 341256-\frac{2}{45}\cdot 342156$$
$$-\frac{1}{30}\cdot 316425-\frac{1}{45}\cdot 351426-\frac{1}{45}\cdot 352416-\frac{1}{45}\cdot 352461-\frac{1}{90}\cdot 362415-\frac{2}{45}\cdot 423156$$
$$+\frac{1}{45}\cdot 421563-\frac{1}{45}\cdot 421635+\frac{1}{45}\cdot 425136+\frac{1}{30}\cdot 426135-\frac{1}{90}\cdot 423516+\frac{1}{45}\cdot 423561$$
$$+\frac{1}{90}\cdot 432516-\frac{1}{45}\cdot 524136-\frac{1}{45}\cdot 624135+\frac{1}{90}\cdot 531246+\frac{1}{90}\cdot 532146+\frac{1}{45}\cdot 631245$$
$$+\frac{2}{45}\cdot 231456+\frac{1}{9}\cdot 321546-\frac{2}{45}\cdot 243156-\frac{1}{45}\cdot 243516-\frac{1}{15}\cdot 251436-\frac{1}{18}\cdot 341526$$
$$-\frac{2}{45}\cdot 431256-\frac{1}{30}\cdot 431526-\frac{2}{45}\cdot 521346+\frac{1}{90}\cdot 435162+\frac{1}{30}\cdot 435261-\frac{1}{90}\cdot 261534$$
$$+\frac{1}{30}\cdot 632415-\frac{1}{15}\cdot 231654-\frac{1}{45}\cdot 136254+\frac{4}{45}\cdot 215634+\frac{2}{45}\cdot 215643+\frac{2}{45}\cdot 216453$$
$$-\frac{1}{90}\cdot 261453+\frac{1}{15}\cdot 321564-\frac{1}{90}\cdot 425163-\frac{4}{45}\cdot 341265-\frac{2}{45}\cdot 342165+\frac{1}{90}\cdot 316524$$
$$-\frac{1}{30}\cdot 316542-\frac{1}{45}\cdot 326514-\frac{1}{15}\cdot 326541-\frac{1}{90}\cdot 361524-\frac{2}{45}\cdot 361542-\frac{1}{90}\cdot 362541$$
$$-\frac{2}{45}\cdot 423165-\frac{1}{45}\cdot 524163-\frac{2}{45}\cdot 412635+\frac{1}{45}\cdot 521643+\frac{1}{30}\cdot 526143+\frac{1}{30}\cdot 423615$$
$$+\frac{4}{45}\cdot 423651+\frac{1}{30}\cdot 432615+\frac{1}{15}\cdot 432651-\frac{1}{15}\cdot 621543-\frac{1}{90}\cdot 625143+\frac{4}{45}\cdot 631254$$
$$+\frac{1}{15}\cdot 632154+\frac{2}{45}\cdot 216534+\frac{1}{15}\cdot 321645-\frac{1}{30}\cdot 436152+\frac{1}{90}\cdot 531264+\frac{1}{30}\cdot 532164$$
$$-\frac{1}{15}\cdot 312654+\frac{1}{90}\cdot 413625+\frac{2}{45}\cdot 413652-\frac{2}{45}\cdot 243165-\frac{2}{45}\cdot 431265-\frac{1}{90}\cdot 431625$$
$$+\frac{1}{45}\cdot 431652-\frac{1}{30}\cdot 261543+\frac{1}{45}\cdot 362154+\frac{1}{45}\cdot 326145+\frac{1}{90}\cdot 436251+\frac{1}{30}\cdot 352164$$
$$+\frac{1}{90}\cdot 632514+\frac{1}{30}\cdot 245136+\frac{2}{45}\cdot 245163+\frac{1}{30}\cdot 245316+\frac{1}{18}\cdot 253416-\frac{1}{30}\cdot 342516$$
$$-\frac{1}{45}\cdot 354126-\frac{1}{45}\cdot 354216-\frac{2}{45}\cdot 364125-\frac{2}{45}\cdot 364215+\frac{1}{15}\cdot 435126+\frac{1}{15}\cdot 435216$$
$$-\frac{1}{45}\cdot 524316+\frac{1}{45}\cdot 532416+\frac{1}{45}\cdot 324615+\frac{2}{45}\cdot 345126+\frac{2}{45}\cdot 345216+\frac{1}{90}\cdot 246153$$
$$-\frac{1}{90}\cdot 523146+\frac{1}{45}\cdot 523416-\frac{1}{90}\cdot 351264+\frac{1}{45}\cdot 452163-\frac{1}{90}\cdot 253164-\frac{1}{45}\cdot 453261$$
$$+\frac{1}{30}\cdot 263514-\frac{1}{45}\cdot 634215+\frac{1}{45}\cdot 235461+\frac{1}{45}\cdot 235614-\frac{1}{45}\cdot 243561-\frac{1}{30}\cdot 245613$$
$$-\frac{1}{30}\cdot 245631-\frac{1}{30}\cdot 263451-\frac{1}{90}\cdot 263541-\frac{1}{15}\cdot 324561+\frac{2}{45}\cdot 364512+\frac{2}{45}\cdot 364521$$
$$+\frac{1}{45}\cdot 415632-\frac{2}{45}\cdot 435612-\frac{2}{45}\cdot 435621+\frac{2}{45}\cdot 625341-\frac{1}{90}\cdot 531462-\frac{2}{45}\cdot 632451$$
$$+\frac{1}{15}\cdot 234651+\frac{1}{45}\cdot 341562-\frac{1}{45}\cdot 342561+\frac{1}{30}\cdot 345162+\frac{1}{30}\cdot 345261+\frac{2}{45}\cdot 346512$$
$$+\frac{2}{45}\cdot 346521+\frac{1}{30}\cdot 523461+\frac{1}{90}\cdot 524361-\frac{2}{45}\cdot 453612-\frac{2}{45}\cdot 453621+\frac{2}{45}\cdot 623541$$
$$-\frac{2}{45}\cdot 634251-\frac{1}{90}\cdot 146325-\frac{1}{45}\cdot 256134-\frac{1}{45}\cdot 265134-\frac{1}{30}\cdot 351246-\frac{1}{90}\cdot 352146$$
$$-\frac{1}{45}\cdot 361245+\frac{1}{45}\cdot 346215+\frac{1}{45}\cdot 356142+\frac{1}{45}\cdot 356241+\frac{1}{45}\cdot 365142+\frac{1}{45}\cdot 365241$$

$$
\begin{aligned}
&+\frac{1}{90}\cdot 461253+\frac{1}{90}\cdot 462153-\frac{1}{30}\cdot 425613-\frac{1}{90}\cdot 426513-\frac{1}{45}\cdot 462351-\frac{1}{45}\cdot 463251\\
&+\frac{1}{45}\cdot 624513+\frac{1}{45}\cdot 625413-\frac{1}{45}\cdot 536124-\frac{1}{45}\cdot 536214-\frac{1}{45}\cdot 635124-\frac{1}{45}\cdot 635214\\
&+\frac{1}{30}\cdot 461325+\frac{1}{90}\cdot 461352+\frac{1}{90}\cdot 462135-\frac{1}{90}\cdot 246315-\frac{1}{45}\cdot 462315-\frac{1}{45}\cdot 436125\\
&-\frac{1}{45}\cdot 463152+\frac{1}{45}\cdot 426153-\frac{1}{45}\cdot 256143-\frac{1}{45}\cdot 265143+\frac{1}{45}\cdot 356214+\frac{1}{45}\cdot 365214\\
&-\frac{1}{90}\cdot 246513-\frac{1}{90}\cdot 246531+\frac{2}{45}\cdot 356412+\frac{2}{45}\cdot 356421+\frac{2}{45}\cdot 365412+\frac{2}{45}\cdot 365421\\
&+\frac{1}{45}\cdot 416532+\frac{1}{45}\cdot 461523+\frac{1}{45}\cdot 461532-\frac{1}{18}\cdot 425631-\frac{1}{30}\cdot 426531-\frac{1}{45}\cdot 463512\\
&-\frac{1}{45}\cdot 463521+\frac{2}{45}\cdot 624531+\frac{2}{45}\cdot 625431-\frac{1}{45}\cdot 531642-\frac{1}{45}\cdot 536142-\frac{1}{45}\cdot 635241\\
&+\frac{1}{30}\cdot 514236+\frac{1}{45}\cdot 451326+\frac{1}{45}\cdot 541326+\frac{1}{45}\cdot 452136+\frac{1}{45}\cdot 542136+\frac{2}{45}\cdot 451236\\
&+\frac{2}{45}\cdot 541236+\frac{1}{45}\cdot 534162-\frac{1}{45}\cdot 351624-\frac{1}{90}\cdot 531624-\frac{1}{90}\cdot 532461-\frac{1}{90}\cdot 642135\\
&+\frac{1}{45}\cdot 512634-\frac{1}{45}\cdot 514623-\frac{1}{45}\cdot 514632-\frac{1}{45}\cdot 451362-\frac{1}{45}\cdot 541263-\frac{1}{45}\cdot 541362\\
&-\frac{1}{90}\cdot 351642-\frac{1}{90}\cdot 532641-\frac{1}{30}\cdot 631542-\frac{1}{90}\cdot 642153-\frac{1}{45}\cdot 541632-\frac{1}{18}\cdot 631452\\
&+\frac{1}{45}\cdot 452613+\frac{1}{45}\cdot 542613+\frac{1}{90}\cdot 523641-\frac{1}{90}\cdot 524613-\frac{1}{90}\cdot 524631+\frac{1}{90}\cdot 354261\\
&+\frac{1}{45}\cdot 542361-\frac{1}{45}\cdot 541623-\frac{1}{45}\cdot 543612-\frac{1}{45}\cdot 543621-\frac{1}{45}\cdot 643251+\frac{1}{45}\cdot 612435\\
&-\frac{1}{45}\cdot 613245-\frac{1}{30}\cdot 613452-\frac{1}{30}\cdot 516234-\frac{1}{30}\cdot 615234-\frac{1}{90}\cdot 615243-\frac{1}{15}\cdot 621345\\
&+\frac{2}{45}\cdot 561423+\frac{2}{45}\cdot 651423-\frac{2}{45}\cdot 562134-\frac{2}{45}\cdot 652134+\frac{1}{15}\cdot 612354-\frac{1}{45}\cdot 623145\\
&+\frac{1}{30}\cdot 623415+\frac{1}{30}\cdot 461235+\frac{1}{30}\cdot 641235+\frac{1}{90}\cdot 641325+\frac{2}{45}\cdot 561243+\frac{2}{45}\cdot 651243\\
&-\frac{2}{45}\cdot 562314-\frac{2}{45}\cdot 652314-\frac{1}{90}\cdot 613542+\frac{2}{45}\cdot 561342+\frac{2}{45}\cdot 561432+\frac{2}{45}\cdot 651342\\
&+\frac{2}{45}\cdot 651432-\frac{1}{45}\cdot 562413-\frac{1}{45}\cdot 652413+\frac{1}{90}\cdot 641253-\frac{1}{90}\cdot 641352+\frac{1}{90}\cdot 624315\\
&+\frac{1}{45}\cdot 643125-\frac{1}{45}\cdot 563214-\frac{1}{45}\cdot 653214
\end{aligned}
$$

$$
\begin{aligned}
[\![x_4\times x_4]\!]=&\frac{2}{45}\cdot 125346+\frac{2}{15}\cdot 125436+\frac{2}{45}\cdot 215346+\frac{2}{15}\cdot 215436-\frac{2}{45}\cdot 351426+\frac{2}{45}\cdot 125364\\
&+\frac{4}{45}\cdot 125463+\frac{2}{45}\cdot 215364+\frac{4}{45}\cdot 215463+\frac{4}{45}\cdot 126435+\frac{4}{45}\cdot 216435-\frac{2}{45}\cdot 361425\\
&+\frac{4}{45}\cdot 142356+\frac{4}{15}\cdot 143256+\frac{4}{45}\cdot 241536+\frac{2}{45}\cdot 413526+\frac{4}{45}\cdot 142365+\frac{4}{15}\cdot 143265\\
&+\frac{4}{45}\cdot 241635+\frac{2}{45}\cdot 413625+\frac{2}{45}\cdot 142536+\frac{4}{45}\cdot 143526-\frac{4}{45}\cdot 145236-\frac{2}{45}\cdot 145326\\
&-\frac{4}{45}\cdot 243516-\frac{2}{45}\cdot 235146-\frac{4}{45}\cdot 235416+\frac{2}{45}\cdot 325146-\frac{8}{45}\cdot 325416-\frac{2}{45}\cdot 415236\\
&-\frac{2}{45}\cdot 415326-\frac{8}{45}\cdot 243561-\frac{4}{45}\cdot 145263-\frac{4}{45}\cdot 145362-\frac{4}{45}\cdot 235461-\frac{16}{45}\cdot 325461
\end{aligned}
$$

$$
\begin{aligned}
&-\tfrac{2}{45}\cdot 415263-\tfrac{2}{45}\cdot 415362+\tfrac{2}{45}\cdot 142635+\tfrac{4}{45}\cdot 143625-\tfrac{4}{45}\cdot 146235-\tfrac{4}{45}\cdot 243615\\
&-\tfrac{8}{45}\cdot 243651-\tfrac{4}{45}\cdot 146253-\tfrac{2}{45}\cdot 146352+\tfrac{4}{45}\cdot 153246-\tfrac{2}{45}\cdot 153426-\tfrac{4}{45}\cdot 513246\\
&-\tfrac{4}{45}\cdot 512436-\tfrac{8}{45}\cdot 521436-\tfrac{4}{45}\cdot 513264+\tfrac{4}{45}\cdot 153264-\tfrac{8}{45}\cdot 613245-\tfrac{4}{45}\cdot 163425\\
&-\tfrac{4}{45}\cdot 612435-\tfrac{16}{45}\cdot 621435-\tfrac{8}{45}\cdot 613254-\tfrac{2}{45}\cdot 163524+\tfrac{2}{45}\cdot 124536+\tfrac{2}{45}\cdot 214536\\
&-\tfrac{2}{45}\cdot 351462+\tfrac{2}{45}\cdot 124635+\tfrac{2}{45}\cdot 214635+\tfrac{2}{45}\cdot 253146+\tfrac{4}{45}\cdot 134256+\tfrac{4}{45}\cdot 315246\\
&+\tfrac{2}{45}\cdot 253164+\tfrac{4}{45}\cdot 134265+\tfrac{4}{45}\cdot 315264-\tfrac{4}{45}\cdot 153462-\tfrac{2}{45}\cdot 153642+\tfrac{2}{45}\cdot 135246\\
&-\tfrac{2}{45}\cdot 154236-\tfrac{2}{45}\cdot 245136-\tfrac{2}{45}\cdot 254136-\tfrac{2}{45}\cdot 412536+\tfrac{2}{45}\cdot 421536+\tfrac{2}{45}\cdot 135264\\
&-\tfrac{4}{45}\cdot 164235-\tfrac{2}{45}\cdot 246135-\tfrac{2}{45}\cdot 264135-\tfrac{2}{45}\cdot 164253+\tfrac{4}{45}\cdot 125634+\tfrac{2}{45}\cdot 125643\\
&+\tfrac{4}{45}\cdot 215634+\tfrac{2}{45}\cdot 215643+\tfrac{2}{45}\cdot 126453+\tfrac{2}{45}\cdot 216453-\tfrac{2}{45}\cdot 361452+\tfrac{2}{15}\cdot 241563\\
&+\tfrac{4}{45}\cdot 413562+\tfrac{2}{15}\cdot 241653+\tfrac{4}{45}\cdot 413652+\tfrac{2}{45}\cdot 245163-\tfrac{2}{45}\cdot 235164+\tfrac{2}{45}\cdot 325164\\
&-\tfrac{2}{15}\cdot 145623-\tfrac{2}{15}\cdot 145632-\tfrac{2}{45}\cdot 245361-\tfrac{2}{45}\cdot 235614-\tfrac{2}{45}\cdot 235641-\tfrac{2}{15}\cdot 325614\\
&-\tfrac{14}{45}\cdot 325641-\tfrac{2}{45}\cdot 415623-\tfrac{2}{45}\cdot 415632+\tfrac{2}{45}\cdot 246153-\tfrac{4}{45}\cdot 146523-\tfrac{4}{45}\cdot 146532\\
&-\tfrac{2}{45}\cdot 246351+\tfrac{2}{45}\cdot 513462-\tfrac{2}{45}\cdot 512463-\tfrac{2}{15}\cdot 521463+\tfrac{2}{45}\cdot 513642-\tfrac{2}{15}\cdot 163452\\
&-\tfrac{2}{45}\cdot 613425-\tfrac{2}{45}\cdot 612453-\tfrac{14}{45}\cdot 621453-\tfrac{4}{45}\cdot 163542-\tfrac{2}{45}\cdot 613524+\tfrac{2}{45}\cdot 126534\\
&+\tfrac{2}{45}\cdot 216534+\tfrac{4}{45}\cdot 263145+\tfrac{2}{15}\cdot 316245+\tfrac{4}{45}\cdot 263154+\tfrac{2}{15}\cdot 316254+\tfrac{2}{45}\cdot 263415\\
&-\tfrac{2}{45}\cdot 236415-\tfrac{2}{15}\cdot 326415-\tfrac{2}{45}\cdot 253461-\tfrac{2}{45}\cdot 236451-\tfrac{14}{45}\cdot 326451+\tfrac{2}{45}\cdot 263514\\
&-\tfrac{2}{45}\cdot 253641+\tfrac{2}{45}\cdot 416235-\tfrac{2}{45}\cdot 412635+\tfrac{2}{45}\cdot 421635+\tfrac{2}{45}\cdot 416253-\tfrac{2}{15}\cdot 156234\\
&-\tfrac{2}{15}\cdot 165234-\tfrac{2}{45}\cdot 614235-\tfrac{2}{45}\cdot 256134-\tfrac{2}{45}\cdot 265134-\tfrac{2}{45}\cdot 512634-\tfrac{2}{15}\cdot 521634\\
&-\tfrac{2}{45}\cdot 612534-\tfrac{14}{45}\cdot 621534-\tfrac{4}{45}\cdot 156243-\tfrac{4}{45}\cdot 165243-\tfrac{2}{45}\cdot 614253+\tfrac{2}{15}\cdot 312456\\
&+\tfrac{2}{15}\cdot 312465+\tfrac{2}{5}\cdot 321456+\tfrac{2}{5}\cdot 321465+\tfrac{2}{15}\cdot 312546+\tfrac{2}{15}\cdot 312564+\tfrac{2}{5}\cdot 321546\\
&+\tfrac{2}{5}\cdot 321564+\tfrac{2}{15}\cdot 312645+\tfrac{2}{5}\cdot 321645+\tfrac{2}{45}\cdot 314256+\tfrac{2}{45}\cdot 314265+\tfrac{4}{45}\cdot 324156\\
&+\tfrac{4}{45}\cdot 324165-\tfrac{4}{15}\cdot 341256-\tfrac{2}{15}\cdot 342156-\tfrac{2}{15}\cdot 314562-\tfrac{2}{15}\cdot 314652-\tfrac{4}{15}\cdot 324561\\
&-\tfrac{4}{15}\cdot 324651-\tfrac{2}{15}\cdot 341526-\tfrac{4}{45}\cdot 342516-\tfrac{2}{15}\cdot 351246-\tfrac{2}{45}\cdot 352146-\tfrac{4}{45}\cdot 361245\\
&-\tfrac{2}{45}\cdot 362145-\tfrac{2}{15}\cdot 315462-\tfrac{2}{15}\cdot 315642-\tfrac{2}{15}\cdot 316452-\tfrac{2}{45}\cdot 352416-\tfrac{2}{45}\cdot 362415\\
&+\tfrac{4}{45}\cdot 421356+\tfrac{4}{45}\cdot 421365-\tfrac{2}{15}\cdot 423156+\tfrac{2}{45}\cdot 526134-\tfrac{4}{15}\cdot 621345-\tfrac{4}{15}\cdot 621354\\
&-\tfrac{4}{45}\cdot 523146-\tfrac{2}{45}\cdot 524136+\tfrac{2}{45}\cdot 425136+\tfrac{2}{45}\cdot 426135-\tfrac{2}{45}\cdot 314526-\tfrac{2}{45}\cdot 315426
\end{aligned}
$$

$$- \frac{4}{45} \cdot 324516 - \frac{2}{45} \cdot 314625 - \frac{2}{45} \cdot 316425 - \frac{4}{45} \cdot 324615 - \frac{4}{45} \cdot 521346 - \frac{4}{45} \cdot 521364$$
$$+ \frac{2}{15} \cdot 231456 + \frac{2}{15} \cdot 231465 + \frac{2}{15} \cdot 231546 + \frac{2}{15} \cdot 231564 + \frac{2}{15} \cdot 231645 - \frac{4}{45} \cdot 423516$$
$$+ \frac{2}{45} \cdot 425613 - \frac{2}{45} \cdot 425316 + \frac{2}{45} \cdot 241356 + \frac{2}{45} \cdot 241365 - \frac{2}{15} \cdot 431256 - \frac{4}{45} \cdot 341562$$
$$- \frac{2}{45} \cdot 431526 - \frac{2}{45} \cdot 431562 - \frac{2}{15} \cdot 261345 - \frac{2}{15} \cdot 261354 - \frac{4}{45} \cdot 531246 - \frac{2}{15} \cdot 261435$$
$$- \frac{2}{15} \cdot 261453 - \frac{2}{45} \cdot 531426 - \frac{2}{45} \cdot 531462 - \frac{2}{15} \cdot 261534 + \frac{2}{45} \cdot 425163 - \frac{2}{45} \cdot 251346$$
$$- \frac{2}{45} \cdot 251436 - \frac{2}{45} \cdot 251364 - \frac{2}{45} \cdot 251463 + \frac{2}{15} \cdot 312654 + \frac{2}{5} \cdot 321654 + \frac{2}{45} \cdot 426153$$
$$- \frac{4}{15} \cdot 341265 - \frac{2}{15} \cdot 342165 - \frac{2}{15} \cdot 351264 - \frac{2}{45} \cdot 352164 - \frac{2}{15} \cdot 341625 - \frac{4}{45} \cdot 342615$$
$$- \frac{4}{45} \cdot 351624 - \frac{2}{45} \cdot 352614 + \frac{4}{45} \cdot 326145 + \frac{4}{45} \cdot 326154 - \frac{4}{45} \cdot 361254 - \frac{2}{45} \cdot 362154$$
$$- \frac{2}{15} \cdot 316542 - \frac{4}{15} \cdot 326541 - \frac{4}{45} \cdot 361524 - \frac{2}{45} \cdot 362514 - \frac{2}{15} \cdot 423165 - \frac{4}{45} \cdot 521643$$
$$+ \frac{2}{45} \cdot 526143 - \frac{4}{15} \cdot 621543 - \frac{2}{45} \cdot 315624 - \frac{2}{45} \cdot 316524 - \frac{4}{45} \cdot 326514 + \frac{4}{45} \cdot 421563$$
$$+ \frac{4}{45} \cdot 421653 - \frac{4}{45} \cdot 523164 - \frac{2}{45} \cdot 524163 + \frac{2}{15} \cdot 231654 - \frac{4}{45} \cdot 423615 + \frac{2}{45} \cdot 426513$$
$$- \frac{2}{45} \cdot 426315 - \frac{2}{15} \cdot 431265 - \frac{2}{45} \cdot 251634 - \frac{2}{45} \cdot 251643 - \frac{4}{45} \cdot 341652 - \frac{2}{45} \cdot 431625$$
$$- \frac{2}{45} \cdot 431652 - \frac{2}{15} \cdot 261543 - \frac{4}{45} \cdot 531264 - \frac{2}{45} \cdot 531624 - \frac{4}{45} \cdot 351642 - \frac{2}{45} \cdot 531642$$
$$- \frac{2}{45} \cdot 342561 - \frac{2}{45} \cdot 342651 - \frac{2}{45} \cdot 346125 - \frac{2}{45} \cdot 346215 - \frac{2}{45} \cdot 352461 - \frac{2}{45} \cdot 352641$$
$$- \frac{2}{45} \cdot 354126 - \frac{2}{45} \cdot 354216 - \frac{2}{45} \cdot 364125 - \frac{2}{45} \cdot 364215 + \frac{2}{45} \cdot 523614 + \frac{2}{45} \cdot 526314$$
$$- \frac{2}{45} \cdot 623145 - \frac{2}{45} \cdot 623154 - \frac{2}{45} \cdot 524316 - \frac{2}{45} \cdot 624135 - \frac{2}{45} \cdot 624153 + \frac{2}{15} \cdot 345162$$
$$+ \frac{2}{15} \cdot 345261 + \frac{2}{45} \cdot 354162 + \frac{2}{45} \cdot 354261 + \frac{4}{45} \cdot 346152 + \frac{4}{45} \cdot 346251 + \frac{2}{45} \cdot 364152$$
$$+ \frac{2}{45} \cdot 364251 + \frac{2}{15} \cdot 623415 + \frac{2}{45} \cdot 624315 + \frac{4}{45} \cdot 623514 + \frac{2}{45} \cdot 625314 + \frac{2}{45} \cdot 435126$$
$$+ \frac{2}{45} \cdot 435216 + \frac{2}{45} \cdot 435162 + \frac{2}{45} \cdot 435261 + \frac{2}{45} \cdot 532416 + \frac{2}{45} \cdot 632415 + \frac{4}{15} \cdot 345612$$
$$+ \frac{4}{15} \cdot 345621 + \frac{2}{9} \cdot 346512 + \frac{2}{9} \cdot 346521 - \frac{2}{45} \cdot 356124 - \frac{2}{45} \cdot 356214 + \frac{2}{15} \cdot 354612$$
$$+ \frac{2}{15} \cdot 354621 + \frac{2}{15} \cdot 356412 + \frac{2}{15} \cdot 356421 + \frac{2}{15} \cdot 364512 + \frac{2}{15} \cdot 364521 - \frac{2}{45} \cdot 423561$$
$$- \frac{2}{45} \cdot 423651 - \frac{2}{45} \cdot 425361 - \frac{2}{45} \cdot 426351 + \frac{4}{15} \cdot 623451 + \frac{2}{9} \cdot 623541 + \frac{2}{45} \cdot 524613$$
$$+ \frac{2}{15} \cdot 624351 + \frac{2}{15} \cdot 624531 + \frac{2}{15} \cdot 625341 + \frac{2}{15} \cdot 523461 + \frac{2}{45} \cdot 524361 + \frac{4}{45} \cdot 523641$$
$$+ \frac{2}{45} \cdot 524631 + \frac{2}{45} \cdot 435612 + \frac{2}{45} \cdot 435621 + \frac{2}{45} \cdot 532461 + \frac{2}{45} \cdot 632451 - \frac{4}{45} \cdot 361542$$
$$- \frac{2}{45} \cdot 362451 - \frac{2}{45} \cdot 362541 - \frac{2}{45} \cdot 365124 - \frac{2}{45} \cdot 365214 + \frac{2}{45} \cdot 526413 - \frac{2}{45} \cdot 625134$$
$$- \frac{2}{45} \cdot 625143 + \frac{2}{45} \cdot 356142 + \frac{2}{45} \cdot 356241 + \frac{2}{45} \cdot 365142 + \frac{2}{45} \cdot 365241 + \frac{2}{45} \cdot 624513$$

$$
\begin{aligned}
&+\frac{2}{45}\cdot\mathsf{625413}+\frac{2}{15}\cdot\mathsf{365412}+\frac{2}{15}\cdot\mathsf{365421}+\frac{2}{45}\cdot\mathsf{526341}+\frac{2}{45}\cdot\mathsf{526431}+\frac{2}{15}\cdot\mathsf{625431}\\
&-\frac{2}{45}\cdot\mathsf{425631}-\frac{2}{45}\cdot\mathsf{426531}-\frac{2}{45}\cdot\mathsf{451263}-\frac{2}{45}\cdot\mathsf{541263}-\frac{2}{45}\cdot\mathsf{631245}-\frac{2}{45}\cdot\mathsf{631254}\\
&-\frac{2}{45}\cdot\mathsf{451326}-\frac{2}{45}\cdot\mathsf{451362}-\frac{2}{45}\cdot\mathsf{541326}-\frac{2}{45}\cdot\mathsf{541362}-\frac{2}{45}\cdot\mathsf{631425}-\frac{2}{45}\cdot\mathsf{631524}\\
&+\frac{2}{15}\cdot\mathsf{461235}+\frac{2}{45}\cdot\mathsf{461325}+\frac{2}{15}\cdot\mathsf{641235}+\frac{2}{45}\cdot\mathsf{641325}+\frac{4}{45}\cdot\mathsf{461253}+\frac{2}{45}\cdot\mathsf{461352}\\
&+\frac{4}{45}\cdot\mathsf{641253}+\frac{2}{45}\cdot\mathsf{641352}+\frac{2}{45}\cdot\mathsf{452136}+\frac{2}{45}\cdot\mathsf{542136}+\frac{2}{45}\cdot\mathsf{462135}+\frac{2}{45}\cdot\mathsf{642135}\\
&-\frac{2}{45}\cdot\mathsf{451623}-\frac{2}{45}\cdot\mathsf{451632}-\frac{2}{45}\cdot\mathsf{541623}-\frac{2}{45}\cdot\mathsf{541632}+\frac{2}{45}\cdot\mathsf{461523}+\frac{2}{45}\cdot\mathsf{461532}\\
&+\frac{2}{45}\cdot\mathsf{641523}+\frac{2}{45}\cdot\mathsf{641532}-\frac{2}{45}\cdot\mathsf{631452}-\frac{2}{45}\cdot\mathsf{631542}+\frac{4}{15}\cdot\mathsf{561234}+\frac{2}{9}\cdot\mathsf{561243}\\
&+\frac{4}{15}\cdot\mathsf{651234}+\frac{2}{9}\cdot\mathsf{651243}+\frac{2}{15}\cdot\mathsf{561324}+\frac{2}{15}\cdot\mathsf{561342}+\frac{2}{15}\cdot\mathsf{651324}+\frac{2}{15}\cdot\mathsf{651342}\\
&+\frac{2}{15}\cdot\mathsf{561423}+\frac{2}{15}\cdot\mathsf{651423}+\frac{2}{45}\cdot\mathsf{562134}+\frac{2}{45}\cdot\mathsf{652134}+\frac{2}{15}\cdot\mathsf{561432}+\frac{2}{15}\cdot\mathsf{651432}
\end{aligned}
$$

$$
\begin{aligned}
[\![x_4\times x_5]\!]=&-\frac{2}{45}\cdot\mathsf{132465}-\frac{2}{45}\cdot\mathsf{124365}-\frac{1}{45}\cdot\mathsf{124635}-\frac{2}{15}\cdot\mathsf{214365}-\frac{1}{45}\cdot\mathsf{214635}-\frac{2}{45}\cdot\mathsf{132546}\\
&-\frac{1}{45}\cdot\mathsf{135246}+\frac{2}{45}\cdot\mathsf{125346}+\frac{1}{15}\cdot\mathsf{125436}+\frac{1}{45}\cdot\mathsf{215346}-\frac{1}{45}\cdot\mathsf{132564}+\frac{1}{45}\cdot\mathsf{135264}\\
&+\frac{1}{15}\cdot\mathsf{142356}+\frac{2}{15}\cdot\mathsf{143256}+\frac{2}{45}\cdot\mathsf{143526}+\frac{1}{30}\cdot\mathsf{413526}-\frac{4}{45}\cdot\mathsf{145236}-\frac{1}{15}\cdot\mathsf{145326}\\
&-\frac{2}{45}\cdot\mathsf{235146}-\frac{1}{15}\cdot\mathsf{235416}-\frac{1}{45}\cdot\mathsf{325146}-\frac{2}{15}\cdot\mathsf{325416}-\frac{1}{30}\cdot\mathsf{415236}-\frac{1}{18}\cdot\mathsf{415326}\\
&-\frac{2}{45}\cdot\mathsf{142653}-\frac{2}{45}\cdot\mathsf{143652}-\frac{1}{45}\cdot\mathsf{146253}-\frac{1}{45}\cdot\mathsf{146352}-\frac{1}{45}\cdot\mathsf{246351}-\frac{2}{45}\cdot\mathsf{153426}\\
&-\frac{2}{45}\cdot\mathsf{513246}+\frac{1}{90}\cdot\mathsf{513426}-\frac{1}{45}\cdot\mathsf{152364}-\frac{1}{18}\cdot\mathsf{251463}-\frac{1}{15}\cdot\mathsf{254163}-\frac{2}{45}\cdot\mathsf{351462}\\
&-\frac{1}{30}\cdot\mathsf{354162}+\frac{1}{45}\cdot\mathsf{153624}+\frac{2}{45}\cdot\mathsf{513264}+\frac{1}{90}\cdot\mathsf{153462}+\frac{1}{30}\cdot\mathsf{154362}+\frac{2}{45}\cdot\mathsf{253461}\\
&+\frac{1}{15}\cdot\mathsf{254361}-\frac{2}{45}\cdot\mathsf{163254}-\frac{1}{45}\cdot\mathsf{163524}-\frac{1}{45}\cdot\mathsf{613524}+\frac{1}{90}\cdot\mathsf{164235}+\frac{1}{30}\cdot\mathsf{164325}\\
&+\frac{2}{45}\cdot\mathsf{614235}+\frac{1}{15}\cdot\mathsf{614325}+\frac{2}{45}\cdot\mathsf{142365}-\frac{1}{45}\cdot\mathsf{142563}+\frac{1}{90}\cdot\mathsf{152463}+\frac{1}{45}\cdot\mathsf{134256}\\
&+\frac{2}{45}\cdot\mathsf{315246}-\frac{1}{45}\cdot\mathsf{154236}+\frac{1}{90}\cdot\mathsf{154263}+\frac{1}{90}\cdot\mathsf{354261}-\frac{1}{45}\cdot\mathsf{136254}-\frac{1}{90}\cdot\mathsf{146325}\\
&+\frac{1}{30}\cdot\mathsf{246315}+\frac{1}{90}\cdot\mathsf{624315}-\frac{1}{45}\cdot\mathsf{124653}-\frac{1}{45}\cdot\mathsf{135426}+\frac{1}{45}\cdot\mathsf{125463}+\frac{2}{45}\cdot\mathsf{215463}\\
&+\frac{1}{30}\cdot\mathsf{135624}+\frac{1}{30}\cdot\mathsf{135642}+\frac{1}{30}\cdot\mathsf{136452}+\frac{1}{15}\cdot\mathsf{241563}+\frac{1}{45}\cdot\mathsf{413562}-\frac{1}{90}\cdot\mathsf{145263}\\
&-\frac{1}{30}\cdot\mathsf{145362}-\frac{2}{45}\cdot\mathsf{235164}-\frac{1}{45}\cdot\mathsf{415263}+\frac{1}{90}\cdot\mathsf{415362}-\frac{1}{45}\cdot\mathsf{146523}-\frac{1}{45}\cdot\mathsf{146532}\\
&-\frac{1}{45}\cdot\mathsf{513462}+\frac{1}{90}\cdot\mathsf{152634}-\frac{1}{90}\cdot\mathsf{152643}+\frac{1}{30}\cdot\mathsf{251634}+\frac{1}{90}\cdot\mathsf{251643}+\frac{1}{30}\cdot\mathsf{513642}\\
&+\frac{1}{45}\cdot\mathsf{154623}+\frac{1}{45}\cdot\mathsf{154632}-\frac{1}{45}\cdot\mathsf{253614}+\frac{1}{30}\cdot\mathsf{352614}+\frac{1}{45}\cdot\mathsf{352641}-\frac{1}{45}\cdot\mathsf{163542}\\
&+\frac{1}{45}\cdot\mathsf{164352}+\frac{1}{45}\cdot\mathsf{624153}-\frac{1}{45}\cdot\mathsf{126354}-\frac{1}{45}\cdot\mathsf{152436}+\frac{1}{45}\cdot\mathsf{126435}+\frac{2}{45}\cdot\mathsf{216435}
\end{aligned}
$$

$$- \frac{1}{45} \cdot 361425 + \frac{1}{30} \cdot 162453 + \frac{1}{30} \cdot 162534 + \frac{2}{45} \cdot 263145 + \frac{1}{45} \cdot 316245 - \frac{1}{30} \cdot 163425$$
$$- \frac{2}{45} \cdot 236415 - \frac{1}{15} \cdot 326415 - \frac{1}{30} \cdot 146235 - \frac{2}{45} \cdot 416235 - \frac{1}{90} \cdot 364152 + \frac{1}{90} \cdot 416253$$
$$- \frac{1}{45} \cdot 156243 - \frac{1}{45} \cdot 165243 + \frac{1}{45} \cdot 156324 + \frac{1}{45} \cdot 165324 - \frac{2}{45} \cdot 213546 - \frac{1}{45} \cdot 213564$$
$$+ \frac{2}{45} \cdot 231546 - \frac{2}{45} \cdot 231564 - \frac{2}{45} \cdot 231645 - \frac{1}{15} \cdot 236145 - \frac{2}{45} \cdot 214356 - \frac{1}{45} \cdot 241356$$
$$- \frac{1}{45} \cdot 241365 - \frac{1}{45} \cdot 214536 + \frac{1}{15} \cdot 214563 + \frac{2}{45} \cdot 241536 + \frac{1}{15} \cdot 216345 + \frac{1}{15} \cdot 312456$$
$$+ \frac{2}{45} \cdot 312465 + \frac{1}{5} \cdot 321456 + \frac{2}{15} \cdot 321465 + \frac{2}{45} \cdot 324156 - \frac{8}{45} \cdot 341256 - \frac{4}{45} \cdot 342156$$
$$- \frac{2}{45} \cdot 315426 - \frac{1}{30} \cdot 316425 - \frac{1}{30} \cdot 316452 - \frac{4}{45} \cdot 325461 - \frac{1}{15} \cdot 326451 - \frac{1}{45} \cdot 352416$$
$$- \frac{1}{45} \cdot 352461 - \frac{4}{45} \cdot 361452 - \frac{1}{90} \cdot 362415 - \frac{1}{30} \cdot 362451 - \frac{4}{45} \cdot 423156 - \frac{1}{45} \cdot 412536$$
$$- \frac{1}{9} \cdot 412563 + \frac{2}{45} \cdot 425136 + \frac{1}{30} \cdot 426135 + \frac{1}{15} \cdot 521634 + \frac{1}{30} \cdot 526134 - \frac{1}{90} \cdot 423516$$
$$+ \frac{2}{45} \cdot 423561 + \frac{1}{30} \cdot 432516 + \frac{1}{15} \cdot 432561 - \frac{2}{15} \cdot 521436 - \frac{1}{45} \cdot 524136 - \frac{4}{45} \cdot 621435$$
$$- \frac{1}{15} \cdot 621534 - \frac{1}{45} \cdot 624135 - \frac{1}{30} \cdot 625134 + \frac{1}{90} \cdot 531246 + \frac{1}{30} \cdot 532146 + \frac{2}{45} \cdot 631245$$
$$+ \frac{1}{15} \cdot 632145 - \frac{2}{45} \cdot 213465 - \frac{1}{45} \cdot 132645 + \frac{2}{45} \cdot 231465 - \frac{2}{45} \cdot 251346 + \frac{1}{45} \cdot 251364$$
$$- \frac{1}{45} \cdot 213645 + \frac{2}{15} \cdot 321546 - \frac{2}{45} \cdot 243516 - \frac{2}{45} \cdot 324651 - \frac{1}{15} \cdot 521346 - \frac{1}{90} \cdot 435162$$
$$+ \frac{1}{45} \cdot 521364 - \frac{2}{45} \cdot 621354 + \frac{2}{45} \cdot 312546 - \frac{2}{45} \cdot 312564 - \frac{2}{45} \cdot 312645 - \frac{1}{45} \cdot 314526$$
$$+ \frac{1}{15} \cdot 231456 - \frac{4}{45} \cdot 431256 - \frac{1}{30} \cdot 431526 - \frac{1}{15} \cdot 251436 - \frac{1}{30} \cdot 261534 - \frac{1}{90} \cdot 352146$$
$$- \frac{1}{45} \cdot 315264 - \frac{2}{45} \cdot 243156 - \frac{1}{18} \cdot 341526 + \frac{1}{30} \cdot 435261 + \frac{1}{30} \cdot 632415 - \frac{1}{15} \cdot 213654$$
$$- \frac{1}{15} \cdot 231654 - \frac{1}{15} \cdot 132654 - \frac{1}{45} \cdot 236154 + \frac{1}{15} \cdot 143265 + \frac{4}{45} \cdot 215634 + \frac{2}{45} \cdot 215643$$
$$+ \frac{2}{45} \cdot 216453 - \frac{1}{30} \cdot 261453 + \frac{1}{15} \cdot 321564 + \frac{1}{15} \cdot 324165 - \frac{1}{90} \cdot 425163 - \frac{4}{45} \cdot 341265$$
$$- \frac{2}{45} \cdot 342165 + \frac{1}{90} \cdot 316524 - \frac{1}{30} \cdot 316542 - \frac{1}{45} \cdot 326514 - \frac{1}{15} \cdot 326541 - \frac{1}{90} \cdot 361524$$
$$- \frac{2}{45} \cdot 361542 - \frac{1}{90} \cdot 362541 + \frac{1}{45} \cdot 421365 - \frac{2}{45} \cdot 423165 - \frac{2}{45} \cdot 521463 - \frac{1}{30} \cdot 523164$$
$$- \frac{1}{45} \cdot 524163 - \frac{2}{45} \cdot 412635 - \frac{1}{15} \cdot 412653 + \frac{1}{45} \cdot 521643 + \frac{1}{30} \cdot 526143 + \frac{1}{90} \cdot 423615$$
$$+ \frac{4}{45} \cdot 423651 + \frac{1}{30} \cdot 432615 + \frac{1}{15} \cdot 432651 - \frac{1}{15} \cdot 621543 - \frac{1}{90} \cdot 625143 + \frac{4}{45} \cdot 631254$$
$$+ \frac{1}{15} \cdot 632154 + \frac{1}{15} \cdot 241653 + \frac{2}{45} \cdot 216534 + \frac{1}{15} \cdot 321645 - \frac{1}{30} \cdot 315642 - \frac{1}{15} \cdot 325641$$
$$- \frac{1}{30} \cdot 436152 + \frac{1}{45} \cdot 416352 - \frac{1}{15} \cdot 621453 - \frac{1}{90} \cdot 531264 + \frac{1}{30} \cdot 532164 - \frac{1}{15} \cdot 312654$$
$$+ \frac{1}{45} \cdot 413265 + \frac{1}{45} \cdot 314625 + \frac{1}{90} \cdot 413625 + \frac{2}{45} \cdot 413652 - \frac{1}{45} \cdot 243165 - \frac{2}{45} \cdot 431265$$
$$- \frac{1}{90} \cdot 431625 + \frac{1}{45} \cdot 431652 - \frac{1}{30} \cdot 261543 + \frac{1}{45} \cdot 362154 + \frac{1}{45} \cdot 316254 + \frac{1}{45} \cdot 143625$$

$$-\frac{1}{90}\cdot 341625+\frac{1}{90}\cdot 436251+\frac{1}{30}\cdot 352164+\frac{1}{90}\cdot 632514+\frac{1}{30}\cdot 245136+\frac{1}{30}\cdot 245316$$
$$+\frac{1}{18}\cdot 253416+\frac{1}{15}\cdot 263154-\frac{1}{45}\cdot 324516-\frac{1}{30}\cdot 342516-\frac{1}{45}\cdot 354126-\frac{1}{45}\cdot 354216$$
$$-\frac{2}{45}\cdot 364125-\frac{2}{45}\cdot 364215+\frac{1}{90}\cdot 526314+\frac{1}{15}\cdot 435126+\frac{1}{15}\cdot 435216+\frac{2}{45}\cdot 532416$$
$$+\frac{1}{15}\cdot 234165+\frac{1}{90}\cdot 136425+\frac{1}{15}\cdot 234615+\frac{1}{30}\cdot 253146+\frac{1}{15}\cdot 345126+\frac{1}{15}\cdot 345216$$
$$+\frac{4}{45}\cdot 341652+\frac{2}{45}\cdot 342651+\frac{1}{30}\cdot 346152+\frac{1}{30}\cdot 346251+\frac{1}{90}\cdot 364251+\frac{1}{15}\cdot 523416$$
$$+\frac{1}{45}\cdot 451263+\frac{1}{15}\cdot 452163-\frac{2}{45}\cdot 523614-\frac{2}{45}\cdot 452361-\frac{2}{45}\cdot 453261+\frac{2}{45}\cdot 623154$$
$$+\frac{1}{30}\cdot 623514+\frac{1}{90}\cdot 625314-\frac{2}{45}\cdot 634125-\frac{2}{45}\cdot 634215+\frac{1}{45}\cdot 324615+\frac{1}{90}\cdot 246153$$
$$-\frac{1}{90}\cdot 523146-\frac{1}{90}\cdot 351264-\frac{1}{90}\cdot 253164+\frac{1}{30}\cdot 263514+\frac{1}{45}\cdot 235461+\frac{1}{45}\cdot 235614$$
$$+\frac{1}{45}\cdot 235641-\frac{1}{45}\cdot 243561-\frac{1}{30}\cdot 245613-\frac{1}{30}\cdot 245631-\frac{1}{30}\cdot 263451-\frac{1}{90}\cdot 263541$$
$$-\frac{1}{15}\cdot 324561+\frac{2}{45}\cdot 364512+\frac{2}{45}\cdot 364521+\frac{2}{45}\cdot 415623+\frac{1}{45}\cdot 415632+\frac{1}{45}\cdot 426351$$
$$-\frac{2}{45}\cdot 435612-\frac{2}{45}\cdot 435621+\frac{2}{45}\cdot 625341-\frac{1}{90}\cdot 531462-\frac{2}{45}\cdot 632451+\frac{1}{15}\cdot 234651$$
$$+\frac{1}{45}\cdot 236451-\frac{1}{30}\cdot 254613-\frac{1}{90}\cdot 254631+\frac{1}{45}\cdot 341562+\frac{1}{30}\cdot 345162+\frac{1}{30}\cdot 345261$$
$$+\frac{2}{45}\cdot 346512+\frac{2}{45}\cdot 346521+\frac{1}{30}\cdot 523461+\frac{1}{90}\cdot 524361-\frac{1}{45}\cdot 451632-\frac{2}{45}\cdot 453612$$
$$-\frac{2}{45}\cdot 453621+\frac{2}{45}\cdot 623541-\frac{2}{45}\cdot 634251-\frac{1}{30}\cdot 246513+\frac{1}{90}\cdot 136524+\frac{1}{45}\cdot 236514$$
$$+\frac{1}{90}\cdot 254136+\frac{1}{45}\cdot 142635+\frac{1}{45}\cdot 256143+\frac{1}{90}\cdot 264135+\frac{1}{30}\cdot 315624+\frac{1}{45}\cdot 325614$$
$$-\frac{1}{90}\cdot 425613-\frac{1}{90}\cdot 342615-\frac{1}{45}\cdot 365124-\frac{1}{45}\cdot 365214-\frac{1}{90}\cdot 524613-\frac{1}{15}\cdot 416325$$
$$-\frac{1}{45}\cdot 426153+\frac{1}{45}\cdot 526413+\frac{1}{45}\cdot 436125+\frac{1}{45}\cdot 436215+\frac{1}{45}\cdot 631524-\frac{1}{45}\cdot 265134$$
$$-\frac{1}{30}\cdot 351246-\frac{1}{45}\cdot 361245+\frac{1}{45}\cdot 346125+\frac{1}{45}\cdot 346215+\frac{1}{45}\cdot 356142+\frac{1}{45}\cdot 356241$$
$$+\frac{1}{45}\cdot 365142+\frac{1}{45}\cdot 365241+\frac{1}{30}\cdot 461253+\frac{1}{90}\cdot 462153-\frac{1}{90}\cdot 426513-\frac{1}{45}\cdot 462351$$
$$-\frac{1}{45}\cdot 463251+\frac{1}{45}\cdot 624513+\frac{1}{45}\cdot 625413-\frac{1}{45}\cdot 536124-\frac{1}{45}\cdot 536214-\frac{1}{45}\cdot 635124$$
$$-\frac{1}{45}\cdot 635214+\frac{1}{15}\cdot 236541+\frac{1}{30}\cdot 136542+\frac{1}{30}\cdot 254316-\frac{2}{45}\cdot 256341-\frac{1}{45}\cdot 256431$$
$$-\frac{1}{90}\cdot 264351-\frac{1}{45}\cdot 264531-\frac{1}{18}\cdot 425631+\frac{1}{15}\cdot 365412+\frac{1}{15}\cdot 365421+\frac{1}{90}\cdot 523641$$
$$+\frac{1}{90}\cdot 524631+\frac{1}{15}\cdot 416523+\frac{2}{45}\cdot 416532-\frac{2}{45}\cdot 436512-\frac{2}{45}\cdot 436521+\frac{1}{15}\cdot 625431$$
$$-\frac{2}{45}\cdot 632541-\frac{1}{90}\cdot 246531-\frac{1}{45}\cdot 265341+\frac{2}{45}\cdot 356412+\frac{2}{45}\cdot 356421+\frac{1}{45}\cdot 461523$$
$$+\frac{1}{45}\cdot 461532-\frac{1}{30}\cdot 426531-\frac{1}{45}\cdot 463512-\frac{1}{45}\cdot 463521+\frac{2}{45}\cdot 624531-\frac{1}{45}\cdot 531642$$
$$-\frac{1}{45}\cdot 536142-\frac{1}{45}\cdot 635241-\frac{1}{45}\cdot 512436-\frac{1}{45}\cdot 512463+\frac{1}{30}\cdot 514236+\frac{1}{30}\cdot 514263$$

$$
\begin{aligned}
&+ \frac{1}{45}\cdot 451326 + \frac{1}{45}\cdot 541326 + \frac{1}{45}\cdot 452136 + \frac{1}{45}\cdot 542136 + \frac{1}{15}\cdot 412365 + \frac{1}{15}\cdot 512364\\
&- \frac{1}{45}\cdot 514362 + \frac{1}{15}\cdot 451236 + \frac{1}{15}\cdot 541236 + \frac{1}{45}\cdot 534162 - \frac{1}{45}\cdot 351624 - \frac{1}{90}\cdot 531624\\
&- \frac{1}{90}\cdot 532461 - \frac{1}{45}\cdot 534261 + \frac{2}{45}\cdot 361254 - \frac{1}{90}\cdot 462135 - \frac{1}{45}\cdot 462315 - \frac{1}{90}\cdot 642135\\
&- \frac{1}{45}\cdot 642315 + \frac{1}{90}\cdot 461325 + \frac{1}{90}\cdot 641325 + \frac{1}{45}\cdot 512634 + \frac{1}{45}\cdot 512643 - \frac{1}{45}\cdot 514623\\
&- \frac{1}{45}\cdot 514632 - \frac{1}{45}\cdot 451362 - \frac{1}{45}\cdot 541263 - \frac{1}{45}\cdot 541362 - \frac{1}{90}\cdot 351642 - \frac{1}{90}\cdot 532641\\
&- \frac{1}{30}\cdot 631542 - \frac{1}{90}\cdot 642153 - \frac{1}{30}\cdot 516243 - \frac{1}{30}\cdot 516324 - \frac{1}{15}\cdot 541632 - \frac{1}{18}\cdot 631452\\
&+ \frac{1}{45}\cdot 452613 + \frac{1}{45}\cdot 542163 + \frac{1}{45}\cdot 542613 + \frac{1}{45}\cdot 612435 + \frac{1}{45}\cdot 612453 - \frac{1}{45}\cdot 613245\\
&- \frac{1}{30}\cdot 613452 - \frac{1}{30}\cdot 516234 - \frac{1}{30}\cdot 615234 - \frac{1}{90}\cdot 615243 - \frac{1}{15}\cdot 621345 - \frac{2}{45}\cdot 541623\\
&+ \frac{2}{45}\cdot 561423 + \frac{2}{45}\cdot 651423 - \frac{2}{45}\cdot 562134 - \frac{2}{45}\cdot 652134 + \frac{1}{15}\cdot 612354 + \frac{1}{45}\cdot 612534\\
&- \frac{1}{90}\cdot 614352 + \frac{1}{30}\cdot 623415 + \frac{1}{30}\cdot 461235 + \frac{1}{30}\cdot 641235 + \frac{2}{45}\cdot 561243 + \frac{2}{45}\cdot 651243\\
&- \frac{2}{45}\cdot 562314 - \frac{2}{45}\cdot 652314 + \frac{1}{15}\cdot 612543 + \frac{1}{30}\cdot 162543 + \frac{1}{30}\cdot 514326 - \frac{2}{45}\cdot 614523\\
&- \frac{1}{45}\cdot 614532 - \frac{1}{90}\cdot 615324 - \frac{1}{45}\cdot 615342 + \frac{1}{90}\cdot 461352 + \frac{1}{90}\cdot 641253 + \frac{1}{90}\cdot 641352\\
&+ \frac{1}{15}\cdot 561432 + \frac{1}{15}\cdot 651432 - \frac{2}{45}\cdot 562143 - \frac{2}{45}\cdot 652143 - \frac{1}{90}\cdot 613542 - \frac{1}{45}\cdot 615423\\
&+ \frac{2}{45}\cdot 561342 + \frac{2}{45}\cdot 651342 - \frac{1}{45}\cdot 562413 - \frac{1}{45}\cdot 652413
\end{aligned}
$$

$$
\begin{aligned}
[\![x_5 \times x_5]\!] = {} & \frac{2}{45}\cdot 123645 + \frac{1}{9}\cdot 123654 + \frac{1}{45}\cdot 132645 + \frac{2}{45}\cdot 132654 + \frac{1}{45}\cdot 126354 + \frac{1}{9}\cdot 125436\\
&+ \frac{1}{45}\cdot 125463 + \frac{1}{45}\cdot 152436 + \frac{1}{45}\cdot 152463 - \frac{2}{45}\cdot 132465 + \frac{1}{45}\cdot 134265 - \frac{4}{45}\cdot 125634\\
&- \frac{2}{45}\cdot 125643 - \frac{2}{45}\cdot 134625 - \frac{2}{45}\cdot 134652 - \frac{2}{45}\cdot 143625 - \frac{4}{45}\cdot 143652 - \frac{2}{45}\cdot 152634\\
&- \frac{2}{45}\cdot 152643 - \frac{1}{45}\cdot 126435 - \frac{2}{45}\cdot 126453 - \frac{1}{45}\cdot 162435 + \frac{1}{45}\cdot 162453 - \frac{2}{45}\cdot 213546\\
&+ \frac{1}{45}\cdot 213564 + \frac{1}{45}\cdot 231546 - \frac{2}{45}\cdot 231564 - \frac{2}{45}\cdot 213465 - \frac{2}{15}\cdot 214365 - \frac{2}{45}\cdot 312564\\
&- \frac{2}{45}\cdot 315264 - \frac{2}{15}\cdot 412563 - \frac{2}{45}\cdot 415263 + \frac{1}{45}\cdot 231465 + \frac{1}{15}\cdot 234165 + \frac{1}{45}\cdot 236514\\
&+ \frac{1}{15}\cdot 236541 + \frac{1}{45}\cdot 263514 + \frac{1}{45}\cdot 263541 + \frac{1}{15}\cdot 412365 + \frac{2}{45}\cdot 413265 + \frac{2}{45}\cdot 512364\\
&+ \frac{2}{45}\cdot 513264 + \frac{1}{45}\cdot 314625 + \frac{1}{45}\cdot 314652 + \frac{1}{45}\cdot 341625 + \frac{1}{9}\cdot 341652 + \frac{1}{45}\cdot 512643\\
&- \frac{1}{45}\cdot 516243 + \frac{1}{45}\cdot 324615 - \frac{2}{45}\cdot 324651 - \frac{1}{45}\cdot 342615 - \frac{1}{45}\cdot 342651 + \frac{1}{15}\cdot 612543\\
&+ \frac{1}{45}\cdot 615243 - \frac{2}{45}\cdot 621354 - \frac{1}{45}\cdot 623154 + \frac{2}{45}\cdot 123564 + \frac{2}{45}\cdot 213654 + \frac{2}{45}\cdot 124536\\
&- \frac{2}{45}\cdot 124365 - \frac{2}{45}\cdot 124635 - \frac{2}{45}\cdot 214635 - \frac{1}{45}\cdot 124653 - \frac{2}{45}\cdot 126534 - \frac{2}{45}\cdot 132546
\end{aligned}
$$

$$
\begin{aligned}
&-\frac{2}{45}\cdot 135246-\frac{2}{45}\cdot 231645-\frac{2}{45}\cdot 236145+\frac{1}{45}\cdot 312465-\frac{2}{45}\cdot 312645+\frac{2}{45}\cdot 234615\\
&+\frac{2}{45}\cdot 324165+\frac{2}{45}\cdot 135642+\frac{2}{45}\cdot 136542+\frac{2}{45}\cdot 235641+\frac{1}{45}\cdot 142365+\frac{1}{45}\cdot 142635\\
&+\frac{1}{45}\cdot 412635+\frac{2}{45}\cdot 241653+\frac{2}{45}\cdot 246153+\frac{2}{45}\cdot 346152-\frac{2}{45}\cdot 142563-\frac{2}{45}\cdot 142653\\
&-\frac{2}{45}\cdot 412653-\frac{2}{45}\cdot 146352-\frac{2}{45}\cdot 243651-\frac{2}{45}\cdot 246351+\frac{2}{45}\cdot 162543+\frac{2}{45}\cdot 612453\\
&-\frac{4}{45}\cdot 163254-\frac{2}{45}\cdot 163524-\frac{2}{45}\cdot 253164-\frac{2}{45}\cdot 253614-\frac{2}{45}\cdot 523164-\frac{4}{45}\cdot 523614\\
&-\frac{2}{45}\cdot 613254-\frac{2}{45}\cdot 613524+\frac{2}{45}\cdot 134256+\frac{1}{9}\cdot 143256+\frac{2}{45}\cdot 143265-\frac{1}{45}\cdot 135426\\
&-\frac{1}{45}\cdot 135462-\frac{2}{45}\cdot 153426+\frac{1}{45}\cdot 153462-\frac{2}{45}\cdot 136245-\frac{2}{45}\cdot 136254-\frac{4}{45}\cdot 145236\\
&-\frac{2}{45}\cdot 145263-\frac{2}{45}\cdot 154236-\frac{2}{45}\cdot 154263-\frac{2}{45}\cdot 163245-\frac{2}{45}\cdot 214356-\frac{2}{45}\cdot 241356\\
&-\frac{2}{45}\cdot 241365+\frac{1}{45}\cdot 215346+\frac{2}{45}\cdot 245316+\frac{2}{45}\cdot 245361+\frac{2}{45}\cdot 254316+\frac{4}{45}\cdot 254361\\
&+\frac{1}{45}\cdot 312546+\frac{1}{45}\cdot 315246-\frac{2}{45}\cdot 314526-\frac{2}{45}\cdot 315426-\frac{2}{45}\cdot 413625-\frac{2}{45}\cdot 416325\\
&-\frac{2}{45}\cdot 513624-\frac{2}{45}\cdot 516324-\frac{4}{45}\cdot 325416-\frac{2}{45}\cdot 325461-\frac{2}{45}\cdot 352416-\frac{2}{45}\cdot 352461\\
&+\frac{1}{45}\cdot 513426+\frac{2}{45}\cdot 514326+\frac{2}{45}\cdot 613425+\frac{4}{45}\cdot 614325-\frac{4}{45}\cdot 521436-\frac{2}{45}\cdot 524136\\
&-\frac{2}{45}\cdot 621435-\frac{2}{45}\cdot 624135+\frac{2}{45}\cdot 125346+\frac{2}{45}\cdot 215436+\frac{1}{45}\cdot 132564+\frac{1}{45}\cdot 135264\\
&+\frac{2}{45}\cdot 142356+\frac{1}{45}\cdot 143526+\frac{1}{45}\cdot 413256+\frac{1}{45}\cdot 413526-\frac{2}{45}\cdot 145326-\frac{2}{45}\cdot 235146\\
&-\frac{2}{45}\cdot 235416-\frac{2}{45}\cdot 325146-\frac{2}{45}\cdot 415236-\frac{2}{45}\cdot 415326-\frac{1}{45}\cdot 153246-\frac{1}{45}\cdot 513246\\
&-\frac{2}{45}\cdot 152364-\frac{2}{45}\cdot 153264-\frac{2}{45}\cdot 251463-\frac{2}{45}\cdot 254163-\frac{2}{45}\cdot 351462-\frac{2}{45}\cdot 354162\\
&+\frac{2}{45}\cdot 154362+\frac{2}{45}\cdot 253461+\frac{2}{45}\cdot 164235+\frac{2}{45}\cdot 164325+\frac{2}{45}\cdot 614235+\frac{2}{45}\cdot 145623\\
&+\frac{2}{45}\cdot 145632+\frac{2}{45}\cdot 154623+\frac{2}{45}\cdot 154632+\frac{1}{45}\cdot 136425+\frac{1}{45}\cdot 136452+\frac{1}{45}\cdot 163425\\
&+\frac{1}{45}\cdot 163452+\frac{1}{45}\cdot 214536+\frac{1}{15}\cdot 214563+\frac{1}{45}\cdot 241536+\frac{1}{45}\cdot 241563+\frac{2}{45}\cdot 215463\\
&+\frac{2}{45}\cdot 314562+\frac{2}{45}\cdot 315462-\frac{1}{45}\cdot 235164-\frac{1}{45}\cdot 246513-\frac{1}{45}\cdot 246531-\frac{1}{45}\cdot 264513\\
&-\frac{1}{45}\cdot 264531-\frac{2}{45}\cdot 513462-\frac{2}{45}\cdot 514362+\frac{1}{45}\cdot 315624-\frac{1}{45}\cdot 315642-\frac{2}{45}\cdot 351624\\
&-\frac{1}{45}\cdot 351642+\frac{1}{45}\cdot 513642+\frac{1}{45}\cdot 516342+\frac{1}{45}\cdot 325614+\frac{1}{45}\cdot 325641+\frac{1}{45}\cdot 352614\\
&+\frac{1}{45}\cdot 352641-\frac{1}{45}\cdot 613542-\frac{1}{45}\cdot 615342+\frac{1}{45}\cdot 621453+\frac{1}{45}\cdot 624153+\frac{2}{45}\cdot 156234\\
&+\frac{2}{45}\cdot 156243+\frac{2}{45}\cdot 165234+\frac{2}{45}\cdot 165243+\frac{1}{15}\cdot 216345+\frac{2}{45}\cdot 216354+\frac{2}{45}\cdot 261345\\
&+\frac{1}{45}\cdot 261354+\frac{1}{45}\cdot 213645-\frac{2}{45}\cdot 256314-\frac{2}{45}\cdot 256341-\frac{2}{45}\cdot 265314-\frac{2}{45}\cdot 265341\\
&-\frac{1}{45}\cdot 316245-\frac{2}{45}\cdot 316425-\frac{2}{45}\cdot 316452-\frac{2}{45}\cdot 361425-\frac{4}{45}\cdot 361452+\frac{2}{45}\cdot 316524
\end{aligned}
$$

$$+\frac{2}{45}\cdot 415623+\frac{4}{45}\cdot 416523-\frac{2}{45}\cdot 614523-\frac{2}{45}\cdot 615423+\frac{2}{45}\cdot 421635+\frac{2}{45}\cdot 426135$$
$$+\frac{1}{9}\cdot 521634+\frac{2}{45}\cdot 526134+\frac{2}{45}\cdot 312456+\frac{1}{9}\cdot 321456+\frac{2}{45}\cdot 321465+\frac{1}{45}\cdot 324156$$
$$-\frac{4}{45}\cdot 341256-\frac{2}{45}\cdot 342156-\frac{1}{45}\cdot 421356-\frac{2}{45}\cdot 423156-\frac{2}{45}\cdot 412536-\frac{2}{45}\cdot 421536$$
$$-\frac{2}{45}\cdot 421563+\frac{1}{45}\cdot 423516+\frac{2}{45}\cdot 423561+\frac{2}{45}\cdot 432516+\frac{1}{15}\cdot 432561+\frac{2}{45}\cdot 531246$$
$$+\frac{2}{45}\cdot 532146+\frac{2}{45}\cdot 631245+\frac{1}{15}\cdot 632145+\frac{2}{45}\cdot 231456+\frac{2}{45}\cdot 321546-\frac{1}{45}\cdot 243156$$
$$-\frac{1}{45}\cdot 243516-\frac{1}{45}\cdot 326451-\frac{2}{45}\cdot 251346-\frac{2}{45}\cdot 251436-\frac{2}{45}\cdot 341526-\frac{2}{45}\cdot 431256$$
$$-\frac{2}{45}\cdot 431526-\frac{2}{45}\cdot 521346+\frac{1}{45}\cdot 431562-\frac{1}{45}\cdot 435162+\frac{1}{45}\cdot 251364+\frac{1}{45}\cdot 251634$$
$$+\frac{1}{45}\cdot 521364+\frac{1}{45}\cdot 435261-\frac{1}{45}\cdot 261534-\frac{1}{45}\cdot 621534+\frac{1}{45}\cdot 362145+\frac{1}{45}\cdot 362415$$
$$+\frac{1}{45}\cdot 632415+\frac{2}{45}\cdot 345126+\frac{2}{45}\cdot 345216+\frac{2}{45}\cdot 435126+\frac{2}{45}\cdot 435216+\frac{1}{45}\cdot 253146$$
$$+\frac{1}{45}\cdot 253416+\frac{1}{45}\cdot 523146+\frac{1}{45}\cdot 523416+\frac{1}{45}\cdot 351264+\frac{2}{45}\cdot 352164+\frac{2}{45}\cdot 451263$$
$$+\frac{4}{45}\cdot 452163-\frac{2}{45}\cdot 452361-\frac{2}{45}\cdot 453261-\frac{2}{45}\cdot 364125-\frac{2}{45}\cdot 364215-\frac{2}{45}\cdot 634125$$
$$-\frac{2}{45}\cdot 634215+\frac{2}{45}\cdot 356412+\frac{2}{45}\cdot 356421+\frac{2}{45}\cdot 365412+\frac{2}{45}\cdot 365421+\frac{1}{45}\cdot 423651$$
$$+\frac{1}{45}\cdot 426351+\frac{2}{45}\cdot 416532+\frac{2}{45}\cdot 461523+\frac{2}{45}\cdot 461532-\frac{2}{45}\cdot 425631-\frac{2}{45}\cdot 426531$$
$$-\frac{2}{45}\cdot 436512-\frac{2}{45}\cdot 436521-\frac{2}{45}\cdot 463512-\frac{2}{45}\cdot 463521+\frac{2}{45}\cdot 624531+\frac{2}{45}\cdot 625431$$
$$-\frac{2}{45}\cdot 531642-\frac{2}{45}\cdot 536142-\frac{2}{45}\cdot 632541-\frac{2}{45}\cdot 635241+\frac{2}{45}\cdot 451236+\frac{2}{45}\cdot 451326$$
$$+\frac{2}{45}\cdot 541236+\frac{2}{45}\cdot 541326+\frac{1}{45}\cdot 531462+\frac{1}{45}\cdot 534162-\frac{1}{45}\cdot 531264-\frac{1}{45}\cdot 531624$$
$$-\frac{1}{45}\cdot 532461-\frac{1}{45}\cdot 534261+\frac{1}{45}\cdot 361254+\frac{1}{45}\cdot 361524+\frac{1}{45}\cdot 631254+\frac{1}{45}\cdot 631524$$
$$-\frac{1}{45}\cdot 462135-\frac{1}{45}\cdot 462315-\frac{1}{45}\cdot 642135-\frac{1}{45}\cdot 642315+\frac{2}{45}\cdot 512634+\frac{2}{45}\cdot 521643$$
$$-\frac{2}{45}\cdot 514623-\frac{2}{45}\cdot 514632-\frac{2}{45}\cdot 523641-\frac{2}{45}\cdot 532614-\frac{2}{45}\cdot 532641-\frac{2}{45}\cdot 541623$$
$$-\frac{4}{45}\cdot 541632-\frac{2}{45}\cdot 641253-\frac{2}{45}\cdot 642153+\frac{2}{45}\cdot 341562+\frac{2}{45}\cdot 431652-\frac{2}{45}\cdot 361542$$
$$-\frac{2}{45}\cdot 451362-\frac{2}{45}\cdot 451632-\frac{2}{45}\cdot 541362-\frac{2}{45}\cdot 631452-\frac{2}{45}\cdot 631542+\frac{2}{45}\cdot 452613$$
$$+\frac{2}{45}\cdot 542163+\frac{2}{45}\cdot 542613+\frac{2}{45}\cdot 534612+\frac{2}{45}\cdot 534621+\frac{2}{45}\cdot 543612+\frac{2}{45}\cdot 543621$$
$$+\frac{2}{45}\cdot 642351+\frac{2}{45}\cdot 643251+\frac{2}{45}\cdot 561342+\frac{2}{45}\cdot 561432+\frac{2}{45}\cdot 651342+\frac{2}{45}\cdot 651432$$
$$-\frac{2}{45}\cdot 562143-\frac{2}{45}\cdot 562413-\frac{2}{45}\cdot 652143-\frac{2}{45}\cdot 652413+\frac{2}{45}\cdot 563124+\frac{2}{45}\cdot 563214$$
$$+\frac{2}{45}\cdot 653124+\frac{2}{45}\cdot 653214$$

$$
\begin{aligned}
[\![y_1 \times y_1]\!] = {} & \frac{1}{15}\cdot 123465 + \frac{2}{45}\cdot 124365 + \frac{2}{45}\cdot 132465 - \frac{1}{45}\cdot 134265 - \frac{1}{45}\cdot 142365 + \frac{2}{45}\cdot 213465 \\
& + \frac{1}{5}\cdot 214365 - \frac{1}{45}\cdot 231465 + \frac{2}{45}\cdot 241365 - \frac{1}{45}\cdot 312465 + \frac{2}{45}\cdot 314265 + \frac{1}{45}\cdot 341265 \\
& + \frac{1}{15}\cdot 123546 + \frac{2}{45}\cdot 132546 + \frac{2}{45}\cdot 213546 - \frac{1}{45}\cdot 231546 - \frac{1}{45}\cdot 312546 - \frac{2}{15}\cdot 123654 \\
& - \frac{2}{45}\cdot 124653 - \frac{1}{9}\cdot 132654 + \frac{1}{45}\cdot 142653 - \frac{1}{9}\cdot 213654 - \frac{1}{15}\cdot 214653 + \frac{2}{45}\cdot 231654 \\
& + \frac{2}{45}\cdot 312654 - \frac{1}{15}\cdot 314652 - \frac{8}{45}\cdot 341652 - \frac{2}{45}\cdot 126354 + \frac{1}{45}\cdot 136254 - \frac{1}{15}\cdot 216354 \\
& - \frac{1}{15}\cdot 261354 - \frac{8}{45}\cdot 361254 + \frac{1}{15}\cdot 124356 - \frac{1}{9}\cdot 143265 - \frac{1}{9}\cdot 234165 - \frac{1}{15}\cdot 243165 \\
& - \frac{1}{9}\cdot 321465 - \frac{1}{15}\cdot 324165 + \frac{2}{45}\cdot 342165 - \frac{1}{9}\cdot 412365 - \frac{1}{15}\cdot 413265 - \frac{1}{15}\cdot 421365 \\
& + \frac{2}{45}\cdot 431265 + \frac{2}{45}\cdot 124563 + \frac{1}{45}\cdot 142563 + \frac{2}{45}\cdot 145263 + \frac{1}{9}\cdot 412563 + \frac{4}{45}\cdot 415263 \\
& - \frac{1}{45}\cdot 124635 - \frac{2}{45}\cdot 142635 - \frac{2}{45}\cdot 412635 + \frac{8}{45}\cdot 143652 + \frac{1}{15}\cdot 234651 + \frac{1}{9}\cdot 243651 \\
& + \frac{1}{15}\cdot 324651 - \frac{2}{45}\cdot 342651 + \frac{1}{15}\cdot 412653 + \frac{2}{45}\cdot 413652 - \frac{2}{45}\cdot 423651 - \frac{1}{45}\cdot 125364 \\
& - \frac{2}{45}\cdot 135264 - \frac{2}{45}\cdot 235164 - \frac{2}{15}\cdot 125436 - \frac{2}{45}\cdot 135426 - \frac{2}{45}\cdot 152436 - \frac{2}{45}\cdot 125463 \\
& + \frac{1}{45}\cdot 135462 + \frac{1}{9}\cdot 235461 - \frac{2}{45}\cdot 152463 + \frac{1}{45}\cdot 154263 - \frac{2}{45}\cdot 514263 - \frac{1}{15}\cdot 541263 \\
& + \frac{2}{45}\cdot 125634 + \frac{2}{45}\cdot 135624 + \frac{2}{45}\cdot 152634 + \frac{1}{15}\cdot 125643 + \frac{1}{45}\cdot 152643 - \frac{2}{45}\cdot 156243 \\
& - \frac{1}{45}\cdot 512643 + \frac{2}{45}\cdot 516243 + \frac{1}{15}\cdot 561243 + \frac{2}{45}\cdot 126345 + \frac{1}{45}\cdot 136245 + \frac{2}{45}\cdot 146235 \\
& + \frac{1}{9}\cdot 236145 + \frac{4}{45}\cdot 246135 + \frac{8}{45}\cdot 163254 + \frac{1}{15}\cdot 236154 + \frac{2}{45}\cdot 263154 + \frac{1}{15}\cdot 612354 \\
& + \frac{1}{9}\cdot 613254 + \frac{1}{15}\cdot 621354 - \frac{2}{45}\cdot 623154 - \frac{2}{45}\cdot 631254 - \frac{2}{45}\cdot 126435 - \frac{2}{45}\cdot 136425 \\
& + \frac{1}{45}\cdot 146325 - \frac{2}{45}\cdot 246315 - \frac{1}{15}\cdot 346215 + \frac{1}{45}\cdot 162435 + \frac{1}{9}\cdot 612435 + \frac{1}{45}\cdot 126453 \\
& + \frac{1}{15}\cdot 126534 + \frac{1}{45}\cdot 136524 - \frac{2}{45}\cdot 146523 - \frac{1}{45}\cdot 236514 + \frac{2}{45}\cdot 246513 + \frac{1}{15}\cdot 346512 \\
& + \frac{2}{45}\cdot 126543 - \frac{2}{45}\cdot 136542 - \frac{1}{15}\cdot 146532 - \frac{11}{45}\cdot 236541 - \frac{4}{45}\cdot 246531 - \frac{2}{45}\cdot 162543 \\
& - \frac{1}{45}\cdot 163542 - \frac{4}{45}\cdot 263541 - \frac{11}{45}\cdot 612543 - \frac{4}{45}\cdot 613542 - \frac{1}{15}\cdot 165243 - \frac{4}{45}\cdot 615243 \\
& + \frac{2}{45}\cdot 214356 - \frac{1}{9}\cdot 215436 - \frac{1}{15}\cdot 215463 + \frac{1}{45}\cdot 315426 - \frac{2}{45}\cdot 315462 - \frac{1}{15}\cdot 216435 \\
& + \frac{1}{45}\cdot 251436 - \frac{2}{45}\cdot 261435 + \frac{1}{15}\cdot 132456 - \frac{1}{45}\cdot 132564 - \frac{1}{45}\cdot 132645 - \frac{1}{9}\cdot 321546 \\
& + \frac{2}{45}\cdot 134526 + \frac{1}{45}\cdot 134625 + \frac{1}{45}\cdot 314526 + \frac{2}{45}\cdot 341526 - \frac{1}{45}\cdot 135246 - \frac{2}{45}\cdot 315246 \\
& + \frac{1}{45}\cdot 315264 + \frac{8}{45}\cdot 325416 + \frac{1}{9}\cdot 325461 - \frac{1}{45}\cdot 142536 - \frac{2}{45}\cdot 241536 + \frac{1}{45}\cdot 241635 \\
& - \frac{2}{15}\cdot 143256 - \frac{2}{45}\cdot 143526 + \frac{1}{45}\cdot 143625 - \frac{2}{45}\cdot 243156 + \frac{1}{45}\cdot 243516 - \frac{2}{45}\cdot 243615 \\
& - \frac{2}{45}\cdot 153246 + \frac{1}{45}\cdot 153264 - \frac{2}{45}\cdot 413256 + \frac{1}{45}\cdot 513246 - \frac{2}{45}\cdot 513264 + \frac{1}{9}\cdot 243561
\end{aligned}
$$

$$
\begin{aligned}
&-\frac{2}{45}\cdot 413526+\frac{1}{45}\cdot 431526+\frac{2}{45}\cdot 145236+\frac{2}{45}\cdot 245136+\frac{2}{45}\cdot 415236+\frac{1}{15}\cdot 145326\\
&-\frac{2}{45}\cdot 156324+\frac{1}{45}\cdot 415326+\frac{7}{45}\cdot 416325-\frac{2}{45}\cdot 451326+\frac{1}{15}\cdot 461325+\frac{1}{15}\cdot 516324\\
&+\frac{1}{9}\cdot 561324+\frac{2}{45}\cdot 152346+\frac{1}{45}\cdot 152364+\frac{1}{45}\cdot 251346+\frac{2}{45}\cdot 351246+\frac{8}{45}\cdot 521436\\
&+\frac{1}{9}\cdot 621435-\frac{2}{45}\cdot 253146+\frac{1}{45}\cdot 352146+\frac{1}{9}\cdot 613245+\frac{1}{45}\cdot 153426+\frac{1}{15}\cdot 154236\\
&-\frac{2}{45}\cdot 154623+\frac{1}{45}\cdot 254136+\frac{7}{45}\cdot 254163+\frac{1}{15}\cdot 254613-\frac{2}{45}\cdot 354126+\frac{1}{15}\cdot 354162\\
&+\frac{1}{9}\cdot 354612+\frac{2}{45}\cdot 154326-\frac{2}{45}\cdot 154362-\frac{1}{15}\cdot 154632-\frac{2}{45}\cdot 254316-\frac{4}{15}\cdot 254361\\
&-\frac{1}{15}\cdot 254631-\frac{1}{15}\cdot 354216-\frac{1}{15}\cdot 354261+\frac{2}{45}\cdot 354621-\frac{2}{45}\cdot 164325-\frac{1}{45}\cdot 164352\\
&+\frac{2}{45}\cdot 264315-\frac{1}{15}\cdot 264351-\frac{2}{45}\cdot 514326+\frac{2}{45}\cdot 514362-\frac{1}{45}\cdot 524316-\frac{1}{15}\cdot 524361\\
&-\frac{4}{15}\cdot 614325-\frac{1}{15}\cdot 614352-\frac{1}{15}\cdot 624315+\frac{2}{45}\cdot 624351-\frac{1}{15}\cdot 165324-\frac{1}{15}\cdot 541326\\
&-\frac{1}{15}\cdot 615324-\frac{1}{15}\cdot 641325+\frac{2}{45}\cdot 651324+\frac{2}{45}\cdot 216534+\frac{13}{45}\cdot 216543+\frac{1}{9}\cdot 316542\\
&+\frac{1}{9}\cdot 261543+\frac{1}{9}\cdot 361542+\frac{4}{15}\cdot 321654+\frac{1}{9}\cdot 421653-\frac{1}{15}\cdot 431652-\frac{1}{9}\cdot 145632\\
&-\frac{1}{15}\cdot 415632+\frac{2}{45}\cdot 146352+\frac{2}{45}\cdot 416352-\frac{1}{15}\cdot 326514-\frac{1}{15}\cdot 326541-\frac{8}{45}\cdot 416523\\
&-\frac{1}{15}\cdot 416532-\frac{1}{15}\cdot 426513+\frac{1}{45}\cdot 426531+\frac{2}{45}\cdot 153642+\frac{1}{15}\cdot 514632+\frac{2}{9}\cdot 541632\\
&-\frac{2}{45}\cdot 156342-\frac{8}{45}\cdot 256143-\frac{2}{45}\cdot 516342+\frac{2}{45}\cdot 156432-\frac{11}{45}\cdot 561432-\frac{1}{45}\cdot 163425\\
&-\frac{4}{45}\cdot 163452-\frac{1}{45}\cdot 162453+\frac{2}{45}\cdot 163524-\frac{1}{15}\cdot 621543+\frac{1}{45}\cdot 631542+\frac{2}{45}\cdot 164253\\
&+\frac{2}{45}\cdot 264153-\frac{1}{15}\cdot 362154-\frac{1}{9}\cdot 165234+\frac{2}{45}\cdot 165423-\frac{1}{15}\cdot 265134-\frac{1}{15}\cdot 265143\\
&+\frac{1}{15}\cdot 265314-\frac{2}{45}\cdot 365142-\frac{11}{45}\cdot 365412+\frac{14}{45}\cdot 165432+\frac{1}{15}\cdot 265341+\frac{1}{9}\cdot 265431\\
&+\frac{2}{9}\cdot 365214+\frac{2}{45}\cdot 365241-\frac{1}{9}\cdot 365421+\frac{1}{15}\cdot 615423+\frac{1}{9}\cdot 615432+\frac{2}{45}\cdot 625413\\
&-\frac{1}{9}\cdot 625431-\frac{1}{9}\cdot 651432+\frac{2}{45}\cdot 215643+\frac{1}{9}\cdot 326154-\frac{1}{45}\cdot 153462-\frac{1}{45}\cdot 136452\\
&+\frac{1}{45}\cdot 362541-\frac{2}{45}\cdot 164523-\frac{2}{45}\cdot 264513-\frac{2}{45}\cdot 461532-\frac{1}{15}\cdot 521643-\frac{1}{15}\cdot 526143\\
&+\frac{1}{45}\cdot 625143+\frac{1}{15}\cdot 256431+\frac{2}{45}\cdot 526431+\frac{1}{15}\cdot 614532+\frac{2}{45}\cdot 641532+\frac{1}{15}\cdot 213456\\
&-\frac{1}{45}\cdot 213564-\frac{1}{45}\cdot 213645-\frac{1}{45}\cdot 214536+\frac{2}{45}\cdot 214635-\frac{1}{45}\cdot 215346+\frac{2}{45}\cdot 215364\\
&+\frac{1}{45}\cdot 215634-\frac{1}{9}\cdot 214563-\frac{1}{9}\cdot 216345+\frac{2}{45}\cdot 234156+\frac{1}{45}\cdot 235146-\frac{1}{45}\cdot 241356\\
&-\frac{2}{45}\cdot 241563-\frac{2}{45}\cdot 264135-\frac{1}{45}\cdot 314256-\frac{2}{45}\cdot 316245-\frac{2}{15}\cdot 321456+\frac{2}{45}\cdot 321564\\
&+\frac{2}{45}\cdot 321645-\frac{2}{45}\cdot 324156-\frac{1}{15}\cdot 324615+\frac{1}{45}\cdot 325146-\frac{8}{45}\cdot 325614-\frac{2}{45}\cdot 421356\\
&+\frac{1}{45}\cdot 421536-\frac{1}{15}\cdot 521364-\frac{8}{45}\cdot 521634+\frac{1}{15}\cdot 324561-\frac{2}{45}\cdot 325641+\frac{1}{15}\cdot 326145
\end{aligned}
$$

$$+\frac{2}{45}\cdot 326415-\frac{2}{45}\cdot 326451+\frac{2}{45}\cdot 341256+\frac{1}{15}\cdot 342156-\frac{1}{45}\cdot 362145-\frac{2}{45}\cdot 452136$$
$$+\frac{2}{45}\cdot 462135+\frac{1}{15}\cdot 562134+\frac{2}{45}\cdot 412356+\frac{1}{45}\cdot 412536-\frac{2}{45}\cdot 415362+\frac{1}{15}\cdot 421563$$
$$+\frac{2}{45}\cdot 521463+\frac{1}{15}\cdot 621345-\frac{2}{45}\cdot 621453-\frac{2}{45}\cdot 621534+\frac{1}{45}\cdot 423156+\frac{1}{15}\cdot 431256$$
$$-\frac{1}{45}\cdot 431562-\frac{2}{45}\cdot 435126+\frac{2}{45}\cdot 435162+\frac{1}{15}\cdot 435612+\frac{2}{45}\cdot 432156-\frac{2}{45}\cdot 432516$$
$$-\frac{11}{45}\cdot 432561-\frac{1}{15}\cdot 435216-\frac{4}{45}\cdot 435261-\frac{2}{45}\cdot 532146-\frac{1}{45}\cdot 532416-\frac{4}{45}\cdot 532461$$
$$-\frac{11}{45}\cdot 632145-\frac{4}{45}\cdot 632415-\frac{1}{15}\cdot 542136-\frac{4}{45}\cdot 642135-\frac{2}{45}\cdot 245163-\frac{2}{45}\cdot 246153$$
$$+\frac{1}{45}\cdot 253164-\frac{1}{45}\cdot 351264-\frac{1}{45}\cdot 341625-\frac{8}{45}\cdot 452163-\frac{1}{15}\cdot 462153+\frac{2}{45}\cdot 562143$$
$$-\frac{2}{45}\cdot 416235-\frac{2}{45}\cdot 416253+\frac{1}{45}\cdot 413625-\frac{8}{45}\cdot 436125-\frac{1}{15}\cdot 436152+\frac{2}{45}\cdot 436512$$
$$+\frac{13}{45}\cdot 432165+\frac{1}{9}\cdot 432615-\frac{1}{15}\cdot 432651-\frac{1}{15}\cdot 436215+\frac{1}{45}\cdot 436251+\frac{13}{45}\cdot 436521$$
$$+\frac{1}{9}\cdot 532164+\frac{1}{9}\cdot 532614+\frac{1}{45}\cdot 532641-\frac{1}{15}\cdot 632154+\frac{1}{45}\cdot 632514+\frac{13}{45}\cdot 632541$$
$$-\frac{1}{15}\cdot 542163+\frac{1}{45}\cdot 642153+\frac{13}{45}\cdot 652143-\frac{2}{45}\cdot 425163+\frac{1}{45}\cdot 251463+\frac{2}{45}\cdot 524163$$
$$-\frac{1}{45}\cdot 315624-\frac{1}{45}\cdot 251634-\frac{2}{45}\cdot 426135+\frac{1}{45}\cdot 316425+\frac{2}{45}\cdot 426315+\frac{7}{45}\cdot 234561$$
$$-\frac{2}{45}\cdot 245361+\frac{1}{45}\cdot 246351-\frac{2}{45}\cdot 253461+\frac{1}{45}\cdot 253641+\frac{7}{45}\cdot 256341-\frac{1}{45}\cdot 245631$$
$$-\frac{1}{45}\cdot 263451+\frac{2}{45}\cdot 264531-\frac{1}{15}\cdot 314562+\frac{1}{45}\cdot 315642-\frac{1}{15}\cdot 346152+\frac{1}{45}\cdot 351462$$
$$-\frac{2}{45}\cdot 351642-\frac{1}{15}\cdot 356142-\frac{1}{9}\cdot 345216-\frac{1}{45}\cdot 423516-\frac{4}{45}\cdot 523416-\frac{1}{45}\cdot 345261$$
$$+\frac{2}{45}\cdot 346251+\frac{2}{45}\cdot 356241+\frac{8}{45}\cdot 345612+\frac{8}{45}\cdot 361452+\frac{2}{45}\cdot 364152+\frac{1}{45}\cdot 352461$$
$$+\frac{2}{45}\cdot 362451+\frac{7}{45}\cdot 452361+\frac{2}{45}\cdot 462351+\frac{2}{45}\cdot 562341+\frac{1}{5}\cdot 456123+\frac{1}{15}\cdot 456132$$
$$+\frac{1}{45}\cdot 513462-\frac{1}{45}\cdot 613452-\frac{1}{15}\cdot 425613-\frac{1}{15}\cdot 452613+\frac{1}{15}\cdot 456213+\frac{8}{45}\cdot 523614$$
$$+\frac{2}{45}\cdot 524613-\frac{1}{45}\cdot 623415+\frac{2}{45}\cdot 623514+\frac{2}{45}\cdot 624513+\frac{1}{45}\cdot 425361+\frac{2}{45}\cdot 425631$$
$$+\frac{2}{45}\cdot 452631+\frac{2}{45}\cdot 456231+\frac{2}{45}\cdot 456312-\frac{2}{9}\cdot 456321+\frac{1}{15}\cdot 453261-\frac{2}{45}\cdot 453621$$
$$-\frac{2}{45}\cdot 534621-\frac{2}{9}\cdot 634521+\frac{1}{15}\cdot 542361-\frac{2}{45}\cdot 642351-\frac{2}{9}\cdot 652341-\frac{1}{15}\cdot 234615$$
$$+\frac{1}{45}\cdot 253614+\frac{1}{45}\cdot 342615-\frac{2}{45}\cdot 352614-\frac{1}{45}\cdot 253416-\frac{1}{45}\cdot 523461+\frac{2}{45}\cdot 534261$$
$$+\frac{2}{45}\cdot 523641+\frac{2}{45}\cdot 526341+\frac{2}{45}\cdot 631452+\frac{2}{45}\cdot 634152+\frac{1}{45}\cdot 263415-\frac{2}{45}\cdot 356421$$
$$-\frac{2}{45}\cdot 364521-\frac{2}{45}\cdot 625341+\frac{2}{45}\cdot 426153-\frac{4}{45}\cdot 426351+\frac{1}{45}\cdot 351624+\frac{2}{45}\cdot 352416$$
$$+\frac{2}{45}\cdot 524136-\frac{4}{45}\cdot 352641-\frac{2}{45}\cdot 542613-\frac{1}{15}\cdot 526134-\frac{1}{15}\cdot 536124+\frac{2}{45}\cdot 536142$$
$$-\frac{1}{45}\cdot 256413-\frac{4}{45}\cdot 526413+\frac{1}{45}\cdot 562413-\frac{1}{15}\cdot 261345+\frac{1}{45}\cdot 261534+\frac{1}{45}\cdot 361425$$

$$
\begin{aligned}
&-\frac{2}{45}\cdot 361524-\frac{1}{15}\cdot 461253-\frac{1}{15}\cdot 461523+\frac{2}{45}\cdot 461352+\frac{1}{45}\cdot 613524-\frac{4}{45}\cdot 631524\\
&+\frac{1}{45}\cdot 624135-\frac{4}{45}\cdot 624153-\frac{2}{45}\cdot 263514-\frac{2}{45}\cdot 362415-\frac{1}{45}\cdot 362514-\frac{2}{45}\cdot 462315\\
&-\frac{1}{45}\cdot 463125-\frac{4}{45}\cdot 463152+\frac{1}{45}\cdot 463512+\frac{2}{45}\cdot 463251+\frac{4}{45}\cdot 463521+\frac{1}{15}\cdot 364215\\
&+\frac{2}{45}\cdot 635214+\frac{4}{45}\cdot 635241+\frac{4}{45}\cdot 652413+\frac{2}{45}\cdot 425316-\frac{2}{45}\cdot 364251-\frac{2}{45}\cdot 462531\\
&-\frac{1}{15}\cdot 562431+\frac{1}{15}\cdot 465123+\frac{1}{15}\cdot 465132-\frac{2}{45}\cdot 513642+\frac{2}{45}\cdot 462513+\frac{1}{15}\cdot 465213\\
&+\frac{2}{45}\cdot 526314-\frac{2}{45}\cdot 625314-\frac{1}{15}\cdot 465231-\frac{1}{15}\cdot 465312-\frac{1}{15}\cdot 465321+\frac{4}{45}\cdot 536421\\
&-\frac{1}{15}\cdot 635421+\frac{2}{45}\cdot 542631+\frac{4}{45}\cdot 642531-\frac{1}{15}\cdot 652431-\frac{2}{45}\cdot 524631+\frac{1}{45}\cdot 256314\\
&-\frac{1}{15}\cdot 635412+\frac{2}{45}\cdot 531426-\frac{1}{45}\cdot 453162+\frac{1}{45}\cdot 563142-\frac{1}{15}\cdot 512364+\frac{1}{45}\cdot 513624\\
&+\frac{1}{45}\cdot 531264-\frac{2}{45}\cdot 531624+\frac{1}{45}\cdot 614253-\frac{2}{45}\cdot 536214+\frac{1}{45}\cdot 631425-\frac{2}{45}\cdot 531462\\
&-\frac{1}{45}\cdot 531642-\frac{2}{45}\cdot 534162-\frac{1}{45}\cdot 516423+\frac{1}{45}\cdot 536412+\frac{1}{15}\cdot 541362+\frac{2}{45}\cdot 643152\\
&+\frac{4}{45}\cdot 653142-\frac{2}{45}\cdot 452316+\frac{2}{45}\cdot 453216-\frac{11}{45}\cdot 563214-\frac{1}{45}\cdot 523146-\frac{1}{45}\cdot 513426\\
&-\frac{1}{9}\cdot 541236+\frac{2}{45}\cdot 543126-\frac{11}{45}\cdot 543612+\frac{14}{45}\cdot 543216+\frac{1}{9}\cdot 543261-\frac{1}{9}\cdot 543621\\
&+\frac{1}{15}\cdot 643125+\frac{1}{9}\cdot 643215-\frac{1}{9}\cdot 643251-\frac{1}{9}\cdot 653214-\frac{2}{45}\cdot 534126+\frac{1}{15}\cdot 634215\\
&+\frac{1}{45}\cdot 451362-\frac{1}{15}\cdot 563241+\frac{1}{15}\cdot 546123+\frac{1}{15}\cdot 546132+\frac{1}{15}\cdot 546213-\frac{1}{15}\cdot 546231\\
&-\frac{1}{15}\cdot 546312-\frac{1}{15}\cdot 546321-\frac{1}{15}\cdot 643512-\frac{1}{15}\cdot 643521-\frac{1}{15}\cdot 653241-\frac{2}{45}\cdot 536241\\
&-\frac{2}{45}\cdot 641352+\frac{2}{15}\cdot 563412+\frac{8}{45}\cdot 561234+\frac{1}{45}\cdot 514623+\frac{7}{45}\cdot 614523+\frac{7}{45}\cdot 634125\\
&+\frac{2}{45}\cdot 635124+\frac{1}{45}\cdot 563421-\frac{1}{15}\cdot 564132+\frac{1}{45}\cdot 564312-\frac{1}{15}\cdot 645132+\frac{1}{45}\cdot 645231\\
&+\frac{1}{45}\cdot 653412+\frac{2}{45}\cdot 641523+\frac{1}{45}\cdot 364125-\frac{1}{15}\cdot 564213-\frac{1}{15}\cdot 645213+\frac{1}{15}\cdot 345621\\
&+\frac{2}{45}\cdot 564123+\frac{1}{45}\cdot 564231+\frac{2}{45}\cdot 564321+\frac{2}{45}\cdot 645321+\frac{2}{45}\cdot 653421+\frac{7}{45}\cdot 612345\\
&-\frac{2}{45}\cdot 613425-\frac{2}{45}\cdot 614235-\frac{1}{45}\cdot 615234+\frac{2}{45}\cdot 615342-\frac{1}{45}\cdot 641235+\frac{2}{45}\cdot 641253\\
&+\frac{2}{45}\cdot 625134+\frac{2}{45}\cdot 645123+\frac{2}{45}\cdot 634512-\frac{2}{45}\cdot 634251-\frac{2}{45}\cdot 653124-\frac{2}{9}\cdot 654123\\
&-\frac{2}{45}\cdot 652314+\frac{2}{45}\cdot 642315-\frac{2}{45}\cdot 624531-\frac{2}{45}\cdot 651423-\frac{2}{45}\cdot 651342-\frac{2}{45}\cdot 635142\\
&-\frac{1}{15}\cdot 654132-\frac{2}{45}\cdot 642513-\frac{1}{15}\cdot 654213+\frac{1}{15}\cdot 623451+\frac{1}{45}\cdot 645312+\frac{2}{45}\cdot 654231\\
&+\frac{1}{15}\cdot 651234+\frac{2}{45}\cdot 654312+\frac{7}{15}\cdot 654321
\end{aligned}
$$

$$
[\![y_1\times y_2]\!]=-\frac{1}{30}\cdot 123654-\frac{1}{90}\cdot 132654-\frac{1}{90}\cdot 213654+\frac{1}{90}\cdot 231654+\frac{1}{90}\cdot 312654+\frac{1}{90}\cdot 124563
$$

$$+\frac{1}{90}\cdot 142563+\frac{1}{45}\cdot 412563-\frac{1}{30}\cdot 125436+\frac{1}{45}\cdot 125634+\frac{1}{90}\cdot 135624+\frac{1}{90}\cdot 152634$$
$$+\frac{1}{90}\cdot 153624+\frac{1}{45}\cdot 253614+\frac{1}{45}\cdot 513624+\frac{2}{45}\cdot 523614+\frac{1}{90}\cdot 126345+\frac{1}{90}\cdot 136245$$
$$+\frac{1}{45}\cdot 236145+\frac{1}{45}\cdot 126543-\frac{1}{90}\cdot 136542-\frac{7}{90}\cdot 236541-\frac{1}{90}\cdot 162543-\frac{7}{90}\cdot 612543$$
$$-\frac{1}{90}\cdot 215436+\frac{1}{90}\cdot 134526+\frac{1}{90}\cdot 134625+\frac{1}{90}\cdot 314526+\frac{1}{90}\cdot 314625-\frac{1}{30}\cdot 143256$$
$$-\frac{1}{90}\cdot 143265+\frac{1}{45}\cdot 145236+\frac{1}{90}\cdot 145263+\frac{1}{90}\cdot 146235+\frac{1}{90}\cdot 146253+\frac{1}{90}\cdot 245136$$
$$+\frac{1}{90}\cdot 415236+\frac{1}{90}\cdot 425136+\frac{1}{90}\cdot 152346+\frac{1}{90}\cdot 152364+\frac{1}{90}\cdot 251346+\frac{1}{90}\cdot 251364$$
$$+\frac{1}{45}\cdot 154326-\frac{1}{90}\cdot 154362-\frac{1}{90}\cdot 254316-\frac{1}{18}\cdot 254361-\frac{1}{90}\cdot 164325-\frac{1}{90}\cdot 514326$$
$$-\frac{1}{18}\cdot 614325+\frac{1}{15}\cdot 216543+\frac{1}{90}\cdot 316542-\frac{1}{30}\cdot 145632-\frac{1}{45}\cdot 415632-\frac{1}{45}\cdot 156324$$
$$-\frac{1}{45}\cdot 156342-\frac{1}{45}\cdot 156243-\frac{1}{18}\cdot 256143-\frac{1}{90}\cdot 516243-\frac{1}{90}\cdot 516342-\frac{1}{90}\cdot 526143$$
$$-\frac{1}{90}\cdot 162435-\frac{1}{90}\cdot 162453-\frac{1}{90}\cdot 163425-\frac{1}{18}\cdot 163452-\frac{1}{90}\cdot 261435-\frac{1}{90}\cdot 261453$$
$$+\frac{1}{90}\cdot 165423+\frac{2}{15}\cdot 165432+\frac{1}{45}\cdot 265431+\frac{1}{45}\cdot 615432+\frac{1}{90}\cdot 261543-\frac{1}{90}\cdot 135462$$
$$-\frac{1}{90}\cdot 136452-\frac{1}{90}\cdot 153462-\frac{1}{90}\cdot 315462-\frac{1}{90}\cdot 316452-\frac{1}{45}\cdot 154623-\frac{1}{45}\cdot 164523$$
$$-\frac{1}{45}\cdot 146523-\frac{1}{90}\cdot 246513-\frac{1}{90}\cdot 264513-\frac{1}{18}\cdot 416523-\frac{1}{90}\cdot 426513-\frac{1}{30}\cdot 165234$$
$$-\frac{1}{45}\cdot 265134+\frac{1}{90}\cdot 156432+\frac{1}{90}\cdot 234156+\frac{1}{90}\cdot 235146-\frac{1}{30}\cdot 321456-\frac{1}{90}\cdot 321465$$
$$-\frac{1}{90}\cdot 321546+\frac{1}{90}\cdot 321564+\frac{1}{90}\cdot 321645+\frac{1}{45}\cdot 341256+\frac{1}{90}\cdot 341526+\frac{1}{90}\cdot 351246$$
$$+\frac{1}{90}\cdot 351426+\frac{1}{45}\cdot 351462+\frac{1}{45}\cdot 361425+\frac{2}{45}\cdot 361452+\frac{1}{90}\cdot 412356+\frac{1}{90}\cdot 412536$$
$$+\frac{1}{45}\cdot 432156-\frac{1}{90}\cdot 432516-\frac{7}{90}\cdot 432561-\frac{1}{90}\cdot 532146-\frac{7}{90}\cdot 632145-\frac{1}{90}\cdot 234165$$
$$-\frac{1}{90}\cdot 235164-\frac{1}{90}\cdot 236154+\frac{1}{15}\cdot 321654-\frac{1}{45}\cdot 341265-\frac{1}{90}\cdot 341625-\frac{1}{18}\cdot 341652$$
$$-\frac{1}{90}\cdot 351264-\frac{1}{45}\cdot 351624-\frac{1}{45}\cdot 351642-\frac{1}{18}\cdot 361254-\frac{1}{45}\cdot 361524-\frac{1}{45}\cdot 361542$$
$$-\frac{1}{90}\cdot 412365-\frac{1}{90}\cdot 412635-\frac{1}{90}\cdot 412653+\frac{1}{15}\cdot 432165+\frac{1}{90}\cdot 432615+\frac{1}{90}\cdot 532164$$
$$-\frac{1}{90}\cdot 214563-\frac{1}{90}\cdot 241563-\frac{1}{90}\cdot 421563-\frac{1}{45}\cdot 215634-\frac{1}{90}\cdot 251634-\frac{1}{90}\cdot 315624$$
$$-\frac{1}{18}\cdot 325614-\frac{1}{45}\cdot 352614-\frac{1}{18}\cdot 521634-\frac{1}{45}\cdot 531624-\frac{1}{45}\cdot 532614-\frac{1}{90}\cdot 216345$$
$$-\frac{1}{90}\cdot 316245-\frac{1}{90}\cdot 326145-\frac{1}{90}\cdot 143562-\frac{1}{90}\cdot 145362+\frac{1}{15}\cdot 234561+\frac{1}{90}\cdot 234651$$
$$+\frac{1}{90}\cdot 235461-\frac{1}{90}\cdot 235641-\frac{1}{90}\cdot 236451-\frac{1}{90}\cdot 324516-\frac{1}{90}\cdot 324615-\frac{1}{90}\cdot 342516$$
$$-\frac{1}{90}\cdot 342615-\frac{1}{30}\cdot 345216-\frac{1}{45}\cdot 346215-\frac{1}{90}\cdot 356214+\frac{2}{15}\cdot 345612+\frac{1}{45}\cdot 346512$$
$$+\frac{1}{45}\cdot 354612+\frac{1}{90}\cdot 345162-\frac{1}{90}\cdot 415623+\frac{1}{45}\cdot 451623+\frac{2}{15}\cdot 456123-\frac{1}{45}\cdot 435621$$

$$- \frac{1}{45} \cdot 453621 - \frac{7}{90} \cdot 456321 - \frac{1}{90} \cdot 435261 - \frac{1}{90} \cdot 532461 - \frac{1}{90} \cdot 534261 - \frac{1}{45} \cdot 534621$$
$$- \frac{1}{45} \cdot 632451 - \frac{1}{45} \cdot 634251 - \frac{7}{90} \cdot 634521 - \frac{1}{90} \cdot 134652 - \frac{1}{90} \cdot 135642 - \frac{1}{90} \cdot 314652$$
$$- \frac{1}{90} \cdot 315642 - \frac{1}{90} \cdot 451632 + \frac{1}{90} \cdot 243561 + \frac{1}{90} \cdot 324561 - \frac{1}{90} \cdot 342561 - \frac{1}{90} \cdot 423561$$
$$- \frac{1}{90} \cdot 235416 - \frac{1}{90} \cdot 245316 + \frac{1}{90} \cdot 245613 + \frac{1}{45} \cdot 435612 - \frac{1}{90} \cdot 346125 + \frac{1}{45} \cdot 356124$$
$$- \frac{1}{45} \cdot 346521 - \frac{1}{45} \cdot 356421 - \frac{1}{90} \cdot 246531 - \frac{1}{90} \cdot 263541 - \frac{1}{90} \cdot 264531 - \frac{1}{45} \cdot 364521$$
$$- \frac{1}{45} \cdot 623541 - \frac{1}{45} \cdot 624531 + \frac{1}{90} \cdot 136425 + \frac{1}{90} \cdot 136524 + \frac{1}{90} \cdot 146325 + \frac{1}{90} \cdot 316425$$
$$+ \frac{1}{90} \cdot 316524 + \frac{1}{45} \cdot 416325 - \frac{1}{90} \cdot 425613 + \frac{1}{90} \cdot 253146 + \frac{1}{90} \cdot 253164 + \frac{1}{90} \cdot 254136$$
$$+ \frac{1}{45} \cdot 254163 + \frac{1}{90} \cdot 352146 + \frac{1}{90} \cdot 352164 - \frac{1}{90} \cdot 256134 - \frac{1}{18} \cdot 436125 + \frac{1}{90} \cdot 461235$$
$$- \frac{1}{90} \cdot 461253 + \frac{1}{45} \cdot 364215 + \frac{1}{90} \cdot 364251 + \frac{2}{45} \cdot 365214 + \frac{1}{90} \cdot 365241 + \frac{1}{90} \cdot 463251$$
$$+ \frac{1}{45} \cdot 265314 + \frac{1}{90} \cdot 625314 + \frac{1}{90} \cdot 625413 + \frac{1}{90} \cdot 635214 + \frac{1}{45} \cdot 143652 + \frac{1}{90} \cdot 146352$$
$$+ \frac{1}{90} \cdot 146532 + \frac{1}{45} \cdot 325416 + \frac{1}{90} \cdot 326415 + \frac{1}{90} \cdot 326514 + \frac{1}{90} \cdot 352416 + \frac{1}{90} \cdot 354216$$
$$+ \frac{1}{45} \cdot 362415 + \frac{1}{45} \cdot 362514 - \frac{1}{10} \cdot 365412 - \frac{1}{90} \cdot 346152 + \frac{1}{90} \cdot 465123 + \frac{2}{45} \cdot 436521$$
$$+ \frac{1}{45} \cdot 463521 + \frac{1}{90} \cdot 436251 + \frac{1}{90} \cdot 532641 + \frac{1}{45} \cdot 536241 + \frac{1}{45} \cdot 536421 + \frac{2}{45} \cdot 632541$$
$$+ \frac{1}{45} \cdot 635241 + \frac{1}{90} \cdot 245631 + \frac{1}{90} \cdot 425631 + \frac{1}{90} \cdot 256314 + \frac{2}{45} \cdot 256341 + \frac{1}{45} \cdot 356241$$
$$+ \frac{1}{45} \cdot 526341 + \frac{1}{45} \cdot 536142 + \frac{1}{45} \cdot 263415 + \frac{1}{90} \cdot 263451 + \frac{1}{90} \cdot 362451 - \frac{1}{90} \cdot 365421$$
$$- \frac{1}{90} \cdot 625431 + \frac{1}{90} \cdot 152463 + \frac{1}{90} \cdot 152643 + \frac{1}{90} \cdot 154263 + \frac{1}{90} \cdot 251463 + \frac{1}{90} \cdot 251643$$
$$+ \frac{1}{90} \cdot 413526 + \frac{1}{90} \cdot 413625 + \frac{1}{90} \cdot 415326 + \frac{1}{90} \cdot 431526 + \frac{1}{90} \cdot 431625 - \frac{1}{90} \cdot 451263$$
$$- \frac{1}{18} \cdot 452163 + \frac{1}{90} \cdot 516234 - \frac{1}{90} \cdot 526134 + \frac{1}{45} \cdot 514632 + \frac{1}{90} \cdot 524631 + \frac{1}{90} \cdot 526431$$
$$+ \frac{2}{45} \cdot 541632 + \frac{1}{90} \cdot 542631 + \frac{1}{45} \cdot 541362 + \frac{1}{90} \cdot 641352 + \frac{1}{90} \cdot 641532 + \frac{1}{90} \cdot 643152$$
$$- \frac{1}{45} \cdot 452136 - \frac{1}{45} \cdot 452316 - \frac{1}{90} \cdot 462135 - \frac{1}{90} \cdot 462153 - \frac{1}{90} \cdot 462315 - \frac{1}{45} \cdot 451326$$
$$- \frac{1}{90} \cdot 513246 - \frac{1}{90} \cdot 513264 - \frac{1}{90} \cdot 513426 - \frac{1}{90} \cdot 523146 - \frac{1}{90} \cdot 523164 - \frac{1}{18} \cdot 523416$$
$$+ \frac{1}{90} \cdot 543126 + \frac{2}{15} \cdot 543216 + \frac{1}{45} \cdot 543261 + \frac{1}{45} \cdot 643215 - \frac{1}{90} \cdot 243516 - \frac{1}{90} \cdot 243615$$
$$- \frac{1}{90} \cdot 253416 - \frac{1}{90} \cdot 423516 - \frac{1}{90} \cdot 423615 - \frac{1}{45} \cdot 435126 - \frac{1}{90} \cdot 435162 - \frac{1}{90} \cdot 436152$$
$$- \frac{1}{45} \cdot 534126 - \frac{1}{90} \cdot 534162 - \frac{1}{45} \cdot 354126 - \frac{1}{30} \cdot 541236 - \frac{1}{45} \cdot 541263 + \frac{1}{90} \cdot 453216$$
$$+ \frac{1}{90} \cdot 345261 + \frac{1}{90} \cdot 346251 + \frac{2}{45} \cdot 452361 + \frac{1}{45} \cdot 452631 + \frac{1}{45} \cdot 462351 + \frac{1}{45} \cdot 462513$$
$$+ \frac{1}{45} \cdot 462531 + \frac{1}{90} \cdot 451362 + \frac{1}{45} \cdot 513462 + \frac{1}{45} \cdot 513642 + \frac{1}{90} \cdot 523461 + \frac{1}{90} \cdot 523641$$

$$- \frac{1}{10} \cdot 543612 - \frac{1}{90} \cdot 543621 - \frac{1}{90} \cdot 643251 + \frac{1}{90} \cdot 153642 + \frac{1}{90} \cdot 154632 + \frac{1}{90} \cdot 413652$$
$$+ \frac{1}{90} \cdot 431652 + \frac{1}{45} \cdot 531642 + \frac{1}{90} \cdot 425316 + \frac{1}{90} \cdot 435216 + \frac{1}{90} \cdot 546123 + \frac{1}{90} \cdot 362541$$
$$+ \frac{1}{90} \cdot 426531 + \frac{1}{45} \cdot 642531 - \frac{1}{45} \cdot 156423 - \frac{1}{90} \cdot 254613 - \frac{1}{90} \cdot 256413 - \frac{1}{45} \cdot 453126$$
$$- \frac{1}{90} \cdot 461325 - \frac{1}{90} \cdot 463125 + \frac{1}{90} \cdot 456213 + \frac{2}{15} \cdot 561234 + \frac{1}{45} \cdot 562134 - \frac{1}{45} \cdot 546132$$
$$- \frac{1}{45} \cdot 546231 - \frac{1}{10} \cdot 561432 - \frac{1}{45} \cdot 562431 - \frac{1}{45} \cdot 564132 - \frac{1}{45} \cdot 564231 - \frac{1}{45} \cdot 546312$$
$$- \frac{1}{45} \cdot 643512 - \frac{1}{45} \cdot 645132 - \frac{1}{45} \cdot 645312 - \frac{1}{90} \cdot 516324 - \frac{1}{90} \cdot 516423 - \frac{1}{90} \cdot 354162$$
$$- \frac{1}{90} \cdot 453162 + \frac{1}{90} \cdot 456132 + \frac{1}{45} \cdot 561243 - \frac{1}{45} \cdot 465213 - \frac{1}{45} \cdot 465231 - \frac{1}{10} \cdot 563214$$
$$- \frac{1}{45} \cdot 563241 - \frac{1}{45} \cdot 564213 - \frac{1}{45} \cdot 465312 - \frac{1}{45} \cdot 635412 - \frac{1}{45} \cdot 645213 + \frac{1}{90} \cdot 245361$$
$$+ \frac{1}{90} \cdot 246351 + \frac{1}{90} \cdot 425361 + \frac{1}{90} \cdot 426351 + \frac{1}{90} \cdot 562341 + \frac{1}{45} \cdot 463512 + \frac{1}{15} \cdot 563412$$
$$+ \frac{1}{45} \cdot 536412 + \frac{1}{90} \cdot 564123 + \frac{1}{45} \cdot 564321 + \frac{1}{45} \cdot 645321 - \frac{1}{90} \cdot 163245 - \frac{1}{90} \cdot 164235$$
$$- \frac{1}{90} \cdot 521346 - \frac{1}{90} \cdot 521364 - \frac{1}{90} \cdot 531246 - \frac{1}{90} \cdot 531264 - \frac{1}{90} \cdot 541623 + \frac{1}{45} \cdot 561324$$
$$+ \frac{1}{15} \cdot 612345 + \frac{1}{90} \cdot 612354 + \frac{1}{90} \cdot 612435 - \frac{1}{90} \cdot 612453 - \frac{1}{90} \cdot 612534 - \frac{1}{90} \cdot 632415$$
$$- \frac{1}{90} \cdot 642135 - \frac{1}{90} \cdot 642315 - \frac{1}{45} \cdot 642351 - \frac{1}{45} \cdot 652134 - \frac{1}{45} \cdot 652314 - \frac{7}{90} \cdot 652341$$
$$- \frac{1}{45} \cdot 653124 - \frac{7}{90} \cdot 654123 - \frac{1}{90} \cdot 162354 - \frac{1}{90} \cdot 162534 - \frac{1}{90} \cdot 261354 - \frac{1}{90} \cdot 261534$$
$$- \frac{1}{90} \cdot 365124 - \frac{1}{90} \cdot 512436 - \frac{1}{90} \cdot 514236 + \frac{1}{90} \cdot 613245 + \frac{1}{90} \cdot 621345 - \frac{1}{90} \cdot 623145$$
$$- \frac{1}{90} \cdot 631245 - \frac{1}{90} \cdot 613542 - \frac{1}{90} \cdot 615243 - \frac{1}{90} \cdot 615342 - \frac{1}{45} \cdot 625341 - \frac{1}{45} \cdot 651243$$
$$- \frac{1}{45} \cdot 651342 - \frac{1}{45} \cdot 651423 + \frac{1}{45} \cdot 163254 + \frac{1}{90} \cdot 164253 + \frac{1}{90} \cdot 165243 + \frac{1}{45} \cdot 521436$$
$$+ \frac{1}{90} \cdot 521463 + \frac{1}{90} \cdot 521643 + \frac{1}{90} \cdot 531426 + \frac{1}{45} \cdot 531462 + \frac{1}{90} \cdot 541326 + \frac{1}{90} \cdot 632514$$
$$+ \frac{1}{90} \cdot 642153 + \frac{1}{45} \cdot 642513 + \frac{2}{45} \cdot 652143 + \frac{1}{45} \cdot 652413 + \frac{1}{45} \cdot 653142 + \frac{1}{90} \cdot 613452$$
$$+ \frac{1}{90} \cdot 631452 + \frac{1}{90} \cdot 514623 + \frac{2}{45} \cdot 614523 + \frac{1}{45} \cdot 624513 + \frac{1}{45} \cdot 641523 + \frac{1}{90} \cdot 615234$$
$$+ \frac{1}{90} \cdot 625134 - \frac{1}{90} \cdot 651432 + \frac{1}{90} \cdot 163524 + \frac{1}{90} \cdot 165324 + \frac{1}{90} \cdot 263154 + \frac{1}{45} \cdot 263514$$
$$+ \frac{1}{90} \cdot 362154 + \frac{1}{90} \cdot 524136 + \frac{1}{90} \cdot 542136 + \frac{1}{90} \cdot 625143 + \frac{1}{90} \cdot 631542 + \frac{1}{45} \cdot 635142$$
$$+ \frac{1}{90} \cdot 623415 + \frac{1}{90} \cdot 623514 + \frac{2}{45} \cdot 634125 + \frac{1}{45} \cdot 634152 + \frac{1}{45} \cdot 635124 + \frac{1}{90} \cdot 364125$$
$$+ \frac{1}{90} \cdot 641235 + \frac{1}{90} \cdot 641253 - \frac{1}{90} \cdot 653214 - \frac{1}{90} \cdot 163542 - \frac{1}{90} \cdot 164352 + \frac{1}{90} \cdot 164532$$
$$+ \frac{1}{90} \cdot 165342 + \frac{1}{90} \cdot 253461 + \frac{1}{90} \cdot 253641 + \frac{1}{90} \cdot 352461 + \frac{1}{90} \cdot 352641 + \frac{1}{90} \cdot 456231$$
$$- \frac{1}{90} \cdot 524316 - \frac{1}{90} \cdot 532416 + \frac{1}{90} \cdot 534216 + \frac{1}{90} \cdot 542316 + \frac{1}{90} \cdot 524613 + \frac{1}{90} \cdot 526314$$

$$
\begin{aligned}
&+\frac{1}{90}\cdot 526413+\frac{1}{45}\cdot 562413+\frac{1}{90}\cdot 364152+\frac{1}{90}\cdot 461352+\frac{1}{90}\cdot 463152+\frac{1}{45}\cdot 563142\\
&+\frac{1}{90}\cdot 613425+\frac{1}{90}\cdot 613524+\frac{1}{90}\cdot 631425+\frac{1}{90}\cdot 631524+\frac{1}{90}\cdot 645123+\frac{1}{45}\cdot 653421\\
&+\frac{1}{45}\cdot 654231+\frac{1}{90}\cdot 456312+\frac{1}{90}\cdot 614235+\frac{1}{90}\cdot 614253+\frac{1}{90}\cdot 624135+\frac{1}{90}\cdot 624153\\
&+\frac{1}{90}\cdot 634512+\frac{1}{45}\cdot 654312-\frac{1}{45}\cdot 563421-\frac{1}{90}\cdot 614352-\frac{1}{90}\cdot 614532-\frac{1}{90}\cdot 624315\\
&-\frac{1}{45}\cdot 624351-\frac{1}{90}\cdot 634215+\frac{1}{5}\cdot 654321-\frac{1}{90}\cdot 254631-\frac{1}{90}\cdot 256431-\frac{1}{90}\cdot 354261\\
&-\frac{1}{45}\cdot 354621-\frac{1}{90}\cdot 453261-\frac{1}{90}\cdot 536214-\frac{1}{90}\cdot 542613-\frac{1}{45}\cdot 546213-\frac{1}{45}\cdot 564312\\
&-\frac{1}{90}\cdot 365142-\frac{1}{90}\cdot 461532-\frac{1}{45}\cdot 465132-\frac{1}{90}\cdot 615324-\frac{1}{90}\cdot 615423-\frac{1}{90}\cdot 641325\\
&-\frac{1}{90}\cdot 643125-\frac{1}{45}\cdot 651324-\frac{1}{45}\cdot 645231-\frac{1}{90}\cdot 264351-\frac{1}{90}\cdot 265341-\frac{1}{90}\cdot 524361\\
&-\frac{1}{90}\cdot 542361-\frac{1}{45}\cdot 653412
\end{aligned}
$$

$$
\begin{aligned}
[\![y_1\times y_3]\!]=&\ \frac{1}{30}\cdot 123564+\frac{1}{45}\cdot 125364+\frac{1}{90}\cdot 132564+\frac{1}{90}\cdot 135264-\frac{1}{30}\cdot 152364+\frac{1}{90}\cdot 213564\\
&+\frac{1}{45}\cdot 215364-\frac{1}{45}\cdot 231564+\frac{1}{45}\cdot 251364-\frac{1}{45}\cdot 312564+\frac{7}{90}\cdot 351264+\frac{1}{30}\cdot 123645\\
&+\frac{1}{45}\cdot 124635+\frac{1}{90}\cdot 132645-\frac{1}{30}\cdot 134625+\frac{1}{90}\cdot 142635+\frac{1}{90}\cdot 213645+\frac{1}{45}\cdot 214635\\
&-\frac{1}{45}\cdot 231645-\frac{1}{45}\cdot 312645+\frac{1}{45}\cdot 314625+\frac{7}{90}\cdot 341625+\frac{1}{10}\cdot 123654+\frac{1}{30}\cdot 132654\\
&-\frac{1}{90}\cdot 142653+\frac{1}{30}\cdot 213654-\frac{1}{15}\cdot 231654-\frac{1}{15}\cdot 312654+\frac{1}{18}\cdot 314652+\frac{11}{90}\cdot 341652\\
&-\frac{1}{90}\cdot 136254+\frac{1}{18}\cdot 261354+\frac{11}{90}\cdot 361254+\frac{1}{30}\cdot 124536+\frac{1}{45}\cdot 142536-\frac{1}{30}\cdot 412536\\
&-\frac{2}{45}\cdot 412635-\frac{1}{18}\cdot 143625+\frac{1}{90}\cdot 234615+\frac{1}{90}\cdot 243615+\frac{1}{30}\cdot 324615-\frac{1}{90}\cdot 413625\\
&+\frac{1}{45}\cdot 423615-\frac{1}{9}\cdot 143652-\frac{1}{45}\cdot 243651+\frac{2}{45}\cdot 342651-\frac{2}{45}\cdot 412653-\frac{1}{90}\cdot 413652\\
&+\frac{1}{15}\cdot 423651+\frac{1}{30}\cdot 125346+\frac{1}{45}\cdot 135246-\frac{1}{30}\cdot 235146-\frac{2}{45}\cdot 235164-\frac{1}{18}\cdot 153264\\
&-\frac{1}{90}\cdot 253164+\frac{1}{90}\cdot 512364+\frac{1}{90}\cdot 513264+\frac{1}{30}\cdot 521364+\frac{1}{45}\cdot 523164+\frac{1}{10}\cdot 125436\\
&+\frac{1}{45}\cdot 125463-\frac{1}{45}\cdot 235461-\frac{1}{30}\cdot 512463-\frac{2}{45}\cdot 125634-\frac{1}{45}\cdot 135624-\frac{1}{90}\cdot 235614\\
&-\frac{1}{45}\cdot 152634-\frac{1}{90}\cdot 512634+\frac{1}{90}\cdot 153624+\frac{1}{90}\cdot 253614+\frac{1}{90}\cdot 513624-\frac{1}{9}\cdot 523614\\
&-\frac{4}{45}\cdot 125643+\frac{1}{90}\cdot 135642+\frac{1}{45}\cdot 235641-\frac{2}{45}\cdot 152643+\frac{1}{90}\cdot 512643-\frac{2}{45}\cdot 236154\\
&-\frac{1}{9}\cdot 163254-\frac{1}{90}\cdot 263154-\frac{1}{45}\cdot 613254+\frac{1}{15}\cdot 623154+\frac{2}{45}\cdot 631254+\frac{1}{45}\cdot 126435\\
&-\frac{1}{30}\cdot 236415-\frac{1}{45}\cdot 612435-\frac{1}{15}\cdot 126453+\frac{1}{90}\cdot 136452+\frac{1}{90}\cdot 162453-\frac{4}{45}\cdot 126534\\
&-\frac{2}{45}\cdot 136524+\frac{1}{90}\cdot 236514+\frac{1}{90}\cdot 162534+\frac{1}{45}\cdot 612534+\frac{1}{90}\cdot 214536+\frac{1}{90}\cdot 241536
\end{aligned}
$$

$$+ \frac{1}{90} \cdot 215346 + \frac{1}{90} \cdot 315246 + \frac{1}{30} \cdot 215436 + \frac{1}{45} \cdot 215463 - \frac{1}{90} \cdot 315426 + \frac{1}{18} \cdot 315462$$
$$+ \frac{1}{45} \cdot 216435 - \frac{1}{90} \cdot 251436 + \frac{1}{18} \cdot 261435 + \frac{1}{30} \cdot 134256 + \frac{1}{90} \cdot 134265 + \frac{1}{45} \cdot 314256$$
$$+ \frac{1}{45} \cdot 314265 - \frac{1}{18} \cdot 325146 - \frac{1}{9} \cdot 325416 - \frac{1}{45} \cdot 325461 + \frac{1}{30} \cdot 142356 + \frac{1}{90} \cdot 142365$$
$$+ \frac{1}{45} \cdot 241356 + \frac{1}{45} \cdot 241365 - \frac{1}{18} \cdot 421536 + \frac{1}{10} \cdot 143256 + \frac{1}{30} \cdot 143265 + \frac{1}{45} \cdot 143526$$
$$+ \frac{1}{45} \cdot 153246 + \frac{1}{45} \cdot 143562 - \frac{1}{45} \cdot 243561 - \frac{2}{45} \cdot 145236 - \frac{1}{45} \cdot 145263 - \frac{1}{45} \cdot 146235$$
$$+ \frac{1}{90} \cdot 146253 - \frac{1}{45} \cdot 245136 - \frac{1}{45} \cdot 415236 + \frac{1}{90} \cdot 425136 - \frac{4}{45} \cdot 145326 - \frac{1}{30} \cdot 145362$$
$$- \frac{2}{45} \cdot 146325 - \frac{1}{45} \cdot 146352 + \frac{1}{90} \cdot 245316 + \frac{1}{45} \cdot 245361 + \frac{1}{45} \cdot 246315 - \frac{2}{45} \cdot 415326$$
$$- \frac{1}{9} \cdot 521436 - \frac{1}{45} \cdot 621435 + \frac{1}{45} \cdot 163245 - \frac{1}{45} \cdot 613245 - \frac{1}{15} \cdot 153426 - \frac{1}{90} \cdot 153462$$
$$- \frac{1}{45} \cdot 153642 + \frac{1}{90} \cdot 253416 + \frac{1}{45} \cdot 253461 - \frac{1}{90} \cdot 163425 - \frac{1}{45} \cdot 163524 + \frac{1}{90} \cdot 513426$$
$$+ \frac{1}{45} \cdot 613425 - \frac{4}{45} \cdot 154236 - \frac{2}{45} \cdot 254136 - \frac{2}{45} \cdot 154263 - \frac{1}{30} \cdot 164235 - \frac{1}{45} \cdot 164253$$
$$+ \frac{1}{90} \cdot 514236 + \frac{1}{45} \cdot 514263 + \frac{1}{45} \cdot 614235 - \frac{2}{45} \cdot 215643 - \frac{1}{45} \cdot 216453 - \frac{8}{45} \cdot 126543$$
$$- \frac{2}{45} \cdot 216534 - \frac{8}{45} \cdot 216543 + \frac{1}{45} \cdot 415362 - \frac{1}{9} \cdot 416325 - \frac{1}{30} \cdot 416352 - \frac{1}{15} \cdot 326154$$
$$+ \frac{1}{30} \cdot 416253 + \frac{7}{90} \cdot 146523 + \frac{1}{90} \cdot 146532 + \frac{1}{9} \cdot 236541 + \frac{1}{18} \cdot 326514 + \frac{1}{9} \cdot 326541$$
$$+ \frac{7}{45} \cdot 416523 + \frac{1}{9} \cdot 416532 - \frac{1}{18} \cdot 251463 - \frac{1}{30} \cdot 251643 + \frac{1}{18} \cdot 521643 - \frac{8}{45} \cdot 154326$$
$$- \frac{1}{9} \cdot 254163 - \frac{1}{15} \cdot 514362 + \frac{1}{10} \cdot 154623 + \frac{1}{30} \cdot 154632 + \frac{1}{9} \cdot 254361 - \frac{7}{90} \cdot 514632$$
$$+ \frac{1}{10} \cdot 156324 + \frac{1}{9} \cdot 156342 + \frac{7}{90} \cdot 156243 + \frac{7}{45} \cdot 256143 + \frac{2}{45} \cdot 516342 + \frac{1}{15} \cdot 526143$$
$$+ \frac{4}{45} \cdot 156423 + \frac{2}{45} \cdot 516432 - \frac{1}{30} \cdot 162543 - \frac{1}{90} \cdot 163542 - \frac{1}{45} \cdot 261543 + \frac{1}{9} \cdot 612543$$
$$+ \frac{1}{9} \cdot 621543 - \frac{1}{18} \cdot 164325 - \frac{1}{30} \cdot 264153 + \frac{1}{30} \cdot 164352 + \frac{1}{9} \cdot 614325 + \frac{1}{9} \cdot 164523$$
$$+ \frac{1}{45} \cdot 164532 + \frac{2}{45} \cdot 264351 + \frac{1}{90} \cdot 165243 + \frac{1}{45} \cdot 165342 + \frac{1}{9} \cdot 265143 - \frac{1}{18} \cdot 316425$$
$$- \frac{1}{30} \cdot 316524 - \frac{1}{30} \cdot 136542 - \frac{1}{45} \cdot 316542 + \frac{1}{45} \cdot 264135 + \frac{1}{30} \cdot 246153 - \frac{1}{15} \cdot 421653$$
$$- \frac{1}{15} \cdot 264315 - \frac{1}{18} \cdot 154362 + \frac{2}{45} \cdot 264513 + \frac{1}{15} \cdot 426513 - \frac{7}{90} \cdot 265314 + \frac{1}{30} \cdot 165324$$
$$+ \frac{2}{45} \cdot 614352 + \frac{2}{45} \cdot 265413 + \frac{1}{30} \cdot 231456 + \frac{1}{90} \cdot 231465 + \frac{1}{90} \cdot 231546 + \frac{1}{30} \cdot 312456$$
$$+ \frac{1}{90} \cdot 312465 + \frac{1}{90} \cdot 312546 + \frac{1}{10} \cdot 321456 + \frac{1}{30} \cdot 321465 + \frac{1}{30} \cdot 321546 - \frac{1}{15} \cdot 321564$$
$$- \frac{1}{15} \cdot 321645 + \frac{1}{45} \cdot 324156 + \frac{1}{45} \cdot 324165 + \frac{1}{45} \cdot 324516 - \frac{2}{45} \cdot 325164 + \frac{11}{90} \cdot 325614$$
$$+ \frac{1}{45} \cdot 421356 + \frac{1}{45} \cdot 421365 - \frac{2}{45} \cdot 421635 + \frac{1}{45} \cdot 521346 + \frac{11}{90} \cdot 521634 + \frac{1}{15} \cdot 325641$$
$$- \frac{1}{15} \cdot 326145 - \frac{1}{18} \cdot 326415 + \frac{2}{45} \cdot 326451 + \frac{1}{90} \cdot 426135 + \frac{2}{45} \cdot 526134 - \frac{2}{45} \cdot 341256$$

$$-\frac{1}{45}\cdot 341526-\frac{1}{30}\cdot 341562-\frac{1}{45}\cdot 351246+\frac{1}{90}\cdot 351426-\frac{1}{30}\cdot 351462-\frac{1}{30}\cdot 361245$$
$$-\frac{1}{30}\cdot 361425-\frac{1}{9}\cdot 361452-\frac{4}{45}\cdot 342156-\frac{1}{30}\cdot 342516-\frac{2}{45}\cdot 352146-\frac{1}{45}\cdot 352416$$
$$-\frac{1}{30}\cdot 362145+\frac{1}{90}\cdot 362415+\frac{1}{45}\cdot 362451-\frac{1}{15}\cdot 421563+\frac{1}{90}\cdot 425163+\frac{2}{45}\cdot 425613$$
$$-\frac{1}{18}\cdot 521463+\frac{2}{45}\cdot 621453+\frac{1}{15}\cdot 621534-\frac{1}{15}\cdot 423156-\frac{1}{90}\cdot 423516+\frac{1}{45}\cdot 423561$$
$$-\frac{1}{45}\cdot 425316-\frac{1}{45}\cdot 425631-\frac{1}{90}\cdot 523146-\frac{1}{45}\cdot 524136+\frac{1}{45}\cdot 623145-\frac{1}{45}\cdot 625134$$
$$-\frac{4}{45}\cdot 431256-\frac{2}{45}\cdot 431526-\frac{1}{30}\cdot 431562-\frac{1}{30}\cdot 531246-\frac{1}{45}\cdot 531426+\frac{1}{90}\cdot 531462$$
$$+\frac{1}{45}\cdot 631452-\frac{1}{5}\cdot 321654-\frac{1}{45}\cdot 426153+\frac{2}{45}\cdot 341265+\frac{1}{45}\cdot 351624-\frac{2}{45}\cdot 342165$$
$$+\frac{1}{90}\cdot 352164+\frac{1}{15}\cdot 352614+\frac{1}{15}\cdot 352641+\frac{1}{30}\cdot 362154+\frac{1}{45}\cdot 362514+\frac{4}{45}\cdot 362541$$
$$-\frac{1}{45}\cdot 423165+\frac{1}{90}\cdot 426315+\frac{1}{15}\cdot 426351+\frac{2}{45}\cdot 426531+\frac{1}{90}\cdot 524163+\frac{1}{15}\cdot 624153$$
$$+\frac{2}{45}\cdot 625143-\frac{2}{45}\cdot 431265+\frac{1}{90}\cdot 431625+\frac{1}{30}\cdot 431652+\frac{1}{15}\cdot 531624+\frac{1}{45}\cdot 531642$$
$$+\frac{1}{15}\cdot 631524+\frac{4}{45}\cdot 631542-\frac{1}{45}\cdot 432615+\frac{1}{9}\cdot 432651-\frac{1}{45}\cdot 532164+\frac{2}{45}\cdot 215634$$
$$+\frac{1}{90}\cdot 315624+\frac{1}{90}\cdot 251634-\frac{2}{45}\cdot 532614+\frac{1}{9}\cdot 632154+\frac{2}{45}\cdot 134562+\frac{1}{90}\cdot 142563$$
$$+\frac{1}{18}\cdot 145623+\frac{7}{90}\cdot 145632+\frac{7}{90}\cdot 163452+\frac{2}{45}\cdot 234516-\frac{1}{45}\cdot 245613-\frac{1}{45}\cdot 245163$$
$$-\frac{1}{45}\cdot 245631+\frac{1}{90}\cdot 314526+\frac{1}{18}\cdot 345126+\frac{4}{45}\cdot 346125+\frac{1}{45}\cdot 356124+\frac{1}{30}\cdot 314562$$
$$-\frac{1}{45}\cdot 345162+\frac{2}{45}\cdot 346152+\frac{1}{90}\cdot 356142+\frac{7}{90}\cdot 345216+\frac{1}{15}\cdot 346215+\frac{7}{90}\cdot 523416$$
$$-\frac{1}{45}\cdot 346251-\frac{1}{18}\cdot 356241-\frac{1}{45}\cdot 523461-\frac{1}{15}\cdot 523641-\frac{1}{90}\cdot 526341-\frac{8}{45}\cdot 345612$$
$$-\frac{2}{45}\cdot 346512-\frac{1}{15}\cdot 354612-\frac{1}{90}\cdot 356412-\frac{1}{30}\cdot 364512-\frac{1}{45}\cdot 354162-\frac{1}{18}\cdot 364152$$
$$-\frac{4}{45}\cdot 345621-\frac{2}{45}\cdot 346521-\frac{1}{15}\cdot 354621-\frac{1}{30}\cdot 356421-\frac{1}{18}\cdot 364521+\frac{1}{90}\cdot 413562$$
$$+\frac{1}{15}\cdot 415632+\frac{1}{30}\cdot 451362+\frac{1}{45}\cdot 451632-\frac{1}{9}\cdot 456132-\frac{2}{45}\cdot 513462-\frac{1}{9}\cdot 456213$$
$$-\frac{1}{90}\cdot 524613-\frac{1}{45}\cdot 623415-\frac{1}{15}\cdot 623514-\frac{1}{90}\cdot 624513-\frac{4}{45}\cdot 456231-\frac{1}{45}\cdot 524361$$
$$-\frac{1}{90}\cdot 524631-\frac{4}{45}\cdot 623451-\frac{1}{15}\cdot 623541-\frac{1}{15}\cdot 624351-\frac{1}{90}\cdot 624531-\frac{1}{90}\cdot 625341$$
$$-\frac{2}{45}\cdot 435612+\frac{1}{15}\cdot 453162-\frac{1}{30}\cdot 453612-\frac{4}{45}\cdot 456312-\frac{1}{90}\cdot 534612-\frac{4}{45}\cdot 634512$$
$$+\frac{1}{15}\cdot 415623+\frac{1}{45}\cdot 451623+\frac{1}{90}\cdot 452613-\frac{1}{90}\cdot 452631+\frac{4}{45}\cdot 534162-\frac{2}{45}\cdot 435621$$
$$-\frac{1}{18}\cdot 453621-\frac{1}{30}\cdot 534621-\frac{1}{18}\cdot 634152-\frac{2}{45}\cdot 263415+\frac{1}{90}\cdot 263514-\frac{1}{45}\cdot 416235$$
$$-\frac{2}{45}\cdot 236145+\frac{1}{15}\cdot 256134+\frac{7}{45}\cdot 436125+\frac{2}{45}\cdot 436152-\frac{1}{90}\cdot 256314+\frac{2}{45}\cdot 256413$$
$$+\frac{4}{45}\cdot 436215-\frac{1}{90}\cdot 526314+\frac{1}{18}\cdot 526413-\frac{1}{45}\cdot 461325-\frac{1}{15}\cdot 462513+\frac{4}{45}\cdot 462315$$

$$+\frac{1}{30}\cdot 364125+\frac{1}{45}\cdot 365124+\frac{1}{15}\cdot 463125+\frac{1}{15}\cdot 265134+\frac{7}{90}\cdot 354126+\frac{1}{30}\cdot 365142$$
$$+\frac{1}{90}\cdot 354216-\frac{1}{30}\cdot 364215-\frac{2}{15}\cdot 365214-\frac{1}{90}\cdot 524316+\frac{1}{45}\cdot 354261-\frac{1}{90}\cdot 364251$$
$$-\frac{1}{30}\cdot 365241+\frac{1}{90}\cdot 526431+\frac{17}{90}\cdot 365412+\frac{1}{30}\cdot 365421-\frac{1}{18}\cdot 461352+\frac{1}{30}\cdot 461532$$
$$-\frac{1}{15}\cdot 465132+\frac{1}{90}\cdot 513642+\frac{1}{45}\cdot 613542-\frac{1}{15}\cdot 465213-\frac{1}{45}\cdot 624315-\frac{1}{90}\cdot 625314$$
$$+\frac{1}{90}\cdot 625413+\frac{2}{45}\cdot 465231+\frac{1}{18}\cdot 625431+\frac{1}{18}\cdot 463152-\frac{2}{45}\cdot 463512+\frac{2}{45}\cdot 465312$$
$$-\frac{2}{45}\cdot 536412+\frac{1}{45}\cdot 635412+\frac{2}{45}\cdot 436251-\frac{4}{45}\cdot 436521-\frac{1}{15}\cdot 256341-\frac{1}{15}\cdot 536142$$
$$+\frac{1}{45}\cdot 536241-\frac{2}{45}\cdot 256431+\frac{1}{45}\cdot 263541-\frac{4}{45}\cdot 632541-\frac{1}{15}\cdot 265341-\frac{2}{45}\cdot 412563$$
$$+\frac{4}{45}\cdot 451263+\frac{7}{45}\cdot 452163+\frac{2}{45}\cdot 461253+\frac{2}{45}\cdot 462153-\frac{1}{90}\cdot 514623+\frac{2}{45}\cdot 516423$$
$$+\frac{1}{15}\cdot 541263+\frac{4}{45}\cdot 542163-\frac{1}{18}\cdot 641523-\frac{8}{45}\cdot 432156-\frac{8}{45}\cdot 432165+\frac{1}{9}\cdot 432561$$
$$+\frac{1}{10}\cdot 435126+\frac{1}{30}\cdot 435216+\frac{1}{30}\cdot 536214+\frac{1}{10}\cdot 452136+\frac{1}{9}\cdot 452316+\frac{7}{90}\cdot 451326$$
$$+\frac{4}{45}\cdot 453126+\frac{1}{15}\cdot 463215-\frac{1}{30}\cdot 514326-\frac{1}{18}\cdot 532146+\frac{1}{30}\cdot 532416+\frac{1}{9}\cdot 632145$$
$$+\frac{1}{45}\cdot 532461+\frac{1}{9}\cdot 534126+\frac{1}{45}\cdot 534216+\frac{1}{90}\cdot 541326+\frac{1}{45}\cdot 542316+\frac{2}{45}\cdot 642135$$
$$+\frac{2}{45}\cdot 642153-\frac{1}{30}\cdot 254316-\frac{1}{18}\cdot 432516+\frac{2}{45}\cdot 435261+\frac{1}{30}\cdot 542613+\frac{1}{30}\cdot 542136$$
$$+\frac{1}{45}\cdot 632415+\frac{1}{15}\cdot 543162-\frac{1}{15}\cdot 452361-\frac{1}{18}\cdot 462351+\frac{1}{45}\cdot 462531-\frac{2}{45}\cdot 463521$$
$$-\frac{1}{15}\cdot 453261+\frac{1}{90}\cdot 536124-\frac{1}{45}\cdot 632451-\frac{2}{45}\cdot 536421-\frac{7}{90}\cdot 634251-\frac{2}{45}\cdot 635241$$
$$-\frac{1}{30}\cdot 541362-\frac{2}{45}\cdot 542361-\frac{7}{90}\cdot 642351-\frac{2}{45}\cdot 642531-\frac{2}{15}\cdot 541632+\frac{1}{90}\cdot 542631$$
$$+\frac{17}{90}\cdot 543612+\frac{1}{30}\cdot 543621-\frac{1}{15}\cdot 546132-\frac{1}{90}\cdot 641352-\frac{1}{30}\cdot 643152-\frac{1}{15}\cdot 546213$$
$$+\frac{2}{45}\cdot 546231+\frac{2}{45}\cdot 546312+\frac{1}{45}\cdot 642513+\frac{1}{15}\cdot 643512+\frac{1}{18}\cdot 156234+\frac{1}{18}\cdot 451236$$
$$-\frac{1}{45}\cdot 461235-\frac{1}{5}\cdot 456123-\frac{1}{9}\cdot 465123-\frac{2}{45}\cdot 561243-\frac{1}{15}\cdot 614523-\frac{1}{15}\cdot 561324$$
$$-\frac{1}{90}\cdot 562314-\frac{1}{15}\cdot 634125-\frac{1}{90}\cdot 635124-\frac{1}{30}\cdot 561342-\frac{4}{45}\cdot 562341-\frac{1}{9}\cdot 546123$$
$$-\frac{4}{45}\cdot 564123+\frac{2}{45}\cdot 564213-\frac{4}{45}\cdot 645123-\frac{1}{45}\cdot 516234+\frac{1}{90}\cdot 461523-\frac{1}{90}\cdot 561423$$
$$-\frac{2}{45}\cdot 562134+\frac{1}{45}\cdot 562431-\frac{1}{30}\cdot 563124+\frac{2}{45}\cdot 645132+\frac{17}{90}\cdot 561432-\frac{2}{45}\cdot 562413$$
$$-\frac{2}{45}\cdot 563142+\frac{17}{90}\cdot 563214-\frac{1}{30}\cdot 463251+\frac{1}{15}\cdot 563241-\frac{2}{45}\cdot 534261-\frac{2}{15}\cdot 563412$$
$$+\frac{2}{45}\cdot 563421+\frac{2}{45}\cdot 564132-\frac{1}{15}\cdot 614532-\frac{1}{30}\cdot 641532-\frac{2}{45}\cdot 634215+\frac{1}{90}\cdot 635214$$
$$+\frac{2}{45}\cdot 645213+\frac{2}{45}\cdot 564231+\frac{2}{45}\cdot 645231+\frac{2}{45}\cdot 564312+\frac{2}{45}\cdot 645312+\frac{1}{90}\cdot 136245$$
$$+\frac{2}{45}\cdot 162345+\frac{7}{90}\cdot 165234+\frac{1}{90}\cdot 251346+\frac{1}{30}\cdot 261345+\frac{1}{90}\cdot 263145+\frac{2}{45}\cdot 512346$$

$$
\begin{aligned}
&+\frac{7}{90}\cdot 541236-\frac{8}{45}\cdot 561234-\frac{1}{45}\cdot 615234-\frac{1}{45}\cdot 641253-\frac{4}{45}\cdot 651234-\frac{2}{45}\cdot 651243\\
&-\frac{1}{15}\cdot 651324-\frac{1}{18}\cdot 651342-\frac{1}{30}\cdot 651423-\frac{2}{45}\cdot 652134-\frac{1}{30}\cdot 652314-\frac{1}{18}\cdot 653124\\
&+\frac{1}{45}\cdot 641325+\frac{1}{30}\cdot 651432-\frac{4}{45}\cdot 652143-\frac{2}{45}\cdot 615423+\frac{1}{30}\cdot 653214+\frac{1}{45}\cdot 635142\\
&-\frac{2}{45}\cdot 652413-\frac{1}{15}\cdot 643125-\frac{2}{45}\cdot 653142-\frac{2}{45}\cdot 264531-\frac{2}{45}\cdot 615342-\frac{2}{45}\cdot 642315\\
&+\frac{2}{45}\cdot 653412-\frac{2}{9}\cdot 165432-\frac{4}{45}\cdot 265431+\frac{2}{45}\cdot 465321-\frac{2}{9}\cdot 543216-\frac{4}{45}\cdot 543261\\
&+\frac{2}{45}\cdot 546321+\frac{4}{45}\cdot 564321-\frac{4}{45}\cdot 615432+\frac{1}{45}\cdot 635421-\frac{4}{45}\cdot 643215+\frac{1}{90}\cdot 643251\\
&+\frac{1}{15}\cdot 643521+\frac{4}{45}\cdot 645321+\frac{1}{45}\cdot 652431+\frac{4}{45}\cdot 653421+\frac{1}{15}\cdot 653241+\frac{2}{45}\cdot 654132\\
&+\frac{2}{45}\cdot 654213+\frac{4}{45}\cdot 654231+\frac{4}{45}\cdot 654312
\end{aligned}
$$

$$
\begin{aligned}
[\![y_1\times y_4]\!] = &\frac{1}{15}\cdot 123564+\frac{1}{45}\cdot 132564+\frac{1}{45}\cdot 213564-\frac{2}{45}\cdot 231564-\frac{1}{45}\cdot 312564+\frac{1}{45}\cdot 125364\\
&+\frac{1}{45}\cdot 215364+\frac{2}{45}\cdot 251364+\frac{7}{90}\cdot 351264+\frac{1}{10}\cdot 123654-\frac{1}{90}\cdot 124653+\frac{1}{30}\cdot 132654\\
&+\frac{1}{90}\cdot 134652-\frac{1}{30}\cdot 142653+\frac{1}{30}\cdot 213654+\frac{1}{90}\cdot 214653-\frac{1}{10}\cdot 231654-\frac{1}{30}\cdot 241653\\
&-\frac{1}{30}\cdot 312654+\frac{1}{18}\cdot 314652+\frac{11}{90}\cdot 341652+\frac{1}{30}\cdot 126354-\frac{1}{30}\cdot 136254+\frac{1}{90}\cdot 162354\\
&+\frac{1}{90}\cdot 216354+\frac{1}{30}\cdot 261354-\frac{1}{90}\cdot 316254+\frac{11}{90}\cdot 361254+\frac{1}{15}\cdot 124536+\frac{1}{45}\cdot 142536\\
&+\frac{1}{45}\cdot 124635+\frac{1}{45}\cdot 142635-\frac{1}{9}\cdot 143652-\frac{1}{30}\cdot 234651-\frac{1}{45}\cdot 243651-\frac{1}{45}\cdot 324651\\
&+\frac{1}{18}\cdot 342651-\frac{1}{18}\cdot 412653-\frac{2}{45}\cdot 413652+\frac{1}{30}\cdot 423651-\frac{2}{45}\cdot 235164-\frac{1}{30}\cdot 153264\\
&-\frac{1}{45}\cdot 253164+\frac{1}{90}\cdot 513264+\frac{1}{30}\cdot 521364+\frac{1}{90}\cdot 523164+\frac{1}{90}\cdot 531264+\frac{1}{10}\cdot 125436\\
&-\frac{1}{90}\cdot 135426+\frac{1}{90}\cdot 235416+\frac{1}{30}\cdot 152436+\frac{1}{90}\cdot 512436-\frac{1}{90}\cdot 125463+\frac{1}{90}\cdot 135462\\
&-\frac{1}{30}\cdot 235461-\frac{2}{45}\cdot 125634-\frac{1}{30}\cdot 135624-\frac{1}{45}\cdot 235614-\frac{1}{90}\cdot 152634-\frac{1}{45}\cdot 512634\\
&+\frac{1}{90}\cdot 153624-\frac{1}{90}\cdot 253614-\frac{1}{90}\cdot 513624-\frac{1}{9}\cdot 523614+\frac{1}{90}\cdot 146253-\frac{1}{18}\cdot 236154\\
&+\frac{2}{45}\cdot 246153+\frac{1}{15}\cdot 346152-\frac{1}{9}\cdot 163254-\frac{1}{45}\cdot 263154+\frac{1}{30}\cdot 612354-\frac{1}{45}\cdot 613254\\
&+\frac{1}{45}\cdot 621354+\frac{7}{90}\cdot 623154+\frac{1}{18}\cdot 631254+\frac{1}{30}\cdot 126435-\frac{1}{90}\cdot 236415-\frac{1}{90}\cdot 162435\\
&-\frac{1}{90}\cdot 612435-\frac{1}{15}\cdot 126453-\frac{1}{90}\cdot 136452-\frac{1}{45}\cdot 236451-\frac{1}{90}\cdot 146352+\frac{1}{90}\cdot 246351\\
&-\frac{1}{30}\cdot 346251-\frac{4}{45}\cdot 126534-\frac{1}{18}\cdot 136524-\frac{2}{45}\cdot 236514-\frac{1}{30}\cdot 162534-\frac{1}{45}\cdot 612534\\
&-\frac{1}{30}\cdot 163524-\frac{1}{90}\cdot 613524-\frac{1}{30}\cdot 623514+\frac{1}{45}\cdot 214536+\frac{1}{45}\cdot 214635+\frac{1}{30}\cdot 215436\\
&+\frac{1}{90}\cdot 215463-\frac{1}{30}\cdot 315426+\frac{1}{18}\cdot 315462+\frac{1}{90}\cdot 216435-\frac{1}{30}\cdot 251436+\frac{1}{90}\cdot 261435
\end{aligned}
$$

$$
\begin{aligned}
&+ \frac{1}{15} \cdot 134256 + \frac{1}{45} \cdot 134265 + \frac{1}{45} \cdot 135246 + \frac{1}{45} \cdot 314256 + \frac{1}{45} \cdot 314265 + \frac{1}{45} \cdot 315246 \\
&- \frac{1}{9} \cdot 325416 - \frac{1}{45} \cdot 325461 - \frac{1}{30} \cdot 421536 + \frac{1}{10} \cdot 143256 + \frac{1}{30} \cdot 143265 - \frac{1}{90} \cdot 143526 \\
&- \frac{1}{30} \cdot 143625 - \frac{1}{90} \cdot 243156 + \frac{1}{90} \cdot 243165 + \frac{1}{90} \cdot 243516 + \frac{1}{18} \cdot 243615 + \frac{1}{30} \cdot 153246 \\
&+ \frac{1}{30} \cdot 413256 + \frac{1}{90} \cdot 413265 - \frac{1}{90} \cdot 513246 + \frac{1}{90} \cdot 143562 - \frac{1}{30} \cdot 243561 - \frac{2}{45} \cdot 145236 \\
&- \frac{1}{30} \cdot 145263 - \frac{1}{90} \cdot 146235 - \frac{1}{30} \cdot 245136 - \frac{1}{90} \cdot 415236 + \frac{1}{90} \cdot 425136 - \frac{1}{45} \cdot 251463 \\
&+ \frac{1}{90} \cdot 351426 - \frac{1}{90} \cdot 351462 - \frac{1}{9} \cdot 521436 - \frac{1}{45} \cdot 621435 + \frac{1}{90} \cdot 163245 - \frac{1}{90} \cdot 613245 \\
&- \frac{1}{15} \cdot 153426 - \frac{1}{90} \cdot 153462 - \frac{1}{90} \cdot 153642 - \frac{1}{90} \cdot 253416 - \frac{1}{45} \cdot 253461 + \frac{1}{90} \cdot 253641 \\
&- \frac{1}{90} \cdot 352416 + \frac{1}{90} \cdot 352461 - \frac{4}{45} \cdot 154236 - \frac{1}{18} \cdot 154263 - \frac{1}{18} \cdot 254136 - \frac{1}{30} \cdot 164235 \\
&- \frac{1}{30} \cdot 164253 - \frac{1}{30} \cdot 514236 + \frac{1}{90} \cdot 514263 - \frac{1}{90} \cdot 614253 + \frac{1}{90} \cdot 264135 - \frac{1}{30} \cdot 524136 \\
&- \frac{1}{90} \cdot 624135 - \frac{4}{45} \cdot 125643 - \frac{4}{45} \cdot 215643 + \frac{1}{90} \cdot 351642 - \frac{8}{45} \cdot 126543 - \frac{8}{45} \cdot 216543 \\
&- \frac{1}{45} \cdot 361542 - \frac{4}{45} \cdot 145326 + \frac{1}{30} \cdot 415362 - \frac{1}{30} \cdot 146325 - \frac{1}{9} \cdot 416325 - \frac{1}{90} \cdot 416352 \\
&+ \frac{1}{9} \cdot 146523 + \frac{1}{90} \cdot 146532 + \frac{1}{9} \cdot 236541 + \frac{7}{90} \cdot 326514 + \frac{13}{90} \cdot 326541 + \frac{7}{45} \cdot 416523 \\
&+ \frac{7}{90} \cdot 416532 - \frac{1}{30} \cdot 152643 - \frac{1}{30} \cdot 251643 + \frac{1}{45} \cdot 512643 + \frac{1}{90} \cdot 521643 - \frac{8}{45} \cdot 154326 \\
&- \frac{1}{9} \cdot 254163 - \frac{1}{15} \cdot 514362 + \frac{1}{9} \cdot 154623 + \frac{1}{90} \cdot 154632 + \frac{1}{9} \cdot 254361 + \frac{1}{15} \cdot 156324 \\
&+ \frac{1}{9} \cdot 156342 + \frac{1}{15} \cdot 156243 + \frac{7}{45} \cdot 256143 - \frac{1}{90} \cdot 516324 + \frac{4}{45} \cdot 516342 + \frac{1}{90} \cdot 516243 \\
&+ \frac{2}{45} \cdot 526143 - \frac{1}{30} \cdot 162543 + \frac{1}{90} \cdot 261534 - \frac{1}{30} \cdot 261543 + \frac{1}{90} \cdot 163542 + \frac{1}{9} \cdot 612543 \\
&+ \frac{7}{90} \cdot 621543 - \frac{1}{30} \cdot 164325 - \frac{1}{90} \cdot 264153 + \frac{1}{90} \cdot 164352 + \frac{1}{9} \cdot 614325 + \frac{1}{9} \cdot 164523 \\
&+ \frac{1}{90} \cdot 164532 + \frac{2}{45} \cdot 264351 + \frac{2}{45} \cdot 263541 + \frac{1}{45} \cdot 362514 + \frac{1}{30} \cdot 362541 + \frac{1}{30} \cdot 165324 \\
&+ \frac{1}{30} \cdot 165342 + \frac{1}{30} \cdot 165243 + \frac{11}{90} \cdot 265143 + \frac{1}{45} \cdot 615324 + \frac{2}{45} \cdot 615243 + \frac{1}{18} \cdot 625143 \\
&- \frac{1}{45} \cdot 216453 - \frac{2}{45} \cdot 316425 + \frac{1}{90} \cdot 316524 - \frac{1}{15} \cdot 421653 - \frac{1}{15} \cdot 264315 - \frac{1}{90} \cdot 254613 \\
&+ \frac{2}{45} \cdot 264513 - \frac{1}{90} \cdot 246513 + \frac{1}{15} \cdot 426513 + \frac{1}{90} \cdot 365142 - \frac{7}{90} \cdot 265314 + \frac{1}{18} \cdot 165423 \\
&+ \frac{7}{90} \cdot 265413 + \frac{4}{45} \cdot 156423 + \frac{1}{15} \cdot 256413 + \frac{1}{15} \cdot 231456 + \frac{1}{45} \cdot 231465 + \frac{1}{45} \cdot 231546 \\
&- \frac{1}{45} \cdot 231645 + \frac{1}{45} \cdot 241356 + \frac{1}{45} \cdot 241365 + \frac{7}{90} \cdot 251634 - \frac{2}{45} \cdot 241563 + \frac{1}{90} \cdot 261453 \\
&+ \frac{1}{10} \cdot 321456 + \frac{1}{30} \cdot 321465 + \frac{1}{30} \cdot 321546 - \frac{1}{10} \cdot 321564 - \frac{1}{30} \cdot 321645 - \frac{1}{90} \cdot 324156 \\
&+ \frac{1}{90} \cdot 324165 + \frac{1}{90} \cdot 324516 + \frac{1}{18} \cdot 324615 - \frac{1}{30} \cdot 325146 - \frac{1}{30} \cdot 325164 + \frac{11}{90} \cdot 325614 \\
&+ \frac{1}{30} \cdot 421356 + \frac{1}{90} \cdot 421365 - \frac{1}{90} \cdot 421635 + \frac{1}{90} \cdot 521346 + \frac{11}{90} \cdot 521634 - \frac{1}{30} \cdot 324561
\end{aligned}
$$

$$+\frac{1}{18}\cdot 325641-\frac{1}{18}\cdot 326145-\frac{2}{45}\cdot 326415+\frac{1}{30}\cdot 326451-\frac{2}{45}\cdot 341256-\frac{1}{30}\cdot 341526$$
$$-\frac{1}{45}\cdot 341562-\frac{1}{90}\cdot 351246-\frac{1}{45}\cdot 361245-\frac{1}{90}\cdot 361425-\frac{1}{9}\cdot 361452-\frac{1}{90}\cdot 413562$$
$$-\frac{1}{18}\cdot 421563+\frac{2}{45}\cdot 425163+\frac{1}{15}\cdot 425613-\frac{1}{45}\cdot 521463+\frac{1}{30}\cdot 621345+\frac{7}{90}\cdot 621453$$
$$+\frac{1}{18}\cdot 621534-\frac{1}{15}\cdot 423156-\frac{1}{90}\cdot 423516-\frac{1}{45}\cdot 423561-\frac{1}{90}\cdot 425316+\frac{1}{90}\cdot 425361$$
$$-\frac{1}{30}\cdot 425631-\frac{4}{45}\cdot 431256-\frac{1}{18}\cdot 431526-\frac{2}{45}\cdot 431562-\frac{1}{30}\cdot 531246-\frac{1}{30}\cdot 531426$$
$$-\frac{1}{45}\cdot 631245-\frac{1}{90}\cdot 631425-\frac{1}{30}\cdot 631452-\frac{1}{5}\cdot 321654-\frac{1}{15}\cdot 326154+\frac{2}{45}\cdot 341265$$
$$+\frac{1}{90}\cdot 341625+\frac{1}{45}\cdot 351624+\frac{1}{18}\cdot 361524-\frac{2}{45}\cdot 413625-\frac{1}{45}\cdot 426153-\frac{1}{45}\cdot 423165$$
$$+\frac{1}{90}\cdot 423615-\frac{1}{90}\cdot 426315+\frac{1}{15}\cdot 426351+\frac{1}{30}\cdot 426531+\frac{1}{90}\cdot 431625+\frac{7}{90}\cdot 431652$$
$$+\frac{1}{18}\cdot 531624+\frac{1}{45}\cdot 531642+\frac{4}{45}\cdot 631524+\frac{1}{18}\cdot 631542-\frac{1}{30}\cdot 352164+\frac{1}{90}\cdot 362154$$
$$+\frac{13}{90}\cdot 432651-\frac{1}{30}\cdot 532164+\frac{2}{45}\cdot 215634+\frac{1}{90}\cdot 315624+\frac{1}{90}\cdot 352614-\frac{1}{45}\cdot 532614$$
$$+\frac{1}{15}\cdot 436152+\frac{7}{90}\cdot 632154+\frac{1}{90}\cdot 316452+\frac{1}{30}\cdot 436251+\frac{1}{18}\cdot 632514+\frac{4}{45}\cdot 134562$$
$$+\frac{1}{90}\cdot 135642+\frac{7}{90}\cdot 145632+\frac{1}{90}\cdot 145362+\frac{7}{90}\cdot 163452+\frac{4}{45}\cdot 234516+\frac{2}{45}\cdot 234615$$
$$+\frac{1}{90}\cdot 245316+\frac{1}{30}\cdot 246315-\frac{1}{90}\cdot 245613-\frac{2}{45}\cdot 263415-\frac{1}{45}\cdot 245631+\frac{2}{45}\cdot 314562$$
$$-\frac{1}{90}\cdot 315642-\frac{1}{90}\cdot 345162+\frac{7}{90}\cdot 345216+\frac{1}{18}\cdot 346215+\frac{1}{90}\cdot 356214+\frac{1}{90}\cdot 342516$$
$$-\frac{1}{90}\cdot 342615+\frac{7}{90}\cdot 523416-\frac{1}{45}\cdot 345261-\frac{1}{18}\cdot 356241-\frac{8}{45}\cdot 345612-\frac{4}{45}\cdot 346512$$
$$-\frac{4}{45}\cdot 354612-\frac{1}{15}\cdot 364512-\frac{1}{90}\cdot 354162-\frac{1}{45}\cdot 364152+\frac{1}{18}\cdot 415632+\frac{1}{90}\cdot 451632$$
$$-\frac{1}{18}\cdot 456132-\frac{2}{45}\cdot 513462-\frac{1}{18}\cdot 456213-\frac{1}{45}\cdot 524613-\frac{1}{30}\cdot 624513-\frac{2}{45}\cdot 456231$$
$$-\frac{1}{18}\cdot 452631-\frac{4}{45}\cdot 435612-\frac{1}{9}\cdot 456312-\frac{1}{90}\cdot 435162+\frac{1}{15}\cdot 453162-\frac{1}{15}\cdot 534612$$
$$-\frac{1}{9}\cdot 634512+\frac{2}{45}\cdot 534162-\frac{1}{30}\cdot 634152-\frac{1}{45}\cdot 134625-\frac{1}{45}\cdot 245163-\frac{1}{45}\cdot 235146$$
$$-\frac{2}{45}\cdot 236145-\frac{1}{30}\cdot 352146-\frac{1}{90}\cdot 524163+\frac{2}{45}\cdot 352641+\frac{4}{45}\cdot 256134+\frac{1}{45}\cdot 356124$$
$$+\frac{1}{15}\cdot 346125+\frac{7}{45}\cdot 436125+\frac{1}{45}\cdot 526134-\frac{1}{90}\cdot 461325-\frac{2}{45}\cdot 461352+\frac{1}{45}\cdot 362145$$
$$-\frac{1}{15}\cdot 462513-\frac{1}{90}\cdot 263145+\frac{1}{15}\cdot 624153-\frac{1}{90}\cdot 362451+\frac{4}{45}\cdot 462315-\frac{1}{30}\cdot 462351$$
$$+\frac{7}{90}\cdot 265134+\frac{1}{45}\cdot 364125+\frac{2}{45}\cdot 463125+\frac{1}{18}\cdot 463152+\frac{1}{90}\cdot 365124-\frac{1}{90}\cdot 625134$$
$$-\frac{1}{90}\cdot 635124-\frac{1}{18}\cdot 136542-\frac{1}{18}\cdot 254316-\frac{1}{90}\cdot 316542+\frac{1}{90}\cdot 354216-\frac{1}{30}\cdot 364215$$
$$-\frac{2}{15}\cdot 365214+\frac{1}{45}\cdot 362415+\frac{1}{90}\cdot 524316+\frac{1}{90}\cdot 364251-\frac{1}{45}\cdot 365241+\frac{17}{90}\cdot 365412$$
$$+\frac{1}{18}\cdot 461532-\frac{1}{15}\cdot 465132+\frac{1}{45}\cdot 513642-\frac{1}{15}\cdot 465213-\frac{2}{45}\cdot 526314+\frac{1}{18}\cdot 526413$$

$$
\begin{aligned}
&-\frac{1}{45}\cdot 624315-\frac{1}{30}\cdot 625314-\frac{1}{45}\cdot 625413+\frac{1}{18}\cdot 465231+\frac{1}{90}\cdot 462531-\frac{1}{45}\cdot 463512\\
&+\frac{1}{30}\cdot 465312-\frac{1}{45}\cdot 536412+\frac{7}{90}\cdot 635412-\frac{1}{15}\cdot 536142+\frac{1}{30}\cdot 635142+\frac{2}{45}\cdot 235641\\
&+\frac{2}{45}\cdot 245361-\frac{2}{45}\cdot 346521-\frac{4}{45}\cdot 436521-\frac{1}{90}\cdot 523641+\frac{1}{30}\cdot 532641+\frac{1}{9}\cdot 354126\\
&-\frac{2}{45}\cdot 354621-\frac{1}{15}\cdot 256341-\frac{1}{30}\cdot 526341+\frac{1}{90}\cdot 536241+\frac{1}{45}\cdot 461523-\frac{2}{45}\cdot 623541\\
&-\frac{4}{45}\cdot 632541-\frac{1}{15}\cdot 624351-\frac{2}{45}\cdot 364521-\frac{1}{45}\cdot 463521-\frac{1}{18}\cdot 265341-\frac{1}{15}\cdot 625341\\
&-\frac{2}{45}\cdot 635241-\frac{1}{45}\cdot 142563-\frac{1}{45}\cdot 314526-\frac{2}{45}\cdot 412563-\frac{1}{30}\cdot 415326+\frac{1}{15}\cdot 415623\\
&+\frac{4}{45}\cdot 451263+\frac{7}{45}\cdot 452163+\frac{1}{45}\cdot 461253+\frac{2}{45}\cdot 462153+\frac{1}{45}\cdot 451623-\frac{1}{90}\cdot 512463\\
&+\frac{1}{45}\cdot 514623+\frac{2}{45}\cdot 516423+\frac{1}{90}\cdot 541623+\frac{7}{90}\cdot 541263+\frac{11}{90}\cdot 542163-\frac{1}{90}\cdot 641523\\
&-\frac{1}{90}\cdot 641253+\frac{1}{18}\cdot 642153-\frac{4}{45}\cdot 342156-\frac{4}{45}\cdot 342165-\frac{8}{45}\cdot 432156-\frac{8}{45}\cdot 432165\\
&+\frac{1}{9}\cdot 432561+\frac{1}{9}\cdot 435126+\frac{1}{90}\cdot 435216+\frac{7}{90}\cdot 436215+\frac{1}{15}\cdot 452136+\frac{1}{9}\cdot 452316\\
&+\frac{1}{90}\cdot 462135+\frac{1}{15}\cdot 451326-\frac{1}{30}\cdot 514326-\frac{1}{30}\cdot 532146+\frac{1}{90}\cdot 532416+\frac{1}{9}\cdot 632145\\
&+\frac{2}{45}\cdot 532461+\frac{1}{9}\cdot 534126+\frac{1}{90}\cdot 534216+\frac{2}{45}\cdot 524361+\frac{1}{30}\cdot 542136+\frac{1}{30}\cdot 542316\\
&+\frac{1}{30}\cdot 541326+\frac{2}{45}\cdot 642135+\frac{1}{45}\cdot 641325-\frac{7}{90}\cdot 541362+\frac{1}{90}\cdot 542613+\frac{1}{18}\cdot 543126\\
&+\frac{7}{90}\cdot 543162+\frac{4}{45}\cdot 453126+\frac{2}{45}\cdot 342561-\frac{2}{45}\cdot 435621-\frac{1}{15}\cdot 452361-\frac{1}{30}\cdot 514632\\
&+\frac{1}{45}\cdot 536124+\frac{1}{18}\cdot 536214-\frac{2}{45}\cdot 632451-\frac{2}{45}\cdot 534621-\frac{1}{45}\cdot 536421-\frac{1}{18}\cdot 542361\\
&-\frac{1}{45}\cdot 542631-\frac{1}{15}\cdot 642351-\frac{2}{45}\cdot 642531-\frac{1}{18}\cdot 154362-\frac{2}{15}\cdot 541632-\frac{1}{18}\cdot 432516\\
&-\frac{1}{90}\cdot 432615+\frac{1}{90}\cdot 524631+\frac{17}{90}\cdot 543612-\frac{1}{15}\cdot 546132-\frac{1}{45}\cdot 614352-\frac{1}{30}\cdot 641352\\
&-\frac{1}{45}\cdot 643152-\frac{1}{15}\cdot 546213+\frac{1}{18}\cdot 546231+\frac{1}{30}\cdot 546312+\frac{1}{30}\cdot 642513+\frac{7}{90}\cdot 643512\\
&+\frac{1}{15}\cdot 145623+\frac{1}{15}\cdot 345126-\frac{1}{5}\cdot 456123-\frac{1}{6}\cdot 465123-\frac{1}{15}\cdot 614523-\frac{2}{45}\cdot 561324\\
&+\frac{1}{45}\cdot 562314-\frac{2}{45}\cdot 563124-\frac{1}{15}\cdot 634125+\frac{1}{45}\cdot 561342-\frac{1}{15}\cdot 562341+\frac{1}{90}\cdot 563241\\
&-\frac{1}{6}\cdot 546123-\frac{2}{45}\cdot 561423-\frac{1}{15}\cdot 564123+\frac{1}{18}\cdot 564213-\frac{2}{15}\cdot 645123+\frac{1}{30}\cdot 645213\\
&+\frac{1}{90}\cdot 562431+\frac{1}{18}\cdot 564132+\frac{1}{30}\cdot 645132-\frac{1}{18}\cdot 156432+\frac{1}{30}\cdot 516432+\frac{17}{90}\cdot 561432\\
&-\frac{1}{15}\cdot 562413-\frac{1}{18}\cdot 256431-\frac{1}{15}\cdot 563142-\frac{1}{18}\cdot 453216+\frac{1}{30}\cdot 463215+\frac{17}{90}\cdot 563214\\
&-\frac{1}{18}\cdot 453261-\frac{2}{15}\cdot 563412-\frac{1}{18}\cdot 614532-\frac{1}{18}\cdot 634215+\frac{1}{45}\cdot 564231+\frac{2}{45}\cdot 564312\\
&+\frac{1}{15}\cdot 645312+\frac{2}{45}\cdot 156234+\frac{1}{90}\cdot 163425+\frac{7}{90}\cdot 165234+\frac{2}{45}\cdot 451236-\frac{1}{30}\cdot 461235\\
&-\frac{1}{45}\cdot 263451-\frac{1}{30}\cdot 516234-\frac{1}{45}\cdot 416235+\frac{1}{90}\cdot 523146+\frac{7}{90}\cdot 541236-\frac{1}{45}\cdot 523461
\end{aligned}
$$

$$- \frac{8}{45} \cdot 561234 + \frac{1}{15} \cdot 613425 + \frac{2}{45} \cdot 623145 - \frac{4}{45} \cdot 623451 - \frac{1}{45} \cdot 624531 - \frac{8}{45} \cdot 651234$$
$$- \frac{2}{45} \cdot 651243 - \frac{4}{45} \cdot 651324 - \frac{2}{45} \cdot 651342 - \frac{1}{15} \cdot 651423 + \frac{1}{90} \cdot 162453 + \frac{1}{90} \cdot 513426$$
$$+ \frac{2}{45} \cdot 612453 - \frac{1}{45} \cdot 634251 - \frac{2}{45} \cdot 652134 - \frac{2}{45} \cdot 652314 - \frac{1}{15} \cdot 653124 + \frac{1}{30} \cdot 625431$$
$$+ \frac{1}{18} \cdot 651432 - \frac{4}{45} \cdot 652143 - \frac{1}{18} \cdot 615423 - \frac{1}{15} \cdot 652413 + \frac{1}{30} \cdot 643251 + \frac{1}{18} \cdot 653214$$
$$- \frac{1}{18} \cdot 643125 - \frac{1}{15} \cdot 653142 - \frac{1}{30} \cdot 264531 - \frac{1}{30} \cdot 534261 - \frac{1}{18} \cdot 615342 - \frac{1}{18} \cdot 642315$$
$$+ \frac{2}{45} \cdot 645231 + \frac{2}{45} \cdot 653412 - \frac{1}{45} \cdot 356421 - \frac{2}{9} \cdot 165432 - \frac{2}{45} \cdot 265431 + \frac{1}{90} \cdot 365421$$
$$- \frac{1}{45} \cdot 453621 + \frac{1}{30} \cdot 465321 - \frac{2}{9} \cdot 543216 - \frac{2}{45} \cdot 543261 + \frac{1}{90} \cdot 543621 + \frac{1}{30} \cdot 546321$$
$$+ \frac{2}{45} \cdot 563421 - \frac{2}{15} \cdot 615432 + \frac{1}{30} \cdot 635421 - \frac{2}{15} \cdot 643215 + \frac{1}{30} \cdot 643521 + \frac{1}{15} \cdot 645321$$
$$+ \frac{1}{18} \cdot 653241 + \frac{4}{45} \cdot 653421 + \frac{1}{18} \cdot 652431 + \frac{1}{18} \cdot 654132 + \frac{1}{18} \cdot 654213 + \frac{1}{9} \cdot 654231$$
$$+ \frac{8}{45} \cdot 654312$$

$$[\![y_1 \times y_5]\!] = \frac{1}{30} \cdot 123564 + \frac{1}{90} \cdot 132564 - \frac{1}{90} \cdot 135264 - \frac{1}{90} \cdot 152364 + \frac{1}{90} \cdot 213564 - \frac{1}{45} \cdot 231564$$
$$+ \frac{1}{45} \cdot 251364 + \frac{1}{15} \cdot 351264 - \frac{1}{30} \cdot 123645 - \frac{1}{90} \cdot 132645 - \frac{1}{90} \cdot 213645 + \frac{1}{45} \cdot 312645$$
$$+ \frac{1}{30} \cdot 124536 - \frac{1}{90} \cdot 412536 - \frac{1}{30} \cdot 124653 + \frac{1}{45} \cdot 142653 + \frac{1}{90} \cdot 412653 - \frac{1}{90} \cdot 416253$$
$$- \frac{1}{45} \cdot 461253 - \frac{1}{30} \cdot 125346 - \frac{1}{45} \cdot 153264 - \frac{2}{45} \cdot 235164 + \frac{1}{30} \cdot 253164 - \frac{1}{30} \cdot 512364$$
$$- \frac{2}{45} \cdot 513264 - \frac{1}{45} \cdot 521364 + \frac{1}{90} \cdot 523164 + \frac{1}{90} \cdot 531264 - \frac{1}{90} \cdot 125463 + \frac{2}{45} \cdot 135642$$
$$+ \frac{1}{90} \cdot 152643 + \frac{1}{90} \cdot 153642 + \frac{2}{45} \cdot 235641 + \frac{1}{90} \cdot 253641 + \frac{1}{18} \cdot 512643 + \frac{1}{90} \cdot 513642$$
$$- \frac{1}{30} \cdot 523641 + \frac{1}{90} \cdot 126354 + \frac{1}{45} \cdot 136254 + \frac{1}{90} \cdot 236154 + \frac{1}{30} \cdot 126435 - \frac{1}{45} \cdot 236415$$
$$- \frac{2}{45} \cdot 236451 + \frac{1}{45} \cdot 162453 - \frac{1}{90} \cdot 164253 + \frac{1}{45} \cdot 612453 - \frac{1}{90} \cdot 614253 + \frac{1}{90} \cdot 641253$$
$$- \frac{1}{90} \cdot 136524 - \frac{1}{90} \cdot 236514 - \frac{1}{45} \cdot 612534 + \frac{1}{90} \cdot 214536 - \frac{1}{90} \cdot 241536 - \frac{1}{90} \cdot 215346$$
$$+ \frac{1}{30} \cdot 134256 + \frac{1}{90} \cdot 134265 - \frac{1}{30} \cdot 135426 + \frac{1}{45} \cdot 315426 - \frac{1}{30} \cdot 316425 - \frac{1}{45} \cdot 361425$$
$$- \frac{1}{30} \cdot 142356 - \frac{1}{90} \cdot 142365 + \frac{1}{90} \cdot 142635 + \frac{1}{90} \cdot 142563 - \frac{1}{45} \cdot 421536 - \frac{1}{90} \cdot 143526$$
$$- \frac{1}{45} \cdot 143625 + \frac{1}{90} \cdot 146325 + \frac{2}{45} \cdot 245316 + \frac{1}{45} \cdot 245361 + \frac{1}{90} \cdot 415326 + \frac{1}{90} \cdot 415362$$
$$+ \frac{1}{90} \cdot 425316 + \frac{1}{90} \cdot 425361 + \frac{1}{90} \cdot 152436 + \frac{1}{45} \cdot 251436 + \frac{1}{30} \cdot 153246 + \frac{1}{45} \cdot 253614$$
$$- \frac{1}{45} \cdot 153462 - \frac{2}{45} \cdot 253461 + \frac{1}{45} \cdot 513426 - \frac{1}{90} \cdot 531426 + \frac{2}{45} \cdot 613425 - \frac{1}{90} \cdot 631425$$
$$- \frac{1}{90} \cdot 254136 - \frac{1}{90} \cdot 154263 - \frac{2}{45} \cdot 164235 - \frac{1}{90} \cdot 514263 - \frac{1}{45} \cdot 614235 - \frac{2}{45} \cdot 215643$$

$$
\begin{aligned}
&-\frac{2}{45}\cdot 251643-\frac{1}{90}\cdot 315642-\frac{1}{18}\cdot 351642+\frac{1}{90}\cdot 216435-\frac{1}{90}\cdot 316452-\frac{1}{45}\cdot 146532\\
&-\frac{1}{90}\cdot 416532+\frac{1}{45}\cdot 461532-\frac{1}{45}\cdot 521643-\frac{1}{18}\cdot 156432+\frac{1}{90}\cdot 256431-\frac{1}{45}\cdot 516423\\
&-\frac{1}{30}\cdot 516432+\frac{1}{30}\cdot 526431+\frac{1}{45}\cdot 162543-\frac{1}{45}\cdot 163542-\frac{1}{90}\cdot 261543+\frac{1}{45}\cdot 164352\\
&-\frac{1}{90}\cdot 264135-\frac{1}{45}\cdot 264153-\frac{1}{90}\cdot 164532+\frac{1}{15}\cdot 264351-\frac{2}{45}\cdot 264513+\frac{1}{90}\cdot 264531\\
&-\frac{1}{90}\cdot 614532-\frac{1}{90}\cdot 641532+\frac{1}{90}\cdot 165342+\frac{1}{30}\cdot 265143+\frac{1}{45}\cdot 165324-\frac{1}{90}\cdot 615342\\
&-\frac{1}{90}\cdot 214653+\frac{1}{90}\cdot 241653-\frac{1}{90}\cdot 261453+\frac{2}{45}\cdot 216534+\frac{1}{90}\cdot 261534+\frac{1}{90}\cdot 316542\\
&+\frac{1}{45}\cdot 361542+\frac{1}{30}\cdot 246153-\frac{1}{45}\cdot 154362-\frac{2}{45}\cdot 246531-\frac{1}{90}\cdot 426531-\frac{2}{45}\cdot 265314\\
&-\frac{1}{90}\cdot 265341-\frac{1}{45}\cdot 613542+\frac{1}{18}\cdot 631542+\frac{1}{18}\cdot 165423+\frac{1}{90}\cdot 265413+\frac{1}{90}\cdot 615423\\
&+\frac{1}{30}\cdot 231456+\frac{1}{90}\cdot 231465+\frac{1}{90}\cdot 231546-\frac{1}{30}\cdot 243156+\frac{1}{45}\cdot 263145-\frac{1}{30}\cdot 312456\\
&-\frac{1}{90}\cdot 312465-\frac{1}{90}\cdot 312546+\frac{1}{90}\cdot 314526-\frac{1}{45}\cdot 314625+\frac{1}{90}\cdot 315246-\frac{1}{15}\cdot 315624\\
&+\frac{1}{30}\cdot 314562+\frac{1}{45}\cdot 314652+\frac{2}{45}\cdot 315462+\frac{2}{45}\cdot 316245-\frac{1}{90}\cdot 324156-\frac{1}{45}\cdot 325146\\
&-\frac{1}{90}\cdot 326145+\frac{1}{90}\cdot 352146+\frac{1}{90}\cdot 362145+\frac{1}{45}\cdot 342561+\frac{1}{90}\cdot 413256+\frac{1}{30}\cdot 421356\\
&-\frac{1}{90}\cdot 421563+\frac{1}{90}\cdot 425163+\frac{1}{45}\cdot 425613-\frac{1}{45}\cdot 423516-\frac{1}{45}\cdot 423561-\frac{1}{90}\cdot 425631\\
&+\frac{2}{45}\cdot 623145-\frac{1}{90}\cdot 431526-\frac{1}{18}\cdot 431562-\frac{2}{45}\cdot 531246-\frac{1}{90}\cdot 531462-\frac{2}{45}\cdot 631245\\
&+\frac{1}{30}\cdot 631452-\frac{1}{30}\cdot 231654-\frac{1}{90}\cdot 243165+\frac{1}{30}\cdot 263154+\frac{1}{30}\cdot 312654+\frac{1}{30}\cdot 316254\\
&+\frac{1}{90}\cdot 324165-\frac{1}{30}\cdot 325164-\frac{2}{45}\cdot 342165-\frac{2}{45}\cdot 362154-\frac{1}{90}\cdot 342615-\frac{1}{90}\cdot 342651\\
&-\frac{1}{90}\cdot 413265+\frac{1}{90}\cdot 421365-\frac{1}{90}\cdot 421635-\frac{1}{30}\cdot 426135+\frac{1}{45}\cdot 426513+\frac{1}{90}\cdot 423615\\
&-\frac{1}{90}\cdot 423651+\frac{1}{45}\cdot 426315+\frac{1}{30}\cdot 623154+\frac{2}{45}\cdot 431265+\frac{2}{45}\cdot 431625+\frac{1}{45}\cdot 431652\\
&+\frac{1}{18}\cdot 531624-\frac{1}{90}\cdot 631254+\frac{1}{45}\cdot 631524-\frac{1}{30}\cdot 321564+\frac{1}{30}\cdot 321645-\frac{1}{45}\cdot 462153\\
&-\frac{1}{90}\cdot 532164+\frac{1}{90}\cdot 215463+\frac{1}{90}\cdot 325641-\frac{1}{45}\cdot 352641-\frac{1}{18}\cdot 532641-\frac{1}{90}\cdot 216354\\
&-\frac{1}{30}\cdot 326415-\frac{1}{30}\cdot 326451+\frac{1}{90}\cdot 621453+\frac{1}{90}\cdot 642153+\frac{2}{45}\cdot 326514+\frac{1}{90}\cdot 621534\\
&+\frac{2}{45}\cdot 134562+\frac{1}{90}\cdot 145623+\frac{2}{45}\cdot 234516+\frac{1}{90}\cdot 234615+\frac{1}{90}\cdot 235614-\frac{1}{90}\cdot 243561\\
&+\frac{1}{90}\cdot 345126+\frac{1}{90}\cdot 345162+\frac{1}{45}\cdot 346152-\frac{1}{90}\cdot 356142-\frac{1}{30}\cdot 324561-\frac{1}{45}\cdot 324651\\
&-\frac{1}{90}\cdot 346251+\frac{1}{90}\cdot 352461-\frac{2}{45}\cdot 356241+\frac{4}{45}\cdot 345621+\frac{1}{45}\cdot 354621+\frac{1}{30}\cdot 356421\\
&+\frac{1}{18}\cdot 362451+\frac{1}{45}\cdot 364251-\frac{1}{90}\cdot 364521+\frac{1}{45}\cdot 413562-\frac{1}{90}\cdot 415632+\frac{1}{90}\cdot 451362\\
&+\frac{1}{90}\cdot 451632+\frac{1}{18}\cdot 456132+\frac{1}{18}\cdot 456213+\frac{2}{45}\cdot 456231-\frac{1}{45}\cdot 523461-\frac{1}{90}\cdot 435162
\end{aligned}
$$

$$- \frac{2}{45} \cdot 435612 + \frac{1}{45} \cdot 453162 + \frac{1}{90} \cdot 453612 - \frac{1}{45} \cdot 456312 - \frac{1}{30} \cdot 534612 - \frac{1}{45} \cdot 634512$$
$$+ \frac{1}{90} \cdot 135462 + \frac{1}{90} \cdot 143562 - \frac{1}{90} \cdot 341562 - \frac{1}{45} \cdot 351462 - \frac{1}{30} \cdot 134625 - \frac{1}{90} \cdot 135624$$
$$- \frac{1}{45} \cdot 415623 + \frac{1}{90} \cdot 243516 + \frac{1}{90} \cdot 324516 - \frac{1}{30} \cdot 234651 + \frac{1}{90} \cdot 246351 - \frac{1}{45} \cdot 462351$$
$$- \frac{1}{30} \cdot 235146 - \frac{1}{90} \cdot 245136 - \frac{1}{90} \cdot 354162 - \frac{1}{90} \cdot 235461 - \frac{1}{45} \cdot 245631 + \frac{1}{90} \cdot 453621$$
$$+ \frac{1}{90} \cdot 534621 - \frac{1}{90} \cdot 346215 - \frac{1}{90} \cdot 356214 + \frac{1}{45} \cdot 632451 - \frac{1}{90} \cdot 634251 - \frac{1}{18} \cdot 642351$$
$$- \frac{2}{45} \cdot 346512 + \frac{1}{30} \cdot 356412 - \frac{1}{90} \cdot 246513 - \frac{1}{90} \cdot 263514 - \frac{1}{18} \cdot 364512 - \frac{1}{18} \cdot 623514$$
$$+ \frac{1}{45} \cdot 624513 + \frac{1}{90} \cdot 413625 + \frac{1}{30} \cdot 136245 + \frac{1}{90} \cdot 146235 + \frac{1}{30} \cdot 251346 - \frac{1}{90} \cdot 251463$$
$$+ \frac{1}{90} \cdot 351246 + \frac{1}{45} \cdot 513624 + \frac{1}{90} \cdot 254613 + \frac{1}{90} \cdot 352614 - \frac{1}{30} \cdot 256314 - \frac{1}{30} \cdot 436215$$
$$- \frac{1}{90} \cdot 436251 + \frac{1}{45} \cdot 536214 - \frac{1}{90} \cdot 536241 - \frac{1}{90} \cdot 361524 - \frac{1}{90} \cdot 461325 + \frac{1}{90} \cdot 362415$$
$$+ \frac{1}{90} \cdot 462135 + \frac{1}{30} \cdot 362541 + \frac{2}{45} \cdot 462315 - \frac{1}{90} \cdot 462531 - \frac{1}{30} \cdot 632514 + \frac{1}{90} \cdot 642513$$
$$+ \frac{1}{30} \cdot 364125 + \frac{1}{90} \cdot 365124 + \frac{1}{90} \cdot 265134 - \frac{1}{45} \cdot 365142 + \frac{1}{90} \cdot 625134 + \frac{1}{90} \cdot 625143$$
$$+ \frac{2}{45} \cdot 635124 + \frac{1}{90} \cdot 635142 - \frac{1}{90} \cdot 134652 + \frac{1}{90} \cdot 146523 - \frac{1}{90} \cdot 235416 + \frac{1}{45} \cdot 263541$$
$$+ \frac{1}{90} \cdot 354126 - \frac{1}{90} \cdot 364152 + \frac{1}{30} \cdot 326541 - \frac{1}{30} \cdot 365241 - \frac{1}{45} \cdot 365421 + \frac{1}{90} \cdot 413652$$
$$- \frac{1}{45} \cdot 416352 - \frac{1}{30} \cdot 461352 + \frac{1}{90} \cdot 465231 - \frac{1}{45} \cdot 623541 + \frac{1}{45} \cdot 463512 - \frac{1}{90} \cdot 465312$$
$$+ \frac{1}{45} \cdot 536412 + \frac{1}{90} \cdot 635412 - \frac{1}{45} \cdot 254631 + \frac{1}{45} \cdot 536421 + \frac{2}{45} \cdot 364215 + \frac{1}{18} \cdot 624531$$
$$- \frac{1}{45} \cdot 625314 + \frac{1}{90} \cdot 625341 - \frac{1}{90} \cdot 145263 + \frac{1}{90} \cdot 152634 - \frac{1}{90} \cdot 341526 + \frac{1}{90} \cdot 415236$$
$$- \frac{1}{45} \cdot 512463 + \frac{1}{90} \cdot 516243 - \frac{1}{90} \cdot 521463 + \frac{1}{45} \cdot 524163 + \frac{1}{90} \cdot 516324 + \frac{1}{90} \cdot 526314$$
$$+ \frac{1}{45} \cdot 526341 - \frac{1}{45} \cdot 634152 - \frac{1}{90} \cdot 514623 + \frac{1}{30} \cdot 524613 + \frac{1}{90} \cdot 541263 - \frac{1}{90} \cdot 541623$$
$$+ \frac{1}{90} \cdot 542163 - \frac{1}{45} \cdot 542613 - \frac{1}{45} \cdot 354216 - \frac{1}{18} \cdot 453216 - \frac{1}{90} \cdot 463215 - \frac{1}{90} \cdot 453261$$
$$+ \frac{1}{45} \cdot 514326 - \frac{1}{45} \cdot 524316 + \frac{1}{45} \cdot 532416 - \frac{1}{45} \cdot 532614 + \frac{1}{45} \cdot 532461 - \frac{1}{90} \cdot 534216$$
$$+ \frac{1}{90} \cdot 534261 + \frac{1}{90} \cdot 634215 + \frac{1}{90} \cdot 542316 + \frac{1}{45} \cdot 542136 + \frac{2}{45} \cdot 642135 - \frac{1}{90} \cdot 642315$$
$$+ \frac{1}{90} \cdot 246315 - \frac{1}{45} \cdot 432516 + \frac{1}{90} \cdot 432615 + \frac{1}{90} \cdot 542361 + \frac{1}{90} \cdot 542631 - \frac{1}{15} \cdot 624315$$
$$+ \frac{1}{18} \cdot 543126 + \frac{1}{30} \cdot 543162 - \frac{1}{90} \cdot 643125 - \frac{1}{30} \cdot 643152 - \frac{1}{90} \cdot 463251 + \frac{1}{90} \cdot 536124$$
$$+ \frac{1}{30} \cdot 154623 + \frac{1}{30} \cdot 432651 + \frac{1}{30} \cdot 435126 - \frac{1}{45} \cdot 543621 + \frac{1}{90} \cdot 546231 - \frac{1}{45} \cdot 643251$$
$$- \frac{1}{90} \cdot 546312 + \frac{1}{18} \cdot 643512 + \frac{1}{90} \cdot 245613 - \frac{1}{90} \cdot 156234 - \frac{1}{45} \cdot 354612 - \frac{1}{90} \cdot 451236$$
$$- \frac{1}{90} \cdot 461235 + \frac{1}{45} \cdot 451263 + \frac{2}{45} \cdot 561243 - \frac{1}{90} \cdot 561423 - \frac{1}{45} \cdot 562413 + \frac{1}{45} \cdot 561324$$

$$
\begin{aligned}
&+\frac{1}{18}\cdot 562314+\frac{1}{30}\cdot 561342+\frac{1}{45}\cdot 562341-\frac{1}{18}\cdot 546123+\frac{1}{45}\cdot 564123+\frac{1}{90}\cdot 564213\\
&-\frac{2}{45}\cdot 645123-\frac{1}{30}\cdot 156243-\frac{1}{90}\cdot 516234-\frac{1}{30}\cdot 451326-\frac{1}{90}\cdot 452613+\frac{1}{90}\cdot 461523\\
&+\frac{2}{45}\cdot 562134-\frac{1}{18}\cdot 562431-\frac{1}{18}\cdot 465123-\frac{1}{30}\cdot 563124-\frac{1}{90}\cdot 645132+\frac{1}{45}\cdot 524631\\
&-\frac{1}{45}\cdot 563142-\frac{1}{90}\cdot 563241+\frac{1}{45}\cdot 463521+\frac{1}{90}\cdot 564132-\frac{1}{45}\cdot 564231+\frac{1}{45}\cdot 645312\\
&-\frac{2}{45}\cdot 162345-\frac{1}{90}\cdot 162354-\frac{1}{90}\cdot 162435-\frac{2}{45}\cdot 512346-\frac{1}{90}\cdot 512436+\frac{1}{90}\cdot 512634\\
&-\frac{1}{90}\cdot 513246-\frac{1}{45}\cdot 526134+\frac{1}{90}\cdot 613245+\frac{1}{30}\cdot 621345+\frac{1}{45}\cdot 621354-\frac{1}{90}\cdot 624135\\
&+\frac{1}{45}\cdot 641235-\frac{4}{45}\cdot 651234-\frac{1}{45}\cdot 651324-\frac{1}{90}\cdot 651342-\frac{1}{90}\cdot 651423-\frac{1}{90}\cdot 261345\\
&-\frac{1}{90}\cdot 361245+\frac{1}{30}\cdot 612354-\frac{1}{90}\cdot 613524+\frac{1}{90}\cdot 612435+\frac{1}{45}\cdot 613452+\frac{1}{90}\cdot 652314\\
&-\frac{1}{30}\cdot 653124-\frac{1}{30}\cdot 621543+\frac{1}{90}\cdot 625413+\frac{1}{45}\cdot 625431+\frac{1}{45}\cdot 651432-\frac{1}{45}\cdot 653142\\
&-\frac{1}{90}\cdot 156324+\frac{1}{90}\cdot 163245-\frac{1}{90}\cdot 452136+\frac{1}{90}\cdot 521346-\frac{1}{30}\cdot 632154+\frac{1}{30}\cdot 635214\\
&-\frac{1}{45}\cdot 632415-\frac{1}{90}\cdot 645213+\frac{1}{45}\cdot 653214+\frac{1}{45}\cdot 641325+\frac{1}{90}\cdot 146352-\frac{1}{90}\cdot 163524\\
&+\frac{1}{90}\cdot 352416-\frac{1}{90}\cdot 524136-\frac{1}{45}\cdot 641352-\frac{1}{45}\cdot 652413-\frac{1}{90}\cdot 465321-\frac{1}{90}\cdot 546321\\
&-\frac{4}{45}\cdot 564321-\frac{2}{45}\cdot 615432-\frac{1}{30}\cdot 635421-\frac{2}{45}\cdot 643215+\frac{1}{90}\cdot 643521-\frac{1}{45}\cdot 645321\\
&-\frac{1}{90}\cdot 652431+\frac{1}{30}\cdot 653241+\frac{2}{45}\cdot 265431+\frac{2}{45}\cdot 543261+\frac{1}{90}\cdot 654132+\frac{1}{90}\cdot 654213\\
&+\frac{1}{45}\cdot 654231+\frac{4}{45}\cdot 654312
\end{aligned}
$$

$$
\begin{aligned}
\llbracket y_2\times y_2\rrbracket =\ &\frac{2}{45}\cdot 126453+\frac{2}{45}\cdot 126543+\frac{2}{45}\cdot 216453+\frac{2}{45}\cdot 216543-\frac{1}{45}\cdot 135462-\frac{1}{45}\cdot 135642\\
&-\frac{1}{45}\cdot 145362-\frac{1}{45}\cdot 145632-\frac{1}{45}\cdot 315462-\frac{1}{45}\cdot 315642-\frac{1}{45}\cdot 415362-\frac{1}{45}\cdot 415632\\
&+\frac{2}{45}\cdot 153426+\frac{2}{45}\cdot 154326-\frac{1}{45}\cdot 153624-\frac{1}{45}\cdot 154623-\frac{1}{45}\cdot 156324-\frac{2}{45}\cdot 156423\\
&-\frac{1}{45}\cdot 146253-\frac{1}{45}\cdot 146523-\frac{1}{45}\cdot 156243-\frac{1}{45}\cdot 246153+\frac{1}{45}\cdot 246513-\frac{1}{45}\cdot 256143\\
&-\frac{1}{45}\cdot 256413-\frac{1}{45}\cdot 416253-\frac{1}{45}\cdot 416523-\frac{2}{45}\cdot 426153-\frac{1}{45}\cdot 426513+\frac{1}{45}\cdot 516243\\
&-\frac{1}{45}\cdot 516423-\frac{1}{45}\cdot 526143-\frac{1}{45}\cdot 526413-\frac{1}{45}\cdot 162435-\frac{1}{45}\cdot 162534-\frac{1}{45}\cdot 164235\\
&-\frac{1}{45}\cdot 165234-\frac{1}{45}\cdot 261435-\frac{1}{45}\cdot 261534-\frac{1}{45}\cdot 264135-\frac{1}{45}\cdot 265134+\frac{2}{45}\cdot 164532\\
&+\frac{4}{45}\cdot 165432+\frac{1}{45}\cdot 264531+\frac{2}{45}\cdot 265431+\frac{2}{45}\cdot 165342+\frac{1}{45}\cdot 615342+\frac{2}{45}\cdot 615432\\
&+\frac{2}{45}\cdot 234561+\frac{2}{45}\cdot 234651+\frac{2}{45}\cdot 324561+\frac{2}{45}\cdot 324651-\frac{1}{45}\cdot 243516-\frac{1}{45}\cdot 243615\\
&-\frac{1}{45}\cdot 245316-\frac{1}{45}\cdot 246315-\frac{1}{45}\cdot 342516-\frac{1}{45}\cdot 342615-\frac{1}{45}\cdot 345216-\frac{1}{45}\cdot 346215
\end{aligned}
$$

$$+\frac{2}{45}\cdot 245613+\frac{4}{45}\cdot 345612+\frac{2}{45}\cdot 346512+\frac{2}{45}\cdot 345162+\frac{1}{45}\cdot 435162+\frac{2}{45}\cdot 435612$$
$$+\frac{2}{45}\cdot 351624+\frac{2}{45}\cdot 356124+\frac{2}{45}\cdot 451623+\frac{2}{15}\cdot 456123-\frac{2}{45}\cdot 354621-\frac{1}{45}\cdot 356421$$
$$-\frac{1}{45}\cdot 453621-\frac{1}{45}\cdot 456321-\frac{1}{45}\cdot 254361-\frac{1}{45}\cdot 254631-\frac{1}{45}\cdot 264351-\frac{1}{45}\cdot 354261$$
$$-\frac{1}{45}\cdot 364251-\frac{1}{45}\cdot 364521-\frac{1}{45}\cdot 524361-\frac{1}{45}\cdot 524631+\frac{1}{45}\cdot 534261-\frac{1}{45}\cdot 534621$$
$$-\frac{2}{45}\cdot 624351-\frac{1}{45}\cdot 624531-\frac{1}{45}\cdot 634251-\frac{1}{45}\cdot 634521+\frac{2}{45}\cdot 423156+\frac{2}{45}\cdot 423165$$
$$+\frac{2}{45}\cdot 432156+\frac{2}{45}\cdot 432165-\frac{1}{45}\cdot 425136-\frac{1}{45}\cdot 425163-\frac{1}{45}\cdot 426135-\frac{1}{45}\cdot 435126$$
$$-\frac{1}{45}\cdot 436125-\frac{1}{45}\cdot 436152-\frac{1}{45}\cdot 452136-\frac{1}{45}\cdot 452163-\frac{2}{45}\cdot 453126-\frac{1}{45}\cdot 453162$$
$$+\frac{1}{45}\cdot 462135-\frac{1}{45}\cdot 462153-\frac{1}{45}\cdot 463125-\frac{1}{45}\cdot 463152-\frac{1}{45}\cdot 351426-\frac{1}{45}\cdot 354126$$
$$-\frac{1}{45}\cdot 451326-\frac{1}{45}\cdot 513246-\frac{1}{45}\cdot 513264-\frac{1}{45}\cdot 514236-\frac{1}{45}\cdot 514263-\frac{1}{45}\cdot 531246$$
$$-\frac{1}{45}\cdot 531264-\frac{1}{45}\cdot 541236-\frac{1}{45}\cdot 541263+\frac{2}{45}\cdot 534216+\frac{4}{45}\cdot 543216+\frac{2}{45}\cdot 543261$$
$$+\frac{2}{45}\cdot 542316+\frac{1}{45}\cdot 642315+\frac{2}{45}\cdot 643215+\frac{2}{45}\cdot 456132+\frac{2}{45}\cdot 465123+\frac{2}{45}\cdot 516234$$
$$+\frac{4}{45}\cdot 561234+\frac{2}{45}\cdot 561243-\frac{1}{45}\cdot 536214-\frac{1}{45}\cdot 536241-\frac{1}{45}\cdot 546231-\frac{1}{45}\cdot 563214$$
$$-\frac{1}{45}\cdot 563241-\frac{1}{45}\cdot 564213-\frac{1}{45}\cdot 542613-\frac{1}{45}\cdot 543612-\frac{1}{45}\cdot 546312-\frac{1}{45}\cdot 642513$$
$$-\frac{1}{45}\cdot 643512-\frac{1}{45}\cdot 645213+\frac{2}{45}\cdot 456213+\frac{2}{45}\cdot 546123+\frac{2}{45}\cdot 461235+\frac{2}{45}\cdot 562134$$
$$-\frac{1}{45}\cdot 461532-\frac{1}{45}\cdot 462531-\frac{1}{45}\cdot 465231-\frac{1}{45}\cdot 561432-\frac{1}{45}\cdot 562431-\frac{1}{45}\cdot 564132$$
$$-\frac{1}{45}\cdot 365142-\frac{1}{45}\cdot 365412-\frac{1}{45}\cdot 465312-\frac{1}{45}\cdot 635142-\frac{1}{45}\cdot 635412-\frac{1}{45}\cdot 645132$$
$$+\frac{2}{45}\cdot 612345+\frac{2}{45}\cdot 612354+\frac{2}{45}\cdot 621345+\frac{2}{45}\cdot 621354-\frac{1}{45}\cdot 614325-\frac{1}{45}\cdot 614352$$
$$-\frac{1}{45}\cdot 615324-\frac{1}{45}\cdot 624315-\frac{1}{45}\cdot 625314-\frac{1}{45}\cdot 625341-\frac{1}{45}\cdot 641325-\frac{1}{45}\cdot 641352$$
$$-\frac{1}{45}\cdot 642351-\frac{2}{45}\cdot 651324-\frac{1}{45}\cdot 651342-\frac{1}{45}\cdot 652314-\frac{1}{45}\cdot 652341-\frac{1}{45}\cdot 651423$$
$$-\frac{1}{45}\cdot 653124-\frac{1}{45}\cdot 654123+\frac{2}{45}\cdot 645321+\frac{2}{45}\cdot 654312+\frac{2}{15}\cdot 654321+\frac{2}{45}\cdot 653421$$
$$+\frac{2}{45}\cdot 564321+\frac{2}{45}\cdot 654231$$

$$[\![y_2\times y_3]\!]=-\frac{1}{45}\cdot 124653-\frac{1}{45}\cdot 125643-\frac{1}{45}\cdot 214653-\frac{1}{45}\cdot 215643-\frac{1}{45}\cdot 126354-\frac{1}{45}\cdot 126534$$
$$-\frac{1}{45}\cdot 216354-\frac{1}{45}\cdot 216534-\frac{4}{45}\cdot 126543-\frac{4}{45}\cdot 216543-\frac{2}{45}\cdot 126453-\frac{2}{45}\cdot 216453$$
$$-\frac{1}{45}\cdot 135426-\frac{1}{45}\cdot 145326-\frac{1}{90}\cdot 136425-\frac{1}{90}\cdot 136524-\frac{1}{90}\cdot 146325-\frac{1}{90}\cdot 316425$$
$$-\frac{1}{90}\cdot 316524-\frac{1}{45}\cdot 416325+\frac{1}{45}\cdot 236154+\frac{1}{45}\cdot 236514+\frac{1}{45}\cdot 326154+\frac{1}{45}\cdot 326514$$

$$+\frac{1}{45}\cdot 236541+\frac{1}{45}\cdot 326541-\frac{1}{90}\cdot 136452-\frac{1}{30}\cdot 136542-\frac{1}{90}\cdot 316452-\frac{1}{90}\cdot 316542$$
$$-\frac{1}{45}\cdot 152436-\frac{1}{45}\cdot 154236-\frac{1}{90}\cdot 152463-\frac{1}{90}\cdot 152643-\frac{1}{90}\cdot 154263-\frac{1}{90}\cdot 251463$$
$$-\frac{1}{90}\cdot 251643-\frac{1}{45}\cdot 254163+\frac{1}{45}\cdot 412653+\frac{1}{45}\cdot 421653+\frac{1}{45}\cdot 512643+\frac{1}{45}\cdot 521643$$
$$-\frac{4}{45}\cdot 154326-\frac{2}{45}\cdot 153426+\frac{1}{45}\cdot 254361-\frac{1}{90}\cdot 154362-\frac{1}{45}\cdot 514362-\frac{1}{45}\cdot 514632$$
$$+\frac{1}{45}\cdot 153624+\frac{1}{15}\cdot 154623+\frac{1}{15}\cdot 156324+\frac{1}{15}\cdot 156423+\frac{2}{45}\cdot 156243+\frac{1}{30}\cdot 254613$$
$$+\frac{1}{15}\cdot 256143+\frac{2}{45}\cdot 256413+\frac{2}{45}\cdot 146523+\frac{1}{15}\cdot 416523+\frac{1}{30}\cdot 516324+\frac{2}{45}\cdot 516423$$
$$+\frac{1}{45}\cdot 146253+\frac{1}{30}\cdot 246153+\frac{1}{90}\cdot 246513+\frac{1}{30}\cdot 416253+\frac{2}{45}\cdot 426153+\frac{1}{30}\cdot 426513$$
$$+\frac{1}{90}\cdot 516243+\frac{1}{30}\cdot 526143+\frac{1}{45}\cdot 526413+\frac{1}{90}\cdot 254631+\frac{2}{45}\cdot 156342+\frac{1}{45}\cdot 516342$$
$$+\frac{1}{45}\cdot 516432-\frac{1}{90}\cdot 162453-\frac{1}{30}\cdot 162543-\frac{1}{90}\cdot 261453-\frac{1}{90}\cdot 261543+\frac{1}{45}\cdot 612543$$
$$+\frac{1}{45}\cdot 621543-\frac{1}{90}\cdot 164325-\frac{1}{45}\cdot 264315-\frac{1}{45}\cdot 265314+\frac{1}{45}\cdot 614325+\frac{1}{45}\cdot 164352$$
$$-\frac{1}{45}\cdot 165342+\frac{1}{90}\cdot 264351-\frac{1}{45}\cdot 265341-\frac{1}{45}\cdot 164532+\frac{1}{90}\cdot 614352-\frac{1}{45}\cdot 614532$$
$$+\frac{2}{45}\cdot 164523+\frac{1}{45}\cdot 264513+\frac{1}{45}\cdot 265413+\frac{1}{90}\cdot 615324+\frac{1}{45}\cdot 134562+\frac{1}{45}\cdot 143562$$
$$+\frac{1}{90}\cdot 145263+\frac{2}{45}\cdot 145623+\frac{1}{45}\cdot 415263+\frac{1}{45}\cdot 415623+\frac{1}{45}\cdot 145632+\frac{1}{45}\cdot 415632$$
$$+\frac{1}{45}\cdot 135462+\frac{1}{90}\cdot 135642+\frac{1}{90}\cdot 145362+\frac{1}{45}\cdot 315462+\frac{1}{90}\cdot 315642+\frac{1}{90}\cdot 415362$$
$$+\frac{1}{90}\cdot 153462+\frac{1}{45}\cdot 163452+\frac{1}{45}\cdot 234516+\frac{1}{45}\cdot 234615+\frac{1}{45}\cdot 324516+\frac{1}{45}\cdot 324615$$
$$+\frac{1}{45}\cdot 235614+\frac{1}{45}\cdot 325614-\frac{1}{90}\cdot 245613+\frac{1}{90}\cdot 425163-\frac{1}{90}\cdot 425613-\frac{1}{90}\cdot 245631$$
$$-\frac{1}{90}\cdot 425631+\frac{1}{45}\cdot 235461+\frac{1}{45}\cdot 235641+\frac{1}{45}\cdot 325461+\frac{1}{45}\cdot 325641+\frac{1}{90}\cdot 341526$$
$$+\frac{1}{90}\cdot 341625+\frac{2}{45}\cdot 345126+\frac{2}{45}\cdot 346125+\frac{1}{45}\cdot 341652-\frac{1}{45}\cdot 431562+\frac{1}{45}\cdot 345216$$
$$+\frac{1}{45}\cdot 346215+\frac{1}{45}\cdot 243516+\frac{1}{45}\cdot 243615+\frac{1}{90}\cdot 245316+\frac{1}{90}\cdot 246315+\frac{1}{90}\cdot 342516$$
$$+\frac{1}{90}\cdot 342615-\frac{1}{90}\cdot 253416+\frac{1}{90}\cdot 423516+\frac{1}{90}\cdot 423615+\frac{1}{45}\cdot 523416-\frac{1}{30}\cdot 345261$$
$$-\frac{1}{90}\cdot 346251+\frac{1}{45}\cdot 243561+\frac{1}{45}\cdot 243651+\frac{1}{45}\cdot 423561+\frac{1}{45}\cdot 423651-\frac{4}{45}\cdot 345612$$
$$-\frac{1}{45}\cdot 346512-\frac{1}{45}\cdot 435612-\frac{1}{90}\cdot 345162+\frac{1}{90}\cdot 435162-\frac{2}{45}\cdot 345621-\frac{1}{45}\cdot 346521$$
$$-\frac{1}{90}\cdot 435261-\frac{1}{45}\cdot 435621+\frac{1}{90}\cdot 351642-\frac{4}{45}\cdot 456132-\frac{1}{45}\cdot 361452-\frac{1}{45}\cdot 513462$$
$$-\frac{1}{90}\cdot 531462-\frac{1}{30}\cdot 613452-\frac{1}{90}\cdot 631452-\frac{1}{45}\cdot 356214-\frac{4}{45}\cdot 456213-\frac{1}{45}\cdot 263415$$
$$-\frac{1}{90}\cdot 263514-\frac{1}{45}\cdot 523614-\frac{1}{90}\cdot 623415-\frac{1}{90}\cdot 623514-\frac{1}{45}\cdot 356241-\frac{2}{45}\cdot 456231$$
$$-\frac{1}{30}\cdot 263451-\frac{1}{30}\cdot 263541-\frac{2}{45}\cdot 623451-\frac{2}{45}\cdot 623541+\frac{1}{90}\cdot 354162+\frac{1}{45}\cdot 453162$$

$$-\frac{1}{45}\cdot 453612-\frac{2}{45}\cdot 456312-\frac{1}{45}\cdot 364512-\frac{1}{90}\cdot 524613-\frac{1}{45}\cdot 624513-\frac{2}{45}\cdot 634512$$
$$-\frac{1}{45}\cdot 243156-\frac{1}{45}\cdot 243165-\frac{1}{45}\cdot 342156-\frac{1}{45}\cdot 342165-\frac{1}{90}\cdot 253146-\frac{1}{90}\cdot 253164$$
$$-\frac{1}{90}\cdot 254136-\frac{1}{90}\cdot 352146-\frac{1}{90}\cdot 352164-\frac{1}{30}\cdot 254316-\frac{1}{45}\cdot 413256-\frac{1}{45}\cdot 413265$$
$$-\frac{1}{45}\cdot 431256-\frac{1}{45}\cdot 431265-\frac{1}{90}\cdot 413526-\frac{1}{90}\cdot 413625-\frac{1}{90}\cdot 415326-\frac{1}{90}\cdot 431526$$
$$-\frac{1}{90}\cdot 431625-\frac{4}{45}\cdot 432156-\frac{4}{45}\cdot 432165-\frac{2}{45}\cdot 423156-\frac{2}{45}\cdot 423165+\frac{1}{45}\cdot 432561$$
$$+\frac{1}{45}\cdot 432651-\frac{1}{90}\cdot 432516-\frac{1}{90}\cdot 432615-\frac{1}{45}\cdot 532614-\frac{1}{45}\cdot 536214+\frac{1}{45}\cdot 425136$$
$$+\frac{1}{90}\cdot 426135+\frac{1}{15}\cdot 435126+\frac{1}{15}\cdot 436125+\frac{1}{18}\cdot 436152+\frac{1}{15}\cdot 452136+\frac{1}{15}\cdot 452163$$
$$+\frac{1}{15}\cdot 453126+\frac{1}{90}\cdot 462135+\frac{1}{18}\cdot 462153+\frac{1}{45}\cdot 463125+\frac{1}{45}\cdot 463152+\frac{2}{45}\cdot 451326$$
$$+\frac{1}{90}\cdot 461325+\frac{2}{45}\cdot 354126+\frac{1}{45}\cdot 351426+\frac{1}{90}\cdot 436251-\frac{1}{45}\cdot 453261+\frac{2}{45}\cdot 452316$$
$$-\frac{1}{90}\cdot 513426-\frac{1}{30}\cdot 514326-\frac{1}{90}\cdot 532146-\frac{1}{90}\cdot 532164-\frac{1}{45}\cdot 542613+\frac{1}{45}\cdot 632145$$
$$+\frac{1}{45}\cdot 632154+\frac{1}{45}\cdot 532416+\frac{1}{90}\cdot 532461+\frac{1}{90}\cdot 532641-\frac{1}{45}\cdot 542316-\frac{1}{45}\cdot 534216$$
$$+\frac{1}{90}\cdot 632415+\frac{1}{90}\cdot 632514+\frac{2}{45}\cdot 534126-\frac{1}{90}\cdot 642135+\frac{1}{90}\cdot 642153-\frac{1}{45}\cdot 643125$$
$$+\frac{1}{90}\cdot 135624+\frac{1}{90}\cdot 152634+\frac{2}{45}\cdot 156234+\frac{1}{90}\cdot 245136+\frac{1}{45}\cdot 246135+\frac{1}{30}\cdot 346152$$
$$+\frac{1}{45}\cdot 256134-\frac{1}{90}\cdot 251634-\frac{1}{45}\cdot 256341+\frac{1}{90}\cdot 415236+\frac{2}{45}\cdot 451236+\frac{2}{45}\cdot 451263$$
$$-\frac{1}{90}\cdot 461235+\frac{1}{30}\cdot 461253-\frac{1}{90}\cdot 315624+\frac{1}{45}\cdot 462315+\frac{1}{45}\cdot 534162-\frac{1}{45}\cdot 452361$$
$$-\frac{2}{45}\cdot 452613-\frac{1}{45}\cdot 452631-\frac{1}{45}\cdot 462351-\frac{1}{45}\cdot 462513+\frac{2}{45}\cdot 436512-\frac{1}{5}\cdot 456123$$
$$-\frac{4}{45}\cdot 465123-\frac{1}{45}\cdot 465132-\frac{1}{45}\cdot 351624-\frac{2}{45}\cdot 356124-\frac{2}{45}\cdot 451623-\frac{1}{45}\cdot 465213$$
$$+\frac{1}{45}\cdot 465231-\frac{1}{90}\cdot 352614-\frac{1}{45}\cdot 614523-\frac{1}{45}\cdot 562134+\frac{2}{45}\cdot 562143-\frac{2}{45}\cdot 536124$$
$$-\frac{1}{45}\cdot 536142-\frac{1}{45}\cdot 634125-\frac{1}{45}\cdot 634152-\frac{1}{45}\cdot 635124-\frac{2}{45}\cdot 562341-\frac{1}{90}\cdot 531624$$
$$-\frac{1}{45}\cdot 541623-\frac{4}{45}\cdot 546123-\frac{1}{45}\cdot 563124-\frac{2}{45}\cdot 564123-\frac{1}{45}\cdot 546132-\frac{2}{45}\cdot 645123$$
$$+\frac{1}{45}\cdot 645132-\frac{1}{90}\cdot 516234-\frac{1}{45}\cdot 526341-\frac{1}{45}\cdot 546213+\frac{1}{45}\cdot 546312-\frac{1}{45}\cdot 561243$$
$$-\frac{1}{45}\cdot 641523-\frac{1}{90}\cdot 461352-\frac{1}{45}\cdot 561342-\frac{1}{90}\cdot 364152+\frac{1}{45}\cdot 564213+\frac{1}{90}\cdot 146235$$
$$+\frac{1}{45}\cdot 162345+\frac{1}{45}\cdot 163245+\frac{1}{45}\cdot 162435+\frac{1}{90}\cdot 163425+\frac{1}{45}\cdot 261435+\frac{1}{90}\cdot 162534$$
$$+\frac{1}{90}\cdot 164235+\frac{1}{45}\cdot 165234+\frac{1}{90}\cdot 261534+\frac{1}{90}\cdot 264135+\frac{1}{45}\cdot 265134+\frac{1}{90}\cdot 351246$$
$$+\frac{1}{90}\cdot 351264+\frac{1}{45}\cdot 361254-\frac{1}{45}\cdot 362145-\frac{1}{90}\cdot 362415-\frac{1}{90}\cdot 362451+\frac{1}{90}\cdot 361524$$
$$+\frac{1}{45}\cdot 512346+\frac{1}{45}\cdot 512364+\frac{1}{45}\cdot 521346+\frac{1}{45}\cdot 521364+\frac{1}{45}\cdot 512634+\frac{1}{45}\cdot 521634$$

$$- \frac{1}{90} \cdot 526134 + \frac{1}{45} \cdot 513246 + \frac{1}{45} \cdot 513264 + \frac{1}{90} \cdot 523146 + \frac{1}{90} \cdot 523164 + \frac{1}{90} \cdot 514236$$
$$+ \frac{1}{90} \cdot 514263 + \frac{1}{90} \cdot 531246 + \frac{1}{90} \cdot 531264 + \frac{1}{45} \cdot 541236 + \frac{1}{45} \cdot 541263 - \frac{1}{90} \cdot 513642$$
$$- \frac{1}{90} \cdot 523461 - \frac{1}{90} \cdot 523641 - \frac{4}{45} \cdot 561234 - \frac{1}{90} \cdot 526314 + \frac{1}{45} \cdot 612435 + \frac{1}{45} \cdot 612534$$
$$+ \frac{1}{45} \cdot 621435 + \frac{1}{45} \cdot 621534 - \frac{1}{90} \cdot 615234 - \frac{1}{90} \cdot 625134 + \frac{1}{45} \cdot 613245 + \frac{1}{45} \cdot 613254$$
$$+ \frac{1}{45} \cdot 623145 + \frac{1}{45} \cdot 623154 - \frac{1}{30} \cdot 641235 - \frac{1}{90} \cdot 641253 - \frac{1}{30} \cdot 613542 - \frac{2}{45} \cdot 651234$$
$$- \frac{1}{45} \cdot 652134 - \frac{1}{45} \cdot 651243 - \frac{1}{45} \cdot 146532 - \frac{1}{90} \cdot 246531 - \frac{1}{45} \cdot 163542 - \frac{1}{45} \cdot 165243$$
$$- \frac{1}{9} \cdot 165432 - \frac{1}{45} \cdot 264531 - \frac{2}{45} \cdot 265431 - \frac{1}{45} \cdot 354216 - \frac{1}{90} \cdot 354261 - \frac{1}{45} \cdot 364215$$
$$- \frac{1}{90} \cdot 364251 - \frac{1}{45} \cdot 365214 + \frac{1}{45} \cdot 265143 + \frac{1}{45} \cdot 361542 + \frac{1}{90} \cdot 362541 + \frac{1}{45} \cdot 365142$$
$$+ \frac{2}{45} \cdot 365412 - \frac{1}{45} \cdot 364521 - \frac{1}{45} \cdot 524316 - \frac{1}{90} \cdot 524361 - \frac{1}{45} \cdot 541326 - \frac{1}{45} \cdot 541362$$
$$- \frac{1}{90} \cdot 524631 - \frac{1}{45} \cdot 541632 + \frac{1}{45} \cdot 416532 + \frac{1}{90} \cdot 426531 - \frac{1}{9} \cdot 543216 - \frac{1}{45} \cdot 534261$$
$$- \frac{2}{45} \cdot 543261 + \frac{2}{45} \cdot 543612 + \frac{1}{45} \cdot 546231 + \frac{2}{45} \cdot 563214 + \frac{2}{45} \cdot 563241 + \frac{2}{45} \cdot 564231$$
$$+ \frac{2}{45} \cdot 561432 + \frac{1}{45} \cdot 564132 + \frac{1}{45} \cdot 461532 + \frac{1}{45} \cdot 546321 + \frac{2}{45} \cdot 564312 + \frac{2}{45} \cdot 564321$$
$$+ \frac{2}{45} \cdot 563421 - \frac{2}{45} \cdot 615432 - \frac{1}{45} \cdot 624531 - \frac{1}{45} \cdot 625431 - \frac{2}{45} \cdot 643215 - \frac{1}{45} \cdot 653124$$
$$+ \frac{1}{45} \cdot 643251 + \frac{2}{45} \cdot 643512 + \frac{2}{45} \cdot 643521 + \frac{2}{45} \cdot 653412 + \frac{2}{45} \cdot 653421 + \frac{2}{45} \cdot 645321$$
$$+ \frac{2}{45} \cdot 645231 + \frac{1}{45} \cdot 654132 + \frac{2}{45} \cdot 654231 + \frac{2}{45} \cdot 653241 - \frac{1}{90} \cdot 615243 - \frac{1}{45} \cdot 615342$$
$$- \frac{1}{90} \cdot 624315 - \frac{1}{90} \cdot 625314 + \frac{1}{90} \cdot 625143 - \frac{1}{45} \cdot 625341 - \frac{1}{90} \cdot 641325 - \frac{1}{90} \cdot 641352$$
$$+ \frac{1}{90} \cdot 631542 - \frac{1}{45} \cdot 642315 - \frac{1}{45} \cdot 453621 + \frac{1}{45} \cdot 645213 + \frac{2}{45} \cdot 645312 + \frac{1}{45} \cdot 465312$$
$$+ \frac{1}{45} \cdot 465321 - \frac{1}{45} \cdot 651342 + \frac{2}{45} \cdot 654312 + \frac{1}{45} \cdot 654213$$

$$[\![y_2 \times y_4]\!] = -\frac{1}{45} \cdot 125463 - \frac{2}{45} \cdot 125643 - \frac{1}{45} \cdot 215463 - \frac{2}{45} \cdot 215643 - \frac{1}{45} \cdot 124653 - \frac{1}{45} \cdot 214653$$
$$- \frac{4}{45} \cdot 126543 - \frac{4}{45} \cdot 216543 - \frac{2}{45} \cdot 126453 - \frac{2}{45} \cdot 216453 - \frac{1}{45} \cdot 143526 - \frac{2}{45} \cdot 145326$$
$$- \frac{1}{45} \cdot 135426 - \frac{1}{90} \cdot 136425 - \frac{1}{90} \cdot 136524 - \frac{1}{90} \cdot 146325 - \frac{1}{90} \cdot 316425 - \frac{1}{90} \cdot 316524$$
$$- \frac{1}{45} \cdot 416325 + \frac{1}{45} \cdot 236541 + \frac{1}{45} \cdot 326541 - \frac{1}{90} \cdot 152463 - \frac{1}{90} \cdot 152643 - \frac{1}{90} \cdot 154263$$
$$- \frac{1}{90} \cdot 251463 - \frac{1}{90} \cdot 251643 - \frac{1}{45} \cdot 254163 + \frac{1}{45} \cdot 412653 + \frac{1}{45} \cdot 421653 + \frac{1}{45} \cdot 512643$$
$$+ \frac{1}{45} \cdot 521643 - \frac{4}{45} \cdot 154326 - \frac{2}{45} \cdot 153426 + \frac{1}{45} \cdot 254361 + \frac{1}{45} \cdot 153624 + \frac{1}{15} \cdot 154623$$
$$+ \frac{2}{45} \cdot 156324 + \frac{1}{15} \cdot 156423 + \frac{2}{45} \cdot 156243 + \frac{1}{90} \cdot 254613 + \frac{1}{15} \cdot 256143 + \frac{1}{45} \cdot 256413$$

$$
\begin{aligned}
&+\frac{1}{15}\cdot 146523+\frac{1}{15}\cdot 416523+\frac{1}{30}\cdot 516324+\frac{2}{45}\cdot 516423+\frac{1}{45}\cdot 146253+\frac{1}{30}\cdot 246153\\
&+\frac{1}{90}\cdot 246513+\frac{1}{90}\cdot 416253+\frac{2}{45}\cdot 426153+\frac{1}{30}\cdot 426513+\frac{1}{90}\cdot 516243+\frac{1}{18}\cdot 526143\\
&+\frac{1}{45}\cdot 526413-\frac{1}{30}\cdot 162543-\frac{1}{30}\cdot 261543-\frac{1}{45}\cdot 365142-\frac{1}{90}\cdot 162453-\frac{1}{90}\cdot 261453\\
&+\frac{1}{45}\cdot 612543+\frac{1}{45}\cdot 621543-\frac{1}{30}\cdot 164325-\frac{1}{45}\cdot 264315-\frac{1}{45}\cdot 265314-\frac{1}{90}\cdot 163425\\
&+\frac{1}{45}\cdot 614325+\frac{1}{90}\cdot 264351+\frac{1}{45}\cdot 265341+\frac{1}{90}\cdot 263541+\frac{1}{90}\cdot 362541+\frac{1}{15}\cdot 164523\\
&+\frac{2}{45}\cdot 165423+\frac{1}{45}\cdot 264513+\frac{1}{45}\cdot 265413+\frac{1}{90}\cdot 615324-\frac{1}{90}\cdot 615243+\frac{1}{90}\cdot 625143\\
&+\frac{2}{45}\cdot 134562+\frac{1}{45}\cdot 134652+\frac{1}{45}\cdot 314562+\frac{1}{45}\cdot 314652+\frac{1}{45}\cdot 143562+\frac{1}{45}\cdot 145632\\
&+\frac{1}{45}\cdot 415632+\frac{1}{45}\cdot 135462+\frac{1}{90}\cdot 135642+\frac{1}{90}\cdot 145362+\frac{1}{45}\cdot 315462+\frac{1}{90}\cdot 315642\\
&+\frac{1}{90}\cdot 415362+\frac{1}{90}\cdot 136452+\frac{1}{90}\cdot 153462+\frac{1}{45}\cdot 163452+\frac{1}{90}\cdot 316452+\frac{2}{45}\cdot 234516\\
&+\frac{1}{45}\cdot 235416+\frac{1}{45}\cdot 234615+\frac{1}{45}\cdot 324516+\frac{1}{45}\cdot 324615-\frac{1}{45}\cdot 236514+\frac{1}{45}\cdot 325614\\
&-\frac{1}{90}\cdot 245631-\frac{1}{90}\cdot 425631+\frac{1}{45}\cdot 341652-\frac{1}{45}\cdot 431562+\frac{1}{45}\cdot 345216+\frac{1}{45}\cdot 346215\\
&+\frac{1}{45}\cdot 243516+\frac{1}{45}\cdot 243615+\frac{1}{90}\cdot 245316+\frac{1}{90}\cdot 246315+\frac{1}{90}\cdot 342516+\frac{1}{90}\cdot 342615\\
&+\frac{1}{90}\cdot 253416+\frac{1}{90}\cdot 423516+\frac{1}{90}\cdot 423615+\frac{1}{45}\cdot 523416-\frac{1}{90}\cdot 345261-\frac{1}{90}\cdot 346251\\
&+\frac{1}{90}\cdot 245613-\frac{4}{45}\cdot 345612-\frac{2}{45}\cdot 346512-\frac{2}{45}\cdot 435612+\frac{1}{90}\cdot 345162+\frac{1}{90}\cdot 435162\\
&+\frac{1}{45}\cdot 451632-\frac{2}{45}\cdot 456132+\frac{1}{90}\cdot 351642-\frac{1}{45}\cdot 356142-\frac{1}{45}\cdot 361452-\frac{1}{45}\cdot 513462\\
&-\frac{1}{90}\cdot 531462-\frac{1}{30}\cdot 613452-\frac{1}{90}\cdot 631452+\frac{1}{45}\cdot 356214-\frac{2}{45}\cdot 456213+\frac{1}{90}\cdot 352614\\
&-\frac{1}{45}\cdot 452613-\frac{1}{45}\cdot 263415-\frac{1}{90}\cdot 263514-\frac{1}{45}\cdot 523614-\frac{1}{30}\cdot 623415-\frac{1}{90}\cdot 623514\\
&-\frac{1}{45}\cdot 356241-\frac{1}{45}\cdot 456231-\frac{1}{45}\cdot 452631-\frac{2}{45}\cdot 354612-\frac{1}{45}\cdot 356412-\frac{1}{45}\cdot 453612\\
&-\frac{1}{45}\cdot 456312+\frac{1}{90}\cdot 354162+\frac{1}{45}\cdot 453162-\frac{1}{45}\cdot 364512-\frac{1}{90}\cdot 524613-\frac{1}{45}\cdot 534612\\
&-\frac{1}{45}\cdot 624513-\frac{1}{45}\cdot 634512-\frac{1}{90}\cdot 364152+\frac{1}{45}\cdot 534162-\frac{1}{45}\cdot 634152-\frac{1}{45}\cdot 324156\\
&-\frac{1}{45}\cdot 324165-\frac{2}{45}\cdot 342156-\frac{2}{45}\cdot 342165-\frac{1}{45}\cdot 243156-\frac{1}{45}\cdot 243165+\frac{1}{45}\cdot 326145\\
&+\frac{1}{45}\cdot 326154+\frac{1}{45}\cdot 362145+\frac{1}{45}\cdot 362154-\frac{1}{90}\cdot 253146-\frac{1}{90}\cdot 253164-\frac{1}{90}\cdot 254136\\
&-\frac{1}{90}\cdot 352146-\frac{1}{90}\cdot 352164-\frac{1}{90}\cdot 413526-\frac{1}{90}\cdot 413625-\frac{1}{90}\cdot 415326-\frac{1}{90}\cdot 431526\\
&-\frac{1}{90}\cdot 431625-\frac{4}{45}\cdot 432156-\frac{4}{45}\cdot 432165-\frac{2}{45}\cdot 423156-\frac{2}{45}\cdot 423165+\frac{1}{45}\cdot 432561\\
&+\frac{1}{45}\cdot 432651+\frac{1}{45}\cdot 425136+\frac{1}{30}\cdot 425163+\frac{1}{90}\cdot 426135+\frac{1}{15}\cdot 435126+\frac{1}{15}\cdot 436125\\
&+\frac{1}{30}\cdot 436152+\frac{2}{45}\cdot 452136+\frac{1}{15}\cdot 452163+\frac{1}{15}\cdot 453126+\frac{1}{90}\cdot 462135+\frac{1}{18}\cdot 462153
\end{aligned}
$$

$$+ \frac{2}{45} \cdot 463125 + \frac{1}{45} \cdot 463152 + \frac{2}{45} \cdot 451326 + \frac{1}{30} \cdot 461325 + \frac{1}{15} \cdot 354126 + \frac{1}{45} \cdot 351426$$
$$- \frac{1}{30} \cdot 514326 - \frac{1}{45} \cdot 514362 - \frac{1}{45} \cdot 541362 - \frac{1}{90} \cdot 513426 - \frac{1}{30} \cdot 532146 - \frac{1}{30} \cdot 532164$$
$$- \frac{1}{45} \cdot 542613 - \frac{1}{90} \cdot 523146 - \frac{1}{90} \cdot 523164 + \frac{1}{45} \cdot 632145 + \frac{1}{45} \cdot 632154 + \frac{1}{90} \cdot 532461$$
$$+ \frac{1}{90} \cdot 532641 + \frac{1}{45} \cdot 542361 + \frac{1}{90} \cdot 524361 + \frac{1}{15} \cdot 534126 + \frac{2}{45} \cdot 543126 + \frac{1}{45} \cdot 543162$$
$$- \frac{1}{90} \cdot 642135 + \frac{1}{90} \cdot 642153 + \frac{1}{90} \cdot 641325 + \frac{1}{15} \cdot 145623 + \frac{1}{90} \cdot 135624 + \frac{1}{45} \cdot 156342$$
$$+ \frac{1}{15} \cdot 345126 + \frac{1}{90} \cdot 245136 + \frac{1}{45} \cdot 245163 + \frac{1}{45} \cdot 246135 + \frac{1}{45} \cdot 346125 + \frac{1}{90} \cdot 346152$$
$$- \frac{2}{45} \cdot 356124 - \frac{2}{45} \cdot 365124 + \frac{2}{45} \cdot 256134 - \frac{1}{45} \cdot 256341 + \frac{1}{45} \cdot 415623 - \frac{1}{90} \cdot 315624$$
$$+ \frac{1}{45} \cdot 452316 + \frac{1}{45} \cdot 462315 - \frac{1}{45} \cdot 452361 - \frac{1}{45} \cdot 462351 - \frac{1}{45} \cdot 462513 - \frac{1}{5} \cdot 456123$$
$$- \frac{2}{15} \cdot 465123 - \frac{1}{45} \cdot 465132 - \frac{1}{45} \cdot 351624 - \frac{2}{45} \cdot 451623 + \frac{1}{45} \cdot 516342 + \frac{2}{45} \cdot 561324$$
$$- \frac{1}{45} \cdot 614523 + \frac{4}{45} \cdot 562143 + \frac{1}{90} \cdot 526134 - \frac{1}{45} \cdot 536124 - \frac{1}{45} \cdot 536142 - \frac{1}{45} \cdot 634125$$
$$- \frac{1}{45} \cdot 635124 - \frac{1}{15} \cdot 562341 - \frac{1}{90} \cdot 526314 - \frac{1}{45} \cdot 526341 - \frac{2}{15} \cdot 546123 - \frac{1}{45} \cdot 546132$$
$$- \frac{1}{15} \cdot 564123 + \frac{1}{45} \cdot 564132 - \frac{1}{90} \cdot 531624 - \frac{2}{45} \cdot 541623 - \frac{1}{15} \cdot 645123 + \frac{1}{45} \cdot 645132$$
$$- \frac{1}{45} \cdot 641523 + \frac{1}{90} \cdot 145263 + \frac{1}{45} \cdot 415263 + \frac{1}{90} \cdot 425613 + \frac{1}{90} \cdot 341526 - \frac{1}{90} \cdot 341625$$
$$+ \frac{2}{45} \cdot 451263 - \frac{1}{45} \cdot 546213 + \frac{1}{90} \cdot 461253 - \frac{1}{45} \cdot 461523 - \frac{1}{90} \cdot 461352 - \frac{1}{90} \cdot 361524$$
$$- \frac{1}{45} \cdot 465213 + \frac{1}{45} \cdot 564213 + \frac{1}{45} \cdot 645213 + \frac{1}{90} \cdot 152634 + \frac{1}{45} \cdot 156234 + \frac{1}{90} \cdot 251634$$
$$+ \frac{1}{90} \cdot 146235 + \frac{1}{45} \cdot 162435 + \frac{1}{45} \cdot 261435 + \frac{1}{90} \cdot 162534 + \frac{1}{90} \cdot 164235 + \frac{1}{45} \cdot 165234$$
$$+ \frac{1}{90} \cdot 261534 + \frac{1}{90} \cdot 264135 + \frac{1}{45} \cdot 265134 + \frac{1}{90} \cdot 415236 + \frac{1}{45} \cdot 451236 + \frac{1}{90} \cdot 351246$$
$$+ \frac{1}{90} \cdot 351264 - \frac{1}{45} \cdot 416235 - \frac{1}{30} \cdot 461235 + \frac{1}{45} \cdot 361245 + \frac{1}{45} \cdot 361254 - \frac{1}{90} \cdot 263451$$
$$- \frac{1}{90} \cdot 362415 - \frac{1}{90} \cdot 362451 + \frac{1}{45} \cdot 512634 + \frac{1}{45} \cdot 521634 - \frac{1}{30} \cdot 516234 + \frac{1}{45} \cdot 513246$$
$$+ \frac{1}{45} \cdot 513264 + \frac{1}{90} \cdot 514236 + \frac{1}{90} \cdot 514263 + \frac{1}{90} \cdot 531246 + \frac{1}{90} \cdot 531264 + \frac{1}{45} \cdot 541236$$
$$+ \frac{1}{45} \cdot 541263 - \frac{1}{90} \cdot 513642 - \frac{1}{90} \cdot 523461 - \frac{1}{90} \cdot 523641 - \frac{4}{45} \cdot 561234 + \frac{2}{45} \cdot 612435$$
$$+ \frac{1}{45} \cdot 612453 + \frac{2}{45} \cdot 621435 + \frac{1}{45} \cdot 621453 + \frac{1}{45} \cdot 612534 + \frac{1}{45} \cdot 621534 - \frac{1}{30} \cdot 615234$$
$$- \frac{1}{90} \cdot 625134 + \frac{2}{45} \cdot 613245 + \frac{2}{45} \cdot 613254 + \frac{1}{45} \cdot 623145 + \frac{1}{45} \cdot 623154 + \frac{1}{45} \cdot 631245$$
$$+ \frac{1}{45} \cdot 631254 - \frac{1}{30} \cdot 641235 - \frac{1}{90} \cdot 641253 - \frac{1}{30} \cdot 613542 - \frac{2}{45} \cdot 623451 - \frac{1}{45} \cdot 623541$$
$$- \frac{1}{30} \cdot 632415 - \frac{1}{45} \cdot 632451 - \frac{4}{45} \cdot 651234 - \frac{2}{45} \cdot 651243 - \frac{2}{45} \cdot 652134 - \frac{1}{45} \cdot 154632$$
$$- \frac{2}{45} \cdot 156432 - \frac{1}{90} \cdot 254631 - \frac{1}{45} \cdot 256431 - \frac{1}{45} \cdot 146532 - \frac{1}{90} \cdot 246531 - \frac{1}{9} \cdot 165432$$

$$- \frac{2}{45} \cdot 164532 - \frac{1}{45} \cdot 264531 - \frac{1}{45} \cdot 265431 - \frac{1}{45} \cdot 435216 - \frac{1}{90} \cdot 435261 - \frac{2}{45} \cdot 453216$$
$$- \frac{1}{45} \cdot 453261 - \frac{1}{45} \cdot 354216 - \frac{1}{90} \cdot 354261 + \frac{1}{45} \cdot 436215 + \frac{1}{90} \cdot 436251 - \frac{1}{45} \cdot 364215$$
$$- \frac{1}{90} \cdot 364251 - \frac{1}{45} \cdot 365214 + \frac{2}{45} \cdot 365412 + \frac{1}{45} \cdot 365421 - \frac{1}{45} \cdot 514632 - \frac{1}{90} \cdot 524631$$
$$- \frac{1}{45} \cdot 541632 + \frac{1}{45} \cdot 416532 + \frac{1}{90} \cdot 426531 - \frac{1}{9} \cdot 543216 - \frac{2}{45} \cdot 534216 - \frac{1}{45} \cdot 534261$$
$$- \frac{1}{45} \cdot 543261 + \frac{2}{45} \cdot 543612 + \frac{1}{45} \cdot 543621 + \frac{1}{45} \cdot 536214 + \frac{1}{45} \cdot 546231 + \frac{2}{45} \cdot 563214$$
$$+ \frac{2}{45} \cdot 564231 + \frac{2}{45} \cdot 561432 + \frac{1}{45} \cdot 465231 + \frac{1}{45} \cdot 461532 - \frac{1}{15} \cdot 615432 - \frac{1}{45} \cdot 651423$$
$$- \frac{1}{45} \cdot 651432 - \frac{2}{45} \cdot 614532 - \frac{1}{45} \cdot 624531 - \frac{1}{15} \cdot 643215 - \frac{1}{45} \cdot 653124 - \frac{1}{45} \cdot 653214$$
$$- \frac{2}{45} \cdot 634215 - \frac{1}{45} \cdot 634251 + \frac{2}{45} \cdot 643512 + \frac{1}{45} \cdot 643521 + \frac{4}{45} \cdot 653412 + \frac{2}{45} \cdot 653421$$
$$+ \frac{2}{45} \cdot 635412 + \frac{1}{45} \cdot 635421 + \frac{2}{45} \cdot 645231 + \frac{2}{45} \cdot 654213 + \frac{4}{45} \cdot 654231 + \frac{2}{45} \cdot 654132$$
$$+ \frac{1}{45} \cdot 653241 + \frac{1}{45} \cdot 652431 - \frac{1}{90} \cdot 154362 - \frac{1}{90} \cdot 614352 - \frac{1}{90} \cdot 136542 - \frac{1}{45} \cdot 615342$$
$$- \frac{1}{90} \cdot 432516 - \frac{1}{90} \cdot 254316 - \frac{1}{90} \cdot 624315 + \frac{1}{90} \cdot 432615 + \frac{1}{90} \cdot 632514 - \frac{1}{90} \cdot 625314$$
$$- \frac{1}{90} \cdot 641352 + \frac{1}{90} \cdot 316542 + \frac{1}{90} \cdot 631542 - \frac{1}{45} \cdot 642315 + \frac{1}{45} \cdot 546312 + \frac{2}{45} \cdot 645312$$
$$+ \frac{1}{45} \cdot 465312 - \frac{1}{45} \cdot 651342 - \frac{1}{45} \cdot 652314 + \frac{4}{45} \cdot 654312 + \frac{2}{45} \cdot 564312$$

$$[\![y_2 \times y_5]\!] = -\frac{1}{45} \cdot 124653 - \frac{1}{45} \cdot 125643 - \frac{1}{45} \cdot 214653 - \frac{1}{45} \cdot 215643 + \frac{1}{45} \cdot 126435 + \frac{1}{45} \cdot 126534$$
$$+ \frac{1}{45} \cdot 216435 + \frac{1}{45} \cdot 216534 - \frac{1}{45} \cdot 135426 - \frac{1}{45} \cdot 145326 + \frac{1}{45} \cdot 316542 + \frac{1}{45} \cdot 361542$$
$$+ \frac{1}{45} \cdot 416532 + \frac{2}{45} \cdot 461532 + \frac{1}{45} \cdot 153246 + \frac{1}{45} \cdot 154236 + \frac{1}{45} \cdot 412653 + \frac{2}{45} \cdot 512643$$
$$+ \frac{1}{45} \cdot 521643 + \frac{1}{45} \cdot 153462 + \frac{1}{45} \cdot 154362 - \frac{1}{45} \cdot 156342 - \frac{2}{45} \cdot 156432 - \frac{1}{45} \cdot 146532$$
$$- \frac{1}{45} \cdot 162453 - \frac{1}{45} \cdot 162543 - \frac{1}{45} \cdot 261453 - \frac{1}{45} \cdot 261543 + \frac{1}{45} \cdot 164352 + \frac{1}{45} \cdot 165342$$
$$+ \frac{1}{45} \cdot 264351 + \frac{1}{45} \cdot 265341 - \frac{1}{45} \cdot 163542 - \frac{1}{45} \cdot 164532 - \frac{2}{45} \cdot 613542 - \frac{2}{45} \cdot 614532$$
$$+ \frac{1}{45} \cdot 164523 + \frac{2}{45} \cdot 165423 + \frac{1}{45} \cdot 265413 + \frac{1}{45} \cdot 165324 + \frac{1}{45} \cdot 615324 + \frac{1}{45} \cdot 615423$$
$$+ \frac{1}{45} \cdot 134562 + \frac{1}{45} \cdot 143562 - \frac{1}{45} \cdot 315624 - \frac{1}{45} \cdot 415623 + \frac{1}{45} \cdot 234516 + \frac{1}{45} \cdot 234615$$
$$+ \frac{1}{45} \cdot 324516 + \frac{1}{45} \cdot 324615 - \frac{1}{45} \cdot 235461 - \frac{1}{45} \cdot 236451 - \frac{1}{45} \cdot 325461 - \frac{1}{45} \cdot 326451$$
$$+ \frac{1}{45} \cdot 245163 + \frac{1}{45} \cdot 246153 + \frac{1}{45} \cdot 345162 + \frac{1}{45} \cdot 346152 - \frac{1}{45} \cdot 341562 - \frac{2}{45} \cdot 431562$$
$$- \frac{1}{45} \cdot 243561 - \frac{1}{45} \cdot 243651 - \frac{1}{45} \cdot 342561 - \frac{1}{45} \cdot 342651 + \frac{1}{45} \cdot 245631 + \frac{2}{45} \cdot 345621$$
$$+ \frac{1}{45} \cdot 346521 + \frac{1}{45} \cdot 435621 + \frac{1}{45} \cdot 351642 + \frac{1}{45} \cdot 356142 + \frac{2}{45} \cdot 451632 + \frac{2}{45} \cdot 456132$$

$$+\frac{1}{45}\cdot 356214+\frac{2}{45}\cdot 456213+\frac{1}{45}\cdot 523461+\frac{2}{45}\cdot 532461+\frac{1}{45}\cdot 632451-\frac{1}{45}\cdot 354162$$
$$-\frac{2}{45}\cdot 354612-\frac{1}{45}\cdot 453162-\frac{1}{45}\cdot 453612-\frac{1}{45}\cdot 364512-\frac{1}{45}\cdot 243156-\frac{1}{45}\cdot 243165$$
$$-\frac{1}{45}\cdot 342156-\frac{1}{45}\cdot 342165+\frac{1}{45}\cdot 421356+\frac{1}{45}\cdot 421365+\frac{1}{45}\cdot 431256+\frac{1}{45}\cdot 431265$$
$$-\frac{1}{45}\cdot 421563-\frac{1}{45}\cdot 431652+\frac{1}{45}\cdot 423516+\frac{1}{45}\cdot 423615+\frac{1}{45}\cdot 432516+\frac{1}{45}\cdot 432615$$
$$-\frac{1}{45}\cdot 452316-\frac{2}{45}\cdot 453216-\frac{1}{45}\cdot 463215-\frac{1}{45}\cdot 354216-\frac{1}{45}\cdot 354261-\frac{1}{45}\cdot 453261$$
$$-\frac{1}{45}\cdot 513426-\frac{1}{45}\cdot 514326-\frac{1}{45}\cdot 532164-\frac{1}{45}\cdot 532614-\frac{1}{45}\cdot 542163-\frac{2}{45}\cdot 542613$$
$$+\frac{1}{45}\cdot 532416+\frac{1}{45}\cdot 542316+\frac{2}{45}\cdot 542361-\frac{1}{45}\cdot 524316-\frac{1}{45}\cdot 534216-\frac{1}{45}\cdot 624315$$
$$-\frac{1}{45}\cdot 634215+\frac{1}{45}\cdot 534126+\frac{2}{45}\cdot 543126+\frac{1}{45}\cdot 542136-\frac{1}{45}\cdot 156234-\frac{1}{45}\cdot 156243$$
$$-\frac{1}{45}\cdot 451236-\frac{1}{45}\cdot 451326-\frac{1}{45}\cdot 461235+\frac{1}{45}\cdot 461523-\frac{1}{45}\cdot 425613-\frac{1}{45}\cdot 426513$$
$$-\frac{1}{45}\cdot 435612-\frac{2}{45}\cdot 436512+\frac{1}{45}\cdot 456312+\frac{1}{45}\cdot 516324+\frac{1}{45}\cdot 516423+\frac{2}{45}\cdot 561324$$
$$+\frac{1}{45}\cdot 561423+\frac{1}{45}\cdot 562134+\frac{2}{45}\cdot 562143-\frac{1}{45}\cdot 562341-\frac{2}{45}\cdot 562431-\frac{1}{45}\cdot 531624$$
$$-\frac{1}{45}\cdot 536124-\frac{2}{45}\cdot 541623-\frac{2}{45}\cdot 546123-\frac{1}{45}\cdot 645123+\frac{1}{45}\cdot 145623+\frac{1}{45}\cdot 154623$$
$$+\frac{1}{45}\cdot 245613-\frac{1}{45}\cdot 416235-\frac{1}{45}\cdot 426135-\frac{1}{45}\cdot 516234-\frac{1}{45}\cdot 526134+\frac{1}{45}\cdot 345126$$
$$+\frac{1}{45}\cdot 435126-\frac{1}{45}\cdot 346512+\frac{1}{45}\cdot 351264+\frac{1}{45}\cdot 451263-\frac{1}{45}\cdot 452613+\frac{1}{45}\cdot 456231$$
$$+\frac{1}{45}\cdot 461253+\frac{1}{45}\cdot 462153+\frac{1}{45}\cdot 561243+\frac{1}{45}\cdot 562314+\frac{1}{45}\cdot 634512+\frac{2}{45}\cdot 643512$$
$$-\frac{2}{45}\cdot 465123-\frac{1}{45}\cdot 564123-\frac{1}{45}\cdot 365124-\frac{1}{45}\cdot 162345-\frac{1}{45}\cdot 162354-\frac{1}{45}\cdot 261345$$
$$-\frac{1}{45}\cdot 261354-\frac{1}{45}\cdot 512346-\frac{1}{45}\cdot 512436+\frac{1}{45}\cdot 512634+\frac{1}{45}\cdot 612435+\frac{1}{45}\cdot 612534$$
$$+\frac{1}{45}\cdot 621435+\frac{1}{45}\cdot 621534+\frac{1}{45}\cdot 613245+\frac{1}{45}\cdot 613254+\frac{1}{45}\cdot 623145+\frac{1}{45}\cdot 623154$$
$$-\frac{1}{45}\cdot 613452-\frac{1}{45}\cdot 623541-\frac{1}{45}\cdot 641235-\frac{2}{45}\cdot 651234-\frac{1}{45}\cdot 652134-\frac{1}{45}\cdot 651243$$
$$+\frac{1}{45}\cdot 534621+\frac{1}{45}\cdot 543621-\frac{2}{45}\cdot 563421-\frac{2}{45}\cdot 564321-\frac{1}{45}\cdot 465321-\frac{1}{45}\cdot 615432$$
$$-\frac{1}{45}\cdot 624531-\frac{1}{45}\cdot 625431-\frac{1}{45}\cdot 643215-\frac{1}{45}\cdot 653124-\frac{1}{45}\cdot 653214+\frac{1}{45}\cdot 643521$$
$$+\frac{2}{45}\cdot 653412-\frac{1}{45}\cdot 635421-\frac{2}{45}\cdot 645321+\frac{1}{45}\cdot 654132+\frac{2}{45}\cdot 654231+\frac{1}{45}\cdot 653241$$
$$+\frac{1}{45}\cdot 265431+\frac{1}{45}\cdot 356421+\frac{1}{45}\cdot 365421+\frac{1}{45}\cdot 543261+\frac{1}{45}\cdot 642351+\frac{1}{45}\cdot 643251$$
$$-\frac{1}{45}\cdot 546321-\frac{1}{45}\cdot 651342-\frac{1}{45}\cdot 651432-\frac{1}{45}\cdot 652431+\frac{2}{45}\cdot 654312+\frac{1}{45}\cdot 654213$$

$$[\![y_3\times y_3]\!]=\frac{2}{45}\cdot 124563+\frac{2}{45}\cdot 125463+\frac{2}{45}\cdot 214563+\frac{2}{45}\cdot 215463+\frac{2}{45}\cdot 125634+\frac{2}{45}\cdot 215634$$

$$+\frac{4}{45}\cdot 351624+\frac{2}{15}\cdot 125643+\frac{2}{15}\cdot 215643+\frac{1}{15}\cdot 351642+\frac{4}{45}\cdot 124653+\frac{4}{45}\cdot 214653$$
$$+\frac{2}{15}\cdot 126453+\frac{2}{15}\cdot 216453+\frac{2}{45}\cdot 134526+\frac{2}{45}\cdot 143526+\frac{2}{45}\cdot 134625+\frac{2}{45}\cdot 143625$$
$$+\frac{1}{15}\cdot 315624-\frac{1}{15}\cdot 153624-\frac{2}{45}\cdot 235614-\frac{2}{45}\cdot 325614-\frac{2}{45}\cdot 153642-\frac{2}{45}\cdot 235641$$
$$-\frac{2}{45}\cdot 325641+\frac{2}{45}\cdot 134652+\frac{2}{45}\cdot 143652+\frac{2}{45}\cdot 315642+\frac{2}{45}\cdot 145236-\frac{1}{45}\cdot 145263$$
$$-\frac{2}{45}\cdot 245163+\frac{1}{45}\cdot 154263+\frac{2}{45}\cdot 254163+\frac{2}{15}\cdot 145326+\frac{4}{45}\cdot 135426+\frac{2}{15}\cdot 153426$$
$$-\frac{2}{45}\cdot 245361+\frac{1}{45}\cdot 135462+\frac{1}{45}\cdot 153462-\frac{1}{45}\cdot 135624-\frac{2}{15}\cdot 145623-\frac{1}{15}\cdot 245613$$
$$-\frac{1}{5}\cdot 154623-\frac{2}{45}\cdot 513624-\frac{1}{9}\cdot 254613-\frac{1}{15}\cdot 145632-\frac{1}{45}\cdot 245631-\frac{4}{45}\cdot 154632$$
$$-\frac{1}{15}\cdot 513642-\frac{1}{15}\cdot 146253-\frac{7}{45}\cdot 156243-\frac{4}{45}\cdot 246153-\frac{7}{45}\cdot 256143-\frac{2}{45}\cdot 164253$$
$$+\frac{1}{45}\cdot 146325-\frac{2}{45}\cdot 613425-\frac{2}{9}\cdot 156342-\frac{2}{45}\cdot 246351+\frac{1}{45}\cdot 136452-\frac{2}{45}\cdot 163452$$
$$-\frac{1}{45}\cdot 613452-\frac{7}{45}\cdot 146523-\frac{2}{9}\cdot 156423-\frac{4}{45}\cdot 246513-\frac{1}{9}\cdot 256413-\frac{2}{9}\cdot 164523$$
$$-\frac{2}{45}\cdot 613524+\frac{2}{45}\cdot 126345+\frac{2}{45}\cdot 126435+\frac{2}{45}\cdot 216345+\frac{2}{45}\cdot 216435+\frac{4}{45}\cdot 126354$$
$$+\frac{4}{45}\cdot 216354+\frac{2}{15}\cdot 126534+\frac{2}{15}\cdot 216534+\frac{1}{15}\cdot 361524-\frac{1}{45}\cdot 146235-\frac{2}{45}\cdot 416235$$
$$+\frac{2}{45}\cdot 416325-\frac{2}{45}\cdot 146352-\frac{4}{45}\cdot 416253-\frac{7}{45}\cdot 416523+\frac{2}{45}\cdot 152346+\frac{2}{45}\cdot 153246$$
$$+\frac{2}{45}\cdot 152364+\frac{2}{45}\cdot 153264+\frac{1}{15}\cdot 251634-\frac{2}{45}\cdot 512634-\frac{2}{45}\cdot 521634+\frac{4}{45}\cdot 152436$$
$$+\frac{2}{15}\cdot 154236-\frac{2}{45}\cdot 253461-\frac{1}{45}\cdot 152634-\frac{2}{15}\cdot 156234-\frac{1}{5}\cdot 156324-\frac{2}{45}\cdot 253614$$
$$-\frac{1}{15}\cdot 516234-\frac{1}{9}\cdot 516324-\frac{2}{45}\cdot 253641-\frac{4}{45}\cdot 516243-\frac{1}{9}\cdot 516423+\frac{2}{45}\cdot 162354$$
$$+\frac{2}{45}\cdot 163254+\frac{2}{45}\cdot 261534-\frac{2}{45}\cdot 163524-\frac{2}{45}\cdot 612534-\frac{2}{45}\cdot 621534+\frac{1}{45}\cdot 162435$$
$$+\frac{1}{45}\cdot 163425-\frac{2}{45}\cdot 614235+\frac{1}{45}\cdot 162453-\frac{1}{45}\cdot 263451-\frac{2}{45}\cdot 614253-\frac{1}{15}\cdot 165234$$
$$-\frac{4}{45}\cdot 165324-\frac{1}{15}\cdot 263514-\frac{1}{45}\cdot 615234+\frac{4}{15}\cdot 126543+\frac{4}{15}\cdot 216543+\frac{2}{45}\cdot 361542$$
$$-\frac{2}{45}\cdot 236154-\frac{2}{45}\cdot 326154-\frac{2}{45}\cdot 146532-\frac{4}{45}\cdot 236514-\frac{4}{45}\cdot 236541-\frac{4}{45}\cdot 326514$$
$$-\frac{4}{45}\cdot 326541-\frac{4}{45}\cdot 416532+\frac{1}{15}\cdot 251463+\frac{1}{15}\cdot 251643-\frac{4}{45}\cdot 512643-\frac{4}{45}\cdot 521643$$
$$+\frac{4}{15}\cdot 154326+\frac{2}{45}\cdot 514362-\frac{1}{9}\cdot 254361+\frac{2}{45}\cdot 514632-\frac{4}{45}\cdot 516342-\frac{4}{45}\cdot 526143$$
$$-\frac{2}{15}\cdot 156432-\frac{4}{45}\cdot 516432+\frac{1}{15}\cdot 162543+\frac{1}{15}\cdot 261543-\frac{4}{45}\cdot 612543-\frac{4}{45}\cdot 621543$$
$$+\frac{2}{45}\cdot 164235+\frac{1}{15}\cdot 164325-\frac{4}{45}\cdot 164352-\frac{1}{9}\cdot 614325-\frac{2}{15}\cdot 164532-\frac{4}{45}\cdot 264351$$
$$-\frac{2}{45}\cdot 165243-\frac{2}{15}\cdot 165342-\frac{4}{45}\cdot 265143-\frac{2}{45}\cdot 615324+\frac{1}{45}\cdot 136425+\frac{1}{45}\cdot 136524$$
$$+\frac{1}{15}\cdot 316425+\frac{1}{15}\cdot 316524+\frac{1}{15}\cdot 136542+\frac{1}{15}\cdot 316452+\frac{1}{15}\cdot 316542+\frac{1}{45}\cdot 152463$$

$$+\frac{1}{45}\cdot 152643-\frac{2}{45}\cdot 412653-\frac{2}{45}\cdot 421653+\frac{1}{15}\cdot 154362-\frac{4}{45}\cdot 426153-\frac{4}{45}\cdot 426513$$
$$-\frac{1}{15}\cdot 526413-\frac{2}{45}\cdot 254631-\frac{2}{45}\cdot 256431+\frac{1}{15}\cdot 261453+\frac{2}{45}\cdot 264315+\frac{2}{45}\cdot 265314$$
$$-\frac{4}{45}\cdot 614352-\frac{2}{15}\cdot 165423-\frac{4}{45}\cdot 264513-\frac{4}{45}\cdot 265413-\frac{2}{45}\cdot 615423+\frac{2}{45}\cdot 145362$$
$$+\frac{2}{45}\cdot 234156+\frac{2}{45}\cdot 234165+\frac{2}{45}\cdot 324156+\frac{2}{45}\cdot 324165+\frac{2}{45}\cdot 235146+\frac{2}{45}\cdot 235164$$
$$+\frac{2}{45}\cdot 325146+\frac{2}{45}\cdot 325164-\frac{1}{15}\cdot 425136-\frac{2}{45}\cdot 425316+\frac{2}{45}\cdot 235416+\frac{2}{45}\cdot 325416$$
$$+\frac{2}{45}\cdot 341256+\frac{2}{45}\cdot 341265-\frac{1}{45}\cdot 341526-\frac{1}{45}\cdot 341625+\frac{1}{45}\cdot 431526+\frac{2}{15}\cdot 342156$$
$$+\frac{2}{15}\cdot 342165+\frac{4}{45}\cdot 243156+\frac{4}{45}\cdot 243165+\frac{2}{15}\cdot 423156+\frac{2}{15}\cdot 423165+\frac{1}{45}\cdot 243516$$
$$+\frac{1}{45}\cdot 243615+\frac{1}{45}\cdot 423516+\frac{1}{45}\cdot 423615+\frac{4}{45}\cdot 523614-\frac{1}{45}\cdot 245136-\frac{2}{45}\cdot 246135$$
$$-\frac{2}{15}\cdot 345126-\frac{1}{15}\cdot 345162-\frac{4}{45}\cdot 346125-\frac{1}{15}\cdot 346152-\frac{1}{5}\cdot 435126-\frac{4}{45}\cdot 435162$$
$$-\frac{1}{15}\cdot 345216-\frac{1}{45}\cdot 345261-\frac{1}{45}\cdot 346215-\frac{1}{45}\cdot 346251-\frac{4}{45}\cdot 435216-\frac{1}{15}\cdot 351426$$
$$-\frac{7}{45}\cdot 451326-\frac{2}{45}\cdot 531426+\frac{1}{45}\cdot 352146+\frac{1}{45}\cdot 352164+\frac{4}{45}\cdot 452613-\frac{2}{45}\cdot 263145$$
$$-\frac{2}{45}\cdot 263154-\frac{2}{45}\cdot 623145-\frac{2}{45}\cdot 623154-\frac{2}{45}\cdot 352461-\frac{2}{45}\cdot 352641-\frac{2}{9}\cdot 452316$$
$$+\frac{1}{45}\cdot 253416-\frac{2}{45}\cdot 523416-\frac{1}{45}\cdot 623415+\frac{1}{45}\cdot 623514-\frac{7}{45}\cdot 354126-\frac{2}{9}\cdot 453126$$
$$-\frac{1}{15}\cdot 354162-\frac{2}{9}\cdot 534126-\frac{2}{15}\cdot 534162-\frac{2}{45}\cdot 624135-\frac{2}{45}\cdot 624153-\frac{2}{45}\cdot 426135$$
$$-\frac{2}{45}\cdot 426315-\frac{1}{45}\cdot 351246-\frac{1}{45}\cdot 351264+\frac{1}{45}\cdot 431625+\frac{1}{45}\cdot 253146+\frac{1}{45}\cdot 253164$$
$$+\frac{1}{45}\cdot 254136-\frac{1}{45}\cdot 524613-\frac{2}{45}\cdot 256134-\frac{7}{45}\cdot 436125-\frac{4}{45}\cdot 436152-\frac{1}{45}\cdot 526134$$
$$+\frac{4}{45}\cdot 356214+\frac{2}{45}\cdot 356241-\frac{2}{45}\cdot 436215-\frac{1}{45}\cdot 526314-\frac{1}{15}\cdot 461325-\frac{2}{45}\cdot 362154$$
$$+\frac{4}{45}\cdot 462513-\frac{1}{15}\cdot 362451-\frac{1}{9}\cdot 362541-\frac{2}{15}\cdot 462315-\frac{2}{45}\cdot 364125+\frac{2}{45}\cdot 365124$$
$$-\frac{1}{9}\cdot 463125-\frac{1}{45}\cdot 265134-\frac{1}{45}\cdot 625134-\frac{1}{15}\cdot 625143-\frac{1}{15}\cdot 436251+\frac{2}{15}\cdot 532614$$
$$-\frac{2}{45}\cdot 352416-\frac{2}{45}\cdot 524136-\frac{2}{45}\cdot 524163+\frac{4}{45}\cdot 356124+\frac{4}{45}\cdot 536124+\frac{1}{15}\cdot 536214$$
$$+\frac{2}{45}\cdot 356142-\frac{2}{45}\cdot 361254-\frac{1}{45}\cdot 632514-\frac{1}{45}\cdot 261435-\frac{1}{15}\cdot 362415+\frac{4}{45}\cdot 361452$$
$$+\frac{4}{45}\cdot 365214-\frac{2}{45}\cdot 346512-\frac{4}{45}\cdot 436512-\frac{1}{45}\cdot 246531-\frac{1}{15}\cdot 426531+\frac{1}{45}\cdot 523641$$
$$-\frac{1}{45}\cdot 532641-\frac{2}{45}\cdot 354216-\frac{2}{45}\cdot 354612+\frac{4}{45}\cdot 536142+\frac{1}{45}\cdot 536241+\frac{1}{45}\cdot 356421$$
$$-\frac{2}{45}\cdot 526431-\frac{1}{45}\cdot 263541+\frac{2}{45}\cdot 623541+\frac{2}{45}\cdot 364512+\frac{1}{15}\cdot 364521+\frac{1}{45}\cdot 624531$$
$$+\frac{1}{45}\cdot 365142+\frac{1}{45}\cdot 625341-\frac{2}{45}\cdot 341652-\frac{2}{45}\cdot 431652+\frac{1}{15}\cdot 254316-\frac{2}{45}\cdot 354261$$
$$+\frac{8}{45}\cdot 465132-\frac{1}{45}\cdot 613542-\frac{1}{9}\cdot 631542+\frac{8}{45}\cdot 465213+\frac{1}{15}\cdot 465231-\frac{1}{45}\cdot 264531$$

$$- \frac{1}{15} \cdot 365412 - \frac{1}{15} \cdot 463152 - \frac{2}{45} \cdot 625413 + \frac{1}{9} \cdot 635412 + \frac{2}{45} \cdot 412356 + \frac{2}{45} \cdot 412365$$
$$+ \frac{2}{45} \cdot 421356 + \frac{2}{45} \cdot 421365 + \frac{2}{45} \cdot 412536 + \frac{2}{45} \cdot 412635 + \frac{2}{45} \cdot 421536 + \frac{2}{45} \cdot 421635$$
$$+ \frac{4}{45} \cdot 413256 + \frac{4}{45} \cdot 413265 + \frac{2}{15} \cdot 431256 + \frac{2}{15} \cdot 431265 - \frac{2}{45} \cdot 413562 - \frac{2}{45} \cdot 413652$$
$$- \frac{2}{45} \cdot 423561 - \frac{2}{45} \cdot 423651 - \frac{1}{45} \cdot 415236 - \frac{2}{45} \cdot 415263 - \frac{2}{15} \cdot 451236 - \frac{4}{45} \cdot 451263$$
$$- \frac{1}{15} \cdot 461235 - \frac{1}{15} \cdot 461253 - \frac{1}{5} \cdot 452136 - \frac{4}{45} \cdot 462135 - \frac{2}{45} \cdot 425361 - \frac{2}{45} \cdot 426351$$
$$+ \frac{2}{45} \cdot 512436 + \frac{2}{45} \cdot 521436 + \frac{1}{45} \cdot 513246 + \frac{1}{45} \cdot 513264 + \frac{1}{45} \cdot 523146 + \frac{1}{45} \cdot 523164$$
$$+ \frac{1}{45} \cdot 513426 - \frac{1}{45} \cdot 523461 - \frac{2}{45} \cdot 631425 - \frac{2}{45} \cdot 631524 - \frac{1}{15} \cdot 541236 - \frac{4}{45} \cdot 542136$$
$$- \frac{1}{45} \cdot 541263 - \frac{1}{45} \cdot 641235 - \frac{1}{45} \cdot 641253 - \frac{2}{45} \cdot 425163 + \frac{1}{45} \cdot 413526 + \frac{1}{45} \cdot 413625$$
$$+ \frac{1}{45} \cdot 415326 - \frac{2}{45} \cdot 415623 - \frac{1}{45} \cdot 425613 - \frac{7}{45} \cdot 452163 - \frac{4}{45} \cdot 462153 - \frac{1}{45} \cdot 415632$$
$$- \frac{1}{45} \cdot 425631 - \frac{2}{45} \cdot 451362 + \frac{2}{45} \cdot 451632 - \frac{1}{9} \cdot 453162 - \frac{1}{15} \cdot 631452 - \frac{2}{45} \cdot 542163$$
$$+ \frac{4}{45} \cdot 541623 + \frac{2}{45} \cdot 641523 - \frac{1}{45} \cdot 315462 - \frac{1}{15} \cdot 531462 + \frac{4}{45} \cdot 451623 + \frac{1}{15} \cdot 542613$$
$$+ \frac{4}{45} \cdot 541632 - \frac{1}{15} \cdot 642153 + \frac{2}{45} \cdot 461523 + \frac{4}{15} \cdot 432156 + \frac{4}{15} \cdot 432165 - \frac{4}{45} \cdot 432561$$
$$- \frac{4}{45} \cdot 432651 - \frac{2}{15} \cdot 453216 - \frac{4}{45} \cdot 463215 + \frac{1}{15} \cdot 514326 + \frac{2}{45} \cdot 531246 + \frac{2}{45} \cdot 531264$$
$$+ \frac{1}{15} \cdot 532146 + \frac{1}{15} \cdot 532164 - \frac{4}{45} \cdot 532416 - \frac{4}{45} \cdot 632145 - \frac{4}{45} \cdot 632154 - \frac{2}{45} \cdot 531642$$
$$- \frac{1}{15} \cdot 532461 - \frac{2}{15} \cdot 534216 - \frac{2}{45} \cdot 541326 - \frac{2}{15} \cdot 542316 - \frac{1}{15} \cdot 642135 + \frac{1}{15} \cdot 432516$$
$$+ \frac{1}{15} \cdot 432615 - \frac{1}{15} \cdot 435261 - \frac{2}{45} \cdot 542361 - \frac{2}{45} \cdot 542631 - \frac{1}{15} \cdot 632415 - \frac{2}{45} \cdot 634215$$
$$- \frac{2}{45} \cdot 635214 - \frac{2}{15} \cdot 543126 - \frac{4}{45} \cdot 543162 + \frac{2}{45} \cdot 342516 + \frac{2}{45} \cdot 342615 - \frac{2}{45} \cdot 362514$$
$$- \frac{2}{45} \cdot 435612 + \frac{2}{45} \cdot 462351 + \frac{1}{45} \cdot 462531 + \frac{2}{45} \cdot 453612 + \frac{1}{15} \cdot 453621 + \frac{2}{45} \cdot 463512$$
$$+ \frac{2}{45} \cdot 463521 - \frac{2}{45} \cdot 632451 + \frac{1}{45} \cdot 534621 + \frac{2}{45} \cdot 536412 + \frac{2}{45} \cdot 536421 + \frac{1}{15} \cdot 634251$$
$$+ \frac{2}{45} \cdot 635241 + \frac{1}{15} \cdot 642351 + \frac{2}{45} \cdot 642531 - \frac{1}{45} \cdot 534261 + \frac{8}{45} \cdot 546132 + \frac{8}{45} \cdot 546213$$
$$- \frac{1}{15} \cdot 543612 + \frac{1}{15} \cdot 546312 + \frac{2}{5} \cdot 456123 + \frac{4}{15} \cdot 456132 + \frac{4}{15} \cdot 465123 + \frac{4}{15} \cdot 456213$$
$$+ \frac{8}{45} \cdot 456231 + \frac{1}{45} \cdot 352614 + \frac{8}{45} \cdot 456312 - \frac{2}{45} \cdot 561324 - \frac{2}{45} \cdot 562134 - \frac{4}{45} \cdot 562143$$
$$+ \frac{2}{45} \cdot 634152 + \frac{1}{45} \cdot 635142 + \frac{8}{45} \cdot 562341 + \frac{1}{9} \cdot 562431 + \frac{8}{45} \cdot 634512 + \frac{1}{45} \cdot 531624$$
$$+ \frac{4}{15} \cdot 546123 + \frac{2}{45} \cdot 563124 + \frac{8}{45} \cdot 564123 + \frac{8}{45} \cdot 645123 + \frac{1}{15} \cdot 645132 - \frac{2}{45} \cdot 561243$$
$$+ \frac{2}{45} \cdot 561342 + \frac{1}{15} \cdot 564213 + \frac{1}{45} \cdot 642513 + \frac{1}{45} \cdot 461352 + \frac{1}{45} \cdot 364152 + \frac{1}{9} \cdot 456321$$
$$+ \frac{1}{15} \cdot 465312 + \frac{2}{45} \cdot 465321 - \frac{1}{15} \cdot 561432 - \frac{1}{15} \cdot 563214 + \frac{2}{15} \cdot 563412 + \frac{2}{45} \cdot 563421$$

$$
\begin{aligned}
&+\frac{1}{9}\cdot 634521+\frac{4}{45}\cdot 635421+\frac{1}{15}\cdot 546231+\frac{1}{15}\cdot 564132+\frac{2}{45}\cdot 564231+\frac{2}{45}\cdot 645231\\
&+\frac{2}{45}\cdot 546321+\frac{1}{45}\cdot 461532+\frac{1}{45}\cdot 563241+\frac{2}{45}\cdot 564312+\frac{1}{15}\cdot 645213+\frac{2}{45}\cdot 645312\\
&-\frac{1}{45}\cdot 615243-\frac{2}{45}\cdot 641325-\frac{1}{45}\cdot 615342+\frac{1}{45}\cdot 651423+\frac{1}{15}\cdot 651342-\frac{1}{45}\cdot 642315\\
&+\frac{1}{45}\cdot 652314+\frac{2}{45}\cdot 562413+\frac{2}{45}\cdot 652413+\frac{2}{45}\cdot 563142+\frac{1}{15}\cdot 653124+\frac{2}{45}\cdot 653142\\
&+\frac{1}{9}\cdot 652341+\frac{4}{45}\cdot 652431+\frac{1}{45}\cdot 643512+\frac{2}{45}\cdot 653412+\frac{1}{9}\cdot 654123+\frac{2}{45}\cdot 654213\\
&+\frac{2}{45}\cdot 654132
\end{aligned}
$$

$$
\begin{aligned}
[\![y_3\times y_4]\!]=&\frac{1}{15}\cdot 124563+\frac{1}{15}\cdot 214563+\frac{4}{45}\cdot 125463+\frac{4}{45}\cdot 215463+\frac{8}{45}\cdot 125643+\frac{8}{45}\cdot 215643\\
&+\frac{1}{30}\cdot 351642+\frac{4}{45}\cdot 124653+\frac{4}{45}\cdot 214653+\frac{2}{15}\cdot 126453+\frac{2}{15}\cdot 216453+\frac{1}{15}\cdot 134526\\
&+\frac{4}{45}\cdot 143526+\frac{2}{45}\cdot 134625+\frac{2}{45}\cdot 143625+\frac{1}{18}\cdot 315624-\frac{1}{45}\cdot 153642-\frac{1}{15}\cdot 235641\\
&-\frac{1}{15}\cdot 325641-\frac{1}{30}\cdot 145263-\frac{2}{45}\cdot 245163-\frac{1}{90}\cdot 154263+\frac{2}{45}\cdot 254163-\frac{1}{45}\cdot 412563\\
&-\frac{1}{45}\cdot 421563+\frac{8}{45}\cdot 145326+\frac{4}{45}\cdot 135426+\frac{2}{15}\cdot 153426-\frac{1}{15}\cdot 245361-\frac{1}{90}\cdot 135624\\
&-\frac{1}{5}\cdot 145623-\frac{1}{10}\cdot 245613-\frac{11}{45}\cdot 154623-\frac{2}{45}\cdot 513624-\frac{1}{10}\cdot 254613-\frac{4}{45}\cdot 156243\\
&-\frac{8}{45}\cdot 256143+\frac{1}{15}\cdot 356142-\frac{1}{15}\cdot 146253-\frac{1}{45}\cdot 164253-\frac{7}{90}\cdot 246153-\frac{1}{45}\cdot 612453\\
&-\frac{1}{45}\cdot 621453+\frac{7}{90}\cdot 146325+\frac{2}{45}\cdot 256314+\frac{1}{30}\cdot 136425-\frac{2}{15}\cdot 156324-\frac{2}{45}\cdot 613425\\
&-\frac{8}{45}\cdot 156342-\frac{2}{45}\cdot 246351+\frac{2}{45}\cdot 256341+\frac{2}{45}\cdot 356241+\frac{1}{90}\cdot 136524-\frac{11}{45}\cdot 146523\\
&-\frac{2}{9}\cdot 156423-\frac{1}{10}\cdot 246513-\frac{2}{15}\cdot 256413-\frac{4}{15}\cdot 164523-\frac{2}{45}\cdot 613524-\frac{2}{15}\cdot 264513\\
&-\frac{2}{45}\cdot 614523+\frac{1}{45}\cdot 125364+\frac{2}{45}\cdot 125634+\frac{1}{45}\cdot 215364+\frac{2}{45}\cdot 215634+\frac{1}{15}\cdot 351624\\
&+\frac{2}{45}\cdot 126354+\frac{2}{45}\cdot 216354+\frac{4}{45}\cdot 126534+\frac{4}{45}\cdot 216534+\frac{1}{18}\cdot 361524+\frac{1}{45}\cdot 142536\\
&+\frac{2}{45}\cdot 145236+\frac{1}{90}\cdot 146235-\frac{2}{45}\cdot 146352-\frac{1}{45}\cdot 236451-\frac{1}{45}\cdot 326451-\frac{7}{90}\cdot 416253\\
&+\frac{1}{45}\cdot 416352+\frac{1}{45}\cdot 152364+\frac{1}{45}\cdot 153264+\frac{1}{30}\cdot 251634-\frac{1}{15}\cdot 153624-\frac{1}{45}\cdot 512634\\
&-\frac{1}{45}\cdot 521634+\frac{2}{45}\cdot 152436+\frac{4}{45}\cdot 154236-\frac{1}{45}\cdot 253461-\frac{1}{90}\cdot 152634-\frac{1}{15}\cdot 156234\\
&-\frac{1}{45}\cdot 253614-\frac{1}{30}\cdot 516234-\frac{1}{10}\cdot 516324+\frac{2}{45}\cdot 162354+\frac{2}{45}\cdot 163254+\frac{7}{90}\cdot 261453\\
&+\frac{1}{15}\cdot 361452+\frac{1}{90}\cdot 364152+\frac{1}{18}\cdot 261534-\frac{2}{45}\cdot 163524-\frac{1}{45}\cdot 612534-\frac{1}{45}\cdot 621534\\
&+\frac{1}{45}\cdot 162435+\frac{1}{30}\cdot 163425+\frac{1}{45}\cdot 263415+\frac{1}{18}\cdot 164235+\frac{1}{30}\cdot 162453-\frac{1}{15}\cdot 163452\\
&-\frac{1}{30}\cdot 263451-\frac{4}{45}\cdot 164352-\frac{1}{10}\cdot 264351+\frac{1}{90}\cdot 162534-\frac{1}{15}\cdot 165234-\frac{4}{45}\cdot 165324
\end{aligned}
$$

$$
\begin{aligned}
&-\frac{1}{18}\cdot 263514-\frac{1}{30}\cdot 615234-\frac{7}{90}\cdot 615324+\frac{4}{15}\cdot 126543+\frac{4}{15}\cdot 216543+\frac{2}{45}\cdot 361542\\
&+\frac{1}{90}\cdot 415362-\frac{1}{15}\cdot 146532-\frac{1}{15}\cdot 236514-\frac{2}{15}\cdot 236541-\frac{4}{45}\cdot 326514-\frac{2}{15}\cdot 326541\\
&-\frac{7}{45}\cdot 416523-\frac{1}{15}\cdot 416532+\frac{1}{18}\cdot 152643+\frac{1}{18}\cdot 251643-\frac{1}{15}\cdot 512643-\frac{1}{15}\cdot 521643\\
&+\frac{4}{15}\cdot 154326+\frac{2}{45}\cdot 514362-\frac{1}{15}\cdot 154632-\frac{2}{15}\cdot 254361-\frac{7}{90}\cdot 516243-\frac{4}{45}\cdot 516342\\
&-\frac{11}{90}\cdot 526143+\frac{1}{10}\cdot 162543+\frac{1}{10}\cdot 261543-\frac{2}{45}\cdot 163542-\frac{1}{15}\cdot 612543-\frac{1}{15}\cdot 621543\\
&+\frac{1}{10}\cdot 164325-\frac{1}{15}\cdot 614325-\frac{1}{9}\cdot 164532-\frac{1}{18}\cdot 263541-\frac{1}{45}\cdot 362514-\frac{7}{90}\cdot 362541\\
&-\frac{7}{45}\cdot 165342-\frac{2}{45}\cdot 165243-\frac{1}{9}\cdot 265143-\frac{1}{18}\cdot 615243-\frac{7}{90}\cdot 625143+\frac{1}{18}\cdot 316425\\
&+\frac{1}{18}\cdot 316524+\frac{4}{45}\cdot 416325+\frac{1}{30}\cdot 152463+\frac{1}{18}\cdot 251463-\frac{2}{45}\cdot 412653-\frac{2}{45}\cdot 421653\\
&-\frac{1}{9}\cdot 516423-\frac{1}{15}\cdot 426153+\frac{1}{15}\cdot 365142+\frac{1}{15}\cdot 264315+\frac{1}{15}\cdot 265314+\frac{1}{45}\cdot 365241\\
&-\frac{1}{5}\cdot 165423-\frac{2}{15}\cdot 265413-\frac{1}{15}\cdot 615423-\frac{1}{45}\cdot 625413-\frac{7}{90}\cdot 426513+\frac{1}{45}\cdot 314625\\
&+\frac{1}{15}\cdot 234156+\frac{1}{15}\cdot 234165+\frac{4}{45}\cdot 324156+\frac{4}{45}\cdot 324165+\frac{1}{45}\cdot 236145-\frac{1}{45}\cdot 236154\\
&+\frac{2}{45}\cdot 235146+\frac{1}{45}\cdot 235164+\frac{2}{45}\cdot 325146+\frac{1}{45}\cdot 325164-\frac{1}{45}\cdot 425316-\frac{1}{30}\cdot 341526\\
&+\frac{1}{90}\cdot 341625-\frac{1}{90}\cdot 431526+\frac{8}{45}\cdot 342156+\frac{8}{45}\cdot 342165+\frac{4}{45}\cdot 243156+\frac{4}{45}\cdot 243165\\
&+\frac{2}{15}\cdot 423156+\frac{2}{15}\cdot 423165-\frac{1}{15}\cdot 342561-\frac{1}{15}\cdot 342651-\frac{1}{90}\cdot 245136-\frac{1}{45}\cdot 246135\\
&-\frac{1}{5}\cdot 345126-\frac{1}{10}\cdot 345162-\frac{1}{9}\cdot 346125-\frac{1}{18}\cdot 346152-\frac{11}{45}\cdot 435126-\frac{1}{10}\cdot 435162\\
&-\frac{4}{45}\cdot 451326+\frac{1}{45}\cdot 451362-\frac{1}{15}\cdot 351426-\frac{1}{45}\cdot 531426+\frac{7}{90}\cdot 352146+\frac{1}{18}\cdot 352164\\
&+\frac{1}{9}\cdot 452613+\frac{1}{30}\cdot 253146+\frac{1}{30}\cdot 253164-\frac{2}{15}\cdot 452136-\frac{2}{15}\cdot 452163-\frac{1}{45}\cdot 263145\\
&-\frac{1}{45}\cdot 263154-\frac{1}{15}\cdot 623145-\frac{1}{15}\cdot 623154-\frac{2}{45}\cdot 352461-\frac{1}{15}\cdot 352641-\frac{8}{45}\cdot 452316\\
&+\frac{2}{45}\cdot 452361+\frac{1}{90}\cdot 254136-\frac{11}{45}\cdot 354126-\frac{1}{10}\cdot 354162-\frac{2}{9}\cdot 453126-\frac{2}{15}\cdot 453162\\
&-\frac{1}{30}\cdot 264135-\frac{4}{15}\cdot 534126-\frac{2}{15}\cdot 534162-\frac{2}{45}\cdot 624135-\frac{2}{45}\cdot 624153-\frac{4}{45}\cdot 364125\\
&-\frac{2}{45}\cdot 634125-\frac{2}{45}\cdot 326154+\frac{1}{90}\cdot 431625-\frac{1}{15}\cdot 256134-\frac{1}{5}\cdot 436125-\frac{7}{90}\cdot 436152\\
&-\frac{1}{30}\cdot 526134-\frac{1}{18}\cdot 461325+\frac{1}{18}\cdot 461352-\frac{1}{45}\cdot 361425-\frac{1}{45}\cdot 362145-\frac{1}{15}\cdot 362154\\
&+\frac{1}{9}\cdot 462513-\frac{1}{90}\cdot 362451-\frac{2}{15}\cdot 462315+\frac{4}{45}\cdot 462351-\frac{2}{45}\cdot 265134-\frac{1}{9}\cdot 463125\\
&-\frac{1}{15}\cdot 463152+\frac{4}{45}\cdot 365124-\frac{1}{90}\cdot 625134+\frac{2}{45}\cdot 635124-\frac{2}{45}\cdot 235614-\frac{1}{15}\cdot 325614\\
&-\frac{1}{15}\cdot 425136+\frac{1}{45}\cdot 241635-\frac{1}{30}\cdot 426135+\frac{1}{90}\cdot 346251-\frac{1}{90}\cdot 436251-\frac{1}{90}\cdot 351264\\
&+\frac{1}{15}\cdot 523614+\frac{4}{45}\cdot 532614-\frac{2}{45}\cdot 352416-\frac{2}{45}\cdot 524136+\frac{4}{45}\cdot 356124+\frac{1}{15}\cdot 356214
\end{aligned}
$$

$$+\frac{2}{45}\cdot 536124-\frac{1}{15}\cdot 361254-\frac{7}{90}\cdot 461253-\frac{11}{90}\cdot 462153+\frac{1}{90}\cdot 623514-\frac{1}{90}\cdot 632514$$
$$-\frac{1}{45}\cdot 261435-\frac{1}{30}\cdot 362415+\frac{1}{45}\cdot 463251+\frac{1}{9}\cdot 365214-\frac{1}{45}\cdot 635214+\frac{1}{90}\cdot 246315$$
$$+\frac{2}{45}\cdot 346521+\frac{4}{45}\cdot 436521-\frac{1}{45}\cdot 253641+\frac{1}{90}\cdot 523641-\frac{1}{18}\cdot 532641-\frac{1}{15}\cdot 354216$$
$$-\frac{2}{45}\cdot 524316+\frac{2}{45}\cdot 354621+\frac{1}{15}\cdot 526341+\frac{4}{45}\cdot 536142+\frac{1}{45}\cdot 536241+\frac{2}{45}\cdot 461523$$
$$+\frac{1}{45}\cdot 623541-\frac{1}{45}\cdot 364215+\frac{2}{45}\cdot 364512+\frac{1}{15}\cdot 364521+\frac{2}{45}\cdot 463512+\frac{2}{45}\cdot 463521$$
$$+\frac{2}{45}\cdot 625341+\frac{2}{45}\cdot 635241+\frac{1}{45}\cdot 135462+\frac{1}{90}\cdot 135642+\frac{1}{30}\cdot 315642+\frac{1}{45}\cdot 134652$$
$$+\frac{2}{45}\cdot 143652+\frac{1}{90}\cdot 136452+\frac{1}{30}\cdot 136542+\frac{1}{30}\cdot 316452+\frac{1}{30}\cdot 316542+\frac{1}{45}\cdot 243516$$
$$+\frac{1}{90}\cdot 245316+\frac{1}{45}\cdot 235416+\frac{2}{45}\cdot 325416+\frac{1}{45}\cdot 236415+\frac{1}{45}\cdot 326415-\frac{1}{30}\cdot 246531$$
$$-\frac{1}{30}\cdot 426531-\frac{1}{45}\cdot 341652-\frac{2}{45}\cdot 431652-\frac{1}{30}\cdot 513642+\frac{1}{90}\cdot 253416+\frac{1}{30}\cdot 254316$$
$$-\frac{1}{30}\cdot 354261+\frac{1}{30}\cdot 526314-\frac{1}{15}\cdot 526413+\frac{8}{45}\cdot 465132-\frac{1}{30}\cdot 613542-\frac{7}{90}\cdot 631542$$
$$+\frac{8}{45}\cdot 465213-\frac{1}{90}\cdot 624315-\frac{1}{90}\cdot 364251+\frac{1}{45}\cdot 465231+\frac{1}{45}\cdot 462531-\frac{1}{15}\cdot 365412$$
$$+\frac{1}{90}\cdot 625314+\frac{1}{15}\cdot 635412+\frac{2}{45}\cdot 635142+\frac{1}{45}\cdot 314256+\frac{1}{45}\cdot 314265+\frac{2}{45}\cdot 341256$$
$$+\frac{2}{45}\cdot 341265-\frac{1}{45}\cdot 316245-\frac{1}{45}\cdot 316254-\frac{1}{45}\cdot 361245+\frac{1}{90}\cdot 351246+\frac{1}{45}\cdot 412536$$
$$+\frac{1}{45}\cdot 412635+\frac{1}{45}\cdot 421536+\frac{1}{45}\cdot 421635+\frac{2}{45}\cdot 413256+\frac{2}{45}\cdot 413265+\frac{4}{45}\cdot 431256$$
$$+\frac{4}{45}\cdot 431265-\frac{1}{45}\cdot 423561-\frac{1}{45}\cdot 423651-\frac{1}{90}\cdot 415236-\frac{2}{45}\cdot 415263-\frac{1}{15}\cdot 451236$$
$$-\frac{1}{15}\cdot 451263-\frac{1}{30}\cdot 461235-\frac{7}{90}\cdot 462135+\frac{2}{45}\cdot 512436+\frac{2}{45}\cdot 521436+\frac{1}{45}\cdot 513246$$
$$+\frac{1}{45}\cdot 513264+\frac{1}{30}\cdot 523146+\frac{1}{30}\cdot 523164+\frac{1}{18}\cdot 531246+\frac{1}{18}\cdot 531264+\frac{1}{45}\cdot 631245$$
$$+\frac{1}{45}\cdot 631254+\frac{1}{30}\cdot 513426-\frac{1}{15}\cdot 523416-\frac{1}{30}\cdot 523461-\frac{4}{45}\cdot 532416-\frac{1}{10}\cdot 532461$$
$$+\frac{1}{90}\cdot 514236-\frac{1}{30}\cdot 514263-\frac{1}{15}\cdot 541236-\frac{2}{45}\cdot 541263-\frac{4}{45}\cdot 542136-\frac{1}{30}\cdot 641235$$
$$-\frac{1}{30}\cdot 641253-\frac{1}{10}\cdot 642135+\frac{1}{45}\cdot 142563+\frac{1}{45}\cdot 142653+\frac{1}{45}\cdot 241563+\frac{1}{45}\cdot 241653$$
$$+\frac{1}{45}\cdot 314526+\frac{1}{45}\cdot 315426-\frac{7}{90}\cdot 425163+\frac{1}{18}\cdot 415326+\frac{1}{30}\cdot 413526+\frac{1}{30}\cdot 413625$$
$$-\frac{1}{45}\cdot 425361-\frac{1}{45}\cdot 426351-\frac{1}{15}\cdot 415623-\frac{1}{18}\cdot 425613-\frac{1}{45}\cdot 524163-\frac{1}{45}\cdot 614253$$
$$+\frac{1}{90}\cdot 531624-\frac{1}{45}\cdot 631425-\frac{1}{15}\cdot 514623+\frac{4}{45}\cdot 541623-\frac{1}{90}\cdot 524613-\frac{1}{15}\cdot 542163$$
$$+\frac{1}{15}\cdot 641523-\frac{1}{10}\cdot 642153+\frac{4}{45}\cdot 451623+\frac{1}{9}\cdot 542613+\frac{2}{45}\cdot 642513+\frac{1}{30}\cdot 352614$$
$$+\frac{4}{15}\cdot 432156+\frac{4}{15}\cdot 432165-\frac{1}{45}\cdot 431562-\frac{2}{15}\cdot 432561-\frac{2}{15}\cdot 432651-\frac{1}{15}\cdot 435216$$
$$-\frac{1}{15}\cdot 436215+\frac{1}{10}\cdot 514326+\frac{1}{10}\cdot 532146+\frac{1}{10}\cdot 532164-\frac{1}{15}\cdot 632145-\frac{1}{15}\cdot 632154$$

$$
\begin{aligned}
& -\frac{1}{18}\cdot 531462-\frac{2}{45}\cdot 531642-\frac{1}{9}\cdot 534216-\frac{1}{18}\cdot 524361-\frac{7}{45}\cdot 542316-\frac{2}{45}\cdot 541326 \\
& -\frac{7}{90}\cdot 641325+\frac{2}{45}\cdot 541362-\frac{1}{5}\cdot 543126-\frac{2}{15}\cdot 543162-\frac{1}{45}\cdot 643125+\frac{2}{45}\cdot 435621 \\
& +\frac{1}{45}\cdot 452631-\frac{1}{45}\cdot 632451+\frac{2}{45}\cdot 534612+\frac{1}{15}\cdot 534621+\frac{1}{15}\cdot 536412+\frac{1}{15}\cdot 536421 \\
& +\frac{4}{45}\cdot 642351+\frac{1}{15}\cdot 642531+\frac{1}{45}\cdot 143562+\frac{1}{90}\cdot 153462+\frac{1}{30}\cdot 154362+\frac{1}{90}\cdot 145362 \\
& +\frac{1}{45}\cdot 324516+\frac{1}{30}\cdot 423615+\frac{1}{90}\cdot 423516-\frac{1}{30}\cdot 254631+\frac{1}{30}\cdot 432516+\frac{1}{30}\cdot 432615 \\
& +\frac{1}{90}\cdot 342516+\frac{1}{30}\cdot 342615-\frac{1}{30}\cdot 435261+\frac{1}{15}\cdot 541632+\frac{8}{45}\cdot 546132-\frac{1}{18}\cdot 614352 \\
& +\frac{8}{45}\cdot 546213-\frac{1}{30}\cdot 632415-\frac{1}{15}\cdot 543612+\frac{1}{45}\cdot 546312+\frac{2}{5}\cdot 456123+\frac{1}{5}\cdot 456132 \\
& +\frac{1}{3}\cdot 465123-\frac{4}{45}\cdot 561324+\frac{1}{45}\cdot 561342+\frac{1}{45}\cdot 561423-\frac{4}{45}\cdot 562134-\frac{8}{45}\cdot 562143 \\
& +\frac{1}{45}\cdot 634152+\frac{1}{5}\cdot 562341+\frac{4}{45}\cdot 562431-\frac{1}{45}\cdot 562314+\frac{1}{3}\cdot 546123+\frac{4}{15}\cdot 564123 \\
& +\frac{4}{45}\cdot 564132+\frac{1}{15}\cdot 563124+\frac{4}{15}\cdot 645123+\frac{4}{45}\cdot 645132+\frac{1}{5}\cdot 456213-\frac{4}{45}\cdot 561243 \\
& +\frac{2}{45}\cdot 563241+\frac{4}{45}\cdot 564213+\frac{4}{45}\cdot 645213-\frac{1}{15}\cdot 145632-\frac{1}{30}\cdot 245631-\frac{1}{15}\cdot 156432 \\
& -\frac{1}{15}\cdot 345216-\frac{1}{30}\cdot 345261-\frac{1}{45}\cdot 346215+\frac{1}{45}\cdot 356421-\frac{1}{45}\cdot 415632-\frac{1}{90}\cdot 425631 \\
& -\frac{1}{15}\cdot 453216-\frac{1}{15}\cdot 463215+\frac{1}{45}\cdot 453621+\frac{1}{15}\cdot 456231+\frac{1}{45}\cdot 451632-\frac{1}{15}\cdot 516432 \\
& -\frac{1}{15}\cdot 561432-\frac{1}{90}\cdot 524631+\frac{1}{45}\cdot 624531-\frac{1}{15}\cdot 563214+\frac{1}{45}\cdot 634251+\frac{2}{15}\cdot 563412 \\
& +\frac{2}{45}\cdot 563421+\frac{1}{45}\cdot 546231+\frac{2}{45}\cdot 564231+\frac{2}{45}\cdot 645231+\frac{1}{15}\cdot 456312-\frac{1}{45}\cdot 614532 \\
& -\frac{1}{15}\cdot 634215+\frac{2}{45}\cdot 564312+\frac{1}{45}\cdot 465312+\frac{2}{45}\cdot 645312-\frac{2}{45}\cdot 615342-\frac{2}{45}\cdot 651324 \\
& -\frac{2}{45}\cdot 651243-\frac{4}{45}\cdot 652143+\frac{2}{45}\cdot 651423+\frac{2}{45}\cdot 562413+\frac{2}{45}\cdot 652413-\frac{1}{18}\cdot 631452 \\
& -\frac{2}{45}\cdot 642315-\frac{2}{45}\cdot 652134+\frac{1}{15}\cdot 563142+\frac{4}{45}\cdot 653124+\frac{1}{15}\cdot 653142+\frac{2}{15}\cdot 634512 \\
& +\frac{1}{15}\cdot 634521+\frac{2}{45}\cdot 635421+\frac{2}{15}\cdot 652341+\frac{1}{15}\cdot 652431+\frac{1}{90}\cdot 641352+\frac{2}{45}\cdot 651342 \\
& -\frac{1}{30}\cdot 613452-\frac{1}{30}\cdot 623415+\frac{1}{45}\cdot 643512+\frac{2}{45}\cdot 653412+\frac{1}{45}\cdot 653241+\frac{1}{5}\cdot 654123 \\
& +\frac{1}{15}\cdot 654213+\frac{1}{15}\cdot 654132
\end{aligned}
$$

$$
\begin{aligned}
[\![y_3\times y_5]\!] =\ & \frac{2}{45}\cdot 124563+\frac{2}{45}\cdot 125463+\frac{2}{45}\cdot 214563+\frac{2}{45}\cdot 215463-\frac{1}{45}\cdot 124635-\frac{1}{45}\cdot 214635 \\
& +\frac{2}{45}\cdot 134526+\frac{2}{45}\cdot 143526-\frac{1}{90}\cdot 316452+\frac{1}{45}\cdot 361452+\frac{1}{90}\cdot 461352-\frac{1}{45}\cdot 135246 \\
& -\frac{1}{30}\cdot 145263-\frac{1}{18}\cdot 154263-\frac{2}{45}\cdot 245163-\frac{2}{45}\cdot 254163-\frac{1}{45}\cdot 412563-\frac{1}{45}\cdot 512463 \\
& -\frac{1}{45}\cdot 521463-\frac{1}{90}\cdot 145362-\frac{1}{90}\cdot 135642+\frac{1}{90}\cdot 245631+\frac{1}{30}\cdot 254631+\frac{4}{45}\cdot 156243
\end{aligned}
$$

$$
\begin{aligned}
&-\frac{1}{90}\cdot 246153+\frac{1}{30}\cdot 146325+\frac{2}{45}\cdot 156324+\frac{1}{30}\cdot 246315+\frac{1}{15}\cdot 256314-\frac{1}{45}\cdot 146352\\
&+\frac{2}{45}\cdot 156342-\frac{1}{45}\cdot 246351+\frac{2}{45}\cdot 256341+\frac{1}{45}\cdot 163452+\frac{1}{90}\cdot 613452+\frac{1}{90}\cdot 614352\\
&-\frac{1}{15}\cdot 146523-\frac{1}{90}\cdot 246513-\frac{1}{30}\cdot 136524-\frac{1}{45}\cdot 163524-\frac{2}{45}\cdot 164523-\frac{1}{45}\cdot 613524\\
&-\frac{2}{45}\cdot 614523+\frac{1}{45}\cdot 351624-\frac{1}{45}\cdot 126345-\frac{1}{45}\cdot 216345+\frac{1}{45}\cdot 416523-\frac{1}{45}\cdot 461523\\
&-\frac{1}{45}\cdot 152346+\frac{1}{45}\cdot 521634-\frac{1}{90}\cdot 152463-\frac{1}{15}\cdot 154623+\frac{1}{90}\cdot 152643+\frac{1}{90}\cdot 516243\\
&+\frac{2}{45}\cdot 516342+\frac{1}{45}\cdot 162354+\frac{1}{90}\cdot 261534+\frac{1}{90}\cdot 163425+\frac{1}{90}\cdot 162453+\frac{1}{90}\cdot 263451\\
&-\frac{1}{45}\cdot 165324-\frac{1}{30}\cdot 263514+\frac{1}{90}\cdot 615234+\frac{2}{45}\cdot 125643+\frac{2}{45}\cdot 215643+\frac{1}{90}\cdot 351642\\
&-\frac{2}{45}\cdot 126435-\frac{2}{45}\cdot 216435+\frac{2}{45}\cdot 145326+\frac{1}{30}\cdot 415362-\frac{2}{45}\cdot 461532-\frac{2}{45}\cdot 153246\\
&-\frac{1}{45}\cdot 512643+\frac{1}{15}\cdot 156432+\frac{1}{45}\cdot 516423+\frac{2}{45}\cdot 516432+\frac{1}{30}\cdot 162543+\frac{2}{45}\cdot 163542\\
&+\frac{1}{30}\cdot 261543+\frac{1}{30}\cdot 164235+\frac{1}{30}\cdot 164325-\frac{1}{45}\cdot 264153+\frac{1}{45}\cdot 164532-\frac{1}{30}\cdot 264351\\
&+\frac{1}{45}\cdot 165243-\frac{1}{45}\cdot 165342-\frac{1}{45}\cdot 265143-\frac{1}{90}\cdot 615324+\frac{2}{45}\cdot 124653+\frac{2}{45}\cdot 214653\\
&-\frac{2}{45}\cdot 126534-\frac{2}{45}\cdot 216534+\frac{2}{45}\cdot 135426-\frac{1}{30}\cdot 136542-\frac{1}{30}\cdot 316542+\frac{1}{45}\cdot 416532\\
&-\frac{2}{45}\cdot 154236-\frac{1}{45}\cdot 412653-\frac{1}{90}\cdot 153462-\frac{1}{30}\cdot 154362+\frac{1}{30}\cdot 246531+\frac{1}{45}\cdot 256431\\
&+\frac{1}{90}\cdot 426531-\frac{1}{45}\cdot 526431+\frac{1}{30}\cdot 261453+\frac{2}{45}\cdot 265314+\frac{1}{45}\cdot 265341+\frac{1}{30}\cdot 613542\\
&-\frac{1}{30}\cdot 631542-\frac{1}{45}\cdot 641532-\frac{1}{15}\cdot 165423-\frac{1}{45}\cdot 265413-\frac{2}{45}\cdot 615423+\frac{1}{90}\cdot 316425\\
&-\frac{1}{90}\cdot 315642-\frac{1}{90}\cdot 513642-\frac{1}{45}\cdot 531642-\frac{1}{45}\cdot 315264-\frac{1}{45}\cdot 415263+\frac{2}{45}\cdot 234156\\
&+\frac{2}{45}\cdot 234165+\frac{2}{45}\cdot 324156+\frac{2}{45}\cdot 324165-\frac{1}{45}\cdot 241356-\frac{1}{45}\cdot 241365+\frac{1}{45}\cdot 241563\\
&+\frac{1}{45}\cdot 241653+\frac{1}{45}\cdot 341562+\frac{1}{45}\cdot 341652-\frac{1}{30}\cdot 341526-\frac{1}{18}\cdot 431526-\frac{1}{90}\cdot 342516\\
&-\frac{1}{90}\cdot 342615-\frac{1}{90}\cdot 245316+\frac{1}{45}\cdot 346215+\frac{1}{90}\cdot 345261+\frac{1}{30}\cdot 435261+\frac{4}{45}\cdot 451326\\
&+\frac{1}{30}\cdot 352146+\frac{1}{90}\cdot 352164+\frac{1}{90}\cdot 352614+\frac{2}{45}\cdot 452136+\frac{2}{45}\cdot 452163+\frac{2}{45}\cdot 452613\\
&-\frac{1}{45}\cdot 352416-\frac{1}{45}\cdot 352461-\frac{2}{45}\cdot 352641+\frac{2}{45}\cdot 452316+\frac{2}{45}\cdot 452361-\frac{2}{45}\cdot 452631\\
&+\frac{1}{45}\cdot 523416+\frac{1}{90}\cdot 623415+\frac{1}{30}\cdot 632415-\frac{1}{15}\cdot 354126-\frac{1}{30}\cdot 254136-\frac{1}{90}\cdot 264135\\
&-\frac{1}{90}\cdot 354162-\frac{1}{15}\cdot 364125-\frac{1}{30}\cdot 364152-\frac{1}{45}\cdot 524136-\frac{2}{45}\cdot 524163-\frac{2}{45}\cdot 534126\\
&-\frac{1}{45}\cdot 624135-\frac{1}{45}\cdot 624153-\frac{2}{45}\cdot 634125-\frac{2}{45}\cdot 634152+\frac{1}{45}\cdot 134625+\frac{1}{45}\cdot 143625\\
&+\frac{1}{30}\cdot 315624-\frac{1}{45}\cdot 136245-\frac{1}{45}\cdot 136254-\frac{1}{45}\cdot 316245-\frac{1}{45}\cdot 316254+\frac{1}{45}\cdot 235146\\
&+\frac{1}{45}\cdot 235164+\frac{1}{45}\cdot 325146+\frac{1}{45}\cdot 325164-\frac{1}{45}\cdot 236514-\frac{1}{45}\cdot 326514-\frac{1}{45}\cdot 251346
\end{aligned}
$$

$$- \frac{1}{45} \cdot 251436 - \frac{1}{30} \cdot 351264 + \frac{1}{90} \cdot 251634 + \frac{1}{90} \cdot 251643 + \frac{1}{45} \cdot 351462 - \frac{1}{90} \cdot 341625$$
$$- \frac{1}{30} \cdot 431625 - \frac{1}{45} \cdot 513624 - \frac{1}{90} \cdot 254613 + \frac{1}{90} \cdot 346251 + \frac{1}{45} \cdot 436215 + \frac{1}{30} \cdot 436251$$
$$+ \frac{1}{30} \cdot 361524 + \frac{1}{30} \cdot 461325 + \frac{1}{45} \cdot 362145 - \frac{1}{90} \cdot 362451 - \frac{1}{30} \cdot 362541 + \frac{1}{90} \cdot 623514$$
$$+ \frac{1}{30} \cdot 632514 + \frac{1}{45} \cdot 365124 + \frac{1}{45} \cdot 463125 - \frac{1}{90} \cdot 625134 - \frac{1}{30} \cdot 625143 - \frac{1}{45} \cdot 235614$$
$$- \frac{1}{45} \cdot 325614 + \frac{1}{45} \cdot 236145 + \frac{1}{45} \cdot 326145 + \frac{1}{30} \cdot 426513 - \frac{1}{45} \cdot 251364 + \frac{1}{45} \cdot 523614$$
$$+ \frac{2}{45} \cdot 532614 + \frac{1}{90} \cdot 251463 - \frac{1}{45} \cdot 356241 - \frac{1}{90} \cdot 526143 - \frac{1}{45} \cdot 536142 - \frac{1}{45} \cdot 536241$$
$$- \frac{1}{45} \cdot 361254 - \frac{1}{45} \cdot 261435 - \frac{1}{90} \cdot 362415 - \frac{1}{15} \cdot 624513 + \frac{1}{45} \cdot 365214 - \frac{1}{45} \cdot 235641$$
$$- \frac{1}{45} \cdot 325641 + \frac{1}{45} \cdot 236451 + \frac{1}{45} \cdot 326451 - \frac{2}{45} \cdot 245361 - \frac{1}{90} \cdot 253164 + \frac{1}{90} \cdot 523641$$
$$- \frac{1}{90} \cdot 532641 - \frac{1}{45} \cdot 356412 - \frac{1}{45} \cdot 356421 + \frac{1}{90} \cdot 263541 - \frac{2}{45} \cdot 364215 + \frac{1}{45} \cdot 364512$$
$$+ \frac{1}{45} \cdot 364521 - \frac{1}{45} \cdot 624531 + \frac{1}{45} \cdot 365142 - \frac{1}{90} \cdot 136425 + \frac{1}{90} \cdot 316524 - \frac{1}{45} \cdot 236541$$
$$- \frac{1}{45} \cdot 326541 - \frac{1}{45} \cdot 462531 - \frac{1}{90} \cdot 253146 + \frac{1}{45} \cdot 431652 - \frac{2}{45} \cdot 254361 + \frac{2}{45} \cdot 354621$$
$$+ \frac{2}{45} \cdot 346521 + \frac{4}{45} \cdot 436521 - \frac{1}{90} \cdot 364251 - \frac{1}{45} \cdot 465231 + \frac{1}{45} \cdot 264531 + \frac{1}{45} \cdot 623541$$
$$+ \frac{1}{90} \cdot 625314 - \frac{2}{45} \cdot 625413 + \frac{1}{45} \cdot 635412 - \frac{1}{45} \cdot 412356 - \frac{1}{45} \cdot 412365 - \frac{1}{90} \cdot 413526$$
$$- \frac{1}{90} \cdot 413625 - \frac{1}{15} \cdot 435126 - \frac{1}{45} \cdot 436125 + \frac{1}{90} \cdot 415326 + \frac{2}{45} \cdot 451362 + \frac{1}{45} \cdot 512436$$
$$+ \frac{1}{45} \cdot 513264 + \frac{1}{90} \cdot 523146 - \frac{1}{90} \cdot 523164 + \frac{1}{90} \cdot 513426 - \frac{1}{45} \cdot 513462 + \frac{1}{90} \cdot 523461$$
$$- \frac{1}{45} \cdot 542136 + \frac{1}{90} \cdot 641235 - \frac{1}{30} \cdot 641253 - \frac{1}{90} \cdot 152634 - \frac{1}{90} \cdot 415236 - \frac{1}{90} \cdot 416253$$
$$- \frac{1}{90} \cdot 425163 - \frac{1}{45} \cdot 413562 - \frac{1}{45} \cdot 413652 + \frac{1}{45} \cdot 431562 + \frac{1}{45} \cdot 415632 - \frac{2}{45} \cdot 451632$$
$$- \frac{1}{90} \cdot 516324 - \frac{1}{90} \cdot 526314 - \frac{2}{45} \cdot 514623 - \frac{1}{18} \cdot 524613 + \frac{1}{45} \cdot 542163 + \frac{1}{45} \cdot 541623$$
$$+ \frac{1}{45} \cdot 412635 + \frac{1}{45} \cdot 421635 + \frac{1}{90} \cdot 346152 + \frac{1}{30} \cdot 436152 + \frac{1}{45} \cdot 451263 - \frac{1}{45} \cdot 541632$$
$$- \frac{1}{45} \cdot 542631 - \frac{1}{45} \cdot 426153 - \frac{1}{45} \cdot 426315 - \frac{1}{45} \cdot 643152 + \frac{1}{45} \cdot 631524 + \frac{2}{45} \cdot 342156$$
$$+ \frac{2}{45} \cdot 342165 - \frac{2}{45} \cdot 421356 - \frac{2}{45} \cdot 421365 + \frac{1}{30} \cdot 426135 + \frac{1}{15} \cdot 453216 + \frac{2}{45} \cdot 463215$$
$$+ \frac{1}{30} \cdot 514326 + \frac{2}{45} \cdot 524316 + \frac{1}{30} \cdot 531246 + \frac{1}{90} \cdot 531264 + \frac{1}{30} \cdot 532146 + \frac{1}{30} \cdot 532164$$
$$- \frac{1}{30} \cdot 531462 - \frac{1}{30} \cdot 532461 + \frac{1}{45} \cdot 534216 + \frac{1}{45} \cdot 541326 - \frac{1}{45} \cdot 542316 - \frac{1}{30} \cdot 642135$$
$$- \frac{1}{18} \cdot 642153 + \frac{2}{45} \cdot 243156 + \frac{2}{45} \cdot 243165 - \frac{1}{30} \cdot 254316 - \frac{2}{45} \cdot 431256 - \frac{2}{45} \cdot 431265$$
$$- \frac{1}{90} \cdot 423516 - \frac{1}{90} \cdot 423615 - \frac{1}{30} \cdot 432516 - \frac{1}{30} \cdot 432615 + \frac{1}{30} \cdot 354261 + \frac{1}{45} \cdot 453261$$
$$+ \frac{1}{15} \cdot 542613 + \frac{1}{45} \cdot 542361 + \frac{1}{18} \cdot 624315 - \frac{2}{45} \cdot 634215 - \frac{1}{15} \cdot 543126 - \frac{1}{45} \cdot 543162$$

$$
\begin{aligned}
&- \frac{1}{90} \cdot 514263 - \frac{1}{90} \cdot 531624 - \frac{1}{45} \cdot 342561 - \frac{1}{45} \cdot 342651 + \frac{1}{45} \cdot 423561 + \frac{1}{45} \cdot 423651 \\
&+ \frac{1}{90} \cdot 425613 - \frac{1}{90} \cdot 425631 - \frac{1}{45} \cdot 453612 - \frac{1}{45} \cdot 453621 - \frac{1}{45} \cdot 514362 + \frac{1}{90} \cdot 524361 \\
&- \frac{1}{45} \cdot 536124 - \frac{2}{45} \cdot 536214 + \frac{1}{45} \cdot 534612 + \frac{1}{45} \cdot 534621 - \frac{1}{45} \cdot 634251 + \frac{1}{45} \cdot 541362 \\
&+ \frac{2}{45} \cdot 642351 - \frac{1}{90} \cdot 435162 - \frac{1}{45} \cdot 432561 - \frac{1}{45} \cdot 432651 + \frac{2}{45} \cdot 435621 + \frac{1}{45} \cdot 534261 \\
&- \frac{1}{45} \cdot 546312 - \frac{1}{90} \cdot 135624 - \frac{1}{15} \cdot 145623 + \frac{1}{15} \cdot 156234 - \frac{1}{90} \cdot 245136 - \frac{1}{15} \cdot 345126 \\
&- \frac{1}{30} \cdot 345162 - \frac{1}{45} \cdot 346125 + \frac{2}{45} \cdot 354612 + \frac{1}{15} \cdot 451236 + \frac{1}{30} \cdot 461235 + \frac{1}{45} \cdot 415623 \\
&+ \frac{2}{45} \cdot 435612 + \frac{4}{45} \cdot 436512 - \frac{1}{15} \cdot 456213 - \frac{4}{45} \cdot 456312 - \frac{1}{45} \cdot 465312 - \frac{4}{45} \cdot 456231 \\
&- \frac{2}{45} \cdot 561324 - \frac{2}{45} \cdot 562134 - \frac{4}{45} \cdot 562143 + \frac{2}{45} \cdot 562341 + \frac{2}{45} \cdot 562431 - \frac{1}{45} \cdot 634512 \\
&+ \frac{1}{15} \cdot 546123 + \frac{2}{45} \cdot 563124 + \frac{1}{9} \cdot 564123 + \frac{1}{9} \cdot 645123 + \frac{2}{45} \cdot 645132 - \frac{1}{30} \cdot 245613 \\
&+ \frac{1}{45} \cdot 256134 - \frac{1}{90} \cdot 461253 - \frac{1}{15} \cdot 456132 - \frac{2}{45} \cdot 561243 - \frac{2}{45} \cdot 562314 + \frac{2}{45} \cdot 564213 \\
&+ \frac{1}{30} \cdot 516234 + \frac{2}{45} \cdot 346512 - \frac{1}{45} \cdot 546231 - \frac{1}{45} \cdot 643512 + \frac{1}{15} \cdot 465123 + \frac{1}{90} \cdot 146235 \\
&+ \frac{1}{30} \cdot 526134 + \frac{1}{90} \cdot 351246 - \frac{1}{90} \cdot 462153 + \frac{1}{45} \cdot 462351 - \frac{1}{45} \cdot 635124 + \frac{1}{90} \cdot 462135 \\
&- \frac{4}{45} \cdot 456321 - \frac{1}{45} \cdot 465321 - \frac{1}{45} \cdot 514632 - \frac{1}{90} \cdot 524631 - \frac{1}{45} \cdot 634521 + \frac{2}{45} \cdot 564132 \\
&- \frac{1}{45} \cdot 546321 - \frac{1}{45} \cdot 643521 - \frac{2}{45} \cdot 635214 + \frac{2}{45} \cdot 645213 - \frac{1}{90} \cdot 162534 - \frac{1}{90} \cdot 514236 \\
&+ \frac{1}{45} \cdot 612453 + \frac{2}{45} \cdot 612543 + \frac{1}{45} \cdot 621453 + \frac{2}{45} \cdot 621543 + \frac{1}{45} \cdot 614325 - \frac{1}{45} \cdot 615342 \\
&- \frac{2}{45} \cdot 651243 - \frac{4}{45} \cdot 652143 - \frac{2}{45} \cdot 651324 + \frac{1}{45} \cdot 612534 + \frac{1}{45} \cdot 621534 - \frac{1}{45} \cdot 613425 \\
&+ \frac{1}{45} \cdot 614235 + \frac{1}{90} \cdot 615243 - \frac{1}{45} \cdot 163245 - \frac{2}{45} \cdot 263145 - \frac{2}{45} \cdot 263154 - \frac{1}{45} \cdot 521346 \\
&+ \frac{1}{15} \cdot 631245 + \frac{1}{15} \cdot 631254 + \frac{2}{45} \cdot 632145 + \frac{2}{45} \cdot 632154 - \frac{1}{18} \cdot 631452 - \frac{1}{45} \cdot 632451 \\
&- \frac{1}{90} \cdot 641325 - \frac{1}{45} \cdot 642315 - \frac{2}{45} \cdot 652314 - \frac{2}{45} \cdot 652134 - \frac{1}{45} \cdot 623145 - \frac{1}{45} \cdot 623154 \\
&+ \frac{2}{45} \cdot 653124 - \frac{1}{45} \cdot 463512 - \frac{1}{45} \cdot 463521 + \frac{1}{45} \cdot 635421 - \frac{1}{45} \cdot 635241 + \frac{1}{90} \cdot 641352 \\
&+ \frac{2}{45} \cdot 652341 + \frac{2}{45} \cdot 652431 - \frac{1}{90} \cdot 136452 - \frac{1}{90} \cdot 253416 + \frac{1}{9} \cdot 654123 + \frac{2}{45} \cdot 654213 \\
&- \frac{1}{45} \cdot 562413 - \frac{1}{45} \cdot 652413 + \frac{2}{45} \cdot 654132
\end{aligned}
$$

$$
\begin{aligned}
[\![ y_4 \times y_4 ]\!] = &\frac{2}{15} \cdot 124563 + \frac{2}{15} \cdot 124653 + \frac{2}{15} \cdot 214563 + \frac{2}{15} \cdot 214653 + \frac{2}{9} \cdot 125643 + \frac{2}{9} \cdot 215643 \\
&+ \frac{2}{15} \cdot 125463 + \frac{2}{15} \cdot 215463 + \frac{2}{15} \cdot 126453 + \frac{2}{15} \cdot 216453 + \frac{2}{15} \cdot 134526 + \frac{2}{15} \cdot 135426 \\
&+ \frac{2}{45} \cdot 314625 - \frac{2}{45} \cdot 135624 - \frac{2}{45} \cdot 136524 + \frac{2}{45} \cdot 315624 - \frac{4}{45} \cdot 235641 - \frac{4}{45} \cdot 325641
\end{aligned}
$$

$$+\frac{2}{45}\cdot 142563+\frac{2}{45}\cdot 142653+\frac{2}{45}\cdot 241563+\frac{2}{45}\cdot 241653-\frac{2}{45}\cdot 412563-\frac{2}{45}\cdot 421563$$
$$+\frac{2}{9}\cdot 145326+\frac{2}{45}\cdot 246315+\frac{2}{15}\cdot 143526+\frac{2}{15}\cdot 153426+\frac{2}{45}\cdot 413625-\frac{2}{45}\cdot 146352$$
$$-\frac{4}{45}\cdot 245361-\frac{4}{15}\cdot 145623-\frac{14}{45}\cdot 146523-\frac{2}{15}\cdot 245613-\frac{2}{15}\cdot 246513-\frac{2}{45}\cdot 415263$$
$$-\frac{4}{45}\cdot 425163+\frac{4}{45}\cdot 152643+\frac{4}{45}\cdot 251643+\frac{2}{15}\cdot 356142+\frac{2}{45}\cdot 152463+\frac{2}{45}\cdot 251463$$
$$-\frac{2}{45}\cdot 512463-\frac{2}{45}\cdot 521463-\frac{2}{45}\cdot 612453-\frac{2}{45}\cdot 621453+\frac{4}{45}\cdot 256314-\frac{2}{45}\cdot 153624$$
$$-\frac{2}{45}\cdot 163524-\frac{2}{45}\cdot 613425-\frac{8}{45}\cdot 156342-\frac{2}{45}\cdot 253641-\frac{4}{45}\cdot 352641-\frac{14}{45}\cdot 154623$$
$$-\frac{4}{15}\cdot 156423-\frac{2}{15}\cdot 254613-\frac{2}{15}\cdot 256413-\frac{16}{45}\cdot 164523-\frac{2}{15}\cdot 264513-\frac{2}{45}\cdot 514263$$
$$-\frac{2}{45}\cdot 524163-\frac{2}{45}\cdot 614253-\frac{2}{45}\cdot 624153+\frac{2}{45}\cdot 351642+\frac{2}{45}\cdot 134625+\frac{2}{45}\cdot 143625$$
$$-\frac{2}{45}\cdot 153642-\frac{2}{45}\cdot 145263-\frac{2}{45}\cdot 154263-\frac{4}{45}\cdot 245163-\frac{2}{45}\cdot 254163-\frac{2}{45}\cdot 513624$$
$$-\frac{2}{45}\cdot 146253-\frac{2}{45}\cdot 164253-\frac{4}{45}\cdot 246153-\frac{2}{45}\cdot 264153+\frac{4}{45}\cdot 146325+\frac{2}{45}\cdot 136425$$
$$-\frac{2}{45}\cdot 246351-\frac{2}{45}\cdot 613524+\frac{2}{45}\cdot 126534+\frac{4}{15}\cdot 126543+\frac{2}{45}\cdot 216534+\frac{4}{15}\cdot 216543$$
$$+\frac{2}{45}\cdot 361542+\frac{2}{45}\cdot 415362-\frac{2}{45}\cdot 146532-\frac{2}{45}\cdot 236514-\frac{2}{15}\cdot 236541-\frac{2}{45}\cdot 326514$$
$$-\frac{2}{15}\cdot 326541-\frac{2}{15}\cdot 416523-\frac{2}{45}\cdot 416532-\frac{2}{45}\cdot 512643-\frac{2}{45}\cdot 521643+\frac{2}{45}\cdot 154236$$
$$+\frac{4}{15}\cdot 154326+\frac{2}{45}\cdot 514362-\frac{2}{45}\cdot 154632-\frac{2}{15}\cdot 254361-\frac{4}{45}\cdot 516324-\frac{4}{45}\cdot 516243$$
$$-\frac{2}{15}\cdot 526143+\frac{2}{45}\cdot 162534+\frac{2}{15}\cdot 162543+\frac{2}{45}\cdot 261534+\frac{2}{15}\cdot 261543-\frac{2}{45}\cdot 163542$$
$$+\frac{2}{45}\cdot 164235+\frac{2}{15}\cdot 164325-\frac{2}{45}\cdot 164352-\frac{4}{45}\cdot 164532-\frac{4}{45}\cdot 264351-\frac{2}{45}\cdot 263514$$
$$-\frac{4}{45}\cdot 263541-\frac{2}{45}\cdot 362514-\frac{4}{45}\cdot 362541-\frac{8}{45}\cdot 165342-\frac{4}{45}\cdot 615324-\frac{4}{45}\cdot 615243$$
$$-\frac{2}{15}\cdot 625143+\frac{2}{45}\cdot 316524-\frac{2}{45}\cdot 412653-\frac{2}{45}\cdot 421653-\frac{2}{45}\cdot 416253-\frac{4}{45}\cdot 426153$$
$$+\frac{2}{15}\cdot 365142+\frac{2}{45}\cdot 162453+\frac{2}{45}\cdot 261453+\frac{4}{45}\cdot 265314+\frac{2}{45}\cdot 163425-\frac{4}{15}\cdot 165423$$
$$-\frac{2}{15}\cdot 265413+\frac{2}{45}\cdot 316425+\frac{2}{45}\cdot 264315+\frac{2}{45}\cdot 416325-\frac{2}{45}\cdot 156243-\frac{2}{45}\cdot 165243$$
$$-\frac{4}{45}\cdot 256143-\frac{4}{45}\cdot 265143-\frac{2}{45}\cdot 156324-\frac{2}{45}\cdot 165324+\frac{2}{15}\cdot 234156+\frac{2}{15}\cdot 234165$$
$$+\frac{2}{15}\cdot 243156+\frac{2}{15}\cdot 243165-\frac{2}{45}\cdot 236145-\frac{2}{45}\cdot 236154-\frac{2}{45}\cdot 245136-\frac{2}{45}\cdot 254136$$
$$-\frac{2}{45}\cdot 263145-\frac{2}{45}\cdot 263154+\frac{2}{45}\cdot 314526+\frac{2}{45}\cdot 315426+\frac{2}{45}\cdot 341625+\frac{2}{9}\cdot 342156$$
$$+\frac{2}{9}\cdot 342165+\frac{2}{45}\cdot 352614+\frac{2}{15}\cdot 324156+\frac{2}{15}\cdot 324165+\frac{2}{15}\cdot 423156+\frac{2}{15}\cdot 423165$$
$$-\frac{4}{45}\cdot 342561-\frac{4}{45}\cdot 342651-\frac{2}{45}\cdot 352416-\frac{4}{15}\cdot 345126-\frac{2}{15}\cdot 345162-\frac{14}{45}\cdot 354126$$
$$-\frac{2}{15}\cdot 354162-\frac{2}{45}\cdot 361425+\frac{4}{45}\cdot 415326+\frac{4}{45}\cdot 451362+\frac{2}{45}\cdot 413526+\frac{2}{15}\cdot 452613$$

$$
\begin{aligned}
&- \frac{2}{45} \cdot 425136 - \frac{2}{45} \cdot 524136 - \frac{2}{45} \cdot 623145 - \frac{2}{45} \cdot 623154 - \frac{8}{45} \cdot 452316 - \frac{2}{45} \cdot 425361 \\
&- \frac{14}{45} \cdot 435126 - \frac{2}{15} \cdot 435162 - \frac{4}{15} \cdot 453126 - \frac{2}{15} \cdot 453162 - \frac{16}{45} \cdot 534126 - \frac{2}{15} \cdot 534162 \\
&- \frac{2}{45} \cdot 631425 + \frac{2}{45} \cdot 235146 + \frac{2}{45} \cdot 235164 + \frac{2}{45} \cdot 325146 + \frac{2}{45} \cdot 325164 - \frac{2}{45} \cdot 425316 \\
&- \frac{2}{45} \cdot 341526 - \frac{2}{45} \cdot 431526 - \frac{2}{45} \cdot 246135 - \frac{2}{45} \cdot 351426 - \frac{2}{45} \cdot 531426 + \frac{4}{45} \cdot 352146 \\
&+ \frac{4}{45} \cdot 352164 + \frac{2}{45} \cdot 253146 + \frac{2}{45} \cdot 253164 - \frac{2}{45} \cdot 352461 - \frac{2}{45} \cdot 264135 - \frac{2}{45} \cdot 624135 \\
&- \frac{2}{45} \cdot 256134 - \frac{2}{45} \cdot 265134 - \frac{2}{45} \cdot 362145 - \frac{2}{45} \cdot 362154 - \frac{2}{45} \cdot 326145 - \frac{2}{45} \cdot 326154 \\
&+ \frac{4}{45} \cdot 356124 + \frac{4}{45} \cdot 365124 - \frac{4}{45} \cdot 461325 - \frac{4}{45} \cdot 462135 - \frac{2}{15} \cdot 462153 - \frac{2}{45} \cdot 426135 \\
&- \frac{2}{45} \cdot 526134 - \frac{2}{45} \cdot 625134 + \frac{4}{45} \cdot 462351 + \frac{2}{45} \cdot 462531 + \frac{2}{45} \cdot 431625 + \frac{2}{45} \cdot 536124 \\
&+ \frac{4}{45} \cdot 536142 + \frac{2}{45} \cdot 635124 + \frac{4}{45} \cdot 635142 + \frac{2}{45} \cdot 351624 - \frac{4}{45} \cdot 346125 - \frac{2}{45} \cdot 346152 \\
&- \frac{2}{15} \cdot 436125 - \frac{2}{45} \cdot 436152 + \frac{2}{45} \cdot 461352 + \frac{2}{45} \cdot 361524 + \frac{4}{45} \cdot 462513 - \frac{4}{45} \cdot 462315 \\
&- \frac{2}{15} \cdot 364125 - \frac{2}{45} \cdot 364152 - \frac{4}{45} \cdot 463125 - \frac{2}{45} \cdot 463152 + \frac{2}{45} \cdot 346512 + \frac{2}{45} \cdot 346521 \\
&+ \frac{4}{45} \cdot 436512 + \frac{4}{45} \cdot 436521 - \frac{4}{45} \cdot 532641 - \frac{2}{45} \cdot 354216 - \frac{2}{45} \cdot 524316 + \frac{2}{45} \cdot 354612 \\
&+ \frac{2}{45} \cdot 354621 + \frac{4}{45} \cdot 526341 + \frac{2}{45} \cdot 536241 + \frac{2}{45} \cdot 461523 - \frac{2}{45} \cdot 461532 - \frac{2}{45} \cdot 623541 \\
&- \frac{4}{45} \cdot 632541 - \frac{2}{45} \cdot 364215 - \frac{2}{45} \cdot 624351 + \frac{4}{45} \cdot 364512 + \frac{4}{45} \cdot 364521 + \frac{2}{45} \cdot 463512 \\
&+ \frac{2}{45} \cdot 463521 + \frac{4}{45} \cdot 625341 + \frac{2}{45} \cdot 635241 - \frac{4}{45} \cdot 415623 - \frac{2}{45} \cdot 425613 - \frac{2}{45} \cdot 426513 \\
&- \frac{2}{45} \cdot 451263 - \frac{4}{45} \cdot 452163 - \frac{2}{45} \cdot 461253 + \frac{2}{45} \cdot 526314 + \frac{2}{45} \cdot 531624 - \frac{4}{45} \cdot 516342 \\
&- \frac{2}{15} \cdot 514623 - \frac{4}{45} \cdot 516423 - \frac{2}{45} \cdot 524613 - \frac{2}{45} \cdot 526413 - \frac{2}{45} \cdot 541263 - \frac{4}{45} \cdot 542163 \\
&- \frac{2}{45} \cdot 641253 - \frac{2}{15} \cdot 642153 + \frac{4}{45} \cdot 451623 + \frac{4}{45} \cdot 541623 + \frac{2}{15} \cdot 542613 + \frac{2}{45} \cdot 641523 \\
&+ \frac{4}{45} \cdot 642513 + \frac{2}{45} \cdot 431256 + \frac{2}{45} \cdot 431265 + \frac{4}{15} \cdot 432156 + \frac{4}{15} \cdot 432165 + \frac{2}{45} \cdot 532614 \\
&- \frac{2}{45} \cdot 431562 - \frac{2}{45} \cdot 431652 - \frac{2}{15} \cdot 432561 - \frac{2}{15} \cdot 432651 - \frac{2}{45} \cdot 435216 - \frac{2}{45} \cdot 436215 \\
&+ \frac{2}{45} \cdot 514236 + \frac{2}{15} \cdot 514326 + \frac{2}{45} \cdot 531246 + \frac{2}{45} \cdot 531264 + \frac{2}{15} \cdot 532146 + \frac{2}{15} \cdot 532164 \\
&- \frac{2}{45} \cdot 532416 - \frac{2}{45} \cdot 531462 - \frac{2}{45} \cdot 531642 - \frac{4}{45} \cdot 532461 - \frac{4}{45} \cdot 534216 - \frac{4}{45} \cdot 524361 \\
&- \frac{8}{45} \cdot 542316 - \frac{4}{45} \cdot 642135 - \frac{4}{45} \cdot 641325 + \frac{4}{45} \cdot 541362 + \frac{2}{45} \cdot 513426 + \frac{2}{45} \cdot 523146 \\
&+ \frac{2}{45} \cdot 523164 - \frac{4}{15} \cdot 543126 - \frac{2}{15} \cdot 543162 - \frac{2}{45} \cdot 451326 - \frac{2}{45} \cdot 541326 - \frac{2}{45} \cdot 452136 \\
&- \frac{2}{45} \cdot 542136 + \frac{2}{45} \cdot 435612 + \frac{2}{45} \cdot 435621 - \frac{2}{45} \cdot 514632 - \frac{2}{45} \cdot 536214 - \frac{2}{45} \cdot 632451 \\
&+ \frac{4}{45} \cdot 534612 + \frac{4}{45} \cdot 534621 + \frac{2}{45} \cdot 536412 + \frac{2}{45} \cdot 536421 + \frac{4}{45} \cdot 642351 + \frac{2}{45} \cdot 642531
\end{aligned}
$$

$$+\frac{2}{5}\cdot 456123+\frac{2}{15}\cdot 456132+\frac{2}{5}\cdot 465123+\frac{2}{15}\cdot 465132-\frac{2}{15}\cdot 561324-\frac{2}{15}\cdot 562134$$
$$-\frac{4}{15}\cdot 562143+\frac{4}{15}\cdot 562341+\frac{4}{45}\cdot 562431+\frac{2}{5}\cdot 546123+\frac{2}{15}\cdot 546132+\frac{2}{5}\cdot 564123$$
$$+\frac{2}{15}\cdot 564132+\frac{2}{5}\cdot 645123+\frac{2}{15}\cdot 645132+\frac{2}{15}\cdot 456213+\frac{2}{15}\cdot 465213-\frac{2}{15}\cdot 561243$$
$$+\frac{4}{45}\cdot 563241+\frac{2}{15}\cdot 546213+\frac{2}{15}\cdot 564213+\frac{2}{15}\cdot 645213+\frac{2}{45}\cdot 612534+\frac{2}{45}\cdot 621534$$
$$+\frac{2}{45}\cdot 614235+\frac{2}{45}\cdot 641352-\frac{8}{45}\cdot 614523-\frac{4}{45}\cdot 614532-\frac{2}{45}\cdot 623514-\frac{2}{45}\cdot 632514$$
$$-\frac{2}{45}\cdot 641532-\frac{4}{45}\cdot 615342-\frac{2}{15}\cdot 651324-\frac{2}{15}\cdot 651243-\frac{4}{15}\cdot 652143+\frac{2}{45}\cdot 625314$$
$$+\frac{2}{45}\cdot 631524-\frac{4}{45}\cdot 615423-\frac{2}{45}\cdot 624513-\frac{2}{45}\cdot 625413+\frac{4}{45}\cdot 561423+\frac{4}{45}\cdot 651423$$
$$+\frac{2}{45}\cdot 562413+\frac{2}{45}\cdot 652413+\frac{2}{45}\cdot 631245+\frac{2}{45}\cdot 631254-\frac{2}{45}\cdot 631452-\frac{2}{45}\cdot 631542$$
$$-\frac{8}{45}\cdot 634125-\frac{4}{45}\cdot 634215-\frac{2}{45}\cdot 635214-\frac{4}{45}\cdot 642315-\frac{2}{15}\cdot 652134-\frac{2}{45}\cdot 634152$$
$$-\frac{4}{45}\cdot 643125-\frac{2}{45}\cdot 643152+\frac{4}{45}\cdot 563124+\frac{2}{45}\cdot 563142+\frac{4}{45}\cdot 653124+\frac{2}{45}\cdot 653142$$
$$+\frac{2}{15}\cdot 634512+\frac{2}{15}\cdot 634521+\frac{2}{45}\cdot 635412+\frac{2}{45}\cdot 635421+\frac{4}{15}\cdot 652341+\frac{4}{45}\cdot 652431$$
$$+\frac{2}{45}\cdot 643512+\frac{2}{45}\cdot 643521+\frac{4}{45}\cdot 653241+\frac{2}{5}\cdot 654123+\frac{2}{15}\cdot 654132+\frac{2}{15}\cdot 654213$$

$$[\![y_4\times y_5]\!]=\frac{1}{15}\cdot 124563+\frac{1}{15}\cdot 214563-\frac{2}{45}\cdot 125634-\frac{2}{45}\cdot 215634+\frac{1}{15}\cdot 134526+\frac{1}{45}\cdot 314625$$
$$-\frac{1}{45}\cdot 135462-\frac{1}{90}\cdot 136452-\frac{1}{30}\cdot 316452+\frac{1}{45}\cdot 351462-\frac{1}{15}\cdot 361452-\frac{2}{45}\cdot 145236$$
$$+\frac{1}{45}\cdot 146253-\frac{1}{15}\cdot 412563-\frac{1}{45}\cdot 421563-\frac{1}{45}\cdot 143562-\frac{2}{45}\cdot 143652+\frac{1}{15}\cdot 145632$$
$$+\frac{1}{45}\cdot 146532+\frac{1}{30}\cdot 245631+\frac{1}{45}\cdot 415632-\frac{1}{90}\cdot 425631+\frac{1}{90}\cdot 152463+\frac{1}{90}\cdot 152643$$
$$+\frac{4}{45}\cdot 156243+\frac{1}{90}\cdot 251463+\frac{1}{30}\cdot 251643+\frac{2}{45}\cdot 256143+\frac{2}{45}\cdot 156324+\frac{1}{15}\cdot 256314$$
$$-\frac{2}{45}\cdot 256341-\frac{1}{90}\cdot 153462+\frac{1}{15}\cdot 163452-\frac{1}{45}\cdot 513462+\frac{1}{90}\cdot 531462+\frac{1}{30}\cdot 613452$$
$$-\frac{1}{18}\cdot 631452-\frac{1}{18}\cdot 154263-\frac{1}{15}\cdot 154623-\frac{2}{45}\cdot 156423-\frac{4}{45}\cdot 254163-\frac{1}{30}\cdot 254613$$
$$-\frac{4}{45}\cdot 164523-\frac{2}{45}\cdot 514623-\frac{2}{15}\cdot 614523+\frac{2}{45}\cdot 125463+\frac{2}{45}\cdot 215463-\frac{1}{45}\cdot 124635$$
$$-\frac{1}{45}\cdot 214635+\frac{2}{45}\cdot 143526-\frac{1}{45}\cdot 134652+\frac{1}{90}\cdot 461352-\frac{1}{45}\cdot 135246-\frac{1}{30}\cdot 145263$$
$$-\frac{2}{45}\cdot 245163-\frac{1}{45}\cdot 512463-\frac{1}{45}\cdot 521463-\frac{1}{90}\cdot 145362-\frac{1}{90}\cdot 135642+\frac{1}{45}\cdot 154632$$
$$+\frac{1}{30}\cdot 254631-\frac{1}{90}\cdot 246153+\frac{1}{30}\cdot 146325+\frac{1}{30}\cdot 246315-\frac{1}{45}\cdot 146352-\frac{1}{45}\cdot 246351$$
$$+\frac{1}{90}\cdot 614352-\frac{1}{15}\cdot 146523-\frac{1}{30}\cdot 246513-\frac{1}{30}\cdot 136524-\frac{1}{45}\cdot 163524-\frac{1}{45}\cdot 613524$$
$$+\frac{2}{45}\cdot 125643+\frac{2}{45}\cdot 215643+\frac{1}{90}\cdot 351642-\frac{2}{45}\cdot 126435-\frac{2}{45}\cdot 216435+\frac{2}{45}\cdot 145326$$

$$+\frac{1}{30}\cdot 415362-\frac{2}{45}\cdot 461532-\frac{2}{45}\cdot 153246+\frac{1}{45}\cdot 153624-\frac{1}{45}\cdot 512643+\frac{1}{45}\cdot 521643$$
$$+\frac{1}{15}\cdot 156432+\frac{1}{45}\cdot 516423+\frac{1}{15}\cdot 516432+\frac{1}{30}\cdot 162543+\frac{2}{45}\cdot 163542+\frac{1}{30}\cdot 261543$$
$$+\frac{1}{30}\cdot 164235+\frac{1}{30}\cdot 164325-\frac{1}{45}\cdot 264153+\frac{1}{45}\cdot 164532-\frac{1}{30}\cdot 264351+\frac{2}{45}\cdot 165243$$
$$-\frac{1}{45}\cdot 165342-\frac{1}{45}\cdot 265143-\frac{1}{90}\cdot 615324+\frac{2}{45}\cdot 124653+\frac{2}{45}\cdot 214653-\frac{2}{45}\cdot 126534$$
$$-\frac{2}{45}\cdot 216534+\frac{2}{45}\cdot 135426-\frac{1}{30}\cdot 136542-\frac{1}{30}\cdot 316542-\frac{2}{45}\cdot 361542+\frac{1}{45}\cdot 416532$$
$$-\frac{2}{45}\cdot 154236-\frac{2}{45}\cdot 412653-\frac{1}{30}\cdot 154362+\frac{1}{30}\cdot 246531+\frac{1}{90}\cdot 426531-\frac{1}{45}\cdot 526431$$
$$+\frac{1}{90}\cdot 162453+\frac{1}{90}\cdot 261453+\frac{2}{45}\cdot 265314+\frac{1}{30}\cdot 613542-\frac{1}{45}\cdot 614532-\frac{1}{30}\cdot 631542$$
$$-\frac{1}{45}\cdot 641532-\frac{1}{15}\cdot 165423-\frac{1}{15}\cdot 615423+\frac{1}{90}\cdot 316425-\frac{1}{30}\cdot 315642+\frac{1}{30}\cdot 513642$$
$$-\frac{1}{45}\cdot 531642+\frac{1}{15}\cdot 234156+\frac{1}{15}\cdot 234165-\frac{1}{45}\cdot 243516-\frac{1}{90}\cdot 253416-\frac{2}{45}\cdot 341256$$
$$-\frac{2}{45}\cdot 341265-\frac{1}{45}\cdot 351624+\frac{2}{45}\cdot 341562+\frac{1}{15}\cdot 341652+\frac{1}{45}\cdot 351426-\frac{1}{45}\cdot 324516$$
$$-\frac{2}{45}\cdot 325416-\frac{1}{30}\cdot 342615+\frac{1}{15}\cdot 345216+\frac{1}{45}\cdot 354216+\frac{1}{30}\cdot 362415+\frac{1}{30}\cdot 345261$$
$$+\frac{1}{90}\cdot 413526+\frac{1}{90}\cdot 415326+\frac{4}{45}\cdot 451326+\frac{2}{45}\cdot 452136+\frac{4}{45}\cdot 452163+\frac{1}{15}\cdot 452613$$
$$-\frac{2}{45}\cdot 452361-\frac{2}{45}\cdot 452631-\frac{1}{90}\cdot 423516+\frac{1}{15}\cdot 523416+\frac{1}{30}\cdot 623415-\frac{1}{18}\cdot 431526$$
$$-\frac{1}{15}\cdot 435126-\frac{2}{45}\cdot 453126-\frac{1}{30}\cdot 435162-\frac{4}{45}\cdot 534126-\frac{2}{15}\cdot 634125-\frac{2}{45}\cdot 634152$$
$$-\frac{1}{45}\cdot 315264-\frac{1}{45}\cdot 415263+\frac{2}{45}\cdot 324156+\frac{2}{45}\cdot 324165-\frac{1}{45}\cdot 235416-\frac{1}{45}\cdot 241356$$
$$-\frac{1}{45}\cdot 241365+\frac{1}{45}\cdot 241563+\frac{1}{45}\cdot 241653-\frac{1}{30}\cdot 341526-\frac{1}{90}\cdot 342516-\frac{1}{90}\cdot 245316$$
$$+\frac{1}{45}\cdot 346215+\frac{1}{45}\cdot 435216+\frac{1}{30}\cdot 435261+\frac{1}{30}\cdot 352146+\frac{1}{30}\cdot 352164+\frac{1}{90}\cdot 352614$$
$$-\frac{1}{45}\cdot 352416-\frac{1}{45}\cdot 352461-\frac{1}{45}\cdot 352641+\frac{1}{30}\cdot 632415-\frac{1}{15}\cdot 354126-\frac{1}{30}\cdot 254136$$
$$-\frac{1}{90}\cdot 264135-\frac{1}{30}\cdot 354162-\frac{1}{15}\cdot 364125-\frac{1}{30}\cdot 364152-\frac{1}{45}\cdot 524136-\frac{2}{45}\cdot 524163$$
$$-\frac{1}{45}\cdot 624135-\frac{1}{45}\cdot 236145-\frac{1}{45}\cdot 236154+\frac{1}{90}\cdot 263514+\frac{1}{45}\cdot 361245+\frac{1}{45}\cdot 361254$$
$$+\frac{1}{45}\cdot 325614-\frac{1}{45}\cdot 356214-\frac{1}{15}\cdot 365214+\frac{1}{90}\cdot 346251-\frac{1}{90}\cdot 413625-\frac{2}{45}\cdot 416325$$
$$+\frac{1}{90}\cdot 461325-\frac{1}{90}\cdot 462135-\frac{1}{90}\cdot 462153+\frac{1}{45}\cdot 462351+\frac{1}{45}\cdot 462531-\frac{1}{30}\cdot 423615$$
$$-\frac{1}{15}\cdot 523614+\frac{1}{90}\cdot 623514-\frac{1}{90}\cdot 431625+\frac{1}{45}\cdot 436125+\frac{1}{45}\cdot 463125+\frac{1}{30}\cdot 436152$$
$$-\frac{1}{45}\cdot 536142-\frac{1}{45}\cdot 635124+\frac{2}{45}\cdot 635142+\frac{1}{45}\cdot 134625+\frac{1}{45}\cdot 143625+\frac{1}{30}\cdot 315624$$
$$-\frac{1}{45}\cdot 136245-\frac{1}{45}\cdot 136254-\frac{1}{45}\cdot 316245-\frac{1}{45}\cdot 316254+\frac{1}{45}\cdot 235146+\frac{1}{45}\cdot 235164$$
$$+\frac{1}{45}\cdot 325146+\frac{1}{45}\cdot 325164-\frac{1}{45}\cdot 236514-\frac{1}{45}\cdot 251346-\frac{1}{45}\cdot 251436-\frac{1}{30}\cdot 351264$$

$$+\frac{1}{90}\cdot 251634-\frac{1}{90}\cdot 341625-\frac{1}{45}\cdot 513624+\frac{1}{45}\cdot 436215+\frac{1}{30}\cdot 436251+\frac{1}{30}\cdot 361524$$
$$+\frac{1}{45}\cdot 362145+\frac{1}{45}\cdot 362154-\frac{1}{90}\cdot 362451-\frac{1}{30}\cdot 362541+\frac{1}{30}\cdot 632514-\frac{1}{90}\cdot 625134$$
$$-\frac{1}{30}\cdot 625143-\frac{1}{45}\cdot 235641-\frac{1}{45}\cdot 325641+\frac{1}{45}\cdot 236451+\frac{1}{45}\cdot 326451-\frac{1}{45}\cdot 245361$$
$$+\frac{1}{45}\cdot 253461-\frac{1}{90}\cdot 253164+\frac{1}{90}\cdot 523641-\frac{1}{90}\cdot 532641-\frac{1}{45}\cdot 356421+\frac{1}{90}\cdot 263541$$
$$-\frac{2}{45}\cdot 364215+\frac{2}{45}\cdot 364512+\frac{1}{45}\cdot 364521-\frac{1}{45}\cdot 624531+\frac{1}{45}\cdot 365142-\frac{1}{90}\cdot 152634$$
$$-\frac{1}{90}\cdot 415236-\frac{1}{90}\cdot 416253-\frac{1}{90}\cdot 425163-\frac{1}{45}\cdot 413562-\frac{1}{45}\cdot 413652+\frac{1}{45}\cdot 431562$$
$$+\frac{2}{45}\cdot 431652+\frac{2}{45}\cdot 451362+\frac{1}{45}\cdot 463152-\frac{1}{15}\cdot 451632-\frac{1}{30}\cdot 516324-\frac{1}{90}\cdot 526314$$
$$+\frac{2}{45}\cdot 516342-\frac{1}{18}\cdot 524613+\frac{1}{45}\cdot 526413+\frac{1}{45}\cdot 542163+\frac{1}{45}\cdot 412635+\frac{1}{45}\cdot 421635$$
$$+\frac{1}{45}\cdot 512634+\frac{1}{15}\cdot 521634+\frac{1}{90}\cdot 346152+\frac{1}{45}\cdot 451263-\frac{1}{9}\cdot 541632-\frac{1}{45}\cdot 542631$$
$$-\frac{1}{45}\cdot 426153-\frac{1}{90}\cdot 516243-\frac{1}{90}\cdot 526143-\frac{1}{45}\cdot 426315+\frac{1}{45}\cdot 426351-\frac{1}{45}\cdot 643152$$
$$+\frac{1}{15}\cdot 416523+\frac{1}{30}\cdot 426513+\frac{1}{30}\cdot 316524+\frac{2}{45}\cdot 631524+\frac{2}{45}\cdot 342156+\frac{2}{45}\cdot 342165$$
$$-\frac{2}{45}\cdot 421356-\frac{2}{45}\cdot 421365+\frac{1}{45}\cdot 425136+\frac{1}{30}\cdot 426135+\frac{1}{15}\cdot 453216+\frac{1}{15}\cdot 463215$$
$$+\frac{1}{30}\cdot 514326+\frac{2}{45}\cdot 524316+\frac{1}{30}\cdot 531246-\frac{1}{90}\cdot 531264+\frac{1}{30}\cdot 532146+\frac{1}{30}\cdot 532164$$
$$-\frac{1}{30}\cdot 532461+\frac{1}{45}\cdot 534216+\frac{2}{45}\cdot 541326-\frac{1}{45}\cdot 542316-\frac{1}{30}\cdot 642135-\frac{1}{18}\cdot 642153$$
$$+\frac{2}{45}\cdot 243156+\frac{2}{45}\cdot 243165-\frac{1}{30}\cdot 254316-\frac{2}{45}\cdot 431256-\frac{2}{45}\cdot 431265-\frac{1}{30}\cdot 432516$$
$$-\frac{1}{30}\cdot 432615+\frac{1}{30}\cdot 354261+\frac{1}{90}\cdot 513426+\frac{1}{15}\cdot 542613+\frac{1}{18}\cdot 624315-\frac{1}{15}\cdot 634215$$
$$-\frac{1}{15}\cdot 543126-\frac{1}{45}\cdot 643125-\frac{1}{90}\cdot 514263-\frac{1}{90}\cdot 531624-\frac{1}{45}\cdot 342561-\frac{1}{45}\cdot 342651$$
$$+\frac{1}{45}\cdot 423561+\frac{1}{45}\cdot 423651+\frac{1}{90}\cdot 425613-\frac{1}{45}\cdot 453621-\frac{1}{45}\cdot 514362+\frac{1}{90}\cdot 524361$$
$$-\frac{2}{45}\cdot 536214+\frac{2}{45}\cdot 534612+\frac{1}{45}\cdot 534621-\frac{1}{45}\cdot 634251+\frac{1}{45}\cdot 541362+\frac{2}{45}\cdot 642351$$
$$-\frac{1}{90}\cdot 135624-\frac{1}{15}\cdot 145623+\frac{1}{15}\cdot 156234-\frac{1}{90}\cdot 245136-\frac{1}{15}\cdot 345126-\frac{1}{30}\cdot 345162$$
$$-\frac{1}{45}\cdot 346125+\frac{2}{45}\cdot 354612+\frac{1}{15}\cdot 451236+\frac{1}{30}\cdot 461235+\frac{1}{45}\cdot 415623+\frac{2}{45}\cdot 435612$$
$$+\frac{4}{45}\cdot 436512-\frac{1}{15}\cdot 456213-\frac{1}{15}\cdot 456312-\frac{2}{45}\cdot 465213-\frac{1}{45}\cdot 465312-\frac{1}{45}\cdot 356241$$
$$-\frac{1}{15}\cdot 456231-\frac{2}{45}\cdot 561324+\frac{1}{45}\cdot 561423-\frac{2}{45}\cdot 562134-\frac{4}{45}\cdot 562143+\frac{1}{15}\cdot 562341$$
$$+\frac{2}{45}\cdot 562431-\frac{1}{15}\cdot 624513+\frac{1}{15}\cdot 546123+\frac{1}{15}\cdot 563124+\frac{2}{15}\cdot 564123-\frac{2}{45}\cdot 546132$$
$$+\frac{2}{15}\cdot 645123+\frac{2}{45}\cdot 645132-\frac{1}{30}\cdot 245613+\frac{1}{45}\cdot 256134-\frac{1}{90}\cdot 461253-\frac{1}{15}\cdot 456132$$
$$-\frac{2}{45}\cdot 465132-\frac{2}{45}\cdot 561243-\frac{1}{45}\cdot 562314+\frac{1}{45}\cdot 561342-\frac{2}{45}\cdot 546213+\frac{2}{45}\cdot 564213$$

$$+\frac{1}{30}\cdot 516234+\frac{2}{45}\cdot 346512-\frac{1}{45}\cdot 546231-\frac{1}{45}\cdot 643512+\frac{1}{15}\cdot 465123+\frac{1}{90}\cdot 146235$$
$$+\frac{1}{30}\cdot 526134+\frac{1}{90}\cdot 351246+\frac{1}{45}\cdot 356142-\frac{1}{45}\cdot 162435-\frac{1}{45}\cdot 261435-\frac{1}{45}\cdot 513246$$
$$+\frac{1}{45}\cdot 513264-\frac{1}{45}\cdot 514632+\frac{1}{15}\cdot 561432+\frac{2}{45}\cdot 564132+\frac{1}{15}\cdot 612543+\frac{1}{15}\cdot 621543$$
$$+\frac{2}{45}\cdot 614235+\frac{1}{15}\cdot 614325-\frac{2}{45}\cdot 624351-\frac{2}{45}\cdot 615342-\frac{4}{45}\cdot 651243-\frac{8}{45}\cdot 652143$$
$$-\frac{4}{45}\cdot 651324-\frac{1}{90}\cdot 162534-\frac{1}{90}\cdot 261534-\frac{1}{90}\cdot 514236+\frac{1}{45}\cdot 612453+\frac{1}{45}\cdot 621453$$
$$+\frac{1}{30}\cdot 625314-\frac{2}{45}\cdot 625413-\frac{1}{30}\cdot 641253+\frac{1}{45}\cdot 612534+\frac{1}{45}\cdot 621534+\frac{1}{90}\cdot 615243$$
$$-\frac{2}{45}\cdot 163245-\frac{2}{45}\cdot 163254-\frac{2}{45}\cdot 263145-\frac{2}{45}\cdot 263154-\frac{2}{45}\cdot 521346-\frac{2}{45}\cdot 521436$$
$$-\frac{1}{30}\cdot 523164+\frac{1}{15}\cdot 563214+\frac{1}{15}\cdot 631245+\frac{1}{15}\cdot 631254+\frac{1}{15}\cdot 632145+\frac{1}{15}\cdot 632154$$
$$-\frac{1}{15}\cdot 632451-\frac{4}{45}\cdot 632541-\frac{2}{45}\cdot 635214-\frac{1}{90}\cdot 641325-\frac{2}{45}\cdot 642315-\frac{2}{45}\cdot 652314$$
$$-\frac{4}{45}\cdot 652134+\frac{1}{90}\cdot 136425+\frac{1}{90}\cdot 253146+\frac{1}{90}\cdot 364251+\frac{2}{45}\cdot 642513+\frac{2}{45}\cdot 645213$$
$$-\frac{1}{45}\cdot 623145-\frac{1}{45}\cdot 623154+\frac{2}{45}\cdot 653124+\frac{1}{30}\cdot 263451+\frac{1}{30}\cdot 523461+\frac{1}{45}\cdot 536241$$
$$-\frac{2}{45}\cdot 564231-\frac{1}{45}\cdot 463512-\frac{1}{45}\cdot 463521-\frac{2}{15}\cdot 563412-\frac{2}{45}\cdot 563421+\frac{1}{15}\cdot 634521$$
$$+\frac{1}{45}\cdot 635412+\frac{2}{45}\cdot 635421-\frac{1}{45}\cdot 635241-\frac{2}{45}\cdot 645231+\frac{1}{30}\cdot 641352+\frac{2}{15}\cdot 652341$$
$$+\frac{1}{15}\cdot 652431+\frac{1}{90}\cdot 163425+\frac{1}{90}\cdot 523146+\frac{1}{90}\cdot 524631-\frac{1}{45}\cdot 623541+\frac{1}{45}\cdot 653241$$
$$+\frac{1}{15}\cdot 165234+\frac{1}{15}\cdot 365412+\frac{1}{15}\cdot 541236+\frac{1}{15}\cdot 543612-\frac{2}{45}\cdot 564312-\frac{1}{45}\cdot 465231$$
$$-\frac{2}{45}\cdot 645312+\frac{1}{5}\cdot 654123+\frac{1}{15}\cdot 654132+\frac{1}{15}\cdot 654213+\frac{1}{30}\cdot 615234+\frac{1}{30}\cdot 641235$$
$$-\frac{1}{45}\cdot 546312-\frac{1}{45}\cdot 562413-\frac{1}{45}\cdot 652413-\frac{2}{45}\cdot 653412$$

$$[\![y_5\times y_5]\!]=\frac{2}{45}\cdot 124563+\frac{2}{45}\cdot 125463+\frac{2}{45}\cdot 214563+\frac{2}{45}\cdot 215463-\frac{2}{45}\cdot 124635-\frac{2}{45}\cdot 125634$$
$$-\frac{2}{45}\cdot 214635-\frac{2}{45}\cdot 215634+\frac{2}{45}\cdot 134526+\frac{2}{45}\cdot 143526-\frac{2}{45}\cdot 134652-\frac{2}{45}\cdot 143652$$
$$-\frac{2}{45}\cdot 316452-\frac{2}{45}\cdot 361452-\frac{2}{45}\cdot 416352-\frac{2}{45}\cdot 461352-\frac{2}{45}\cdot 135246-\frac{2}{45}\cdot 145236$$
$$-\frac{2}{45}\cdot 145263-\frac{2}{45}\cdot 154263-\frac{2}{45}\cdot 245163-\frac{4}{45}\cdot 254163-\frac{4}{45}\cdot 412563-\frac{2}{45}\cdot 421563$$
$$-\frac{2}{45}\cdot 512463-\frac{2}{45}\cdot 521463-\frac{1}{45}\cdot 135462-\frac{1}{45}\cdot 145362+\frac{1}{45}\cdot 135642+\frac{1}{15}\cdot 145632$$
$$+\frac{2}{45}\cdot 154632+\frac{2}{45}\cdot 245631+\frac{1}{45}\cdot 254631+\frac{1}{45}\cdot 146253+\frac{1}{45}\cdot 156243+\frac{1}{45}\cdot 246153$$
$$+\frac{1}{45}\cdot 256143-\frac{2}{45}\cdot 146352-\frac{2}{45}\cdot 156342-\frac{2}{45}\cdot 246351-\frac{4}{45}\cdot 256341+\frac{4}{45}\cdot 163452$$
$$+\frac{2}{45}\cdot 164352+\frac{2}{45}\cdot 613452+\frac{1}{45}\cdot 614352-\frac{1}{45}\cdot 146523-\frac{2}{45}\cdot 156423-\frac{1}{45}\cdot 246513$$

$$+\frac{1}{45}\cdot 256413-\frac{2}{45}\cdot 163524-\frac{2}{45}\cdot 164523-\frac{2}{45}\cdot 613524-\frac{4}{45}\cdot 614523+\frac{2}{45}\cdot 126345$$
$$+\frac{2}{45}\cdot 126354+\frac{2}{45}\cdot 216345+\frac{2}{45}\cdot 216354-\frac{2}{45}\cdot 315264-\frac{2}{45}\cdot 415263+\frac{2}{45}\cdot 316524$$
$$+\frac{2}{45}\cdot 361524+\frac{1}{9}\cdot 416523+\frac{2}{45}\cdot 461523+\frac{2}{45}\cdot 152346+\frac{2}{45}\cdot 152436-\frac{2}{45}\cdot 152634$$
$$-\frac{2}{45}\cdot 152643+\frac{2}{45}\cdot 412635+\frac{2}{45}\cdot 421635+\frac{2}{45}\cdot 512634+\frac{4}{45}\cdot 521634+\frac{1}{45}\cdot 153624$$
$$+\frac{1}{45}\cdot 154623-\frac{1}{45}\cdot 156324-\frac{4}{45}\cdot 416325-\frac{2}{45}\cdot 426315-\frac{2}{45}\cdot 516324-\frac{2}{45}\cdot 526314$$
$$-\frac{1}{45}\cdot 162435-\frac{1}{45}\cdot 162534-\frac{1}{45}\cdot 261435-\frac{1}{45}\cdot 261534-\frac{2}{45}\cdot 163245-\frac{2}{45}\cdot 163254$$
$$-\frac{2}{45}\cdot 263145-\frac{2}{45}\cdot 263154+\frac{2}{45}\cdot 163542+\frac{2}{45}\cdot 263451+\frac{2}{45}\cdot 263541+\frac{1}{45}\cdot 164235$$
$$+\frac{1}{15}\cdot 165234+\frac{1}{45}\cdot 264135+\frac{1}{45}\cdot 265134+\frac{2}{45}\cdot 165243+\frac{2}{45}\cdot 615234+\frac{2}{45}\cdot 615243$$
$$+\frac{2}{45}\cdot 234156+\frac{2}{45}\cdot 234165+\frac{2}{45}\cdot 324156+\frac{2}{45}\cdot 324165-\frac{2}{45}\cdot 235416-\frac{2}{45}\cdot 236415$$
$$-\frac{2}{45}\cdot 325416-\frac{2}{45}\cdot 326415-\frac{2}{45}\cdot 241356-\frac{2}{45}\cdot 241365-\frac{2}{45}\cdot 341256-\frac{2}{45}\cdot 341265$$
$$+\frac{2}{45}\cdot 241563+\frac{2}{45}\cdot 241653+\frac{2}{45}\cdot 341562+\frac{4}{45}\cdot 341652-\frac{2}{45}\cdot 341526-\frac{2}{45}\cdot 431526$$
$$-\frac{1}{45}\cdot 243516-\frac{1}{45}\cdot 243615-\frac{1}{45}\cdot 342516-\frac{1}{45}\cdot 342615+\frac{1}{45}\cdot 245316+\frac{1}{45}\cdot 246315$$
$$+\frac{1}{15}\cdot 345216+\frac{1}{45}\cdot 346215+\frac{2}{45}\cdot 345261+\frac{2}{45}\cdot 435216+\frac{2}{45}\cdot 435261+\frac{1}{45}\cdot 351426$$
$$+\frac{1}{45}\cdot 451326+\frac{2}{45}\cdot 352164+\frac{2}{45}\cdot 352614+\frac{1}{9}\cdot 452163+\frac{2}{45}\cdot 452613-\frac{2}{45}\cdot 352416$$
$$-\frac{2}{45}\cdot 352461-\frac{2}{45}\cdot 452316-\frac{4}{45}\cdot 452361+\frac{4}{45}\cdot 523416+\frac{2}{45}\cdot 532416+\frac{2}{45}\cdot 623415$$
$$+\frac{2}{45}\cdot 632415-\frac{1}{45}\cdot 354126-\frac{2}{45}\cdot 453126-\frac{2}{45}\cdot 264153-\frac{2}{45}\cdot 354162-\frac{2}{45}\cdot 364152$$
$$-\frac{2}{45}\cdot 524136-\frac{2}{45}\cdot 534126-\frac{2}{45}\cdot 624135-\frac{4}{45}\cdot 634125+\frac{2}{45}\cdot 235641+\frac{2}{45}\cdot 236541$$
$$+\frac{2}{45}\cdot 325641+\frac{2}{45}\cdot 326541+\frac{2}{45}\cdot 346152+\frac{2}{45}\cdot 431652+\frac{1}{45}\cdot 436152+\frac{1}{45}\cdot 254361$$
$$+\frac{1}{45}\cdot 264351+\frac{1}{45}\cdot 354261+\frac{1}{45}\cdot 364251-\frac{1}{45}\cdot 264531-\frac{2}{45}\cdot 354621-\frac{1}{45}\cdot 364521$$
$$-\frac{2}{45}\cdot 346521-\frac{4}{45}\cdot 436521-\frac{1}{45}\cdot 365142-\frac{2}{45}\cdot 465132-\frac{2}{45}\cdot 365214-\frac{2}{45}\cdot 465213$$
$$-\frac{2}{45}\cdot 265341-\frac{2}{45}\cdot 356241-\frac{2}{45}\cdot 365241-\frac{2}{45}\cdot 523641-\frac{2}{45}\cdot 532641-\frac{2}{45}\cdot 623541$$
$$-\frac{4}{45}\cdot 632541+\frac{1}{15}\cdot 365412+\frac{1}{45}\cdot 465312+\frac{2}{45}\cdot 265413+\frac{2}{45}\cdot 356412+\frac{2}{45}\cdot 412356$$
$$+\frac{2}{45}\cdot 412365+\frac{2}{45}\cdot 413256+\frac{2}{45}\cdot 413265-\frac{2}{45}\cdot 412653-\frac{2}{45}\cdot 413562-\frac{2}{45}\cdot 413652$$
$$-\frac{2}{45}\cdot 415236-\frac{2}{45}\cdot 415326-\frac{2}{45}\cdot 416235+\frac{1}{45}\cdot 425136+\frac{1}{45}\cdot 426135+\frac{1}{45}\cdot 435126$$
$$+\frac{1}{45}\cdot 436125-\frac{1}{45}\cdot 452136-\frac{1}{45}\cdot 462135+\frac{1}{45}\cdot 463125-\frac{1}{45}\cdot 513246-\frac{1}{45}\cdot 514236$$
$$-\frac{2}{45}\cdot 521346-\frac{2}{45}\cdot 521436-\frac{2}{45}\cdot 523164-\frac{2}{45}\cdot 523614-\frac{2}{45}\cdot 524163-\frac{2}{45}\cdot 524613$$

$$+ \frac{2}{45}\cdot 523461 + \frac{2}{45}\cdot 524316 + \frac{1}{45}\cdot 524361 + \frac{1}{45}\cdot 531246 + \frac{1}{15}\cdot 541236 + \frac{2}{45}\cdot 541326$$
$$+ \frac{2}{45}\cdot 641235 + \frac{1}{45}\cdot 641325 + \frac{2}{45}\cdot 415623 + \frac{1}{45}\cdot 415632 + \frac{2}{45}\cdot 416532 - \frac{1}{45}\cdot 425163$$
$$- \frac{2}{45}\cdot 426153 - \frac{1}{45}\cdot 435162 + \frac{1}{45}\cdot 453162 + \frac{1}{45}\cdot 462153 + \frac{1}{45}\cdot 463152 + \frac{1}{45}\cdot 513264$$
$$+ \frac{1}{45}\cdot 514263 + \frac{2}{45}\cdot 521643 + \frac{2}{45}\cdot 526134 + \frac{1}{45}\cdot 526143 - \frac{2}{45}\cdot 526341 - \frac{2}{45}\cdot 526431$$
$$- \frac{1}{45}\cdot 531264 + \frac{1}{45}\cdot 541263 - \frac{2}{45}\cdot 541623 - \frac{2}{15}\cdot 541632 - \frac{2}{45}\cdot 641523 - \frac{2}{45}\cdot 641532$$
$$+ \frac{2}{45}\cdot 451263 + \frac{2}{45}\cdot 542163 + \frac{1}{45}\cdot 315462 + \frac{1}{45}\cdot 415362 - \frac{1}{45}\cdot 315642 - \frac{2}{45}\cdot 451632$$
$$- \frac{2}{45}\cdot 452631 - \frac{2}{45}\cdot 542631 - \frac{1}{45}\cdot 416253 - \frac{1}{45}\cdot 516243 - \frac{2}{45}\cdot 634152 - \frac{2}{45}\cdot 643152$$
$$+ \frac{1}{45}\cdot 426513 + \frac{1}{45}\cdot 516423 + \frac{1}{45}\cdot 526413 + \frac{2}{45}\cdot 423561 + \frac{2}{45}\cdot 423651 + \frac{2}{45}\cdot 432561$$
$$+ \frac{2}{45}\cdot 432651 - \frac{2}{45}\cdot 425631 - \frac{2}{45}\cdot 426531 - \frac{2}{45}\cdot 435621 - \frac{2}{45}\cdot 453261 - \frac{2}{45}\cdot 462351$$
$$- \frac{2}{45}\cdot 463251 - \frac{1}{45}\cdot 453621 - \frac{2}{45}\cdot 513462 - \frac{2}{45}\cdot 514362 - \frac{2}{45}\cdot 531642 - \frac{2}{45}\cdot 536142$$
$$- \frac{2}{45}\cdot 546132 - \frac{1}{45}\cdot 536214 - \frac{2}{45}\cdot 546213 + \frac{1}{45}\cdot 536241 + \frac{1}{45}\cdot 546231 - \frac{1}{45}\cdot 534261$$
$$- \frac{2}{45}\cdot 624351 - \frac{1}{45}\cdot 634251 + \frac{2}{45}\cdot 534162 + \frac{2}{45}\cdot 534612 + \frac{2}{45}\cdot 543162 + \frac{1}{15}\cdot 543612$$
$$+ \frac{1}{45}\cdot 542613 + \frac{1}{45}\cdot 642513 + \frac{1}{45}\cdot 643512 + \frac{2}{45}\cdot 456231 + \frac{1}{9}\cdot 456321 + \frac{1}{45}\cdot 465231$$
$$+ \frac{2}{45}\cdot 465321 + \frac{1}{45}\cdot 356421 + \frac{2}{45}\cdot 516342 + \frac{2}{45}\cdot 516432 + \frac{2}{45}\cdot 561342 + \frac{1}{15}\cdot 561432$$
$$+ \frac{1}{15}\cdot 563214 + \frac{1}{45}\cdot 564213 + \frac{1}{45}\cdot 563241 - \frac{2}{45}\cdot 564231 + \frac{1}{45}\cdot 524631 + \frac{1}{45}\cdot 534621$$
$$+ \frac{1}{45}\cdot 624531 + \frac{1}{9}\cdot 634521 - \frac{2}{15}\cdot 563412 - \frac{2}{45}\cdot 564312 + \frac{1}{45}\cdot 546312 + \frac{1}{45}\cdot 645213$$
$$- \frac{2}{45}\cdot 645312 + \frac{2}{45}\cdot 456312 + \frac{2}{45}\cdot 546321 + \frac{1}{45}\cdot 461532 + \frac{1}{45}\cdot 462531 + \frac{1}{45}\cdot 562431$$
$$+ \frac{2}{45}\cdot 463215 + \frac{2}{45}\cdot 563124 - \frac{2}{45}\cdot 463512 - \frac{2}{45}\cdot 463521 - \frac{2}{45}\cdot 563421 + \frac{2}{45}\cdot 643521$$
$$+ \frac{1}{45}\cdot 564132 - \frac{2}{45}\cdot 635241 - \frac{2}{45}\cdot 645231 + \frac{2}{45}\cdot 612453 + \frac{2}{45}\cdot 612543 + \frac{2}{45}\cdot 621453$$
$$+ \frac{2}{45}\cdot 621543 + \frac{1}{45}\cdot 614325 + \frac{1}{45}\cdot 615324 + \frac{1}{45}\cdot 624315 + \frac{1}{45}\cdot 625314 - \frac{1}{45}\cdot 615342$$
$$- \frac{1}{45}\cdot 625341 + \frac{1}{45}\cdot 635142 + \frac{1}{45}\cdot 645132 - \frac{2}{45}\cdot 615423 - \frac{2}{45}\cdot 624513 - \frac{2}{45}\cdot 625413$$
$$- \frac{2}{45}\cdot 641253 - \frac{2}{45}\cdot 642153 - \frac{2}{45}\cdot 651243 - \frac{4}{45}\cdot 652143 - \frac{2}{45}\cdot 651324 - \frac{1}{45}\cdot 651423$$
$$+ \frac{2}{45}\cdot 631245 + \frac{2}{45}\cdot 631254 + \frac{2}{45}\cdot 632145 + \frac{2}{45}\cdot 632154 - \frac{2}{45}\cdot 631452 - \frac{2}{45}\cdot 631542$$
$$- \frac{2}{45}\cdot 632451 - \frac{2}{45}\cdot 634215 - \frac{2}{45}\cdot 635124 - \frac{2}{45}\cdot 635214 - \frac{1}{45}\cdot 642315 - \frac{1}{45}\cdot 652314$$
$$- \frac{2}{45}\cdot 652134 + \frac{2}{45}\cdot 634512 + \frac{1}{45}\cdot 635412 + \frac{2}{45}\cdot 635421 + \frac{1}{45}\cdot 641352 + \frac{1}{45}\cdot 642351$$
$$+ \frac{1}{45}\cdot 651342 + \frac{1}{9}\cdot 652341 + \frac{2}{45}\cdot 652431 + \frac{2}{45}\cdot 562341 + \frac{2}{45}\cdot 653241 - \frac{2}{45}\cdot 562413$$

$$
-\frac{2}{45}\cdot\mathtt{652413}-\frac{2}{45}\cdot\mathtt{653412}+\frac{2}{45}\cdot\mathtt{645123}+\frac{1}{9}\cdot\mathtt{654123}+\frac{2}{45}\cdot\mathtt{654213}+\frac{1}{45}\cdot\mathtt{653124}
+\frac{2}{45}\cdot\mathtt{564123}+\frac{2}{45}\cdot\mathtt{654132}
$$
