# Supplementary material for: Six Permutation Patterns Force Quasirandomness
Source: arXiv:2303.04776 ancillary file (2024-10-03)
Supplement: Supplementary file 2 [file OptimalityAppendix.pdf]

# Appendix B: Fuzzy Permutation and Cover Matrices

Our goal in this section is to establish the correspondence between fuzzy permutation matrices and cover matrices described in Lemma 4.5.

*Proof of Lemma 4.5.* Let $\sigma \in S_k$ and $n \geq k$ be fixed. For each triple $(S, T, \rho)$ such that $S = \{s_1 < \cdots < s_{n-k}\}$ and $T = \{t_1 < \cdots < t_{n-k}\}$ are subsets of $[n]$ of cardinality $n-k$ and $\rho \in S_{n-k}$, let $\sigma_{S,T,\rho}$ be the unique permutation in $S_n$ such that

- $\sigma_{S,T,\rho}(s_i) = t_{\rho(i)}$ for $1 \leq i \leq n-k$ and
- $[n] \setminus S$ is a copy of $\sigma$ in $\sigma_{S,T,\rho}$.

Note that different choices of $S, T$ and $\rho$ can yield the same permutation $\sigma_{S,T,\rho}$. For example, if $\sigma = 12$ and $\rho$ is the unique permutation of order one, then

$$\sigma_{\{1\},\{1\},\rho} = \sigma_{\{2\},\{2\},\rho} = \sigma_{\{3\},\{3\},\rho} = 123.$$

Now, for any permutation $\pi \in S_n$, it is evident that

$$d(\sigma, \pi) = \frac{|\{(S,T,\rho) : \sigma_{S,T,\rho} = \pi\}|}{\binom{n}{k}}.$$

Therefore, $A_\sigma^{\uparrow n}$ can be equivalently written as

$$A_\sigma^{\uparrow n} = \frac{1}{\binom{n}{k}} \sum_{\substack{S \subseteq [n] \\ |S| = n-k}} \sum_{\substack{T \subseteq [n] \\ |T| = n-k}} \sum_{\rho \in S_{n-k}} A_{\sigma_{S,T,\rho}}. \tag{B.1}$$

Now, for subsets $S = \{s_1 < \cdots < s_{n-k}\}$ and $T = \{t_1 < \cdots < t_{n-k}\}$ of $[n]$ of cardinality $n-k$ and $\rho \in S_{n-k}$, define $B_{S,T,\rho}$ to be the $n \times n$ matrix where $B_{S,T,\rho}(s_i, t_{\rho(i)}) = 1$ for $1 \leq i \leq n-k$ and all other entries of $B_{S,T,\rho}$ are zero. Define

$$C_{\sigma_{S,T,\rho}} := A_{\sigma_{S,T,\rho}} - B_{S,T,\rho}.$$

In other words, $C_{\sigma_{S,T,\rho}}$ encodes the copy of $\sigma$ on $[n] \setminus S$ in $A_{\sigma_{S,T,\rho}}$. By (B.1),

$$A_\sigma^{\uparrow n} = \frac{1}{\binom{n}{k}} \sum_{\substack{S \subseteq [n] \\ |S| = n-k}} \sum_{\substack{T \subseteq [n] \\ |T| = n-k}} \sum_{\rho \in S_{n-k}} B_{S,T,\rho} + \frac{1}{\binom{n}{k}} \sum_{\substack{S \subseteq [n] \\ |S| = n-k}} \sum_{\substack{T \subseteq [n] \\ |T| = n-k}} \sum_{\rho \in S_{n-k}} C_{\sigma_{S,T,\rho}}.$$

Thus, we will be done if we can establish the following two equalities:

$$\frac{1}{\binom{n}{k}} \sum_{\substack{S \subseteq [n] \\ |S| = n-k}} \sum_{\substack{T \subseteq [n] \\ |T| = n-k}} \sum_{\rho \in S_{n-k}} B_{S,T,\rho} = \frac{(n-1)!}{(k-1)!} \left( \frac{1}{k} - \frac{1}{n} \right) J_n \tag{B.2}$$

and

$$\frac{1}{\binom{n}{k}} \sum_{\substack{S \subseteq [n] \\ |S|=n-k}} \sum_{\substack{T \subseteq [n] \\ |T|=n-k}} \sum_{\rho \in S_{n-k}} C_{\sigma_{S,T,\rho}} = F_\sigma^{\uparrow n}. \tag{B.3}$$

We prove (B.2) first. For any $1 \leq i, j \leq n$, the number of choices of $(S, T, \rho)$ for which the support of $B_{S,T,\rho}$ contains the entry on the $i$th row and $j$th column is precisely $\binom{n-1}{n-k-1}^2 (n-k-1)!$. Thus, every entry of the matrix on the left side of (B.2) is equal to

$$\frac{\binom{n-1}{n-k-1}^2 (n-k-1)!}{\binom{n}{k}} = \frac{(n-1)!}{(k-1)!} \left( \frac{1}{k} - \frac{1}{n} \right)$$

and so (B.2) holds.

Finally, we prove (B.3). Let $1 \leq x, y \leq n$. Then the entry of the left side of (B.3) on the $x$th row and $y$th column is equal to $\binom{n}{k}^{-1}$ times the number of choices of $(j, S, T, \rho)$ such that

- $1 \leq j \leq k$,
- $S, T \subseteq [n]$ have cardinality $n - k$,
- $x$ is the $j$th smallest element of $[n] \setminus S$,
- $\sigma(j)$ is the $y$th smallest element of $[n] \setminus T$ and
- $\rho \in S_{n-k}$.

For a fixed $j$, the number of choices for $S$ is precisely

$$\binom{x-1}{j-1} \binom{n-x}{k-j} = f_{k,j}^{\uparrow n}(x).$$

Likewise, the number of choices for $T$ is

$$\binom{y-1}{\sigma(j)-1} \binom{n-y}{k-\sigma(j)} = f_{k,\sigma(j)}^{\uparrow n}(y).$$

The number of choices for $\rho$ is $(n-k)!$, regardless of the choice of $(j, S, T)$. So, the $(x, y)$ entry of the left side of (B.3) is

$$\frac{(n-k)!}{\binom{n}{k}} \sum_{j=1}^{k} f_{k,j}^{\uparrow n}(x) f_{k,\sigma(j)}^{\uparrow n}(y) = F_\sigma^{\uparrow n}(x, y).$$

This completes the proof. $\square$

# Appendix C: Constant Covers and Hessian Eigenvalues

Hessian matrices based on a $5\times5$ grid are computed $\mathbb{Q}$ as in [1] and use the same row/column labelling as in that paper's appendix `https://arxiv.org/src/1909.11027/anc/Appendices.pdf`. Here, since we encounter permutations lengths ranging from 2 to 5, we extended the calculation of Hessians accordingly. Note that knowing the Hessian matrices for all permutations of length 5 is enough to compute those for all smaller permutation lengths.

Type $(4,4,3,2)$

1. $\rho = 3(\texttt{3142}) + 3(\texttt{2413}) + 4(\texttt{123}) + 3(\texttt{21})$, $\lambda_{\min} = -0.3714$, $\lambda_{\max} = 0.2716$
2. $\rho = 3(\texttt{3412}) + 3(\texttt{2143}) + 4(\texttt{123}) + 3(\texttt{21})$, $\lambda_{\min} = -0.1540$, $\lambda_{\max} = 0.4923$
3. $\rho = 3(\texttt{4231}) + 3(\texttt{1324}) - 4(\texttt{123}) + 3(\texttt{12})$, $\lambda_{\min} = -0.4290$, $\lambda_{\max} = 0.2242$
4. $\rho = -3(\texttt{4231}) - 3(\texttt{1324}) + 4(\texttt{123}) + 3(\texttt{21})$, $\lambda_{\min} = -0.2242$, $\lambda_{\max} = 0.4290$
5. $\rho = 3(\texttt{4321}) + 3(\texttt{1234}) - 4(\texttt{123}) + 3(\texttt{12})$, $\lambda_{\min} = -0.2008$, $\lambda_{\max} = 0.4388$
6. $\rho = -3(\texttt{4321}) - 3(\texttt{1234}) + 4(\texttt{123}) + 3(\texttt{21})$, $\lambda_{\min} = -0.4388$, $\lambda_{\max} = 0.2008$

Type $(4,4,3,3)$

1. $\rho = 3(\texttt{3142}) + 3(\texttt{2413}) + 2(\texttt{321}) + 2(\texttt{123})$, $\lambda_{\min} = -0.1023$, $\lambda_{\max} = 0.06556$
2. $\rho = 3(\texttt{3412}) + 3(\texttt{2143}) + 2(\texttt{321}) + 2(\texttt{123})$, $\lambda_{\min}$ : ad hoc, $\lambda_{\max} = 0.2409$
3. $\rho = -3(\texttt{4231}) - 3(\texttt{1324}) + 2(\texttt{321}) + 2(\texttt{123})$, $\lambda_{\min}$ : ad hoc, $\lambda_{\max} = 0.1777$
4. $\rho = -3(\texttt{4321}) - 3(\texttt{1234}) + 2(\texttt{321}) + 2(\texttt{123})$, $\lambda_{\min} = -0.1735$, $\lambda_{\max} = 0.02801$

Type $(4,4,4,4)$

The nonzero constant covers of this type correspond to latin squares. There are 12 distinct covers, up to scaling and dihedral equivalence. However, none are quasirandom-forcing, as shown in [1].

Type $(5,5,4,3)$

1. $\rho = -36(\texttt{52341}) + 36(\texttt{12345}) + 15(\texttt{2143}) + 10(\texttt{321})$, $\lambda_{\min} = -1.662$, $\lambda_{\max} = 2.864$
2. $\rho = 36(\texttt{52341}) - 36(\texttt{12345}) + 15(\texttt{3412}) + 10(\texttt{123})$, $\lambda_{\min} = -1.986$, $\lambda_{\max} = 2.490$
3. $\rho = -36(\texttt{52431}) + 36(\texttt{12435}) + 15(\texttt{2143}) + 10(\texttt{321})$, $\lambda_{\min} = -1.703$, $\lambda_{\max} = 2.838$
4. $\rho = 36(\texttt{52431}) - 36(\texttt{12435}) + 15(\texttt{3412}) + 10(\texttt{123})$, $\lambda_{\min} = -1.961$, $\lambda_{\max} = 2.544$

Type $(4,4,3,2,2)$

Each of the constant covers $\rho$ listed in the case $(4,4,3,2)$ has a variant $\rho + t\nu$, where $\nu = \mathtt{12} + \mathtt{21}$. For $t \notin \{0,3\}$, this leads to a 5-term constant cover. However, the Hessian matrix for $\nu$ is zero. So, by linearity, the same eigenvalues as before can be used.

Type $(4,4,3,3,2)$

1. $\rho = -3(\mathtt{3142}) - 3(\mathtt{2413}) + 4(\mathtt{213}) + 4(\mathtt{132}) + 3(\mathtt{21})$, $\lambda_{\min} = -0.8939$, $\lambda_{\max} = 0.9958$
2. $\rho = -3(\mathtt{3412}) - 3(\mathtt{2143}) + 4(\mathtt{213}) + 4(\mathtt{132}) + 3(\mathtt{21})$, $\lambda_{\min} = -1.116$, $\lambda_{\max} = 0.7760$
3. $\rho = 3(\mathtt{4231}) + 3(\mathtt{1324}) + 4(\mathtt{213}) + 4(\mathtt{132}) - 3(\mathtt{12})$, $\lambda_{\min} = -1.049$, $\lambda_{\max} = 0.8443$
4. $\rho = 3(\mathtt{4231}) + 3(\mathtt{1324}) + 4(\mathtt{213}) + 4(\mathtt{132}) + 3(\mathtt{21})$, $\lambda_{\min} = -1.049$, $\lambda_{\max} = 0.8443$
5. $\rho = 3(\mathtt{4321}) + 3(\mathtt{1234}) + 4(\mathtt{213}) + 4(\mathtt{132}) - 3(\mathtt{12})$, $\lambda_{\min} = -0.8260$, $\lambda_{\max} = 1.064$
6. $\rho = 3(\mathtt{4321}) + 3(\mathtt{1234}) + 4(\mathtt{213}) + 4(\mathtt{132}) + 3(\mathtt{21})$, $\lambda_{\min} = -0.8260$, $\lambda_{\max} = 1.064$

Additionally, for each of the constant covers $\rho$ listed in the case $(4,4,3,3)$, we obtain a constant cover $\rho + t\xi$, where $\xi = 2(\mathtt{123}) - 2(\mathtt{321}) - 3(\mathtt{12})$. For generic values of $t \in \mathbb{R}$, this yields a 5-term constant cover whose list of permutation lengths is $(4,4,3,3,2)$.

To analyze the Hessian, we computed the zeros of the polynomial $\det(H_\rho + tH_\xi)$ and checked eigenvalues at rational values of $t$ interlacing these zeros. Eigenvalues of both signs exist except for $t$ in an interval around zero. An ad hoc construction is needed for

- $\rho = 3(\mathtt{3412}) + 3(\mathtt{2143}) + 2(\mathtt{321}) + 2(\mathtt{123}) + t\xi$ when $|t| < \frac{265-8\sqrt{185}}{385} \lessapprox 0.41651$; and
- $\rho = -3(\mathtt{4231}) - 3(\mathtt{1324}) + 2(\mathtt{321}) + 2(\mathtt{123}) + t\xi$ when $|t| < 0.15162$.

Type $(4,4,3,3,3)$

1. $\rho = 3(\mathtt{4231}) + 3(\mathtt{1324}) + 2(\mathtt{213}) + 2(\mathtt{132}) - 2(\mathtt{123})$, $\lambda_{\min} = -0.7369$, $\lambda_{\max} = 0.5321$
2. $\rho = 3(\mathtt{4321}) + 3(\mathtt{1234}) + 2(\mathtt{213}) + 2(\mathtt{132}) - 2(\mathtt{123})$, $\lambda_{\min} = -0.5125$, $\lambda_{\max} = 0.7504$

Type $(4,4,4,3,2)$

1. $\rho = -3(\mathtt{2143}) - 4(\mathtt{1324}) - 5(\mathtt{1234}) + 4(\mathtt{321}) + 6(\mathtt{12})$, $\lambda_{\min} = -0.3655$, $\lambda_{\max} = 0.2637$
2. $\rho = 3(\mathtt{2143}) + 4(\mathtt{1324}) + 5(\mathtt{1234}) - 4(\mathtt{321}) + 6(\mathtt{21})$, $\lambda_{\min} = -0.2637$, $\lambda_{\max} = 0.3655$
3. $\rho = 3(\mathtt{3412}) - 4(\mathtt{1324}) - 5(\mathtt{1234}) + 8(\mathtt{123}) + 3(\mathtt{21})$, $\lambda_{\min} = -0.6902$, $\lambda_{\max} = 0.7897$
4. $\rho = 3(\mathtt{3412}) - 4(\mathtt{1324}) - 5(\mathtt{1234}) + 8(\mathtt{321}) + 9(\mathtt{12})$, $\lambda_{\min} = -0.4752$, $\lambda_{\max} = 0.6128$

5. $\rho = -3(\texttt{3412}) + 4(\texttt{1324}) + 5(\texttt{1234}) - 8(\texttt{321}) + 9(\texttt{21})$, $\lambda_{\min} = -0.6128$, $\lambda_{\max} = 0.4752$
6. $\rho = 12(\texttt{4231}) - 9(\texttt{2143}) - 15(\texttt{1234}) - 4(\texttt{123}) + 12(\texttt{12})$, $\lambda_{\min} = -1.251$, $\lambda_{\max} = 0.006867$
7. $\rho = -12(\texttt{4231}) + 9(\texttt{2143}) + 15(\texttt{1234}) + 4(\texttt{123}) + 12(\texttt{21})$, $\lambda_{\min} = -0.006867$, $\lambda_{\max} = 1.251$
8. $\rho = 12(\texttt{4231}) - 9(\texttt{2143}) - 15(\texttt{1234}) - 4(\texttt{321}) + 6(\texttt{12})$, $\lambda_{\min} = -1.455$, $\lambda_{\max} = 0.09272$
9. $\rho = -12(\texttt{4231}) + 9(\texttt{2143}) + 15(\texttt{1234}) + 4(\texttt{321}) + 6(\texttt{21})$, $\lambda_{\min} = -0.09272$, $\lambda_{\max} = 1.455$
10. $\rho = 12(\texttt{4231}) + 9(\texttt{3412}) - 15(\texttt{1234}) + 8(\texttt{123}) + 3(\texttt{12})$, $\lambda_{\min} = -1.216$, $\lambda_{\max} = 0.8079$
11. $\rho = 12(\texttt{4231}) + 9(\texttt{3412}) - 15(\texttt{1234}) + 8(\texttt{123}) - 3(\texttt{21})$, $\lambda_{\min} = -1.216$, $\lambda_{\max} = 0.8079$
12. $\rho = 12(\texttt{4231}) + 9(\texttt{3412}) - 15(\texttt{1234}) + 8(\texttt{321}) + 15(\texttt{12})$, $\lambda_{\min} = -0.8428$, $\lambda_{\max} = 0.4083$
13. $\rho = -12(\texttt{4231}) - 9(\texttt{3412}) + 15(\texttt{1234}) - 8(\texttt{321}) + 15(\texttt{21})$, $\lambda_{\min} = -0.4083$, $\lambda_{\max} = 0.8428$

Type $(4,4,4,3,3)$

1. $\rho = 3(\texttt{2143}) + 4(\texttt{1324}) + 5(\texttt{1234}) + 4(\texttt{312}) + 4(\texttt{231})$, $\lambda_{\min} = -0.7426$, $\lambda_{\max} = 0.9626$
2. $\rho = 3(\texttt{3412}) - 4(\texttt{1324}) - 5(\texttt{1234}) + 2(\texttt{321}) + 6(\texttt{123})$, $\lambda_{\min} = -0.3819$, $\lambda_{\max} = 0.4776$
3. $\rho = -12(\texttt{4231}) + 9(\texttt{2143}) + 15(\texttt{1234}) + 8(\texttt{321}) - 4(\texttt{123})$, $\lambda_{\min} = -0.6306$, $\lambda_{\max} = 2.044$
4. $\rho = 12(\texttt{4231}) + 9(\texttt{3412}) - 15(\texttt{1234}) - 2(\texttt{321}) + 10(\texttt{123})$, $\lambda_{\min} = -1.524$, $\lambda_{\max} = 1.100$

Type $(4,4,4,4,2)$

1. $\rho = 3(\texttt{3412}) + 6(\texttt{2143}) + 4(\texttt{1324}) + 5(\texttt{1234}) + 3(\texttt{21})$, $\lambda_{\min} = -0.1212$, $\lambda_{\max} = 0.4770$
2. $\rho = 3(\texttt{4231}) - 3(\texttt{2143}) - 1(\texttt{1324}) - 5(\texttt{1234}) + 3(\texttt{12})$, $\lambda_{\min} = -0.3730$, $\lambda_{\max} = 0.02695$
3. $\rho = -3(\texttt{4231}) + 3(\texttt{2143}) + 1(\texttt{1324}) + 5(\texttt{1234}) + 3(\texttt{21})$, $\lambda_{\min} = -0.02695$, $\lambda_{\max} = 0.3730$
4. $\rho = 6(\texttt{4231}) + 3(\texttt{3412}) + 2(\texttt{1324}) - 5(\texttt{1234}) + 3(\texttt{12})$, $\lambda_{\min} = -0.3030$, $\lambda_{\max} = 0.07789$
5. $\rho = -6(\texttt{4231}) - 3(\texttt{3412}) - 2(\texttt{1324}) + 5(\texttt{1234}) + 3(\texttt{21})$, $\lambda_{\min} = -0.07789$, $\lambda_{\max} = 0.3030$
6. $\rho = 4(\texttt{4231}) + 1(\texttt{3412}) - 2(\texttt{2143}) - 5(\texttt{1234}) + 3(\texttt{12})$, $\lambda_{\min} = -0.3435$, $\lambda_{\max} = 0.003044$
7. $\rho = -4(\texttt{4231}) - 1(\texttt{3412}) + 2(\texttt{2143}) + 5(\texttt{1234}) + 3(\texttt{21})$, $\lambda_{\min} = -0.003044$, $\lambda_{\max} = 0.3435$
8. $\rho = 3(\texttt{4321}) - 3(\texttt{2143}) - 4(\texttt{1324}) - 2(\texttt{1234}) + 3(\texttt{12})$, $\lambda_{\min} = -0.1579$, $\lambda_{\max} = 0.1823$
9. $\rho = -3(\texttt{4321}) + 3(\texttt{2143}) + 4(\texttt{1324}) + 2(\texttt{1234}) + 3(\texttt{21})$, $\lambda_{\min} = -0.1823$, $\lambda_{\max} = 0.1579$

10. $\rho = 6(\texttt{4321}) + 3(\texttt{3412}) - 4(\texttt{1324}) + 1(\texttt{1234}) + 3(\texttt{12})$, $\lambda_{\min}$ : ad hoc, $\lambda_{\max} = 0.4649$
11. $\rho = -6(\texttt{4321}) - 3(\texttt{3412}) + 4(\texttt{1324}) - 1(\texttt{1234}) + 3(\texttt{21})$, $\lambda_{\min} = -0.4649$, $\lambda_{\max}$ : ad hoc

Type $(4, 4, 4, 4, 3)$

1. $\rho = 6(\texttt{3412}) + 9(\texttt{2143}) + 4(\texttt{1324}) + 5(\texttt{1234}) + 4(\texttt{321})$, $\lambda_{\min} = -0.09399$, $\lambda_{\max} = 0.9180$
2. $\rho = -6(\texttt{4231}) + 3(\texttt{2143}) - 2(\texttt{1324}) + 5(\texttt{1234}) + 4(\texttt{321})$, $\lambda_{\min} = -0.1665$, $\lambda_{\max} = 0.7548$
3. $\rho = 3(\texttt{4231}) + 3(\texttt{3412}) - 1(\texttt{1324}) - 5(\texttt{1234}) + 4(\texttt{123})$, $\lambda_{\min} = -0.4745$, $\lambda_{\max} = 0.3919$
4. $\rho = -4(\texttt{4231}) + 2(\texttt{3412}) + 5(\texttt{2134}) + 5(\texttt{1243}) + 4(\texttt{321})$, $\lambda_{\min} = -0.5446$, $\lambda_{\max} = 0.5487$
5. $\rho = 4(\texttt{4231}) + 4(\texttt{3412}) + 1(\texttt{2143}) - 5(\texttt{1234}) + 4(\texttt{123})$, $\lambda_{\min} = -0.4537$, $\lambda_{\max} = 0.4214$
6. $\rho = -4(\texttt{4231}) + 2(\texttt{3412}) + 5(\texttt{2143}) + 5(\texttt{1234}) + 4(\texttt{321})$, $\lambda_{\min} = -0.1158$, $\lambda_{\max} = 0.8038$
7. $\rho = 3(\texttt{4312}) + 3(\texttt{3421}) - 4(\texttt{1324}) - 2(\texttt{1234}) + 4(\texttt{123})$, $\lambda_{\min} = -0.5379$, $\lambda_{\max} = 0.4519$
8. $\rho = -6(\texttt{4321}) + 3(\texttt{2143}) + 4(\texttt{1324}) - 1(\texttt{1234}) + 4(\texttt{321})$, $\lambda_{\min} = -0.5490$, $\lambda_{\max} = 0.3332$
9. $\rho = 3(\texttt{4321}) + 3(\texttt{3412}) - 4(\texttt{1324}) - 2(\texttt{1234}) + 4(\texttt{123})$, $\lambda_{\min} = -0.2759$, $\lambda_{\max} = 0.5971$

Type $(5, 5, 4, 3, 2)$

1. $\rho = 36(\texttt{41352}) - 36(\texttt{25314}) + 30(\texttt{2413}) + 20(\texttt{123}) + 15(\texttt{21})$, $\lambda_{\min} = -2.141$, $\lambda_{\max} = 1.549$
2. $\rho = 36(\texttt{52341}) - 36(\texttt{12345}) - 15(\texttt{2143}) - 10(\texttt{123}) + 15(\texttt{12})$, $\lambda_{\min} = -1.590$, $\lambda_{\max} = 0.2512$
3. $\rho = -36(\texttt{52341}) + 36(\texttt{12345}) + 15(\texttt{2143}) + 10(\texttt{123}) + 15(\texttt{21})$, $\lambda_{\min} = -0.2512$, $\lambda_{\max} = 1.590$
4. $\rho = 36(\texttt{52341}) - 36(\texttt{12345}) + 15(\texttt{3412}) + 10(\texttt{321}) + 15(\texttt{12})$, $\lambda_{\min} = -0.7880$, $\lambda_{\max} = 1.075$
5. $\rho = -36(\texttt{52341}) + 36(\texttt{12345}) - 15(\texttt{3412}) - 10(\texttt{321}) + 15(\texttt{21})$, $\lambda_{\min} = -1.075$, $\lambda_{\max} = 0.7880$
6. $\rho = 36(\texttt{52431}) - 36(\texttt{12435}) - 15(\texttt{2143}) - 10(\texttt{123}) + 15(\texttt{12})$, $\lambda_{\min} = -1.480$, $\lambda_{\max} = 0.4482$
7. $\rho = -36(\texttt{52431}) + 36(\texttt{12435}) + 15(\texttt{2143}) + 10(\texttt{123}) + 15(\texttt{21})$, $\lambda_{\min} = -0.4482$, $\lambda_{\max} = 1.480$
8. $\rho = 36(\texttt{52431}) - 36(\texttt{12435}) + 15(\texttt{3412}) + 10(\texttt{321}) + 15(\texttt{12})$, $\lambda_{\min} = -0.6858$, $\lambda_{\max} = 1.152$
9. $\rho = -36(\texttt{52431}) + 36(\texttt{12435}) - 15(\texttt{3412}) - 10(\texttt{321}) + 15(\texttt{21})$, $\lambda_{\min} = -1.152$, $\lambda_{\max} = 0.6858$
10. $\rho = 12(\texttt{54321}) - 12(\texttt{12345}) + 15(\texttt{1234}) - 10(\texttt{123}) + 5(\texttt{12})$, $\lambda_{\min} = -0.2250$, $\lambda_{\max} = 0.8488$
11. $\rho = -12(\texttt{54321}) + 12(\texttt{12345}) - 15(\texttt{1234}) + 10(\texttt{123}) + 5(\texttt{21})$, $\lambda_{\min} = -0.8488$, $\lambda_{\max} = 0.2250$

12. $\rho = -12(\texttt{54321}) + 12(\texttt{12345}) - 15(\texttt{1234}) + 10(\texttt{321}) + 10(\texttt{12})$, $\lambda_{\min} = -1.372$, $\lambda_{\max} = 0.7884$
13. $\rho = 12(\texttt{54321}) - 12(\texttt{12345}) + 15(\texttt{1234}) - 10(\texttt{321}) + 10(\texttt{21})$, $\lambda_{\min} = -0.7884$, $\lambda_{\max} = 1.372$

Type $(5, 5, 4, 3, 3)$

1. $\rho = 18(\texttt{41352}) - 18(\texttt{25314}) + 15(\texttt{2413}) + 5(\texttt{321}) + 5(\texttt{123})$, $\lambda_{\min} = -0.6281$, $\lambda_{\max} = 0.2981$
2. $\rho = 36(\texttt{52341}) - 36(\texttt{12345}) - 15(\texttt{2143}) + 10(\texttt{213}) + 10(\texttt{132})$, $\lambda_{\min} = -2.198$, $\lambda_{\max} = 0.4102$
3. $\rho = -36(\texttt{52341}) + 36(\texttt{12345}) - 15(\texttt{3412}) + 10(\texttt{312}) + 10(\texttt{231})$, $\lambda_{\min} = -1.172$, $\lambda_{\max} = 1.355$
4. $\rho = 36(\texttt{52431}) - 36(\texttt{12435}) - 15(\texttt{2143}) + 10(\texttt{213}) + 10(\texttt{132})$, $\lambda_{\min} = -1.788$, $\lambda_{\max} = 0.8451$
5. $\rho = -36(\texttt{52431}) + 36(\texttt{12435}) - 15(\texttt{3412}) + 10(\texttt{312}) + 10(\texttt{231})$, $\lambda_{\min} = -1.627$, $\lambda_{\max} = 1.010$
6. $\rho = -36(\texttt{54321}) + 36(\texttt{12345}) - 45(\texttt{1234}) + 10(\texttt{321}) + 20(\texttt{123})$, $\lambda_{\min} = -1.353$, $\lambda_{\max} = 0.2427$

Type $(5, 5, 4, 4, 2)$

1. $\rho = -24(\texttt{45312}) + 24(\texttt{21354}) + 15(\texttt{3214}) + 15(\texttt{1432}) + 5(\texttt{21})$, $\lambda_{\min} = -1.942$, $\lambda_{\max} = 3.383$
2. $\rho = -24(\texttt{45312}) + 24(\texttt{21354}) + 15(\texttt{3412}) + 15(\texttt{1234}) + 5(\texttt{21})$, $\lambda_{\min} = -1.392$, $\lambda_{\max} = 2.833$
3. $\rho = 24(\texttt{52341}) - 24(\texttt{12345}) + 5(\texttt{3412}) - 5(\texttt{2143}) + 5(\texttt{12})$, $\lambda_{\min} = -1.093$, $\lambda_{\max} = 0.8920$
4. $\rho = -24(\texttt{52341}) + 24(\texttt{12345}) - 5(\texttt{3412}) + 5(\texttt{2143}) + 5(\texttt{21})$, $\lambda_{\min} = -0.8920$, $\lambda_{\max} = 1.093$
5. $\rho = 24(\texttt{52431}) - 24(\texttt{12435}) + 5(\texttt{3412}) - 5(\texttt{2143}) + 5(\texttt{12})$, $\lambda_{\min} = -1.095$, $\lambda_{\max} = 0.9056$
6. $\rho = -24(\texttt{52431}) + 24(\texttt{12435}) - 5(\texttt{3412}) + 5(\texttt{2143}) + 5(\texttt{21})$, $\lambda_{\min} = -0.9056$, $\lambda_{\max} = 1.095$
7. $\rho = -24(\texttt{54321}) + 24(\texttt{12345}) + 15(\texttt{4321}) - 15(\texttt{1234}) + 5(\texttt{12})$, $\lambda_{\min} = -0.5785$, $\lambda_{\max} = 0.5785$

Type $(5, 5, 4, 4, 3)$

1. $\rho = -36(\texttt{54321}) + 36(\texttt{12345}) + 15(\texttt{4321}) - 30(\texttt{1234}) + 10(\texttt{123})$,
$\lambda_{\min} = -0.5702$, $\lambda_{\max} = 0.1621$

Type $(5, 5, 4, 4, 4)$

1. $\rho = 12(\texttt{41352}) - 12(\texttt{25314}) + 5(\texttt{4231}) + 10(\texttt{2413}) + 5(\texttt{1324})$,
$\lambda_{\min} = -0.6199$, $\lambda_{\max} = 0.06927$

2. $\rho = 12(41352) - 12(25314) + 5(4321) + 10(2413) + 5(1234)$,
$\lambda_{\min} = -0.3764$, $\lambda_{\max} = 0.3705$

Type $(5, 5, 5, 5, 5)$

In a constant cover of this type, we have each coefficient equal to 1, and the permutations combining to create a $5 \times 5$ latin square. No such combination can be minimized by quasirandom permutations, since it cannot contain both 12345 and 54321. It is enough, then, to check that $\lambda_{\max} > 0$; this occurs in every case with the exception of one.

1. $\rho = 13254 + 21543 + 34125 + 45312 + 52431$, $\lambda_{\max} = 0.06664$
2. $\rho = 13245 + 21534 + 34152 + 45321 + 52413$, $\lambda_{\max} = 0.02870$
3. $\rho = 13524 + 21345 + 34152 + 45213 + 52431$, $\lambda_{\max} = 0.05002$
4. $\rho = 13542 + 21354 + 34125 + 45213 + 52431$, $\lambda_{\max} = 0.03943$
5. $\rho = 13524 + 21345 + 34152 + 45231 + 52413$, $\lambda_{\max} = 0.04257$
6. $\rho = 13542 + 21354 + 34125 + 45231 + 52413$, $\lambda_{\max} = 0.03722$
7. $\rho = 13425 + 21534 + 34152 + 45213 + 52341$, $\lambda_{\max} = 0.07658$
8. $\rho = 13452 + 21534 + 34125 + 45213 + 52341$, $\lambda_{\max} = 0.1035$
9. $\rho = 13425 + 21543 + 34152 + 45231 + 52314$, $\lambda_{\max} = 0.06499$
10. $\rho = 13452 + 21543 + 34125 + 45231 + 52314$, $\lambda_{\max} = 0.08216$
11. $\rho = 13524 + 21435 + 34152 + 45213 + 52341$, $\lambda_{\max} = 0.05778$
12. $\rho = 13542 + 21453 + 34125 + 45231 + 52314$, $\lambda_{\max} = 0.06132$
13. $\rho = 13245 + 21354 + 34512 + 45123 + 52431$, $\lambda_{\max} = 0.09914$
14. $\rho = 13254 + 21345 + 34512 + 45123 + 52431$, $\lambda_{\max} = 0.1024$
15. $\rho = 13245 + 21354 + 34521 + 45132 + 52413$, $\lambda_{\max} = 0.05048$
16. $\rho = 13254 + 21345 + 34521 + 45132 + 52413$, $\lambda_{\max} = 0.05872$
17. $\rho = 13254 + 21435 + 34512 + 45123 + 52341$, $\lambda_{\max} = 0.1117$
18. $\rho = 13245 + 21453 + 34521 + 45132 + 52314$, $\lambda_{\max} = 0.07616$
19. $\rho = 13542 + 21354 + 34215 + 45123 + 52431$, $\lambda_{\max} = 0.04367$
20. $\rho = 13524 + 21345 + 34251 + 45132 + 52413$, $\lambda_{\max} = 0.02789$
21. $\rho = 13452 + 21534 + 34215 + 45123 + 52341$, $\lambda_{\max} = 0.1097$
22. $\rho = 13425 + 21543 + 34251 + 45132 + 52314$, $\lambda_{\max} = 0.05558$

23. $\rho = 13524 + 21453 + 34215 + 45132 + 52341, \quad \lambda_{\max} = 0.04673$

24. $\rho = 13542 + 21435 + 34251 + 45123 + 52314, \quad \lambda_{\max} = 0.04822$

25. $\rho = 13452 + 21345 + 34521 + 45213 + 52134, \quad \lambda_{\max} = 0.1246$

26. $\rho = 13254 + 21435 + 34512 + 45321 + 52143, \quad \lambda_{\max} = 0.08312$

27. $\rho = 13245 + 21453 + 34512 + 45321 + 52134, \quad \lambda_{\max} = 0.07199$

28. $\rho = 13254 + 21435 + 34521 + 45312 + 52143, \quad \lambda_{\max} = 0.06554$

29. $\rho = 13245 + 21453 + 34521 + 45312 + 52134, \quad \lambda_{\max} = 0.06033$

30. $\rho = 13452 + 21534 + 34215 + 45321 + 52143, \quad \lambda_{\max} = 0.07891$

31. $\rho = 13452 + 21543 + 34215 + 45321 + 52134, \quad \lambda_{\max} = 0.07814$

32. $\rho = 13542 + 21453 + 34215 + 45321 + 52134, \quad \lambda_{\max} = 0.06671$

33. $\rho = 13452 + 21534 + 32145 + 45213 + 54321, \quad \lambda_{\max} = 0.08883$

34. $\rho = 13452 + 21534 + 32145 + 45321 + 54213, \quad \lambda_{\max} = 0.07434$

35. $\rho = 13542 + 21435 + 32154 + 45213 + 54321, \quad \lambda_{\max} = 0.1079$

36. $\rho = 13542 + 21435 + 32154 + 45321 + 54213, \quad \lambda_{\max} = 0.08360$

37. $\rho = 13245 + 21453 + 32514 + 45132 + 54321, \quad \lambda_{\max} = 0.08472$

38. $\rho = 13452 + 21345 + 32514 + 45123 + 54231, \quad \lambda_{\max} = 0.08923$

39. $\rho = 13425 + 21354 + 32541 + 45132 + 54213, \quad \lambda_{\max} = 0.03306$

40. $\rho = 13542 + 21354 + 32415 + 45123 + 54231, \quad \lambda_{\max} = 0.04184$

41. $\rho = 13524 + 21345 + 32451 + 45132 + 54213, \quad \lambda_{\max} = 0.05256$

42. $\rho = 13245 + 21453 + 32514 + 45321 + 54132, \quad \lambda_{\max} = 0.06759$

43. $\rho = 13452 + 21345 + 32514 + 45231 + 54123, \quad \lambda_{\max} = 0.09186$

44. $\rho = 13542 + 21354 + 32415 + 45231 + 54123, \quad \lambda_{\max} = 0.03334$

45. $\rho = 13524 + 21345 + 32451 + 45213 + 54132, \quad \lambda_{\max} = 0.05350$

46. $\rho = 13254 + 21435 + 35142 + 42513 + 54321, \quad \lambda_{\max} = 0.1138$

47. $\rho = 13425 + 21354 + 35142 + 42513 + 54231, \quad \lambda_{\max} = 0.02139$

48. $\rho = 13452 + 21345 + 35124 + 42513 + 54231, \quad \lambda_{\max} = 0.07841$

49. $\rho = 13425 + 21354 + 35142 + 42531 + 54213, \quad \lambda_{\max} = 0.01837$

50. $\rho = 13452 + 21345 + 35124 + 42531 + 54213, \quad \lambda_{\max} = 0.06327$

51. $\rho = 13452 + 21543 + 35124 + 42315 + 54231, \quad \lambda_{\max} = 0.06753$

52. $\rho = 13425 + 21534 + 35142 + 42351 + 54213, \quad \lambda_{\max} = 0.03159$

53. $\rho = 13524 + 21453 + 35142 + 42315 + 54231, \quad \lambda_{\max} = 0.03165$

54. $\rho = 13542 + 21453 + 35124 + 42315 + 54231, \quad \lambda_{\max} = 0.04908$

55. $\rho = 13524 + 21435 + 35142 + 42351 + 54213, \quad \lambda_{\max} = 0.02929$

56. $\rho = 13542 + 21435 + 35124 + 42351 + 54213, \quad \lambda_{\max} = 0.04051$

57. $\rho = 13542 + 21354 + 35421 + 42135 + 54213, \quad \lambda_{\max} = 0.04770$

58. $\rho = 13452 + 21543 + 35214 + 42135 + 54321, \quad \lambda_{\max} = 0.08553$

59. $\rho = 13542 + 21435 + 35214 + 42153 + 54321, \quad \lambda_{\max} = 0.09946$

60. $\rho = 13542 + 21453 + 35214 + 42135 + 54321, \quad \lambda_{\max} = 0.06601$

61. $\rho = 13245 + 21354 + 35421 + 42513 + 54132, \quad \lambda_{\max} = 0.03005$

62. $\rho = 13254 + 21345 + 35421 + 42513 + 54132, \quad \lambda_{\max} = 0.04494$

63. $\rho = 13254 + 21543 + 35421 + 42315 + 54132, \quad \lambda_{\max} = 0.08759$

64. $\rho = 13452 + 21345 + 35214 + 42531 + 54123, \quad \lambda_{\max} = 0.07204$

65. $\rho = 13425 + 21543 + 35214 + 42351 + 54132, \quad \lambda_{\max} = 0.06026$

66. $\rho = 13452 + 21534 + 35241 + 42315 + 54123, \quad \lambda_{\max} = 0.05898$

67. $\rho = 13542 + 21435 + 35214 + 42351 + 54123, \quad \lambda_{\max} = 0.04149$

68. $\rho = 13524 + 21453 + 35241 + 42315 + 54132, \quad \lambda_{\max} = 0.02786$

69. $\rho = 15432 + 21543 + 32154 + 43215 + 54321, \quad \lambda_{\max} = 0.2433$

70. $\rho = 15432 + 21345 + 32154 + 43521 + 54213, \quad \lambda_{\max} = 0.09158$

71. $\rho = 15432 + 21354 + 32145 + 43521 + 54213, \quad \lambda_{\max} = 0.07698$

72. $\rho = 15342 + 21453 + 32514 + 43125 + 54231, \quad \lambda_{\max} = 0.08903$

73. $\rho = 15324 + 21435 + 32541 + 43152 + 54213, \quad \lambda_{\max} = 0.08391$

74. $\rho = 15324 + 21543 + 32415 + 43152 + 54231, \quad \lambda_{\max} = 0.06952$

75. $\rho = 15342 + 21534 + 32451 + 43125 + 54213, \quad \lambda_{\max} = 0.06182$

76. $\rho = 15423 + 21345 + 32514 + 43152 + 54231, \quad \lambda_{\max} = 0.06688$

77. $\rho = 15432 + 21354 + 32541 + 43125 + 54213, \quad \lambda_{\max} = 0.08470$

78. $\rho = 15342 + 21435 + 32514 + 43251 + 54123, \quad \lambda_{\max} = 0.09044$

79. $\rho = 15324 + 21453 + 32541 + 43215 + 54132, \quad \lambda_{\max} = 0.09543$

80. $\rho = 15324 + 21543 + 32415 + 43251 + 54132, \quad \lambda_{\max} = 0.08273$

81. $\rho = 15342 + 21534 + 32415 + 43251 + 54123, \quad \lambda_{\max} = 0.06700$

82. $\rho = 15324 + 21543 + 32451 + 43215 + 54132, \quad \lambda_{\max} = 0.09488$

83. $\rho = 15342 + 21534 + 32451 + 43215 + 54123, \quad \lambda_{\max} = 0.07306$

84. $\rho = 15423 + 21345 + 32514 + 43251 + 54132, \quad \lambda_{\max} = 0.08365$

85. $\rho = 15432 + 21345 + 32514 + 43251 + 54123, \quad \lambda_{\max} = 0.09742$

86. $\rho = 15432 + 21354 + 32541 + 43215 + 54123, \quad \lambda_{\max} = 0.1038$

87. $\rho = 15324 + 21543 + 34152 + 43215 + 52431, \quad \lambda_{\max} = 0.08620$

88. $\rho = 15342 + 21534 + 34125 + 43251 + 52413, \quad \lambda_{\max} = 0.04520$

89. $\rho = 15423 + 21534 + 34152 + 43215 + 52341, \quad \lambda_{\max} = 0.07693$

90. $\rho = 15432 + 21543 + 34125 + 43251 + 52314, \quad \lambda_{\max} = 0.1147$

91. $\rho = 15324 + 21543 + 34215 + 43152 + 52431, \quad \lambda_{\max} = 0.07152$

92. $\rho = 15342 + 21534 + 34251 + 43125 + 52413, \quad \lambda_{\max} = 0.03895$

93. $\rho = 15423 + 21534 + 34215 + 43152 + 52341, \quad \lambda_{\max} = 0.06318$

94. $\rho = 15432 + 21543 + 34251 + 43125 + 52314, \quad \lambda_{\max} = 0.1049$

95. $\rho = 12453 + 21534 + 35142 + 43215 + 54321, \quad \lambda_{\max} = 0.1149$

96. $\rho = 12435 + 21543 + 35214 + 43152 + 54321, \quad \lambda_{\max} = 0.09955$

97. $\rho = 12543 + 21435 + 35214 + 43152 + 54321, \quad \lambda_{\max} = 0.1056$

98. $\rho = 12345 + 21534 + 35421 + 43152 + 54213, \quad \lambda_{\max} = 0.05533$

99. $\rho = 12534 + 21345 + 35421 + 43152 + 54213, \quad \lambda_{\max} = 0.04420$

100. $\rho = 14523 + 21435 + 35142 + 43251 + 52314, \quad \lambda_{\max} = 0.05703$

101. $\rho = 14325 + 21534 + 35142 + 43251 + 52413, \quad \lambda_{\max} = 0.08273$

102. $\rho = 14523 + 21354 + 35142 + 43215 + 52431, \quad \lambda_{\max} = 0.03874$

103. $\rho = 14532 + 21345 + 35124 + 43251 + 52413, \quad \lambda_{\max} = 0.03617$

104. $\rho = 14523 + 21435 + 35214 + 43152 + 52341, \quad \lambda_{\max} = 0.05802$

105. $\rho = 14523 + 21435 + 35241 + 43152 + 52314, \quad \lambda_{\max} = 0.03261$

106. $\rho = 14532 + 21453 + 35241 + 43125 + 52314, \quad \lambda_{\max} = 0.04586$

107. $\rho = \mathtt{14325} + \mathtt{21543} + \mathtt{35214} + \mathtt{43152} + \mathtt{52431}$, $\lambda_{\max} = 0.08978$

108. $\rho = \mathtt{14325} + \mathtt{21534} + \mathtt{35241} + \mathtt{43152} + \mathtt{52413}$, $\lambda_{\max} = 0.03932$

109. $\rho = \mathtt{14352} + \mathtt{21534} + \mathtt{35241} + \mathtt{43125} + \mathtt{52413}$, $\lambda_{\max} = 0.03322$

110. $\rho = \mathtt{14523} + \mathtt{21345} + \mathtt{35214} + \mathtt{43152} + \mathtt{52431}$, $\lambda_{\max} = 0.05521$

111. $\rho = \mathtt{14532} + \mathtt{21354} + \mathtt{35241} + \mathtt{43125} + \mathtt{52413}$, $\lambda_{\max} = 0.03026$

112. $\rho = \mathtt{14352} + \mathtt{21435} + \mathtt{35124} + \mathtt{42513} + \mathtt{53241}$, $\lambda_{\max} = 0.04670$

113. $\rho = \mathtt{14532} + \mathtt{21453} + \mathtt{35124} + \mathtt{42315} + \mathtt{53241}$, $\lambda_{\max} = 0.05947$

114. $\rho = \mathtt{14352} + \mathtt{21435} + \mathtt{35241} + \mathtt{42513} + \mathtt{53124}$, $\lambda_{\max} = 0.03429$

115. $\rho = \mathtt{14532} + \mathtt{21453} + \mathtt{35241} + \mathtt{42315} + \mathtt{53124}$, $\lambda_{\max} = 0.04347$

116. $\rho = \mathtt{15432} + \mathtt{21345} + \mathtt{34251} + \mathtt{42513} + \mathtt{53124}$, $\lambda_{\max} = 0.05556$

117. $\rho = \mathtt{15432} + \mathtt{21543} + \mathtt{34251} + \mathtt{42315} + \mathtt{53124}$, $\lambda_{\max} = 0.1033$

118. $\rho = \mathtt{15342} + \mathtt{21435} + \mathtt{34251} + \mathtt{42513} + \mathtt{53124}$, $\lambda_{\max} = 0.03458$

119. $\rho = \mathtt{12345} + \mathtt{25134} + \mathtt{31452} + \mathtt{43521} + \mathtt{54213}$, $\lambda_{\max} = 0.06679$

120. $\rho = \mathtt{12453} + \mathtt{25134} + \mathtt{31542} + \mathtt{43215} + \mathtt{54321}$, $\lambda_{\max} = 0.1171$

121. $\rho = \mathtt{12543} + \mathtt{25134} + \mathtt{31452} + \mathtt{43215} + \mathtt{54321}$, $\lambda_{\max} = 0.1198$

122. $\rho = \mathtt{12345} + \mathtt{25413} + \mathtt{31524} + \mathtt{43152} + \mathtt{54231}$, $\lambda_{\max} = 0.06219$

123. $\rho = \mathtt{12345} + \mathtt{25431} + \mathtt{31524} + \mathtt{43152} + \mathtt{54213}$, $\lambda_{\max} = 0.06136$

124. $\rho = \mathtt{12453} + \mathtt{25314} + \mathtt{31542} + \mathtt{43125} + \mathtt{54231}$, $\lambda_{\max} = 0.04329$

125. $\rho = \mathtt{12435} + \mathtt{25341} + \mathtt{31524} + \mathtt{43152} + \mathtt{54213}$, $\lambda_{\max} = 0.03901$

126. $\rho = \mathtt{12543} + \mathtt{25314} + \mathtt{31425} + \mathtt{43152} + \mathtt{54231}$, $\lambda_{\max} = 0.03449$

127. $\rho = \mathtt{12543} + \mathtt{25314} + \mathtt{31452} + \mathtt{43125} + \mathtt{54231}$, $\lambda_{\max} = 0.04206$

128. $\rho = \mathtt{12534} + \mathtt{25341} + \mathtt{31425} + \mathtt{43152} + \mathtt{54213}$, $\lambda_{\max} = 0.03967$

129. $\rho = \mathtt{12534} + \mathtt{25341} + \mathtt{31452} + \mathtt{43125} + \mathtt{54213}$, $\lambda_{\max} = 0.04514$

130. $\rho = \mathtt{12453} + \mathtt{25314} + \mathtt{31245} + \mathtt{43521} + \mathtt{54132}$, $\lambda_{\max} = 0.02940$

131. $\rho = \mathtt{12435} + \mathtt{25314} + \mathtt{31542} + \mathtt{43251} + \mathtt{54123}$, $\lambda_{\max} = 0.04687$

132. $\rho = \mathtt{12453} + \mathtt{25341} + \mathtt{31524} + \mathtt{43215} + \mathtt{54132}$, $\lambda_{\max} = 0.04799$

133. $\rho = \mathtt{12543} + \mathtt{25314} + \mathtt{31425} + \mathtt{43251} + \mathtt{54132}$, $\lambda_{\max} = 0.04505$

134. $\rho = \mathtt{12534} + \mathtt{25341} + \mathtt{31452} + \mathtt{43215} + \mathtt{54123}$, $\lambda_{\max} = 0.06277$

135. $\rho = \mathtt{15324} + \mathtt{23415} + \mathtt{31542} + \mathtt{42153} + \mathtt{54231}, \quad \lambda_{\max} = 0.07089$

136. $\rho = \mathtt{15342} + \mathtt{23415} + \mathtt{31524} + \mathtt{42153} + \mathtt{54231}, \quad \lambda_{\max} = 0.05373$

137. $\rho = \mathtt{15324} + \mathtt{23451} + \mathtt{31542} + \mathtt{42135} + \mathtt{54213}, \quad \lambda_{\max} = 0.05541$

138. $\rho = \mathtt{15342} + \mathtt{23451} + \mathtt{31524} + \mathtt{42135} + \mathtt{54213}, \quad \lambda_{\max} = 0.05112$

139. $\rho = \mathtt{15342} + \mathtt{23514} + \mathtt{31425} + \mathtt{42153} + \mathtt{54231}, \quad \lambda_{\max} = 0.03459$

140. $\rho = \mathtt{15324} + \mathtt{23541} + \mathtt{31452} + \mathtt{42135} + \mathtt{54213}, \quad \lambda_{\max} = 0.04550$

141. $\rho = \mathtt{15234} + \mathtt{23415} + \mathtt{31542} + \mathtt{42153} + \mathtt{54321}, \quad \lambda_{\max} = 0.08746$

142. $\rho = \mathtt{15243} + \mathtt{23514} + \mathtt{31452} + \mathtt{42135} + \mathtt{54321}, \quad \lambda_{\max} = 0.04086$

143. $\rho = \mathtt{15243} + \mathtt{23415} + \mathtt{31524} + \mathtt{42351} + \mathtt{54132}, \quad \lambda_{\max} = 0.03842$

144. $\rho = \mathtt{15234} + \mathtt{23415} + \mathtt{31542} + \mathtt{42351} + \mathtt{54123}, \quad \lambda_{\max} = 0.09232$

145. $\rho = \mathtt{15234} + \mathtt{23451} + \mathtt{31542} + \mathtt{42315} + \mathtt{54123}, \quad \lambda_{\max} = 0.09638$

146. $\rho = \mathtt{15243} + \mathtt{23514} + \mathtt{31425} + \mathtt{42351} + \mathtt{54132}, \quad \lambda_{\max} = 0.03014$

147. $\rho = \mathtt{15234} + \mathtt{23541} + \mathtt{31452} + \mathtt{42315} + \mathtt{54123}, \quad \lambda_{\max} = 0.08488$

148. $\rho = \mathtt{15324} + \mathtt{24135} + \mathtt{31452} + \mathtt{42513} + \mathtt{53241}, \quad \lambda_{\max} = 0.01928$

149. $\rho = \mathtt{15342} + \mathtt{24153} + \mathtt{31425} + \mathtt{42531} + \mathtt{53214}, \quad \lambda_{\max} = 0.02338$

150. $\rho = \mathtt{15432} + \mathtt{24153} + \mathtt{31524} + \mathtt{42315} + \mathtt{53241}, \quad \lambda_{\max} = 0.05412$

151. $\rho = \mathtt{15423} + \mathtt{24135} + \mathtt{31542} + \mathtt{42351} + \mathtt{53214}, \quad \lambda_{\max} = 0.05324$

152. $\rho = \mathtt{15324} + \mathtt{24513} + \mathtt{31452} + \mathtt{42135} + \mathtt{53241}, \quad \lambda_{\max} = 0.04040$

153. $\rho = \mathtt{15342} + \mathtt{24531} + \mathtt{31425} + \mathtt{42153} + \mathtt{53214}, \quad \lambda_{\max} = 0.06279$

154. $\rho = \mathtt{15432} + \mathtt{24315} + \mathtt{31524} + \mathtt{42153} + \mathtt{53241}, \quad \lambda_{\max} = 0.07236$

155. $\rho = \mathtt{15423} + \mathtt{24351} + \mathtt{31542} + \mathtt{42135} + \mathtt{53214}, \quad \lambda_{\max} = 0.06988$

156. $\rho = \mathtt{15243} + \mathtt{24315} + \mathtt{31452} + \mathtt{42531} + \mathtt{53124}, \quad \lambda_{\max} = 0.01698$

157. $\rho = \mathtt{15234} + \mathtt{24513} + \mathtt{31425} + \mathtt{42351} + \mathtt{53142}, \quad \lambda_{\max} = 0.04003$

158. $\rho = \mathtt{15243} + \mathtt{24531} + \mathtt{31452} + \mathtt{42315} + \mathtt{53124}, \quad \lambda_{\max} = 0.02687$

159. $\rho = \mathtt{13425} + \mathtt{25134} + \mathtt{31542} + \mathtt{42351} + \mathtt{54213}, \quad \lambda_{\max} = 0.03494$

160. $\rho = \mathtt{13542} + \mathtt{25134} + \mathtt{31425} + \mathtt{42351} + \mathtt{54213}, \quad \lambda_{\max} = 0.02303$

161. $\rho = \mathtt{13425} + \mathtt{25314} + \mathtt{31542} + \mathtt{42153} + \mathtt{54231}, \quad \lambda_{\max} = 0.05398$

162. $\rho = \mathtt{13542} + \mathtt{25314} + \mathtt{31425} + \mathtt{42153} + \mathtt{54231}, \quad \lambda_{\max} = 0.02158$

163. $\rho = 14325 + 25134 + 31452 + 42513 + 53241,\quad \lambda_{\max} = 0.04552$

164. $\rho = 14325 + 25143 + 31452 + 42531 + 53214,\quad \lambda_{\max} = 0.08453$

165. $\rho = 14523 + 25134 + 31452 + 42315 + 53241,\quad \lambda_{\max} = 0.06091$

166. $\rho = 14532 + 25143 + 31425 + 42351 + 53214,\quad \lambda_{\max} = 0.05878$

167. $\rho = 14352 + 25413 + 31524 + 42135 + 53241,\quad \lambda_{\max} = 0.03477$

168. $\rho = 14325 + 25431 + 31542 + 42153 + 53214,\quad \lambda_{\max} = 0.1622$

169. $\rho = 14523 + 25314 + 31452 + 42135 + 53241,\quad \lambda_{\max} = 0.03738$

170. $\rho = 14532 + 25314 + 31425 + 42153 + 53241,\quad \lambda_{\max} = 0.02537$

171. $\rho = 14523 + 25341 + 31452 + 42135 + 53214,\quad \lambda_{\max} = 0.05098$

172. $\rho = 14532 + 25341 + 31425 + 42153 + 53214,\quad \lambda_{\max} = 0.06710$

173. $\rho = 14523 + 25134 + 31452 + 43215 + 52341,\quad \lambda_{\max} = 0.08059$

174. $\rho = 14523 + 25314 + 31245 + 43152 + 52431,\quad \lambda_{\max} = 0.03114$

175. $\rho = 14523 + 25431 + 31245 + 43152 + 52314,\quad \lambda_{\max} = 0.04252$

176. $\rho = 14325 + 25413 + 31542 + 43251 + 52134,\quad \lambda_{\max} = 0.1018$

177. $\rho = 14352 + 25431 + 31524 + 43215 + 52143,\quad \lambda_{\max} = 0.09707$

178. $\rho = 14532 + 25314 + 31425 + 43251 + 52143,\quad \lambda_{\max} = 0.04306$

179. $\rho = 14523 + 25341 + 31452 + 43215 + 52134,\quad \lambda_{\max} = 0.06487$

180. $\rho = 15432 + 24153 + 31524 + 43215 + 52341,\quad \lambda_{\max} = 0.07239$

181. $\rho = 15234 + 24351 + 31542 + 43125 + 52413,\quad \lambda_{\max} = 0.02312$

182. $\rho = 15243 + 24531 + 31452 + 43125 + 52314,\quad \lambda_{\max} = 0.03402$

183. $\rho = 15423 + 24531 + 31245 + 43152 + 52314,\quad \lambda_{\max} = 0.03673$

184. $\rho = 15324 + 24531 + 31452 + 43215 + 52143,\quad \lambda_{\max} = 0.08648$

185. $\rho = 15423 + 24315 + 31542 + 43251 + 52134,\quad \lambda_{\max} = 0.07491$

186. $\rho = 15423 + 24351 + 31542 + 43215 + 52134,\quad \lambda_{\max} = 0.08137$

187. $\rho = 15432 + 24351 + 31524 + 43215 + 52143,\quad \lambda_{\max} = 0.1064$

188. $\rho = 12543 + 25431 + 34125 + 41352 + 53214,\quad \lambda_{\max} = 0.07624$

189. $\rho = 12543 + 25431 + 34215 + 41352 + 53124,\quad \lambda_{\max} = 0.06514$

190. $\rho = 15243 + 24531 + 32415 + 41352 + 53124,\quad \lambda_{\max} = 0.008799$

191. $\rho = 15423 + 23541 + 34215 + 41352 + 52134,\quad \lambda_{\max} = 0.02485$

192. $\rho = 14253 + 25314 + 31425 + 42531 + 53142,\quad \lambda_{\max}$: ad hoc

# Appendix D: Ad-hoc Constructions

Here, we handle the constant covers from Section A which elude the Hessian verification on one of their eigenvalues. Following a similar approach as in [1], we find, for each $\rho$, a permutation using simulated annealing whose associated step permuton $\mu$ yields a density $d(\rho, \mu)$ on the appropriate side of $d(\rho, \lambda)$, where $\lambda$ is the uniform measure on $[0, 1]^2$.

- $\rho = 3(\texttt{3412}) + 3(\texttt{2143}) + 2(\texttt{321}) + 2(\texttt{123})$; $\quad d(\rho, \lambda) = \frac{3}{4!} + \frac{3}{4!} + \frac{2}{3!} + \frac{2}{3!} = \frac{11}{12}$.
  Let $\mu$ be the step permuton based on `(4,5,7,12,11,3,6,10,2,1,8,9)`. Then
  $$d(\rho, \mu) = 3 \cdot \frac{1099}{41472} + 3 \cdot \frac{1357}{41472} + 2 \cdot \frac{169}{864} + 2 \cdot \frac{37}{216} = \frac{175}{192} < \frac{11}{12}.$$
  With $\xi = 2(\texttt{123}) - 2(\texttt{321}) - 3(\texttt{12})$, we have $d(\xi, \lambda) = \frac{2}{3!} - \frac{2}{3!} - \frac{3}{2!} = -\frac{3}{2}$ and $d(\xi, \mu) = -\frac{217}{144}$. The constant covers $\rho + t\xi$ satisfy
  $$d(\rho + t\xi, \mu) = \frac{175}{192} - \frac{217}{144}t < \frac{11}{12} - \frac{3}{2}t$$
  for all $t > -3/4$. This covers the range of $t$ for which the Hessian matrix lacks a negative eigenvalue.

- $\rho = -3(\texttt{4231}) - 3(\texttt{1324}) + 2(\texttt{321}) + 2(\texttt{123})$; $\quad d(\rho, \lambda) = -\frac{3}{4!} - \frac{3}{4!} + \frac{2}{3!} + \frac{2}{3!} = \frac{5}{12}$.
  Let $\mu$ be the step permuton based on `52341`. Then
  $$d(\rho, \mu) = -3 \cdot \frac{2389}{15000} - 3 \cdot \frac{49}{3000} + 2 \cdot \frac{239}{750} + 2 \cdot \frac{19}{150} = \frac{2729}{7500} < \frac{5}{12}.$$
  With $\xi$ as above, we compute $d(\xi, \mu) = -\frac{351}{250}$. The constant covers $\rho + t\xi$ satisfy
  $$d(\rho + t\xi, \mu) = \frac{2729}{2500} - \frac{351}{250}t < \frac{5}{12} - \frac{3}{2}t$$
  for all $t < 11/20$. This covers the range of $t$ for which the Hessian matrix lacks a negative eigenvalue.

- $\rho = 6(\texttt{4321}) + 3(\texttt{3412}) - 4(\texttt{1324}) + \texttt{1234} + 3(\texttt{12})$; $\quad d(\rho, \lambda) = \frac{6}{4!} + \frac{3}{4!} - \frac{4}{4!} + \frac{1}{4!} + \frac{3}{2!} = \frac{7}{4}$.
  Let $\mu$ be the step permuton based on `14325`. Then
  $$d(\rho, \mu) = 6 \cdot \frac{641}{15000} + 3 \cdot \frac{113}{15000} - 4 \cdot \frac{2389}{15000} + \frac{1777}{15000} + 3 \cdot \frac{33}{50} = \frac{4351}{2500} < \frac{7}{4}.$$

- $\rho = -6(\texttt{4321}) - 3(\texttt{3412}) + 4(\texttt{1324}) - \texttt{1234} + 3(\texttt{21})$; $\quad d(\rho, \lambda) = -\frac{6}{4!} - \frac{3}{4!} + \frac{4}{4!} - \frac{1}{4!} + \frac{3}{2!} = \frac{5}{4}$.
  Let $\mu$ be the step permuton based on `21543`. Then
  $$d(\rho, \mu) = -6 \cdot \frac{709}{15000} - 3 \cdot \frac{277}{15000} - 4 \cdot \frac{649}{3000} + \frac{413}{15000} + 3 \cdot \frac{21}{50} = \frac{4397}{2500} > \frac{5}{4}.$$

- $\rho = \texttt{14253} + \texttt{25314} + \texttt{31425} + \texttt{42531} + \texttt{53142}$; $\quad d(\rho, \lambda) = 5 \times \frac{1}{5!} = \frac{1}{24}$.
  Let $\mu$ be the step permuton based on `3164275`. Then
  $$d(\rho, \mu) = 6 \cdot \frac{641}{15000} + 3 \cdot \frac{113}{15000} - 4 \cdot \frac{2389}{15000} + \frac{1777}{15000} + 3 \cdot \frac{33}{50} = \frac{2911}{57624} > \frac{1}{24}.$$

# Appendix E: Some Code Details

Code for the non-vanishing constant cover search, written in Sage [2], can be found in the github repository `https://github.com/pbd345/qr-perms/`.

For expressions of length 5, the search is divided into cases roughly as follows. Given a list of lengths $n = k_1 \geq \cdots \geq k_r$, we may assume by first row considerations alone that

- $\sum_{j=1}^{4} n - k_j + 1 \geq n - 2$, and
- $\sum_{j=1}^{i-1} n - k_j + 1 \geq n - k_i + 1$ for each $i = 2, \ldots, 5$; in particular, $k_1 = k_2 = n$ and $k_3 \in \{n-1, n\}$.

These conditions imply $n \leq 10$ and leave fewer than 100 candidate lists to check. For $n \leq 5$, we conduct a full search of permutations. The search is feasible on its own, but exploiting repeated entries and interpolation (see below) can speed it up. It took roughly four minutes on a standard desktop computer (3.9 GHz processor) to find all constant covers in Appendix C, including their Hessian eigenvalues.

For $n \geq 6$, we implemented a search based on partial permutations of length $m$, using the fact that the first $m$ rows of a fuzzy permutation matrix $F_\sigma^{\uparrow n}$ depend only on $\sigma(1), \ldots, \sigma(m)$. Our search method began takes $(k_1, \ldots, k_5)$ as input and begins with $m = 1$. Every list of five partial permutations which produces a constant cover on the first $m$ rows is stored, if any exist. Then, after incrementing $m$, we search over only those partial permutations whose prefixes of length $m - 1$ match one of the previously stored lists. In practice, this method quickly ruled out each case with $6 \leq n \leq 10$ using only $m \in \{1, 2, 3\}$. Only two cases required $m = 3$; these were $(k_1, \ldots, k_5) = (6, 6, 6, 5, 4)$ and $(7, 7, 6, 5, 4)$. Pseudocode for the search is given below.

```
m = 1, prefixes(0) = [e,e,e,e,e], where e is the empty 0-perm
repeat
    prefixes(m) = []
    search m-perms of length k_i extending some list in prefixes(m-1)
    if a non-vanishing constant cover C of first m rows is found
        add C to prefixes(m)
    m = m+1
until prefixes(m) = [] or m > k_5
```

A summary of the search for $n \geq 6$ is shown in the table below, including the maximum number of rows necessary. This phase of the search took just over two minutes.

| $(k_1,\ldots,k_5)$ | $m$ | $(k_1,\ldots,k_5)$ | $m$ |
|---|---|---|---|
| (6, 6, 5, 3, –) | 2 | (7, 7, 7, 5, 4) | 1 |
| (6, 6, 5, 4, –) | 2 | (7, 7, 7, 5, 5) | 1 |
| (6, 6, 5, 5, –) | 2 | (7, 7, 7, 6, –) | 1 |
| (6, 6, 6, 4, –) | 2 | (8, 8, 7, 5, 2) | 1 |
| (6, 6, 6, 5, 2) | 2 | (8, 8, 7, 5, 3) | 2 |
| (6, 6, 6, 5, 3) | 2 | (8, 8, 7, 5, 4) | 1 |
| (6, 6, 6, 5, 4) | 3 | (8, 8, 7, 5, 5) | 2 |
| (6, 6, 6, 5, 5) | 2 | (8, 8, 7, 6, 2) | 1 |
| (6, 6, 6, 6, 2) | 1 | (8, 8, 7, 6, 3) | 1 |
| (6, 6, 6, 6, 3) | 2 | (8, 8, 7, 6, 4) | 2 |
| (6, 6, 6, 6, 4) | 2 | (8, 8, 7, 6, 5) | 2 |
| (6, 6, 6, 6, 5) | 2 | (8, 8, 7, 6, 6) | 1 |
| (7, 7, 6, 4, 2) | 2 | (8, 8, 7, 7, 2) | 1 |
| (7, 7, 6, 4, 3) | 2 | (8, 8, 7, 7, 3) | 2 |
| (7, 7, 6, 4, 4) | 1 | (8, 8, 7, 7, 4) | 1 |
| (7, 7, 6, 5, 2) | 2 | (8, 8, 7, 7, 5) | 1 |
| (7, 7, 6, 5, 3) | 2 | (8, 8, 7, 7, 6) | 1 |
| (7, 7, 6, 5, 4) | 3 | (8, 8, 7, 7, 7) | 1 |
| (7, 7, 6, 5, 5) | 1 | (8, 8, 8, 6, –) | 1 |
| (7, 7, 6, 6, –) | 1 | (9, 9, 8, 6, –) | 1 |
| (7, 7, 7, 5, 2) | 1 | (9, 9, 8, 7, –) | 1 |
| (7, 7, 7, 5, 3) | 2 | (10, 10, 9, 7, –) | 1 |

An interface for the reader to search specified length lists and check Hessian matrices can be found at `https://www.math.uvic.ca/~dukes/qr.html`.

## Remarks on alternate methods

We remark that various alternate methods of attack can rule out cases with $n > 5$, though we could not find a single unified approach besides the above search by rows.

Considering repeated entries is useful in cases with $k_1 = k_2 = k_3$. For instance, in the case $(k_1,\ldots,k_5) = (6,6,6,5,4)$, the first three $6 \times 6$ permutation matrices leave at least 18 zero entries; that is, $m_0(c_1F_1 + c_2F_2 + c_3F_3) \geq 18$. On the other hand, a quick computation shows $m_*(c_4F_4 + c_5F_5) \leq 16$, meaning a non-vanishing constant cover is impossible.

Another alternate method exploits polynomial interpolation. This has a lot of success in cases with $k_2 > k_3 > k_4 > k_5$, since the 'degree' of each partial sum $c_1F_1 + \cdots + c_rF_r$ must strictly decrease for $r = 1,\ldots,5$.

Let us associate each polynomial $f(x) \in \mathbb{R}[x]$, $\deg(f) < n$, with its list of values $\mathbf{f} = (f(1),\ldots,f(n)) \in \mathbb{R}^n$. With this in mind, the *degree* of a vector $\mathbf{f}$ is well-defined as an integer in $-1,0,\ldots,n-1$.

For $d < n$, consider a 'degree check matrix' $T_{n,d} \in \mathcal{R}^{n\times(n-d-1)}$, whose $(i,j)$-entry equals $(-1)^{i-1}\binom{n-j}{i-1}$.

**Claim.** A row vector $\mathbf{f} \in \mathbb{R}^n$ has degree $\leq d$ if and only if $\mathbf{f}\,T_{n,d} = \mathbf{0}$.

*Proof of claim.* We first check that this holds on a basis $\{\binom{x-1}{0}, \binom{x-1}{1}, \ldots, \binom{x-1}{d}\}$ for the polynomials of degree $\leq d$. We compute for each $h$, $0 \leq h \leq d$,

$$\left(\left(\tbinom{0}{h}, \tbinom{1}{h}, \ldots, \tbinom{n-1}{h}\right) T_{n,d}\right)_j = \sum_{i=0}^{n-1} (-1)^i \binom{i}{h}\binom{n-j}{i} = \binom{n-j}{h} \sum_{i=h}^{n-j} (-1)^i \binom{n-j-h}{i-h}$$

and this equals zero if $n - j - h > 0$. In particular, we obtain zeros in each entry for $h = 0, 1, \ldots, d$. Conversely, $T_{n,d}$ has linearly independent columns, and thus the dimension of its (left) kernel is at most $d + 1$. In other words, a vector $\mathbf{f}$ of degree greater than $d$ has $\mathbf{f}\, T_{n,d} \neq \mathbf{0}$. □

Now, suppose we are given a partial expression $B = c_1F_1 + \cdots + c_{i-1}F_{i-1}$ contributing to a constant cover, where $i \in \{2, 3, 4\}$. Let $T = T_{n,n-k_{i+1}-1}$ and consider the product $BT$. When looping over permutations $\sigma_i$, we need only consider those for which $F^{\uparrow n}_{\sigma_i} T$ is a multiple of $BT$. This is extremely rare in practice, but even if this coincidence occurs, it allows for us to uniquely determine the coefficient $c_i$ before moving on to the next ply of the search.

A special case of the above lets us determine the structure of the first two terms in a constant cover with $k_3 < k_2$.

**Claim.** If $k_1 = k_2 = n$ and $k_3 < n$, then $c_1 = (-1)^n c_2$ and, for each $i$, either $\sigma_1(i) + \sigma_2(i) = n + 1$ or $\sigma_1(i) + (-1)^n \sigma_2(i) = 0$. (The latter can occur only for odd $n$.)

*Proof of Claim.* Suppose wlog that $0 < |c_1| \leq |c_2|$. Consider the row in which $c_1$ appears in the first column, and suppose $c_2$ appears in position $i$. Then the interpolation condition becomes $c_1 = (-1)^i \binom{n-1}{i-1} c_2$. Taking absolute values of both sides shows that $i = n$, from which we have $c_1 = (-1)^n c_2$. When $n$ is even, the binomial coefficients $\binom{n-1}{i}$ pair up into $n/2$ equal pairs centred at $(n-1)/2$. This forces $\sigma_1(j) + \sigma_2(j) = n + 1$ for each $j$. When $n$ is odd, we have $c_1 = -c_2$. So, for each $j$ we have

$$(-1)^{\sigma_1(j)} \binom{n-1}{\sigma_1(j)-1} = (-1)^{\sigma_2(j)} \binom{n-1}{\sigma_2(j)-1},$$

for which the only solutions are $\sigma_1(j) = \sigma_2(j)$ or $\sigma_1(j) + \sigma_2(j) = n + 1$. □

# References


[1] T. F. N. Chan, D. Král', J. A. Noel, Y. Pehova, M. Sharifzadeh, and J. Volec. Characterization of quasirandom permutations by a pattern sum. *Random Structures Algorithms*, 57(4):920–939, 2020.

[2] SageMath, the Sage Mathematics Software System (Version 9.8), The Sage Developers, 2023, `http://www.sagemath.org`.
